# Supplementary material for: Large Berry curvature effects induced by extended nodal structures: Rational design strategy and high-throughput materials predictions
Source: arXiv:2506.03871 source file (2025-06-04)
Supplement: Supplementary file 1 [file SM-II_zip.pdf]

# Supplemental Material for “Large Berry curvature effects induced by extended nodal structures: rational design strategy and high-throughput materials predictions”:

## II. High-throughput materials predictions

Wencheng Wang<sup>1,2</sup>, Minxue Yang<sup>1</sup>, Wei Chen<sup>1</sup>, Xiangang Wan<sup>1,3,4</sup>, and Feng Tang<sup>1\*</sup>

<sup>1</sup>*National Laboratory of Solid State Microstructures and School of Physics, Nanjing University, Nanjing 210093, China and Collaborative Innovation Center of Advanced Microstructures, Nanjing University, Nanjing 210093, China*

<sup>2</sup>*International Quantum Academy, Shenzhen 518048, China*

<sup>3</sup>*Hefei National Laboratory, Hefei 230088, China and*

<sup>4</sup>*Jiangsu Physical Science Research Center*

(Dated: May 9, 2025)

### CONTENTS

|                                                                           |     |
|---------------------------------------------------------------------------|-----|
| SII1. Preliminary remarks                                                 | 1   |
| SII2. 75 Candidate materials exhibiting large anomalous Hall conductivity | 2   |
| SII3. First-principles calculation results for 90 materials               | 5   |
| References                                                                | 107 |

### SII1. PRELIMINARY REMARKS

In Supplemental Material II, we present high-throughput material prediction results obtained through our theoretical strategy with the MAGNDATA magnetic material database [1]. We first explicitly list the 75 candidate materials exhibiting anomalous Hall conductivity (AHC)  $\geq 100 \Omega^{-1} \text{cm}^{-1}$  in Sec. SII2. Then, we provide the detailed first-principles calculation results for 90 materials in Sec. SII3.

---

\* fengtang@nju.edu.cn

## SII2. 75 CANDIDATE MATERIALS EXHIBITING LARGE ANOMALOUS HALL CONDUCTIVITY

In this section, we summarize the calculation results for the 75 material exhibiting AHC  $\sigma \geq 100 \Omega^{-1}\text{cm}^{-1}$ , listed in three tables: 30 magnetic materials exhibiting AHC  $\sigma \geq 1000 \Omega^{-1}\text{cm}^{-1}$  in Table SIII1, 30 magnetic materials exhibiting AHC in the range of  $500 \leq \sigma < 1000 \Omega^{-1}\text{cm}^{-1}$  in Table SIII2, and 15 materials exhibiting AHC in the range of  $100 \leq \sigma < 500 \Omega^{-1}\text{cm}^{-1}$  in Table SIII3. For detailed calculation results, the material names in the tables can be clicked to navigate to their respective pages in this document. It is worth noting that, to the best of our knowledge, 59 of these 75 magnetic materials are newly proposed as candidates for exhibiting large AHC and have not been discussed previously. These 59 newly proposed candidate materials are indicated in the three tables.

TABLE SIII1. 30 materials exhibiting AHC in the range of  $\sigma \geq 1000 \Omega^{-1}\text{cm}^{-1}$ . The seven columns contain the nodal structures, material names in the database, MSGs, the symmetry-adapted AHC tensors of the MSGs, the values of AHC at the Fermi level, the maximum AHC values within an energy range of  $E_F \pm 1 \text{ eV}$ , and whether the material is newly proposed as a candidate exhibiting large AHC. For detailed calculation results, the material names can be clicked to navigate to their respective pages in this document. Notably, although the basis vectors of a material may differ from our convention by a unitary transformation, which results in corresponding unitary transformation in the AHC tensor relative to our theoretical result, the number of nonvanishing AHC components remains invariant.

| Nodal structures     | Materials                                                         | MSGs        | AHC tensors                     | AHC( $E_F$ ) ( $\Omega^{-1}\text{cm}^{-1}$ ) | Max(AHC)             | New? |
|----------------------|-------------------------------------------------------------------|-------------|---------------------------------|----------------------------------------------|----------------------|------|
| <b>Only SNLs</b>     |                                                                   |             |                                 |                                              |                      |      |
|                      | <a href="#">2.70 GdMg</a>                                         | III 15.89   | $(\sigma_{yz}, \sigma_{zx}, 0)$ | $(-381, 0, -1787)$                           | $(-381, 0, -1787)$   | New  |
|                      | <a href="#">0.226 NdCo<sub>2</sub></a>                            | III 15.89   | $(\sigma_{yz}, \sigma_{zx}, 0)$ | $(-475, 0, 79)$                              | $(866, 0, -1019)$    | New  |
|                      | <a href="#">0.149 Nd<sub>3</sub>Ru<sub>4</sub>Al<sub>12</sub></a> | III 63.462  | $(0, 0, \sigma_{xy})$           | $(0, 0, -532)$                               | $(0, 0, -1439)$      | New  |
|                      | <a href="#">0.173 Pr<sub>3</sub>Ru<sub>4</sub>Al<sub>12</sub></a> | III 63.462  | $(0, 0, \sigma_{xy})$           | $(0, 0, -541)$                               | $(0, 0, -1205)$      | New  |
|                      | <a href="#">0.395 MnPtGa</a>                                      | III 63.462  | $(0, 0, \sigma_{xy})$           | $(0, 0, 656)$                                | $(0, 0, 1009)$       |      |
|                      | <a href="#">0.403 NdCo<sub>2</sub></a>                            | III 74.559  | $(\sigma_{yz}, 0, 0)$           | $(-744, 0, 0)$                               | $(-1318, 0, 0)$      | New  |
|                      | <a href="#">2.28 NpNiGa<sub>5</sub></a>                           | III 74.559  | $(\sigma_{yz}, 0, 0)$           | $(412, 0, 0)$                                | $(-1993, 0, 0)$      | New  |
|                      | <a href="#">0.227 NdCo<sub>2</sub></a>                            | III 141.557 | $(0, 0, \sigma_{xy})$           | $(0, 0, 938)$                                | $(0, 0, -1309)$      | New  |
|                      | <a href="#">0.51 Ho<sub>2</sub>Ru<sub>2</sub>O<sub>7</sub></a>    | III 141.557 | $(0, 0, \sigma_{xy})$           | $(93, -31, -71)$                             | $(-300, -421, 1658)$ | New  |
|                      | <a href="#">0.169 U<sub>3</sub>As<sub>4</sub></a>                 | III 161.71  | $(0, 0, \sigma_{xy})$           | $(0, 0, 2649)$                               | $(0, 0, -3362)$      |      |
|                      | <a href="#">0.170 U<sub>3</sub>P<sub>4</sub></a>                  | III 161.71  | $(0, 0, \sigma_{xy})$           | $(0, 0, 2862)$                               | $(0, 0, 2977)$       | New  |
| <b>Only FNSs</b>     |                                                                   |             |                                 |                                              |                      |      |
|                      | <a href="#">0.449 Tb<sub>2</sub>Pt</a>                            | III 11.54   | $(\sigma_{yz}, \sigma_{zx}, 0)$ | $(-77, 0, -224)$                             | $(1257, 0, -237)$    | New  |
|                      | <a href="#">0.832 CeAuGe</a>                                      | III 36.175  | $(\sigma_{yz}, 0, 0)$           | $(140, 0, 0)$                                | $(-2287, 0, 0)$      | New  |
|                      | <a href="#">0.199 Mn<sub>3</sub>Sn</a>                            | III 63.463  | $(\sigma_{yz}, 0, 0)$           | $(25, 0, 45)$                                | $(1019, 0, -39)$     |      |
|                      | <a href="#">0.789 CeCuSi</a>                                      | III 63.463  | $(\sigma_{yz}, 0, 0)$           | $(-101, 0, 0)$                               | $(-1862, 0, 0)$      | New  |
|                      | <a href="#">0.200 Mn<sub>3</sub>Sn</a>                            | III 63.464  | $(0, \sigma_{zx}, 0)$           | $(0, 84, -5)$                                | $(0, -1133, -1)$     |      |
|                      | <a href="#">0.707 Tb<sub>2</sub>Ir<sub>3</sub>Ga<sub>9</sub></a>  | III 63.464  | $(0, \sigma_{zx}, 0)$           | $(0, -51, 0)$                                | $(0, 1124, 0)$       | New  |
|                      | <a href="#">0.772 PrMnSi<sub>2</sub></a>                          | III 63.464  | $(0, \sigma_{zx}, 0)$           | $(0, 315, 0)$                                | $(0, 1208, 0)$       | New  |
|                      | <a href="#">0.79 CaIrO<sub>3</sub></a>                            | III 63.464  | $(0, \sigma_{zx}, 0)$           | $(0, -5, 0)$                                 | $(0, 161, 0)$        |      |
|                      | <a href="#">0.184 Nd<sub>5</sub>Si<sub>4</sub></a>                | III 92.114  | $(0, 0, \sigma_{xy})$           | $(0, 0, -80)$                                | $(0, 0, -1545)$      | New  |
|                      | <a href="#">0.593 UPSe</a>                                        | III 129.417 | $(0, 0, \sigma_{xy})$           | $(0, 0, -1022)$                              | $(0, 0, 2312)$       | New  |
|                      | <a href="#">0.594 UAsS</a>                                        | III 129.417 | $(0, 0, \sigma_{xy})$           | $(0, 0, -1337)$                              | $(0, 0, 2855)$       | New  |
| <b>SNLs and FNSs</b> |                                                                   |             |                                 |                                              |                      |      |
|                      | <a href="#">0.481 HoNi</a>                                        | III 14.79   | $(\sigma_{yz}, \sigma_{zx}, 0)$ | $(-111, -196, 707)$                          | $(1, 132, 875)$      | New  |
|                      | <a href="#">0.664 Mn<sub>3</sub>Sn<sub>2</sub></a>                | III 14.79   | $(\sigma_{yz}, \sigma_{zx}, 0)$ | $(184, -18, -605)$                           | $(-26, -107, -1506)$ |      |
|                      | <a href="#">2.57 TbMn<sub>2</sub>Si<sub>2</sub></a>               | III 59.410  | $(\sigma_{yz}, 0, 0)$           | $(313, 0, 110)$                              | $(1009, 0, 384)$     | New  |
|                      | <a href="#">0.407 NdSi</a>                                        | III 62.446  | $(0, 0, \sigma_{xy})$           | $(0, 0, -656)$                               | $(0, 0, -1203)$      | New  |
|                      | <a href="#">0.687 DyPt</a>                                        | III 62.446  | $(0, 0, \sigma_{xy})$           | $(0, 0, -199)$                               | $(0, 0, -1279)$      | New  |
|                      | <a href="#">0.408 PrSi</a>                                        | III 62.447  | $(\sigma_{yz}, 0, 0)$           | $(-1308, 0, 0)$                              | $(-1928, 0, 0)$      | New  |
|                      | <a href="#">0.480 HoNi</a>                                        | III 62.447  | $(\sigma_{yz}, 0, 0)$           | $(-307, 0, 148)$                             | $(-1591, 0, -165)$   | New  |
|                      | <a href="#">0.685 ErPt</a>                                        | III 62.447  | $(\sigma_{yz}, 0, 0)$           | $(1485, 0, 0)$                               | $(1882, 0, 0)$       | New  |

TABLE III.2. 30 materials exhibiting AHC in the range of  $500 \leq \sigma < 1000 \Omega^{-1} \text{cm}^{-1}$ . The seven columns contain the nodal structures, material names in the database, MSGs, the symmetry-adapted AHC tensors of the MSGs, the values of AHC at the Fermi level, the maximum AHC values within an energy range of  $E_F \pm 1 \text{ eV}$ , and whether the material is newly proposed as a candidate exhibiting large AHC. For detailed calculation results, the material names can be clicked to navigate to their respective pages in this document. Notably, although the basis vectors of a material may differ from our convention by a unitary transformation, which results in a corresponding unitary transformation in the AHC tensor relative to our theoretical result, the number of nonvanishing AHC components remains invariant.

| Nodal structures | Materials                                                         | MSGs        | AHC tensors                     | AHC( $E_F$ ) ( $\Omega^{-1} \text{cm}^{-1}$ ) | Max(AHC)            | New? |
|------------------|-------------------------------------------------------------------|-------------|---------------------------------|-----------------------------------------------|---------------------|------|
| Only SNLs        | <a href="#">0.174 Pr<sub>3</sub>Ru<sub>4</sub>Al<sub>12</sub></a> | III 15.89   | $(\sigma_{yz}, \sigma_{zx}, 0)$ | (105, 0, -416)                                | (95, 0, 1001)       | New  |
|                  | <a href="#">0.690 NdPt</a>                                        | III 15.89   | $(\sigma_{yz}, \sigma_{zx}, 0)$ | (236, -45, 434)                               | (-40, -404, -893)   | New  |
|                  | <a href="#">2.12 TbMg</a>                                         | III 49.270  | $(0, \sigma_{zx}, 0)$           | (0, 83, 0)                                    | (0, 1123, 0)        | New  |
|                  | <a href="#">0.689 PrPt</a>                                        | III 63.462  | $(0, 0, \sigma_{xy})$           | (0, 0, -118)                                  | (0, 0, 622)         | New  |
|                  | <a href="#">0.985 EuPd<sub>3</sub>Si<sub>2</sub></a>              | III 74.559  | $(\sigma_{yz}, 0, 0)$           | (490, 0, 0)                                   | (-658, 0, 0)        | New  |
| Only FNSs        | <a href="#">0.106 DyVO<sub>3</sub></a>                            | III 11.54   | $(\sigma_{yz}, \sigma_{zx}, 0)$ | (-456, 0, -203)                               | (-722, 0, -202)     | New  |
|                  | <a href="#">2.97 GdMn<sub>2</sub>Si<sub>2</sub></a>               | III 59.409  | $(0, 0, \sigma_{xy})$           | (0, 0, -455)                                  | (0, 0, -972)        | New  |
|                  | <a href="#">0.279 Mn<sub>3</sub>As</a>                            | III 63.463  | $(\sigma_{yz}, 0, 0)$           | (371, -71, 0)                                 | (-751, 75, 0)       | New  |
|                  | <a href="#">0.280 Mn<sub>3</sub>As</a>                            | III 63.464  | $(0, \sigma_{zx}, 0)$           | (0, -56, -57)                                 | (0, 1602, -365)     | New  |
|                  | <a href="#">0.377 Mn<sub>3</sub>Ge</a>                            | III 63.464  | $(0, \sigma_{zx}, 0)$           | (0, 129, 62)                                  | (0, -576, -63)      |      |
|                  | <a href="#">0.778 LaMnSi<sub>2</sub></a>                          | III 63.464  | $(0, \sigma_{zx}, 0)$           | (0, 628, 0)                                   | (0, 996, 0)         | New  |
|                  | <a href="#">0.779 LaMnSi<sub>2</sub></a>                          | III 63.464  | $(0, \sigma_{zx}, 0)$           | (0, 628, 0)                                   | (0, 993, 0)         | New  |
|                  | <a href="#">0.780 LaMnSi<sub>2</sub></a>                          | III 63.464  | $(0, \sigma_{zx}, 0)$           | (0, 628, 0)                                   | (0, 995, 0)         | New  |
|                  | <a href="#">0.781 CeMnSi<sub>2</sub></a>                          | III 63.464  | $(0, \sigma_{zx}, 0)$           | (-124, 376, 141)                              | (159, -2238, -31)   | New  |
|                  | <a href="#">0.855 Mn<sub>2</sub>Sb</a>                            | III 129.417 | $(0, 0, \sigma_{xy})$           | (0, 0, -148)                                  | (0, 0, -802)        | New  |
| SNLs and FNSs    | <a href="#">0.796 Ca<sub>2</sub>NiOsO<sub>6</sub></a>             | III 14.79   | $(\sigma_{yz}, \sigma_{zx}, 0)$ | (-139, 0, -76)                                | (350, 0, -577)      | New  |
|                  | <a href="#">0.803 NbMnP</a>                                       | III 31.125  | $(0, \sigma_{zx}, 0)$           | (0, -266, 0)                                  | (0, -664, 0)        |      |
|                  | <a href="#">0.38 GaFeO<sub>3</sub></a>                            | III 33.147  | $(\sigma_{yz}, 0, 0)$           | (-456, -52, -37)                              | (-598, -131, 19)    | New  |
|                  | <a href="#">0.684 TbPt</a>                                        | III 62.446  | $(0, 0, \sigma_{xy})$           | (0, 0, 872)                                   | (0, 0, 977)         | New  |
|                  | <a href="#">0.732 SrRuO<sub>3</sub></a>                           | III 62.446  | $(0, 0, \sigma_{xy})$           | (0, 0, -385)                                  | (0, 0, -610)        |      |
|                  | <a href="#">0.686 HoPt</a>                                        | III 62.447  | $(\sigma_{yz}, 0, 0)$           | (581, 0, 0)                                   | (922, 0, 0)         | New  |
|                  | <a href="#">0.688 TmPt</a>                                        | III 62.447  | $(\sigma_{yz}, 0, 0)$           | (443, 0, 84)                                  | (724, 0, -37)       | New  |
|                  | <a href="#">0.834 CrSbSe<sub>3</sub></a>                          | III 62.447  | $(\sigma_{yz}, 0, 0)$           | (0, 0, 0)                                     | (154, 0, 0)         | New  |
|                  | <a href="#">0.1 LaMnO<sub>3</sub></a>                             | III 62.448  | $(0, \sigma_{zx}, 0)$           | (0, 0, 0)                                     | (11, -408, 1)       |      |
|                  | <a href="#">0.288 NdMnO<sub>3</sub></a>                           | III 62.448  | $(0, \sigma_{zx}, 0)$           | (0, 0, 0)                                     | (0, 35, 0)          | New  |
|                  | <a href="#">0.289 NdMnO<sub>3</sub></a>                           | III 62.448  | $(0, \sigma_{zx}, 0)$           | (0, 0, 0)                                     | (0, 91, 0)          | New  |
|                  | <a href="#">0.642 LaMnO<sub>3</sub></a>                           | III 62.448  | $(0, \sigma_{zx}, 0)$           | (0, 0, 0)                                     | (1, 160, 0)         |      |
|                  | <a href="#">0.662 Mn<sub>3</sub>Sn<sub>2</sub></a>                | III 62.448  | $(0, \sigma_{zx}, 0)$           | (0, 236, 0)                                   | (0, 803, 0)         |      |
|                  | <a href="#">0.663 Mn<sub>3</sub>Sn<sub>2</sub></a>                | III 62.448  | $(0, \sigma_{zx}, 0)$           | (99, 67, 11)                                  | (-1253, -266, -232) |      |

TABLE III. 15 materials exhibiting AHC in the range of  $100 \leq \sigma < 500 \Omega^{-1} \text{cm}^{-1}$ . The seven columns contain the nodal structures, material names in the database, MSGs, the symmetry-adapted AHC tensors of the MSGs, the values of AHC at the Fermi level, the maximum AHC values within an energy range of  $E_F \pm 1 \text{ eV}$ , and whether the material is newly proposed as a candidate exhibiting large AHC. For detailed calculation results, the material names can be clicked to navigate to their respective pages in this document. Notably, although the basis vectors of a material may differ from our convention by a unitary transformation, which results in a corresponding unitary transformation in the AHC tensor relative to our theoretical result, the number of nonvanishing AHC components remains invariant.

| Nodal structures     | Materials                                             | MSGs        | AHC tensors                          | AHC( $E_F$ ) ( $\Omega^{-1} \text{cm}^{-1}$ ) | Max(AHC)          | New? |
|----------------------|-------------------------------------------------------|-------------|--------------------------------------|-----------------------------------------------|-------------------|------|
| <b>Only SNLs</b>     | <a href="#">0.812 Fe<sub>2</sub>WO<sub>6</sub></a>    | III 30.113  | (0, $\sigma_{zx}$ , 0)               | (0, 0, 0)                                     | (224, 3, -41)     | New  |
|                      | <a href="#">0.11 DyFeO<sub>3</sub></a>                | III 33.148  | (0, 0, $\sigma_{xy}$ )               | (0, 0, 0)                                     | (0, 0, -169)      | New  |
|                      | <a href="#">0.886 SnCo<sub>2</sub>O<sub>4</sub></a>   | III 141.557 | (0, 0, $\sigma_{xy}$ )               | (34, -72, -119)                               | (-253, -91, -127) | New  |
|                      | <a href="#">0.286 Mn<sub>5</sub>Ge<sub>3</sub></a>    | III 193.260 | (0, 0, $\sigma_{xy}$ )               | (15, -45, 106)                                | (-25, 6, 452)     |      |
| <b>Only FNSs</b>     | <a href="#">0.358 CaFe<sub>5</sub>O<sub>7</sub></a>   | III 11.54   | ( $\sigma_{yz}$ , $\sigma_{zx}$ , 0) | (0, 3, -36)                                   | (0, 60, 164)      | New  |
| <b>SNLs and FNSs</b> | <a href="#">0.205 Sr<sub>2</sub>MnReO<sub>6</sub></a> | III 14.79   | ( $\sigma_{yz}$ , $\sigma_{zx}$ , 0) | (-26, -40, 168)                               | (104, -118, 243)  | New  |
|                      | <a href="#">0.319 Tm<sub>2</sub>CoMnO<sub>6</sub></a> | III 14.79   | ( $\sigma_{yz}$ , $\sigma_{zx}$ , 0) | (0, 0, 0)                                     | (-147, -32, 181)  | New  |
|                      | <a href="#">0.810 Fe<sub>2</sub>WO<sub>6</sub></a>    | III 60.423  | ( $\sigma_{yz}$ , 0, 0)              | (0, 0, 0)                                     | (19, 0, -204)     | New  |
|                      | <a href="#">0.811 Fe<sub>2</sub>WO<sub>6</sub></a>    | III 60.423  | ( $\sigma_{yz}$ , 0, 0)              | (0, 0, 0)                                     | (0, 530, 55)      | New  |
|                      | <a href="#">0.813 Fe<sub>2</sub>WO<sub>6</sub></a>    | III 60.423  | ( $\sigma_{yz}$ , 0, 0)              | (0, 0, 0)                                     | (0, -655, 28)     | New  |
|                      | <a href="#">0.445 MnCoGe</a>                          | III 62.446  | (0, 0, $\sigma_{xy}$ )               | (109, 0, 167)                                 | (-128, 0, 535)    | New  |
|                      | <a href="#">0.726 CsMn<sub>2</sub>F<sub>6</sub></a>   | III 62.447  | ( $\sigma_{yz}$ , 0, 0)              | (0, 0, 0)                                     | (494, 0, 0)       | New  |
|                      | <a href="#">0.25 NaOsO<sub>3</sub></a>                | III 62.448  | (0, $\sigma_{zx}$ , 0)               | (-1, -1, 0)                                   | (-14, 534, 0)     | New  |
|                      | <a href="#">0.513 YRuO<sub>3</sub></a>                | III 62.448  | (0, $\sigma_{zx}$ , 0)               | (0, 0, 0)                                     | (0, 439, 0)       | New  |
|                      | <a href="#">0.642 LaMnO<sub>3</sub></a>               | III 62.448  | (0, $\sigma_{zx}$ , 0)               | (0, 0, 0)                                     | (1, 160, 0)       |      |



### SII.3. FIRST-PRINCIPLES CALCULATION RESULTS FOR 90 MATERIALS

In this section, we present the material structures, theoretical results, and the first-principles calculation results for 90 magnetic materials. For each material, we begin with a brief description that includes its name in MAGNDATA magnetic material database, which consists of its entry and chemical formula. Note that, for the same chemical formula, different entries correspond to different magnetic configurations. By clicking on the material name, one can access its corresponding webpage in the database. We also provide its MSG, theoretical nodal structure type, and symmetry-adapted AHC tensor of the MSG. The detailed characteristics of the nodal structures are provided in Supplemental Material I [2]. Notably, the basis vectors of a material may differ from our convention by a unitary transformation, which results in corresponding unitary transformation in the coordinates of the SNLs and FNSs as well as in the AHC tensor relative to our theoretical result. However, the number of nonvanishing AHC components remains invariant. Below the description, we provide the comparison table of the experimental and calculated magnetic moments of the material, the first-principles band structure, and the Fermi-level-dependent AHC plot.

**0.149 Nd<sub>3</sub>Ru<sub>4</sub>Al<sub>12</sub>** crystallizes in type III MSG 63.462, which hosts only SNLs. The symmetry-adapted AHC tensor of the MSG is  $(0, 0, \sigma_{xy})$ . Based on the first-principles calculation results, the comparison between the experimental and calculated magnetic moments is provided in Table SII.4. The band structure is shown in the left panel of Fig. 1, and the Fermi-level-dependent AHC is plotted in the right panel.

FIG. 1. First-principles calculation results of 0.149 Nd<sub>3</sub>Ru<sub>4</sub>Al<sub>12</sub>. The band structure is shown in the left panel, and the Fermi-level-dependent AHC is plotted in the right panel. In both plots, the Fermi level is set to 0 eV.

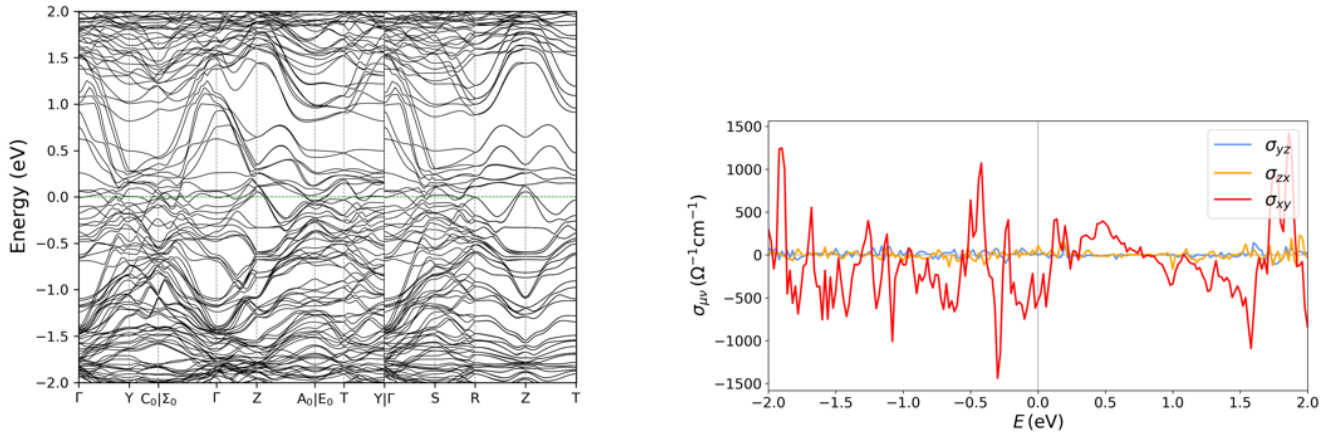

TABLE SII4. The comparison between the experimental and calculated magnetic moments for 0.149 Nd<sub>3</sub>Ru<sub>4</sub>Al<sub>12</sub>. The five columns contain the atom index in the structure file, the atom species, the fractional coordinates, the experimental magnetic moments, and the calculated magnetic moments. The lattice vectors are  $\vec{a}_1 = (4.4299, -7.67281, 0.0)$ ,  $\vec{a}_2 = (4.4299, 7.67281, 0.0)$ ,  $\vec{a}_3 = (0.0, 0.0, 9.6168)$ .

| No. | Atom | Coordinates(fractional) |          |          | Experimental magnetic moments |          |          | Calculated magnetic moments |           |           |
|-----|------|-------------------------|----------|----------|-------------------------------|----------|----------|-----------------------------|-----------|-----------|
| 1   | Nd   | 0.191050                | 0.808950 | 0.250000 | 0.000000                      | 0.000000 | 0.950040 | 0.001000                    | 0.000000  | 1.259000  |
| 2   | Nd   | 0.808950                | 0.191050 | 0.750000 | 0.000000                      | 0.000000 | 0.950040 | -0.001000                   | 0.000000  | 1.262000  |
| 3   | Nd   | 0.191040                | 0.382100 | 0.250000 | 0.000000                      | 0.000000 | 2.660010 | -0.000000                   | 0.001000  | 3.124000  |
| 4   | Nd   | 0.808960                | 0.617900 | 0.750000 | 0.000000                      | 0.000000 | 2.660010 | 0.001000                    | -0.001000 | 3.127000  |
| 5   | Nd   | 0.382100                | 0.191040 | 0.750000 | 0.000000                      | 0.000000 | 2.660010 | 0.000000                    | 0.001000  | 3.125000  |
| 6   | Nd   | 0.617900                | 0.808960 | 0.250000 | 0.000000                      | 0.000000 | 2.660010 | -0.001000                   | -0.001000 | 3.125000  |
| 7   | Ru   | 0.000000                | 0.000000 | 0.000000 | 0.000000                      | 0.000000 | 0.000000 | 0.000000                    | 0.001000  | 0.002000  |
| 8   | Ru   | 0.000000                | 0.000000 | 0.500000 | 0.000000                      | 0.000000 | 0.000000 | -0.000000                   | -0.001000 | 0.000000  |
| 9   | Ru   | 0.500000                | 0.500000 | 0.000000 | 0.000000                      | 0.000000 | 0.000000 | 0.000000                    | -0.001000 | -0.012000 |
| 10  | Ru   | 0.500000                | 0.500000 | 0.500000 | 0.000000                      | 0.000000 | 0.000000 | -0.000000                   | 0.000000  | -0.013000 |
| 11  | Ru   | 0.000000                | 0.500000 | 0.000000 | 0.000000                      | 0.000000 | 0.000000 | -0.001000                   | -0.001000 | 0.021000  |
| 12  | Ru   | 0.000000                | 0.500000 | 0.500000 | 0.000000                      | 0.000000 | 0.000000 | 0.000000                    | 0.000000  | 0.020000  |
| 13  | Ru   | 0.500000                | 0.000000 | 0.000000 | 0.000000                      | 0.000000 | 0.000000 | 0.001000                    | -0.000000 | 0.026000  |
| 14  | Ru   | 0.500000                | 0.000000 | 0.500000 | 0.000000                      | 0.000000 | 0.000000 | -0.002000                   | 0.001000  | 0.026000  |
| 15  | Al   | 0.561590                | 0.438410 | 0.250000 | 0.000000                      | 0.000000 | 0.000000 | -0.001000                   | -0.000000 | -0.002000 |
| 16  | Al   | 0.438410                | 0.561590 | 0.750000 | 0.000000                      | 0.000000 | 0.000000 | 0.001000                    | -0.000000 | -0.002000 |
| 17  | Al   | 0.561590                | 0.123170 | 0.250000 | 0.000000                      | 0.000000 | 0.000000 | 0.000000                    | -0.001000 | -0.000000 |
| 18  | Al   | 0.438410                | 0.876830 | 0.750000 | 0.000000                      | 0.000000 | 0.000000 | -0.000000                   | 0.000000  | -0.001000 |
| 19  | Al   | 0.123170                | 0.561590 | 0.750000 | 0.000000                      | 0.000000 | 0.000000 | -0.000000                   | -0.000000 | -0.000000 |
| 20  | Al   | 0.876830                | 0.438410 | 0.250000 | 0.000000                      | 0.000000 | 0.000000 | 0.000000                    | 0.001000  | -0.000000 |
| 21  | Al   | 0.162310                | 0.837690 | 0.575400 | 0.000000                      | 0.000000 | 0.000000 | -0.000000                   | -0.000000 | -0.002000 |
| 22  | Al   | 0.837690                | 0.162310 | 0.075400 | 0.000000                      | 0.000000 | 0.000000 | -0.000000                   | 0.000000  | -0.001000 |
| 23  | Al   | 0.837690                | 0.162310 | 0.424600 | 0.000000                      | 0.000000 | 0.000000 | -0.000000                   | -0.000000 | -0.002000 |
| 24  | Al   | 0.162310                | 0.837690 | 0.924600 | 0.000000                      | 0.000000 | 0.000000 | 0.000000                    | -0.000000 | -0.001000 |
| 25  | Al   | 0.162320                | 0.324620 | 0.575400 | 0.000000                      | 0.000000 | 0.000000 | -0.000000                   | -0.000000 | 0.001000  |
| 26  | Al   | 0.837680                | 0.675380 | 0.075400 | 0.000000                      | 0.000000 | 0.000000 | 0.000000                    | -0.000000 | 0.001000  |
| 27  | Al   | 0.837680                | 0.675380 | 0.424600 | 0.000000                      | 0.000000 | 0.000000 | -0.000000                   | -0.000000 | 0.001000  |
| 28  | Al   | 0.162320                | 0.324620 | 0.924600 | 0.000000                      | 0.000000 | 0.000000 | 0.000000                    | 0.000000  | 0.000000  |
| 29  | Al   | 0.324620                | 0.162320 | 0.424600 | 0.000000                      | 0.000000 | 0.000000 | 0.000000                    | -0.000000 | 0.001000  |
| 30  | Al   | 0.675380                | 0.837680 | 0.924600 | 0.000000                      | 0.000000 | 0.000000 | -0.000000                   | 0.000000  | 0.001000  |
| 31  | Al   | 0.675380                | 0.837680 | 0.575400 | 0.000000                      | 0.000000 | 0.000000 | 0.000000                    | -0.000000 | 0.001000  |
| 32  | Al   | 0.324620                | 0.162320 | 0.075400 | 0.000000                      | 0.000000 | 0.000000 | -0.000000                   | 0.000000  | 0.001000  |
| 33  | Al   | 0.666667                | 0.333333 | 0.508660 | 0.000000                      | 0.000000 | 0.000000 | 0.000000                    | -0.000000 | 0.006000  |
| 34  | Al   | 0.333333                | 0.666667 | 0.008660 | 0.000000                      | 0.000000 | 0.000000 | 0.000000                    | -0.000000 | 0.006000  |
| 35  | Al   | 0.333333                | 0.666667 | 0.491340 | 0.000000                      | 0.000000 | 0.000000 | -0.000000                   | 0.000000  | 0.006000  |
| 36  | Al   | 0.666667                | 0.333333 | 0.991340 | 0.000000                      | 0.000000 | 0.000000 | -0.000000                   | 0.000000  | 0.005000  |
| 37  | Al   | 0.000000                | 0.000000 | 0.250000 | 0.000000                      | 0.000000 | 0.000000 | 0.000000                    | 0.000000  | 0.002000  |
| 38  | Al   | 0.000000                | 0.000000 | 0.750000 | 0.000000                      | 0.000000 | 0.000000 | 0.000000                    | 0.000000  | 0.002000  |

**0.169 U<sub>3</sub>As<sub>4</sub>** crystallizes in type III MSG 161.71, which hosts only SNLs. The symmetry-adapted AHC tensor of the MSG is  $(0, 0, \sigma_{xy})$ . Based on the first-principles calculation results, the comparison between the experimental and calculated magnetic moments is provided in Table SII5. The band structure is shown in the left panel of Fig. 2, and the Fermi-level-dependent AHC is plotted in the right panel.

TABLE SII5. The comparison between the experimental and calculated magnetic moments for 0.169 U<sub>3</sub>As<sub>4</sub>. The five columns contain the atom index in the structure file, the atom species, the fractional coordinates, the experimental magnetic moments, and the calculated magnetic moments. The lattice vectors are  $\vec{a}_1 = (6.008285, 3.468884962, 2.452873333)$ ,  $\vec{a}_2 = (-6.008285, 3.468884962, 2.452873333)$ ,  $\vec{a}_3 = (0.0, -6.937769924, 2.452873333)$ .

| No. | Atom | Coordinates(fractional) |           |          | Experimental magnetic moments |           |           | Calculated magnetic moments |           |           |
|-----|------|-------------------------|-----------|----------|-------------------------------|-----------|-----------|-----------------------------|-----------|-----------|
| 1   | U    | 0.625000                | 0.375000  | 0.750000 | -0.000480                     | -0.898090 | -1.674010 | 0.003000                    | -1.090000 | -2.028000 |
| 2   | U    | 0.750000                | 0.625000  | 0.375000 | 0.778010                      | 0.448630  | -1.674010 | 0.947000                    | 0.544000  | -2.027000 |
| 3   | U    | 0.375000                | 0.750000  | 0.625000 | -0.777530                     | 0.449460  | -1.674010 | -0.946000                   | 0.540000  | -2.013000 |
| 4   | U    | 0.250000                | 0.875000  | 0.125000 | 0.777530                      | 0.449460  | -1.674010 | 0.946000                    | 0.542000  | -2.026000 |
| 5   | U    | 0.125000                | 0.250000  | 0.875000 | -0.778010                     | 0.448630  | -1.674010 | -0.938000                   | 0.553000  | -2.013000 |
| 6   | U    | 0.875000                | 0.125000  | 0.250000 | 0.000480                      | -0.898090 | -1.674010 | 0.008000                    | -1.092000 | -2.029000 |
| 7   | As   | 0.834000                | 0.834000  | 0.834000 | 0.000000                      | 0.000000  | 0.000000  | -0.000000                   | -0.003000 | 0.122000  |
| 8   | As   | 0.334000                | 0.334000  | 0.334000 | 0.000000                      | 0.000000  | 0.000000  | 0.000000                    | 0.001000  | 0.122000  |
| 9   | As   | 0.666000                | 0.999990  | 0.500000 | 0.000000                      | 0.000000  | 0.000000  | 0.000000                    | -0.002000 | 0.123000  |
| 10  | As   | 0.500000                | 0.666000  | 0.999990 | 0.000000                      | 0.000000  | 0.000000  | 0.000000                    | -0.001000 | 0.123000  |
| 11  | As   | 0.999990                | 0.500000  | 0.666000 | 0.000000                      | 0.000000  | 0.000000  | -0.000000                   | -0.001000 | 0.123000  |
| 12  | As   | 0.000000                | 0.499990  | 0.166000 | 0.000000                      | 0.000000  | 0.000000  | 0.001000                    | 0.001000  | 0.124000  |
| 13  | As   | 0.166000                | -0.000000 | 0.499990 | 0.000000                      | 0.000000  | 0.000000  | -0.001000                   | 0.002000  | 0.122000  |
| 14  | As   | 0.499990                | 0.166000  | 0.000000 | 0.000000                      | 0.000000  | 0.000000  | 0.001000                    | 0.001000  | 0.123000  |

FIG. 2. First-principles calculation results of 0.169 U<sub>3</sub>As<sub>4</sub>. The band structure is shown in the left panel, and the Fermi-level-dependent AHC is plotted in the right panel. In both plots, the Fermi level is set to 0 eV.

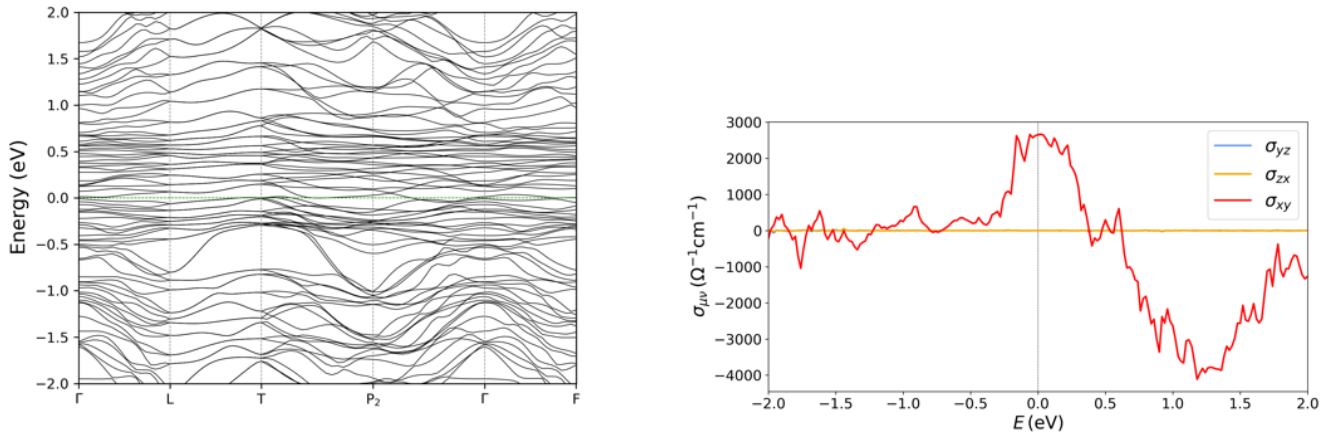

**0.170 U<sub>3</sub>P<sub>4</sub>** crystallizes in type III MSG 161.71, which hosts only SNLs. The symmetry-adapted AHC tensor of the MSG is  $(0, 0, \sigma_{xy})$ . Based on the first-principles calculation results, the comparison between the experimental and calculated magnetic moments is provided in Table SII6. The band structure is shown in the left panel of Fig. 3, and the Fermi-level-dependent AHC is plotted in the right panel.

TABLE SII6. The comparison between the experimental and calculated magnetic moments for 0.170 U<sub>3</sub>P<sub>4</sub>. The five columns contain the atom index in the structure file, the atom species, the fractional coordinates, the experimental magnetic moments, and the calculated magnetic moments. The lattice vectors are  $\vec{a}_1 = (5.80676, 3.352534449, 2.3706)$ ,  $\vec{a}_2 = (-5.80676, 3.352534449, 2.3706)$ ,  $\vec{a}_3 = (0.0, -6.705068898, 2.3706)$ .

| No. | Atom | Coordinates(fractional) |           |          | Experimental magnetic moments |           |           | Calculated magnetic moments |           |           |
|-----|------|-------------------------|-----------|----------|-------------------------------|-----------|-----------|-----------------------------|-----------|-----------|
| 1   | U    | 0.625000                | 0.375000  | 0.750000 | -0.000460                     | -0.326470 | -1.442980 | 0.001000                    | -0.401000 | -1.850000 |
| 2   | U    | 0.750000                | 0.625000  | 0.375000 | 0.282960                      | 0.162830  | -1.442980 | 0.353000                    | 0.200000  | -1.859000 |
| 3   | U    | 0.375000                | 0.750000  | 0.625000 | -0.282500                     | 0.163640  | -1.442980 | -0.354000                   | 0.197000  | -1.840000 |
| 4   | U    | 0.250000                | 0.875000  | 0.125000 | 0.282500                      | 0.163640  | -1.442980 | 0.355000                    | 0.203000  | -1.858000 |
| 5   | U    | 0.125000                | 0.250000  | 0.875000 | -0.282960                     | 0.162830  | -1.442980 | -0.343000                   | 0.208000  | -1.829000 |
| 6   | U    | 0.875000                | 0.125000  | 0.250000 | 0.000460                      | -0.326470 | -1.442980 | 0.006000                    | -0.402000 | -1.862000 |
| 7   | P    | 0.834000                | 0.834000  | 0.834000 | 0.000000                      | 0.000000  | 0.000000  | -0.000000                   | -0.001000 | 0.108000  |
| 8   | P    | 0.334000                | 0.334000  | 0.334000 | 0.000000                      | 0.000000  | 0.000000  | -0.000000                   | 0.001000  | 0.108000  |
| 9   | P    | 0.666000                | 0.999990  | 0.500000 | 0.000000                      | 0.000000  | 0.000000  | 0.001000                    | -0.001000 | 0.108000  |
| 10  | P    | 0.500000                | 0.666000  | 0.999990 | 0.000000                      | 0.000000  | 0.000000  | -0.000000                   | -0.000000 | 0.109000  |
| 11  | P    | 0.999990                | 0.500000  | 0.666000 | 0.000000                      | 0.000000  | 0.000000  | -0.000000                   | -0.000000 | 0.109000  |
| 12  | P    | 0.000000                | 0.499990  | 0.166000 | 0.000000                      | 0.000000  | 0.000000  | 0.001000                    | -0.000000 | 0.109000  |
| 13  | P    | 0.166000                | -0.000000 | 0.499990 | 0.000000                      | 0.000000  | 0.000000  | -0.000000                   | 0.001000  | 0.108000  |
| 14  | P    | 0.499990                | 0.166000  | 0.000000 | 0.000000                      | 0.000000  | 0.000000  | 0.000000                    | 0.001000  | 0.108000  |

FIG. 3. First-principles calculation results of 0.170 U<sub>3</sub>P<sub>4</sub>. The band structure is shown in the left panel, and the Fermi-level-dependent AHC is plotted in the right panel. In both plots, the Fermi level is set to 0 eV.

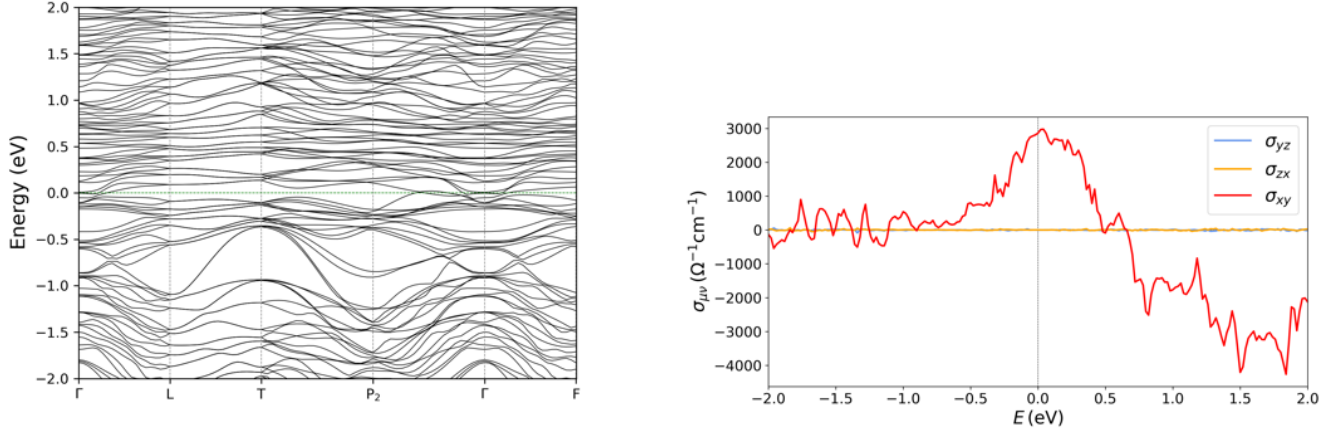

**0.173 Pr<sub>3</sub>Ru<sub>4</sub>Al<sub>12</sub>** crystallizes in type III MSG 63.462, which hosts only SNLs. The symmetry-adapted AHC tensor of the MSG is  $(0, 0, \sigma_{xy})$ . Based on the first-principles calculation results, the comparison between the experimental and calculated magnetic moments is provided in Table SII7. The band structure is shown in the left panel of Fig. 4, and the Fermi-level-dependent AHC is plotted in the right panel.

TABLE SII7. The comparison between the experimental and calculated magnetic moments for 0.173 Pr<sub>3</sub>Ru<sub>4</sub>Al<sub>12</sub>. The five columns contain the atom index in the structure file, the atom species, the fractional coordinates, the experimental magnetic moments, and the calculated magnetic moments. The lattice vectors are  $\vec{a}_1 = (4.429, -7.671255, 0.0)$ ,  $\vec{a}_2 = (4.429, 7.671255, 0.0)$ ,  $\vec{a}_3 = (0.0, 0.0, 9.624)$ .

| No. | Atom | Coordinates(fractional) |          |          | Experimental magnetic moments |          |          | Calculated magnetic moments |           |           |
|-----|------|-------------------------|----------|----------|-------------------------------|----------|----------|-----------------------------|-----------|-----------|
| 1   | Pr   | 0.191650                | 0.808350 | 0.250000 | 0.000000                      | 0.000000 | 3.099990 | 0.000000                    | -0.000000 | 2.745000  |
| 2   | Pr   | 0.808350                | 0.191650 | 0.750000 | 0.000000                      | 0.000000 | 3.099990 | -0.001000                   | -0.000000 | 2.749000  |
| 3   | Pr   | 0.191660                | 0.383300 | 0.250000 | 0.000000                      | 0.000000 | 1.400000 | -0.000000                   | 0.000000  | 1.713000  |
| 4   | Pr   | 0.808340                | 0.616700 | 0.750000 | 0.000000                      | 0.000000 | 1.400000 | 0.001000                    | -0.002000 | 1.714000  |
| 5   | Pr   | 0.383300                | 0.191660 | 0.750000 | 0.000000                      | 0.000000 | 1.400000 | 0.001000                    | 0.001000  | 1.714000  |
| 6   | Pr   | 0.616700                | 0.808340 | 0.250000 | 0.000000                      | 0.000000 | 1.400000 | -0.000000                   | -0.001000 | 1.713000  |
| 7   | Ru   | 0.000000                | 0.000000 | 0.000000 | 0.000000                      | 0.000000 | 0.000000 | 0.000000                    | -0.002000 | -0.053000 |
| 8   | Ru   | 0.000000                | 0.000000 | 0.500000 | 0.000000                      | 0.000000 | 0.000000 | 0.000000                    | 0.002000  | -0.048000 |
| 9   | Ru   | 0.500000                | 0.500000 | 0.000000 | 0.000000                      | 0.000000 | 0.000000 | 0.000000                    | 0.002000  | -0.026000 |
| 10  | Ru   | 0.500000                | 0.500000 | 0.500000 | 0.000000                      | 0.000000 | 0.000000 | -0.000000                   | -0.002000 | -0.026000 |
| 11  | Ru   | 0.000000                | 0.500000 | 0.000000 | 0.000000                      | 0.000000 | 0.000000 | 0.001000                    | -0.002000 | -0.156000 |
| 12  | Ru   | 0.000000                | 0.500000 | 0.500000 | 0.000000                      | 0.000000 | 0.000000 | -0.001000                   | -0.000000 | -0.153000 |
| 13  | Ru   | 0.500000                | 0.000000 | 0.000000 | 0.000000                      | 0.000000 | 0.000000 | -0.002000                   | 0.000000  | -0.156000 |
| 14  | Ru   | 0.500000                | 0.000000 | 0.500000 | 0.000000                      | 0.000000 | 0.000000 | 0.002000                    | 0.000000  | -0.151000 |
| 15  | Al   | 0.561760                | 0.438240 | 0.250000 | 0.000000                      | 0.000000 | 0.000000 | -0.001000                   | -0.000000 | -0.001000 |
| 16  | Al   | 0.438240                | 0.561760 | 0.750000 | 0.000000                      | 0.000000 | 0.000000 | 0.000000                    | -0.000000 | -0.001000 |
| 17  | Al   | 0.561760                | 0.123520 | 0.250000 | 0.000000                      | 0.000000 | 0.000000 | 0.000000                    | -0.000000 | -0.005000 |
| 18  | Al   | 0.438240                | 0.876480 | 0.750000 | 0.000000                      | 0.000000 | 0.000000 | -0.000000                   | 0.000000  | -0.005000 |
| 19  | Al   | 0.123520                | 0.561760 | 0.750000 | 0.000000                      | 0.000000 | 0.000000 | -0.000000                   | -0.000000 | -0.005000 |
| 20  | Al   | 0.876480                | 0.438240 | 0.250000 | 0.000000                      | 0.000000 | 0.000000 | 0.000000                    | 0.000000  | -0.005000 |
| 21  | Al   | 0.162290                | 0.837710 | 0.575580 | 0.000000                      | 0.000000 | 0.000000 | -0.000000                   | 0.000000  | 0.001000  |
| 22  | Al   | 0.837710                | 0.162290 | 0.075580 | 0.000000                      | 0.000000 | 0.000000 | -0.000000                   | -0.000000 | 0.001000  |
| 23  | Al   | 0.837710                | 0.162290 | 0.424420 | 0.000000                      | 0.000000 | 0.000000 | -0.000000                   | 0.000000  | 0.001000  |
| 24  | Al   | 0.162290                | 0.837710 | 0.924420 | 0.000000                      | 0.000000 | 0.000000 | 0.000000                    | -0.000000 | 0.001000  |
| 25  | Al   | 0.162300                | 0.324580 | 0.575580 | 0.000000                      | 0.000000 | 0.000000 | 0.000000                    | -0.000000 | -0.005000 |
| 26  | Al   | 0.837700                | 0.675420 | 0.075580 | 0.000000                      | 0.000000 | 0.000000 | -0.000000                   | -0.000000 | -0.005000 |
| 27  | Al   | 0.837700                | 0.675420 | 0.424420 | 0.000000                      | 0.000000 | 0.000000 | 0.000000                    | -0.000000 | -0.004000 |
| 28  | Al   | 0.162300                | 0.324580 | 0.924420 | 0.000000                      | 0.000000 | 0.000000 | 0.000000                    | -0.000000 | -0.006000 |
| 29  | Al   | 0.324580                | 0.162300 | 0.424420 | 0.000000                      | 0.000000 | 0.000000 | -0.000000                   | 0.000000  | -0.005000 |
| 30  | Al   | 0.675420                | 0.837700 | 0.924420 | 0.000000                      | 0.000000 | 0.000000 | 0.000000                    | -0.000000 | -0.005000 |
| 31  | Al   | 0.675420                | 0.837700 | 0.575580 | 0.000000                      | 0.000000 | 0.000000 | -0.000000                   | 0.000000  | -0.005000 |
| 32  | Al   | 0.324580                | 0.162300 | 0.075580 | 0.000000                      | 0.000000 | 0.000000 | 0.000000                    | -0.000000 | -0.004000 |
| 33  | Al   | 0.666667                | 0.333333 | 0.507810 | 0.000000                      | 0.000000 | 0.000000 | 0.000000                    | -0.000000 | 0.010000  |
| 34  | Al   | 0.333333                | 0.666667 | 0.007810 | 0.000000                      | 0.000000 | 0.000000 | 0.000000                    | -0.000000 | 0.010000  |
| 35  | Al   | 0.333333                | 0.666667 | 0.492190 | 0.000000                      | 0.000000 | 0.000000 | -0.000000                   | 0.000000  | 0.011000  |
| 36  | Al   | 0.666667                | 0.333333 | 0.992190 | 0.000000                      | 0.000000 | 0.000000 | 0.000000                    | -0.000000 | 0.010000  |
| 37  | Al   | 0.000000                | 0.000000 | 0.250000 | 0.000000                      | 0.000000 | 0.000000 | -0.000000                   | 0.000000  | 0.001000  |
| 38  | Al   | 0.000000                | 0.000000 | 0.750000 | 0.000000                      | 0.000000 | 0.000000 | 0.000000                    | 0.000000  | 0.001000  |

FIG. 4. First-principles calculation results of  $0.173 \text{ Pr}_3\text{Ru}_4\text{Al}_{12}$ . The band structure is shown in the left panel, and the Fermi-level-dependent AHC is plotted in the right panel. In both plots, the Fermi level is set to 0 eV.

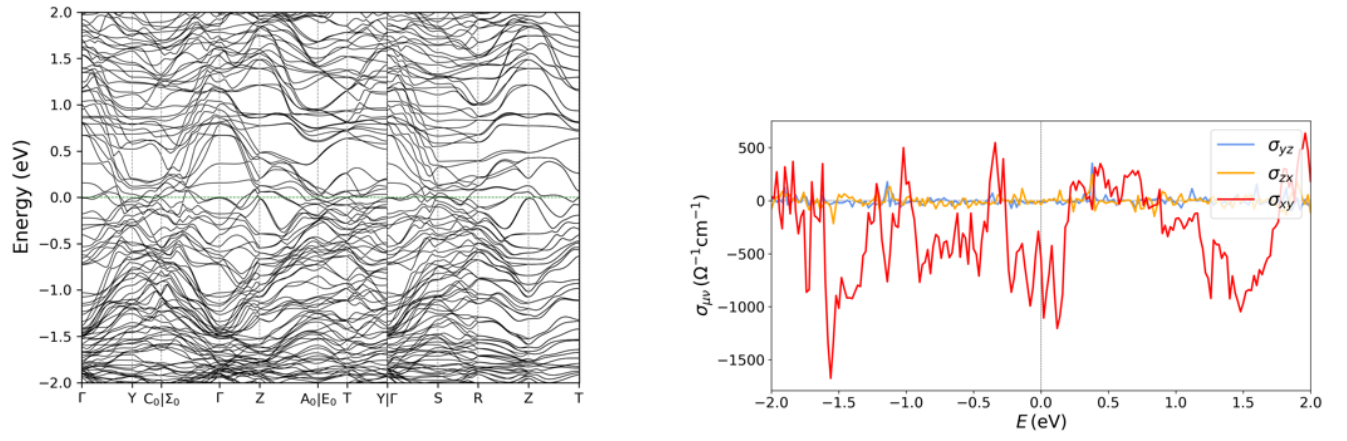

**0.184 Nd<sub>5</sub>Si<sub>4</sub>** crystallizes in type III MSG 92.114, which hosts only FNSs. The symmetry-adapted AHC tensor of the MSG is  $(0, 0, \sigma_{xy})$ . Based on the first-principles calculation results, the comparison between the experimental and calculated magnetic moments is provided in Table SII8. The band structure is shown in the left panel of Fig. 5, and the Fermi-level-dependent AHC is plotted in the right panel.

TABLE SII8. The comparison between the experimental and calculated magnetic moments for 0.184 Nd<sub>5</sub>Si<sub>4</sub>. The five columns contain the atom index in the structure file, the atom species, the fractional coordinates, the experimental magnetic moments, and the calculated magnetic moments. The lattice vectors are  $\vec{a}_1 = (7.876, 0.0, 0.0)$ ,  $\vec{a}_2 = (0.0, 7.876, 0.0)$ ,  $\vec{a}_3 = (0.0, 0.0, 14.801)$ .

| No. | Atom | Coordinates(fractional) |          |          | Experimental magnetic moments |           |          | Calculated magnetic moments |           |           |
|-----|------|-------------------------|----------|----------|-------------------------------|-----------|----------|-----------------------------|-----------|-----------|
| 1   | Nd   | 0.190100                | 0.190100 | 0.000000 | 0.360010                      | -0.360010 | 2.340040 | 0.453000                    | -0.472000 | 3.076000  |
| 2   | Nd   | 0.809900                | 0.809900 | 0.500000 | -0.360010                     | 0.360010  | 2.340040 | -0.456000                   | 0.471000  | 3.078000  |
| 3   | Nd   | 0.309900                | 0.690100 | 0.250000 | 0.360010                      | 0.360010  | 2.340040 | 0.467000                    | 0.453000  | 3.048000  |
| 4   | Nd   | 0.690100                | 0.309900 | 0.750000 | -0.360010                     | -0.360010 | 2.340040 | -0.468000                   | -0.451000 | 3.052000  |
| 5   | Nd   | 0.014200                | 0.132600 | 0.619200 | 0.330000                      | 0.430030  | 2.410050 | 0.347000                    | 0.374000  | 2.344000  |
| 6   | Nd   | 0.985800                | 0.867400 | 0.119200 | -0.330000                     | -0.430030 | 2.410050 | -0.343000                   | -0.370000 | 2.322000  |
| 7   | Nd   | 0.367400                | 0.514200 | 0.869200 | -0.430030                     | 0.330000  | 2.410050 | -0.372000                   | 0.348000  | 2.342000  |
| 8   | Nd   | 0.632600                | 0.485800 | 0.369200 | 0.430030                      | -0.330000 | 2.410050 | 0.369000                    | -0.341000 | 2.302000  |
| 9   | Nd   | 0.514200                | 0.367400 | 0.130800 | -0.330000                     | 0.430030  | 2.410050 | -0.391000                   | 0.512000  | 2.883000  |
| 10  | Nd   | 0.485800                | 0.632600 | 0.630800 | 0.330000                      | -0.430030 | 2.410050 | 0.390000                    | -0.511000 | 2.882000  |
| 11  | Nd   | 0.867400                | 0.985800 | 0.880800 | 0.430030                      | 0.330000  | 2.410050 | 0.517000                    | 0.390000  | 2.880000  |
| 12  | Nd   | 0.132600                | 0.014200 | 0.380800 | -0.430030                     | -0.330000 | 2.410050 | -0.516000                   | -0.389000 | 2.879000  |
| 13  | Nd   | 0.986100                | 0.366700 | 0.202500 | 1.380030                      | 0.579990  | 2.349950 | 1.664000                    | 0.711000  | 2.863000  |
| 14  | Nd   | 0.013900                | 0.633300 | 0.702500 | -1.380030                     | -0.579990 | 2.349950 | -1.662000                   | -0.711000 | 2.857000  |
| 15  | Nd   | 0.133300                | 0.486100 | 0.452500 | -0.579990                     | 1.380030  | 2.349950 | -0.708000                   | 1.663000  | 2.862000  |
| 16  | Nd   | 0.866700                | 0.513900 | 0.952500 | 0.579990                      | -1.380030 | 2.349950 | 0.709000                    | -1.664000 | 2.868000  |
| 17  | Nd   | 0.486100                | 0.133300 | 0.547500 | -1.380030                     | 0.579990  | 2.349950 | -1.614000                   | 0.685000  | 2.792000  |
| 18  | Nd   | 0.513900                | 0.866700 | 0.047500 | 1.380030                      | -0.579990 | 2.349950 | 1.611000                    | -0.686000 | 2.788000  |
| 19  | Nd   | 0.633300                | 0.013900 | 0.297500 | 0.579990                      | 1.380030  | 2.349950 | 0.680000                    | 1.610000  | 2.782000  |
| 20  | Nd   | 0.366700                | 0.986100 | 0.797500 | -0.579990                     | -1.380030 | 2.349950 | -0.679000                   | -1.609000 | 2.784000  |
| 21  | Si   | 0.052900                | 0.281000 | 0.807000 | 0.000000                      | 0.000000  | 0.000000 | 0.003000                    | 0.012000  | -0.038000 |
| 22  | Si   | 0.947100                | 0.719000 | 0.307000 | 0.000000                      | 0.000000  | 0.000000 | -0.003000                   | -0.011000 | -0.039000 |
| 23  | Si   | 0.219000                | 0.552900 | 0.057000 | 0.000000                      | 0.000000  | 0.000000 | -0.011000                   | 0.003000  | -0.038000 |
| 24  | Si   | 0.781000                | 0.447100 | 0.557000 | 0.000000                      | 0.000000  | 0.000000 | 0.011000                    | -0.003000 | -0.038000 |
| 25  | Si   | 0.552900                | 0.219000 | 0.943000 | 0.000000                      | 0.000000  | 0.000000 | -0.005000                   | 0.010000  | -0.039000 |
| 26  | Si   | 0.447100                | 0.781000 | 0.443000 | 0.000000                      | 0.000000  | 0.000000 | 0.004000                    | -0.010000 | -0.038000 |
| 27  | Si   | 0.719000                | 0.947100 | 0.693000 | 0.000000                      | 0.000000  | 0.000000 | 0.010000                    | 0.005000  | -0.040000 |
| 28  | Si   | 0.281000                | 0.052900 | 0.193000 | 0.000000                      | 0.000000  | 0.000000 | -0.009000                   | -0.005000 | -0.040000 |
| 29  | Si   | 0.282600                | 0.327000 | 0.692600 | 0.000000                      | 0.000000  | 0.000000 | 0.013000                    | 0.000000  | -0.034000 |
| 30  | Si   | 0.717400                | 0.673000 | 0.192600 | 0.000000                      | 0.000000  | 0.000000 | -0.013000                   | -0.001000 | -0.034000 |
| 31  | Si   | 0.173000                | 0.782600 | 0.942600 | 0.000000                      | 0.000000  | 0.000000 | -0.002000                   | 0.013000  | -0.033000 |
| 32  | Si   | 0.827000                | 0.217400 | 0.442600 | 0.000000                      | 0.000000  | 0.000000 | 0.002000                    | -0.012000 | -0.032000 |
| 33  | Si   | 0.782600                | 0.173000 | 0.057400 | 0.000000                      | 0.000000  | 0.000000 | -0.013000                   | -0.001000 | -0.035000 |
| 34  | Si   | 0.217400                | 0.827000 | 0.557400 | 0.000000                      | 0.000000  | 0.000000 | 0.013000                    | 0.001000  | -0.035000 |
| 35  | Si   | 0.673000                | 0.717400 | 0.807400 | 0.000000                      | 0.000000  | 0.000000 | -0.000000                   | 0.014000  | -0.036000 |
| 36  | Si   | 0.327000                | 0.282600 | 0.307400 | 0.000000                      | 0.000000  | 0.000000 | -0.001000                   | -0.013000 | -0.036000 |

FIG. 5. First-principles calculation results of  $0.184 \text{ Nd}_5\text{Si}_4$ . The band structure is shown in the left panel, and the Fermi-level-dependent AHC is plotted in the right panel. In both plots, the Fermi level is set to 0 eV.

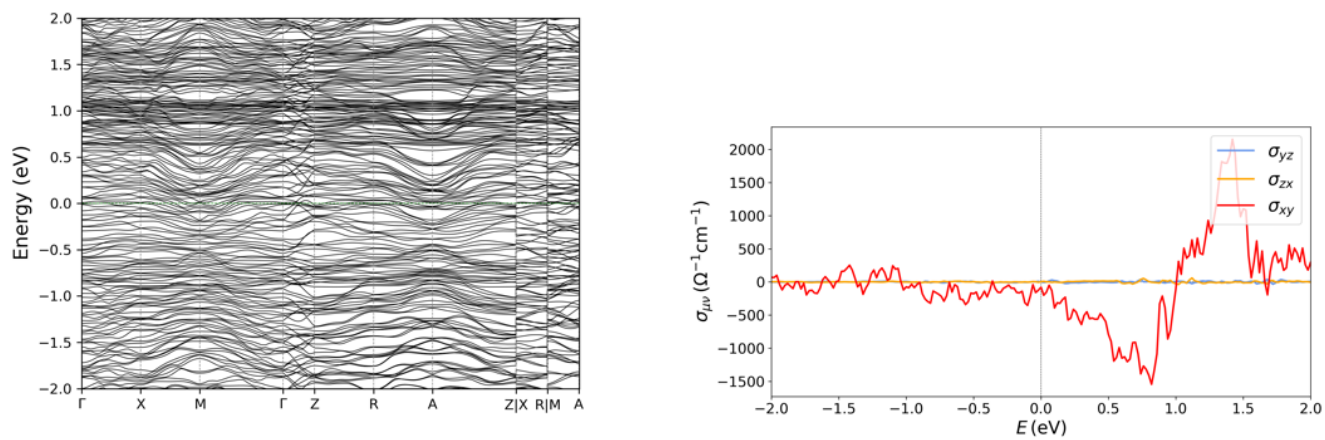



**0.199 Mn<sub>3</sub>Sn** crystallizes in type III MSG 63.463, which hosts only FNSs. The symmetry-adapted AHC tensor of the MSG is  $(\sigma_{yz}, 0, 0)$ . Based on the first-principles calculation results, the comparison between the experimental and calculated magnetic moments is provided in Table SII9. The band structure is shown in the left panel of Fig. 6, and the Fermi-level-dependent AHC is plotted in the right panel.

TABLE SII9. The comparison between the experimental and calculated magnetic moments for 0.199 Mn<sub>3</sub>Sn. The five columns contain the atom index in the structure file, the atom species, the fractional coordinates, the experimental magnetic moments, and the calculated magnetic moments. The lattice vectors are  $\vec{a}_1 = (2.8325, -4.906035, 0.0)$ ,  $\vec{a}_2 = (2.8325, 4.906035, 0.0)$ ,  $\vec{a}_3 = (0.0, 0.0, 4.531)$ .

| No. | Atom | Coordinates(fractional) |          |          | Experimental magnetic moments |           |          | Calculated magnetic moments |           |           |
|-----|------|-------------------------|----------|----------|-------------------------------|-----------|----------|-----------------------------|-----------|-----------|
| 1   | Mn   | 0.838800                | 0.677600 | 0.250000 | 1.499980                      | 2.598040  | 0.000000 | 2.120000                    | 3.679000  | -0.001000 |
| 2   | Mn   | 0.677600                | 0.838800 | 0.750000 | 1.499980                      | -2.598040 | 0.000000 | 2.128000                    | -3.679000 | 0.001000  |
| 3   | Mn   | 0.161200                | 0.322400 | 0.750000 | 1.499980                      | 2.598040  | 0.000000 | 2.119000                    | 3.680000  | 0.001000  |
| 4   | Mn   | 0.322400                | 0.161200 | 0.250000 | 1.499980                      | -2.598040 | 0.000000 | 2.130000                    | -3.678000 | -0.001000 |
| 5   | Mn   | 0.838800                | 0.161200 | 0.250000 | -3.000010                     | 0.000000  | 0.000000 | -4.249000                   | 0.009000  | -0.001000 |
| 6   | Mn   | 0.161200                | 0.838800 | 0.750000 | -3.000010                     | 0.000000  | 0.000000 | -4.248000                   | 0.009000  | 0.001000  |
| 7   | Sn   | 0.333333                | 0.666667 | 0.250000 | 0.000000                      | 0.000000  | 0.000000 | -0.000000                   | -0.009000 | -0.003000 |
| 8   | Sn   | 0.666667                | 0.333333 | 0.750000 | 0.000000                      | 0.000000  | 0.000000 | 0.000000                    | -0.009000 | 0.003000  |

FIG. 6. First-principles calculation results of 0.199 Mn<sub>3</sub>Sn. The band structure is shown in the left panel, and the Fermi-level-dependent AHC is plotted in the right panel. In both plots, the Fermi level is set to 0 eV.

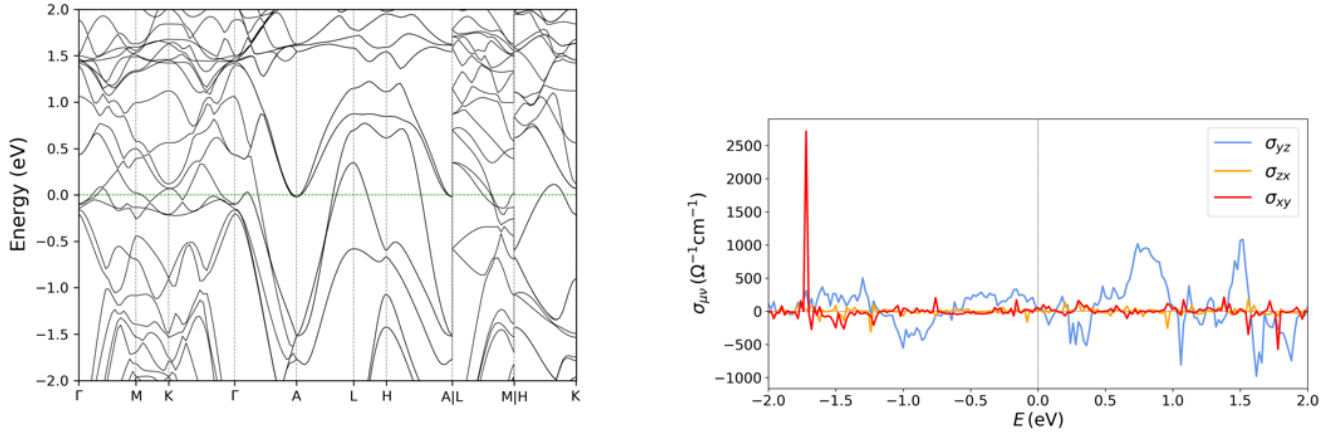

**0.200 Mn<sub>3</sub>Sn** crystallizes in type III MSG 63.464, which hosts only FNSs. The symmetry-adapted AHC tensor of the MSG is  $(0, \sigma_{zx}, 0)$ . Based on the first-principles calculation results, the comparison between the experimental and calculated magnetic moments is provided in Table SIII10. The band structure is shown in the left panel of Fig. 7, and the Fermi-level-dependent AHC is plotted in the right panel.

TABLE SIII10. The comparison between the experimental and calculated magnetic moments for 0.200 Mn<sub>3</sub>Sn. The five columns contain the atom index in the structure file, the atom species, the fractional coordinates, the experimental magnetic moments, and the calculated magnetic moments. The lattice vectors are  $\vec{a}_1 = (2.8325, -4.906035, 0.0)$ ,  $\vec{a}_2 = (2.8325, 4.906035, 0.0)$ ,  $\vec{a}_3 = (0.0, 0.0, 4.531)$ .

| No. | Atom | Coordinates(fractional) |          |          | Experimental magnetic moments |           |          | Calculated magnetic moments |           |           |
|-----|------|-------------------------|----------|----------|-------------------------------|-----------|----------|-----------------------------|-----------|-----------|
| 1   | Mn   | 0.677600                | 0.838800 | 0.250000 | 2.595020                      | 1.498010  | 0.000000 | 3.677000                    | 2.127000  | -0.007000 |
| 2   | Mn   | 0.161200                | 0.322400 | 0.250000 | -2.595020                     | 1.498010  | 0.000000 | -3.678000                   | 2.119000  | 0.007000  |
| 3   | Mn   | 0.322400                | 0.161200 | 0.750000 | 2.595020                      | 1.498010  | 0.000000 | 3.677000                    | 2.128000  | 0.007000  |
| 4   | Mn   | 0.838800                | 0.677600 | 0.750000 | -2.595020                     | 1.498010  | 0.000000 | -3.678000                   | 2.118000  | -0.007000 |
| 5   | Mn   | 0.161200                | 0.838800 | 0.250000 | 0.000000                      | -2.996020 | 0.000000 | -0.008000                   | -4.246000 | 0.000000  |
| 6   | Mn   | 0.838800                | 0.161200 | 0.750000 | 0.000000                      | -2.996020 | 0.000000 | -0.010000                   | -4.246000 | 0.000000  |
| 7   | Sn   | 0.666667                | 0.333333 | 0.250000 | 0.000000                      | 0.000000  | 0.000000 | 0.009000                    | -0.000000 | -0.001000 |
| 8   | Sn   | 0.333333                | 0.666667 | 0.750000 | 0.000000                      | 0.000000  | 0.000000 | 0.009000                    | 0.000000  | 0.000000  |

FIG. 7. First-principles calculation results of 0.200 Mn<sub>3</sub>Sn. The band structure is shown in the left panel, and the Fermi-level-dependent AHC is plotted in the right panel. In both plots, the Fermi level is set to 0 eV.

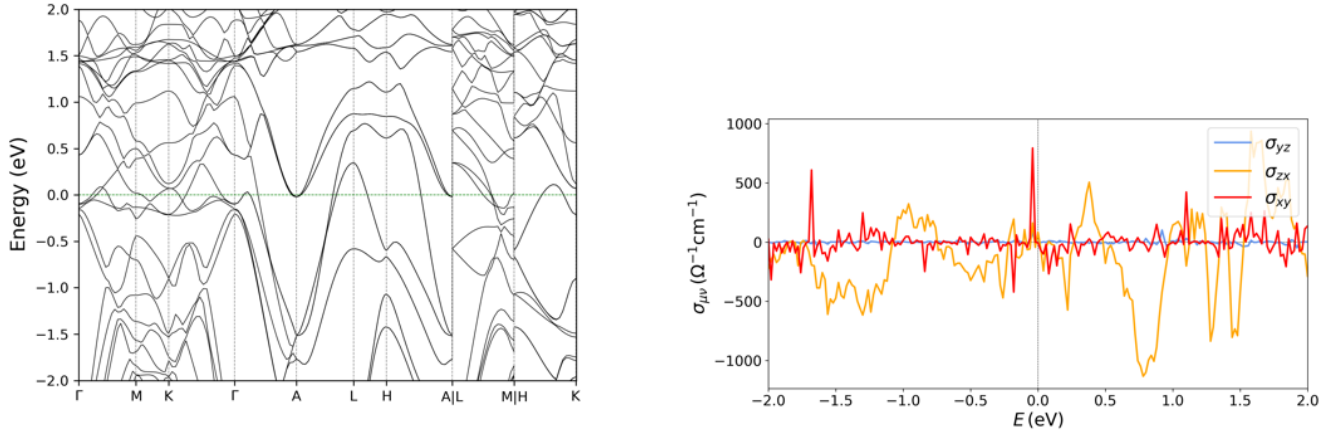

**0.226 NdCo<sub>2</sub>** crystallizes in type III MSG 15.89, which hosts only SNLs. The symmetry-adapted AHC tensor of the MSG is  $(\sigma_{yz}, \sigma_{zx}, 0)$ . Based on the first-principles calculation results, the comparison between the experimental and calculated magnetic moments is provided in Table SIII1. The band structure is shown in the left panel of Fig. 8, and the Fermi-level-dependent AHC is plotted in the right panel.

TABLE SIII1. The comparison between the experimental and calculated magnetic moments for 0.226 NdCo<sub>2</sub>. The five columns contain the atom index in the structure file, the atom species, the fractional coordinates, the experimental magnetic moments, and the calculated magnetic moments. The lattice vectors are  $\vec{a}_1 = (3.63875, -3.6487, 0.0)$ ,  $\vec{a}_2 = (3.63875, 3.6487, 0.0)$ ,  $\vec{a}_3 = (-3.638752823, 0.0, 3.641052547)$ .

| No. | Atom | Coordinates(fractional) |          |          | Experimental magnetic moments |          |          | Calculated magnetic moments |           |          |
|-----|------|-------------------------|----------|----------|-------------------------------|----------|----------|-----------------------------|-----------|----------|
| 1   | Nd   | 0.875000                | 0.125000 | 0.250000 | -1.979590                     | 0.000000 | 1.979820 | -2.418000                   | -0.019000 | 2.483000 |
| 2   | Nd   | 0.125000                | 0.875000 | 0.750000 | -1.979590                     | 0.000000 | 1.979820 | -2.408000                   | -0.018000 | 2.475000 |
| 3   | Co   | 0.500000                | 0.500000 | 0.000000 | -0.519540                     | 0.000000 | 0.519870 | -0.944000                   | -0.026000 | 0.923000 |
| 4   | Co   | 0.500000                | 0.500000 | 0.500000 | -0.519540                     | 0.000000 | 0.519870 | -0.958000                   | -0.016000 | 0.934000 |
| 5   | Co   | 0.000000                | 0.500000 | 0.000000 | -0.519540                     | 0.000000 | 0.519870 | -0.960000                   | -0.014000 | 0.935000 |
| 6   | Co   | 0.500000                | 0.000000 | 0.500000 | -0.519540                     | 0.000000 | 0.519870 | -0.961000                   | -0.018000 | 0.942000 |

FIG. 8. First-principles calculation results of 0.226 NdCo<sub>2</sub>. The band structure is shown in the left panel, and the Fermi-level-dependent AHC is plotted in the right panel. In both plots, the Fermi level is set to 0 eV.

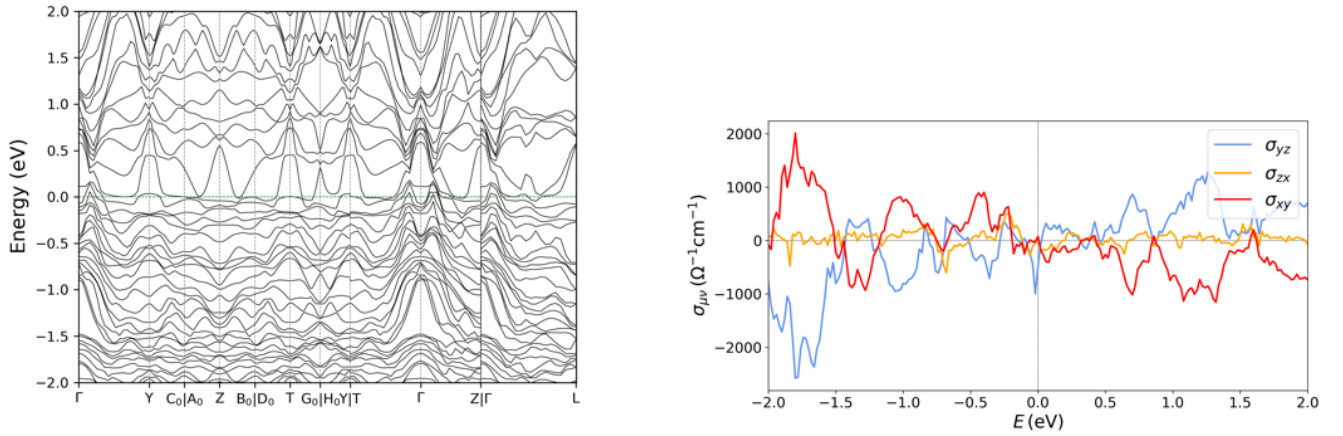

**0.227 NdCo<sub>2</sub>** crystallizes in type III MSG 141.557, which hosts only SNLs. The symmetry-adapted AHC tensor of the MSG is  $(0, 0, \sigma_{xy})$ . Based on the first-principles calculation results, the comparison between the experimental and calculated magnetic moments is provided in Table SIII2. The band structure is shown in the left panel of Fig. 9, and the Fermi-level-dependent AHC is plotted in the right panel.

TABLE SIII2. The comparison between the experimental and calculated magnetic moments for 0.227 NdCo<sub>2</sub>. The five columns contain the atom index in the structure file, the atom species, the fractional coordinates, the experimental magnetic moments, and the calculated magnetic moments. The lattice vectors are  $\vec{a}_1 = (-2.5783, 2.5783, 3.6354)$ ,  $\vec{a}_2 = (2.5783, -2.5783, 3.6354)$ ,  $\vec{a}_3 = (2.5783, 2.5783, -3.6354)$ .

| No. | Atom | Coordinates(fractional) |          |          | Experimental magnetic moments |          | Calculated magnetic moments |           |           |          |
|-----|------|-------------------------|----------|----------|-------------------------------|----------|-----------------------------|-----------|-----------|----------|
| 1   | Nd   | 0.625000                | 0.375000 | 0.250000 | 0.000000                      | 0.000000 | 2.429970                    | 0.003000  | 0.003000  | 2.079000 |
| 2   | Nd   | 0.375000                | 0.625000 | 0.750000 | 0.000000                      | 0.000000 | 2.429970                    | -0.003000 | -0.004000 | 1.940000 |
| 3   | Co   | 0.000000                | 0.000000 | 0.000000 | 0.000000                      | 0.000000 | 0.590030                    | -0.005000 | 0.011000  | 0.755000 |
| 4   | Co   | 0.500000                | 0.000000 | 0.500000 | 0.000000                      | 0.000000 | 0.590030                    | 0.004000  | -0.010000 | 0.746000 |
| 5   | Co   | 0.000000                | 0.500000 | 0.000000 | 0.000000                      | 0.000000 | 0.590030                    | -0.010000 | -0.004000 | 0.745000 |
| 6   | Co   | 0.000000                | 0.000000 | 0.500000 | 0.000000                      | 0.000000 | 0.590030                    | 0.011000  | 0.003000  | 0.754000 |

FIG. 9. First-principles calculation results of 0.227 NdCo<sub>2</sub>. The band structure is shown in the left panel, and the Fermi-level-dependent AHC is plotted in the right panel. In both plots, the Fermi level is set to 0 eV.

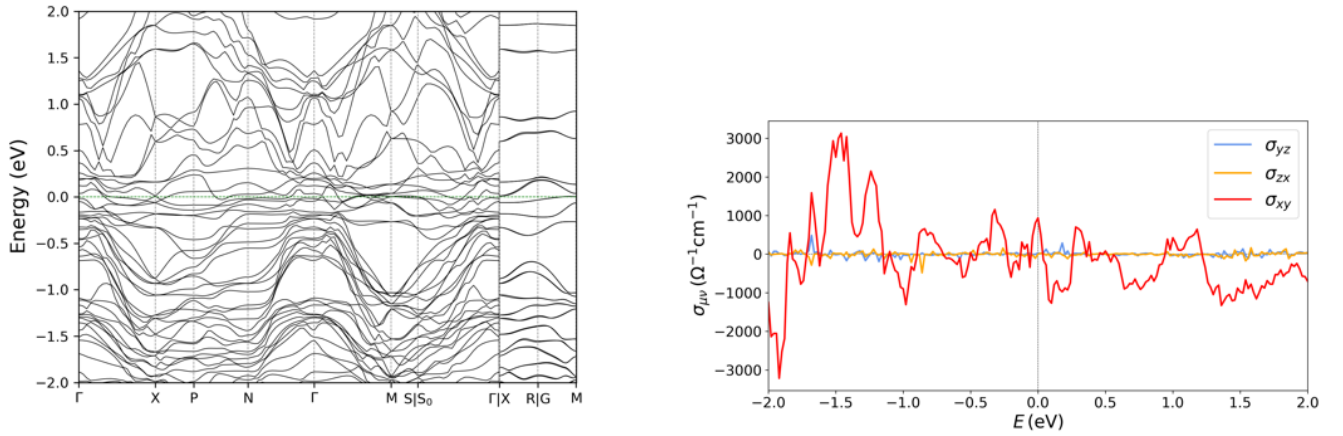

**0.395 MnPtGa** crystallizes in type III MSG 63.462, which hosts only SNLs. The symmetry-adapted AHC tensor of the MSG is  $(0, 0, \sigma_{xy})$ . Based on the first-principles calculation results, the comparison between the experimental and calculated magnetic moments is provided in Table SIII13. The band structure is shown in the left panel of Fig. 10, and the Fermi-level-dependent AHC is plotted in the right panel.

TABLE SIII13. The comparison between the experimental and calculated magnetic moments for 0.395 MnPtGa. The five columns contain the atom index in the structure file, the atom species, the fractional coordinates, the experimental magnetic moments, and the calculated magnetic moments. The lattice vectors are  $\vec{a}_1 = (2.1654, -3.75055, 0.0)$ ,  $\vec{a}_2 = (2.1654, 3.75055, 0.0)$ ,  $\vec{a}_3 = (0.0, 0.0, 5.561)$ .

| No. | Atom | Coordinates(fractional) |          |          | Experimental magnetic moments |          |          | Calculated magnetic moments |           |           |
|-----|------|-------------------------|----------|----------|-------------------------------|----------|----------|-----------------------------|-----------|-----------|
| 1   | Ga   | 0.333333                | 0.666667 | 0.250000 | 0.000000                      | 0.000000 | 0.000000 | 0.000000                    | 0.000000  | -0.076000 |
| 2   | Ga   | 0.666667                | 0.333333 | 0.750000 | 0.000000                      | 0.000000 | 0.000000 | 0.000000                    | 0.000000  | -0.066000 |
| 3   | Mn   | 0.000000                | 0.000000 | 0.000000 | 0.000000                      | 0.000000 | 3.099980 | -0.000000                   | -0.000000 | 3.643000  |
| 4   | Mn   | 0.000000                | 0.000000 | 0.500000 | 0.000000                      | 0.000000 | 3.099980 | -0.000000                   | -0.000000 | 3.648000  |
| 5   | Pt   | 0.666667                | 0.333333 | 0.250000 | 0.000000                      | 0.000000 | 0.000000 | -0.000000                   | 0.000000  | 0.065000  |
| 6   | Pt   | 0.333333                | 0.666667 | 0.750000 | 0.000000                      | 0.000000 | 0.000000 | -0.000000                   | 0.000000  | 0.081000  |

FIG. 10. First-principles calculation results of 0.395 MnPtGa. The band structure is shown in the left panel, and the Fermi-level-dependent AHC is plotted in the right panel. In both plots, the Fermi level is set to 0 eV.

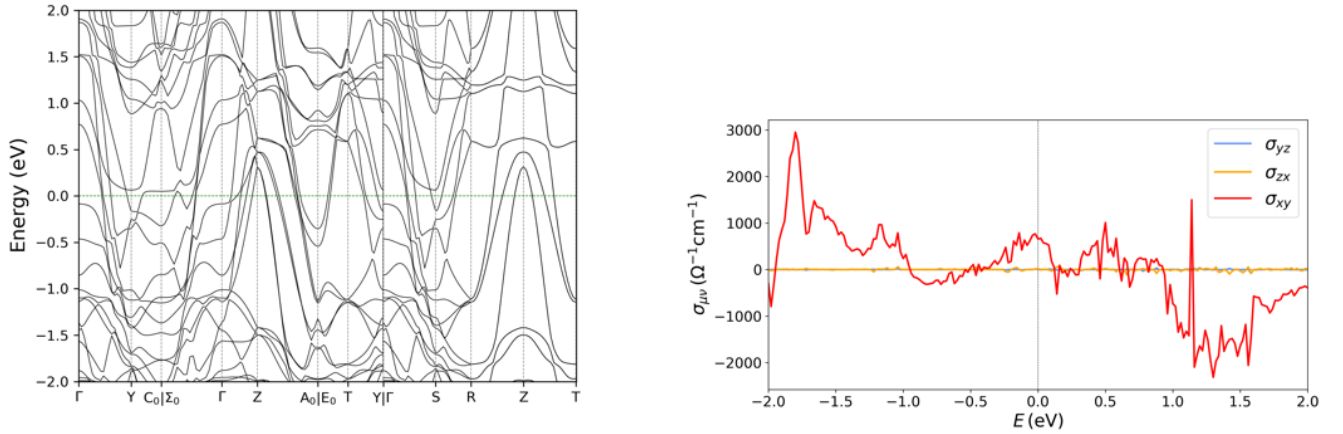

**0.403 NdCo<sub>2</sub>** crystallizes in type III MSG 74.559, which hosts only SNLs. The symmetry-adapted AHC tensor of the MSG is  $(\sigma_{yz}, 0, 0)$ . Based on the first-principles calculation results, the comparison between the experimental and calculated magnetic moments is provided in Table SIII14. The band structure is shown in the left panel of Fig. 11, and the Fermi-level-dependent AHC is plotted in the right panel.

TABLE SIII14. The comparison between the experimental and calculated magnetic moments for 0.403 NdCo<sub>2</sub>. The five columns contain the atom index in the structure file, the atom species, the fractional coordinates, the experimental magnetic moments, and the calculated magnetic moments. The lattice vectors are  $\vec{a}_1 = (-2.57155, 2.5756, 3.64865)$ ,  $\vec{a}_2 = (2.57155, -2.5756, 3.64865)$ ,  $\vec{a}_3 = (2.57155, 2.5756, -3.64865)$ .

| No. | Atom | Coordinates(fractional) |          |          | Experimental magnetic moments |          |          | Calculated magnetic moments |           |           |
|-----|------|-------------------------|----------|----------|-------------------------------|----------|----------|-----------------------------|-----------|-----------|
| 1   | Nd   | 0.625600                | 0.375600 | 0.250000 | 2.380020                      | 0.000000 | 0.000000 | 2.462000                    | 0.003000  | 0.002000  |
| 2   | Nd   | 0.374400                | 0.624400 | 0.750000 | 2.380020                      | 0.000000 | 0.000000 | 2.466000                    | -0.002000 | -0.002000 |
| 3   | Co   | 0.000000                | 0.000000 | 0.500000 | 0.649980                      | 0.000000 | 0.000000 | 1.120000                    | 0.002000  | 0.007000  |
| 4   | Co   | 0.000000                | 0.500000 | 0.000000 | 0.649980                      | 0.000000 | 0.000000 | 1.116000                    | -0.002000 | -0.007000 |
| 5   | Co   | 0.000000                | 0.000000 | 0.000000 | 0.629980                      | 0.000000 | 0.000000 | 1.081000                    | -0.000000 | 0.000000  |
| 6   | Co   | 0.500000                | 0.000000 | 0.500000 | 0.629980                      | 0.000000 | 0.000000 | 1.072000                    | -0.001000 | -0.000000 |

FIG. 11. First-principles calculation results of 0.403 NdCo<sub>2</sub>. The band structure is shown in the left panel, and the Fermi-level-dependent AHC is plotted in the right panel. In both plots, the Fermi level is set to 0 eV.

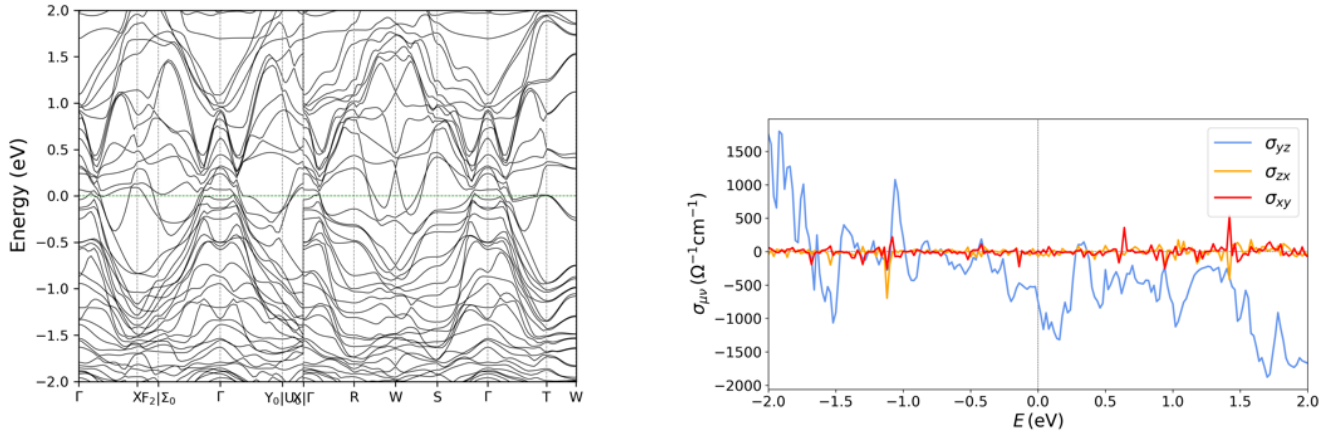

**0.407 NdSi** crystallizes in type III MSG 62.446, which hosts both SNLs and FNSs. The symmetry-adapted AHC tensor of the MSG is  $(0, 0, \sigma_{xy})$ . Based on the first-principles calculation results, the comparison between the experimental and calculated magnetic moments is provided in Table SIII15. The band structure is shown in the left panel of Fig. 12, and the Fermi-level-dependent AHC is plotted in the right panel.

TABLE SIII15. The comparison between the experimental and calculated magnetic moments for 0.407 NdSi. The five columns contain the atom index in the structure file, the atom species, the fractional coordinates, the experimental magnetic moments, and the calculated magnetic moments. The lattice vectors are  $\vec{a}_1 = (8.158, 0.0, 0.0)$ ,  $\vec{a}_2 = (0.0, 3.918, 0.0)$ ,  $\vec{a}_3 = (0.0, 0.0, 5.887)$ .

| No. | Atom | Coordinates(fractional) |          |          | Experimental magnetic moments |          |          | Calculated magnetic moments |           |           |
|-----|------|-------------------------|----------|----------|-------------------------------|----------|----------|-----------------------------|-----------|-----------|
| 1   | Nd   | 0.324000                | 0.250000 | 0.620000 | -0.890040                     | 0.000000 | 2.439980 | -1.061000                   | 0.002000  | 2.928000  |
| 2   | Nd   | 0.176000                | 0.750000 | 0.120000 | 0.890040                      | 0.000000 | 2.439980 | 1.054000                    | -0.002000 | 2.929000  |
| 3   | Nd   | 0.676000                | 0.750000 | 0.380000 | -0.890040                     | 0.000000 | 2.439980 | -1.054000                   | -0.002000 | 2.930000  |
| 4   | Nd   | 0.824000                | 0.250000 | 0.880000 | 0.890040                      | 0.000000 | 2.439980 | 1.061000                    | 0.002000  | 2.928000  |
| 5   | Si   | 0.470000                | 0.250000 | 0.110000 | 0.000000                      | 0.000000 | 0.000000 | 0.002000                    | -0.000000 | -0.027000 |
| 6   | Si   | 0.030000                | 0.750000 | 0.610000 | 0.000000                      | 0.000000 | 0.000000 | -0.001000                   | -0.000000 | -0.027000 |
| 7   | Si   | 0.530000                | 0.750000 | 0.890000 | 0.000000                      | 0.000000 | 0.000000 | 0.001000                    | -0.000000 | -0.028000 |
| 8   | Si   | 0.970000                | 0.250000 | 0.390000 | 0.000000                      | 0.000000 | 0.000000 | -0.002000                   | 0.000000  | -0.026000 |

FIG. 12. First-principles calculation results of 0.407 NdSi. The band structure is shown in the left panel, and the Fermi-level-dependent AHC is plotted in the right panel. In both plots, the Fermi level is set to 0 eV.

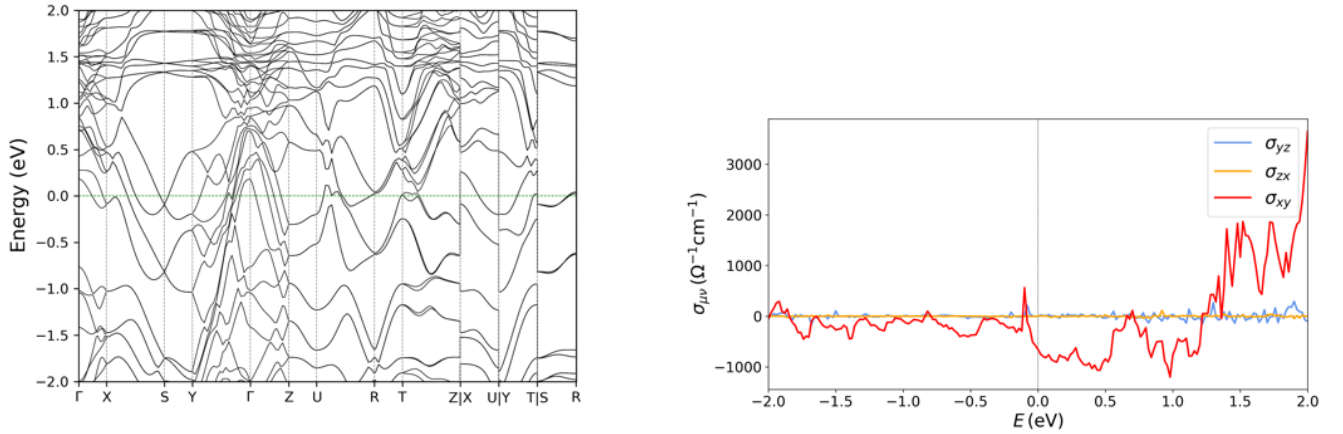



**0.408 PrSi** crystallizes in type III MSG 62.447, which hosts both SNLs and FNSs. The symmetry-adapted AHC tensor of the MSG is  $(\sigma_{yz}, 0, 0)$ . Based on the first-principles calculation results, the comparison between the experimental and calculated magnetic moments is provided in Table SIII16. The band structure is shown in the left panel of Fig. 13, and the Fermi-level-dependent AHC is plotted in the right panel.

TABLE SIII16. The comparison between the experimental and calculated magnetic moments for 0.408 PrSi. The five columns contain the atom index in the structure file, the atom species, the fractional coordinates, the experimental magnetic moments, and the calculated magnetic moments. The lattice vectors are  $\vec{a}_1 = (8.243, 0.0, 0.0)$ ,  $\vec{a}_2 = (0.0, 3.941, 0.0)$ ,  $\vec{a}_3 = (0.0, 0.0, 5.918)$ .

| No. | Atom | Coordinates(fractional) |          |          | Experimental magnetic moments |          | Calculated magnetic moments |           |           |           |
|-----|------|-------------------------|----------|----------|-------------------------------|----------|-----------------------------|-----------|-----------|-----------|
| 1   | Pr   | 0.680000                | 0.250000 | 0.118000 | 2.790010                      | 0.000000 | 0.269980                    | 2.640000  | -0.001000 | 0.251000  |
| 2   | Pr   | 0.180000                | 0.250000 | 0.382000 | 2.790010                      | 0.000000 | -0.269980                   | 2.648000  | -0.001000 | -0.251000 |
| 3   | Pr   | 0.320000                | 0.750000 | 0.882000 | 2.790010                      | 0.000000 | 0.269980                    | 2.639000  | 0.001000  | 0.251000  |
| 4   | Pr   | 0.820000                | 0.750000 | 0.618000 | 2.790010                      | 0.000000 | -0.269980                   | 2.649000  | 0.001000  | -0.252000 |
| 5   | Si   | 0.529000                | 0.250000 | 0.611000 | 0.000000                      | 0.000000 | 0.000000                    | -0.119000 | 0.000000  | -0.002000 |
| 6   | Si   | 0.029000                | 0.250000 | 0.889000 | 0.000000                      | 0.000000 | 0.000000                    | -0.121000 | 0.000000  | 0.002000  |
| 7   | Si   | 0.471000                | 0.750000 | 0.389000 | 0.000000                      | 0.000000 | 0.000000                    | -0.119000 | -0.000000 | -0.002000 |
| 8   | Si   | 0.971000                | 0.750000 | 0.111000 | 0.000000                      | 0.000000 | 0.000000                    | -0.121000 | -0.000000 | 0.002000  |

FIG. 13. First-principles calculation results of 0.408 PrSi. The band structure is shown in the left panel, and the Fermi-level-dependent AHC is plotted in the right panel. In both plots, the Fermi level is set to 0 eV.

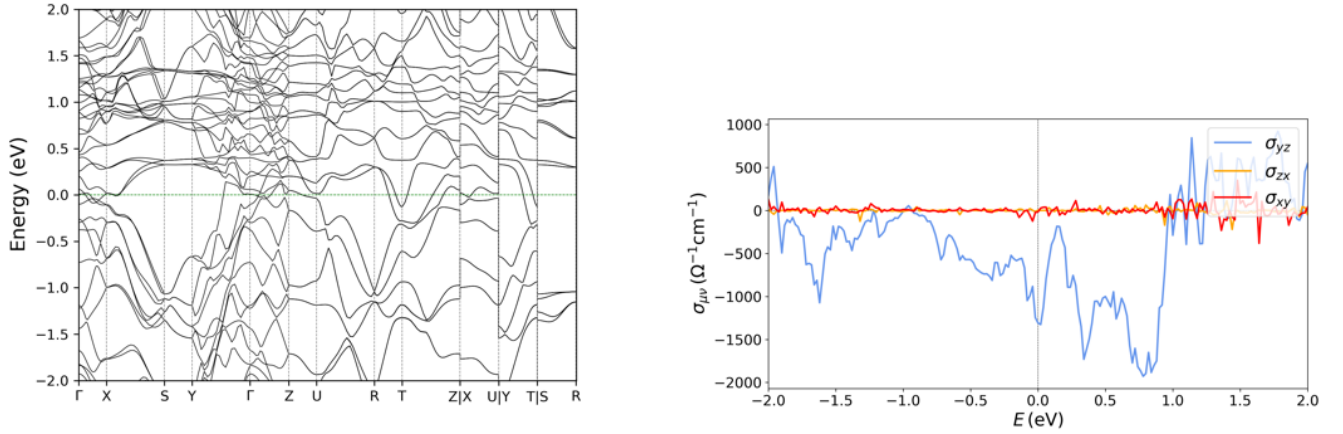



**0.449 Tb<sub>2</sub>Pt** crystallizes in type III MSG 11.54, which hosts only FNSs. The symmetry-adapted AHC tensor of the MSG is  $(\sigma_{yz}, \sigma_{zx}, 0)$ . Based on the first-principles calculation results, the comparison between the experimental and calculated magnetic moments is provided in Table SIII17. The band structure is shown in the left panel of Fig. 14, and the Fermi-level-dependent AHC is plotted in the right panel.

TABLE SIII17. The comparison between the experimental and calculated magnetic moments for 0.449 Tb<sub>2</sub>Pt. The five columns contain the atom index in the structure file, the atom species, the fractional coordinates, the experimental magnetic moments, and the calculated magnetic moments. The lattice vectors are  $\vec{a}_1 = (7.147, 0.0, 0.0)$ ,  $\vec{a}_2 = (0.0, 4.772, 0.0)$ ,  $\vec{a}_3 = (0.0, 0.0, 8.763)$ .

| No. | Atom | Coordinates(fractional) |          |          | Experimental magnetic moments |          |           | Calculated magnetic moments |           |           |
|-----|------|-------------------------|----------|----------|-------------------------------|----------|-----------|-----------------------------|-----------|-----------|
| 1   | Pt   | 0.726000                | 0.250000 | 0.896000 | 0.000000                      | 0.000000 | 0.000000  | -0.043000                   | -0.000000 | -0.044000 |
| 2   | Pt   | 0.274000                | 0.750000 | 0.104000 | 0.000000                      | 0.000000 | 0.000000  | -0.048000                   | 0.000000  | -0.037000 |
| 3   | Pt   | 0.226000                | 0.250000 | 0.604000 | 0.000000                      | 0.000000 | 0.000000  | -0.041000                   | -0.001000 | -0.025000 |
| 4   | Pt   | 0.774000                | 0.750000 | 0.396000 | 0.000000                      | 0.000000 | 0.000000  | -0.038000                   | 0.001000  | -0.019000 |
| 5   | Tb   | 0.132000                | 0.250000 | 0.927000 | 5.200010                      | 0.000000 | 1.999980  | 6.272000                    | -0.001000 | 2.479000  |
| 6   | Tb   | 0.868000                | 0.750000 | 0.073000 | 5.200010                      | 0.000000 | 1.999980  | 6.270000                    | 0.003000  | 2.479000  |
| 7   | Tb   | 0.632000                | 0.250000 | 0.573000 | 5.200010                      | 0.000000 | -1.999980 | 6.071000                    | -0.003000 | -2.243000 |
| 8   | Tb   | 0.368000                | 0.750000 | 0.427000 | 5.200010                      | 0.000000 | -1.999980 | 6.071000                    | 0.007000  | -2.243000 |
| 9   | Tb   | 0.032000                | 0.250000 | 0.227000 | 3.000020                      | 0.000000 | 4.700040  | 3.653000                    | -0.003000 | 5.619000  |
| 10  | Tb   | 0.968000                | 0.750000 | 0.773000 | 3.000020                      | 0.000000 | 4.700040  | 3.656000                    | 0.002000  | 5.618000  |
| 11  | Tb   | 0.532000                | 0.250000 | 0.273000 | -3.000020                     | 0.000000 | 4.700040  | -3.409000                   | 0.001000  | 5.489000  |
| 12  | Tb   | 0.468000                | 0.750000 | 0.727000 | -3.000020                     | 0.000000 | 4.700040  | -3.407000                   | 0.000000  | 5.486000  |

FIG. 14. First-principles calculation results of 0.449 Tb<sub>2</sub>Pt. The band structure is shown in the left panel, and the Fermi-level-dependent AHC is plotted in the right panel. In both plots, the Fermi level is set to 0 eV.

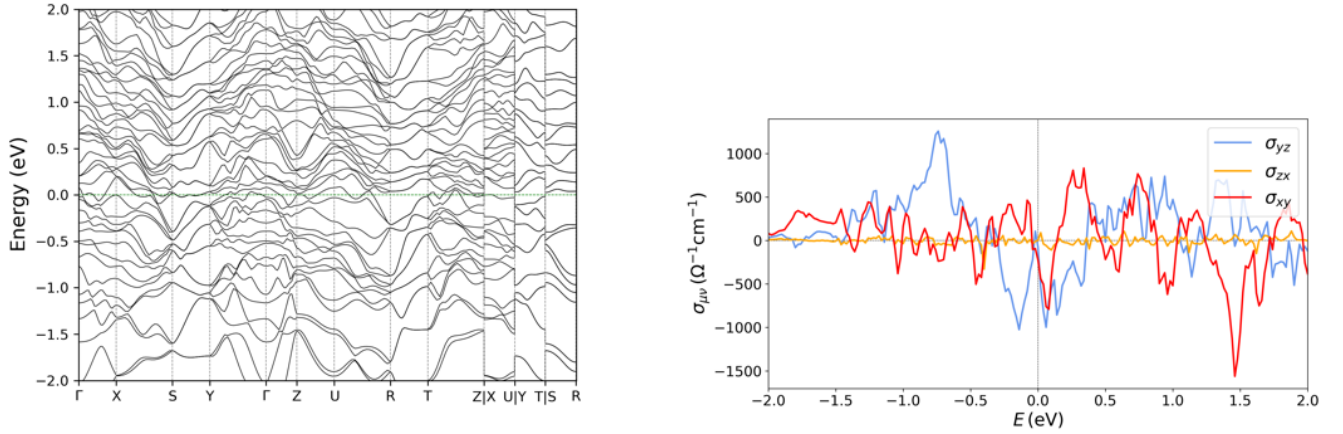

**0.480 HoNi** crystallizes in type III MSG 62.447, which hosts both SNLs and FNSs. The symmetry-adapted AHC tensor of the MSG is  $(\sigma_{yz}, 0, 0)$ . Based on the first-principles calculation results, the comparison between the experimental and calculated magnetic moments is provided in Table SIII18. The band structure is shown in the left panel of Fig. 15, and the Fermi-level-dependent AHC is plotted in the right panel.

TABLE SIII18. The comparison between the experimental and calculated magnetic moments for 0.480 HoNi. The five columns contain the atom index in the structure file, the atom species, the fractional coordinates, the experimental magnetic moments, and the calculated magnetic moments. The lattice vectors are  $\vec{a}_1 = (6.9764, 0.0, 0.0)$ ,  $\vec{a}_2 = (0.0, 4.15478, 0.0)$ ,  $\vec{a}_3 = (0.0, 0.0, 5.4016)$ .

| No. | Atom | Coordinates(fractional) |          |          | Experimental magnetic moments |          | Calculated magnetic moments |          |           |           |
|-----|------|-------------------------|----------|----------|-------------------------------|----------|-----------------------------|----------|-----------|-----------|
| 1   | Ho   | 0.681400                | 0.250000 | 0.133200 | 6.980030                      | 0.000000 | -3.389990                   | 2.524000 | -0.009000 | -1.198000 |
| 2   | Ho   | 0.181400                | 0.250000 | 0.366800 | 6.980030                      | 0.000000 | 3.389990                    | 2.530000 | 0.009000  | 1.203000  |
| 3   | Ho   | 0.318600                | 0.750000 | 0.866800 | 6.980030                      | 0.000000 | -3.389990                   | 2.527000 | -0.011000 | -1.200000 |
| 4   | Ho   | 0.818600                | 0.750000 | 0.633200 | 6.980030                      | 0.000000 | 3.389990                    | 2.526000 | 0.010000  | 1.201000  |
| 5   | Ni   | 0.536200                | 0.250000 | 0.626900 | 0.000000                      | 0.000000 | 0.000000                    | 0.746000 | 0.009000  | -1.038000 |
| 6   | Ni   | 0.036200                | 0.250000 | 0.873100 | 0.000000                      | 0.000000 | 0.000000                    | 0.756000 | -0.000000 | 1.037000  |
| 7   | Ni   | 0.463800                | 0.750000 | 0.373100 | 0.000000                      | 0.000000 | 0.000000                    | 0.750000 | -0.011000 | -1.035000 |
| 8   | Ni   | 0.963800                | 0.750000 | 0.126900 | 0.000000                      | 0.000000 | 0.000000                    | 0.752000 | 0.002000  | 1.041000  |

FIG. 15. First-principles calculation results of 0.480 HoNi. The band structure is shown in the left panel, and the Fermi-level-dependent AHC is plotted in the right panel. In both plots, the Fermi level is set to 0 eV.

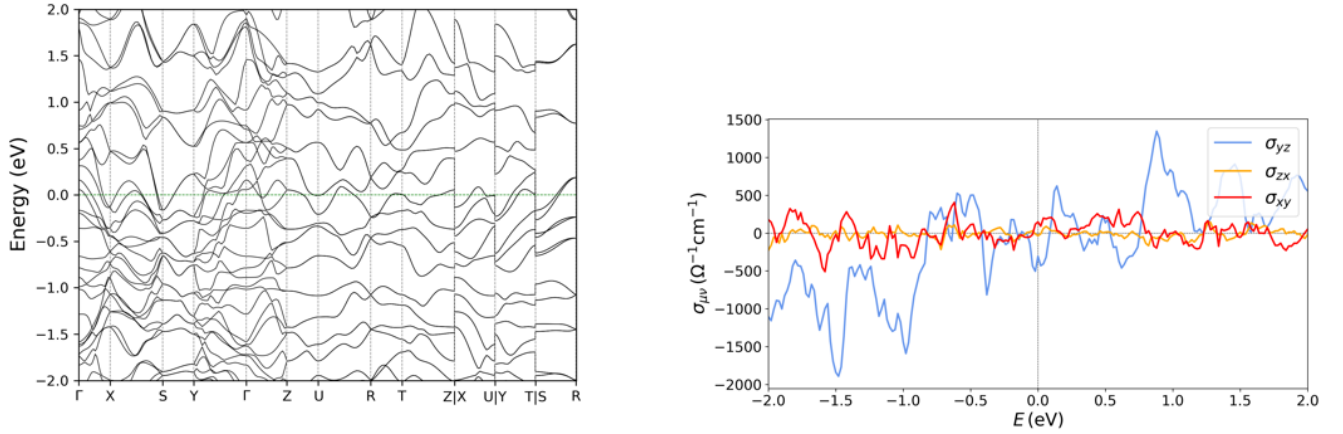

**0.481 HoNi** crystallizes in type III MSG 14.79, which hosts both SNLs and FNSs. The symmetry-adapted AHC tensor of the MSG is  $(\sigma_{yz}, \sigma_{zx}, 0)$ . Based on the first-principles calculation results, the comparison between the experimental and calculated magnetic moments is provided in Table ???. The band structure is shown in the left panel of Fig. 16, and the Fermi-level-dependent AHC is plotted in the right panel.

FIG. 16. First-principles calculation results of 0.481 HoNi. The band structure is shown in the left panel, and the Fermi-level-dependent AHC is plotted in the right panel. In both plots, the Fermi level is set to 0 eV.

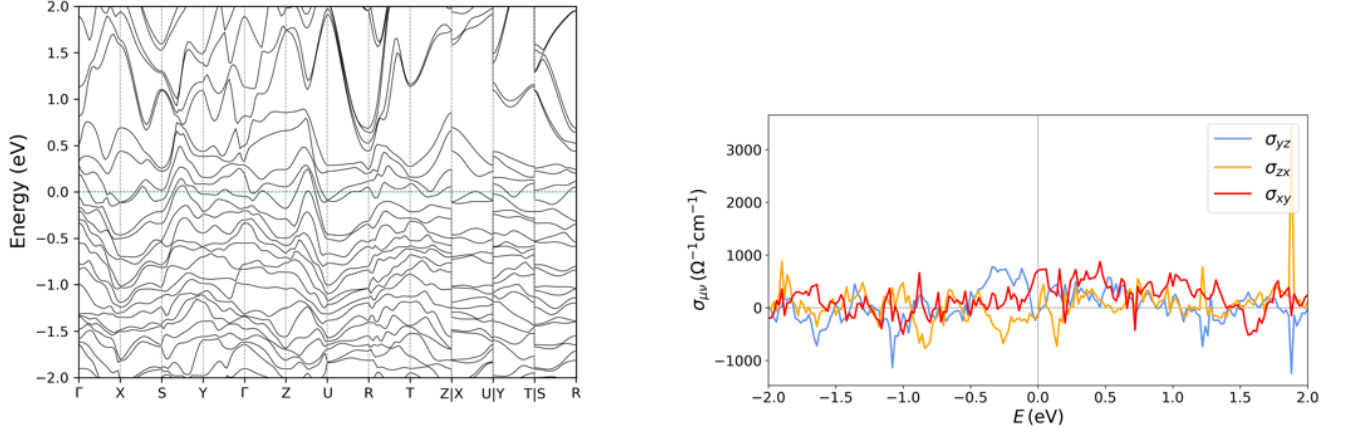

**0.51 Ho<sub>2</sub>Ru<sub>2</sub>O<sub>7</sub>** crystallizes in type III MSG 141.557, which hosts only SNLs. The symmetry-adapted AHC tensor of the MSG is  $(0, 0, \sigma_{xy})$ . Based on the first-principles calculation results, the comparison between the experimental and calculated magnetic moments is provided in Table SIII19. The band structure is shown in the left panel of Fig. 17, and the Fermi-level-dependent AHC is plotted in the right panel.

TABLE SIII19. The comparison between the experimental and calculated magnetic moments for 0.51 Ho<sub>2</sub>Ru<sub>2</sub>O<sub>7</sub>. The five columns contain the atom index in the structure file, the atom species, the fractional coordinates, the experimental magnetic moments, and the calculated magnetic moments. The lattice vectors are  $\vec{a}_1 = (-3.58563, 3.58563, 5.07085)$ ,  $\vec{a}_2 = (3.58563, -3.58563, 5.07085)$ ,  $\vec{a}_3 = (3.58563, 3.58563, -5.07085)$ .

| No. | Atom | Coordinates(fractional) |          |          | Experimental magnetic moments |           |           | Calculated magnetic moments |           |           |
|-----|------|-------------------------|----------|----------|-------------------------------|-----------|-----------|-----------------------------|-----------|-----------|
| 1   | O    | 0.911000                | 0.661000 | 0.822000 | 0.000000                      | 0.000000  | 0.000000  | 0.094000                    | -0.094000 | -0.048000 |
| 2   | O    | 0.339000                | 0.089000 | 0.678000 | 0.000000                      | 0.000000  | 0.000000  | -0.093000                   | 0.095000  | -0.048000 |
| 3   | O    | 0.661000                | 0.339000 | 0.750000 | 0.000000                      | 0.000000  | 0.000000  | 0.093000                    | 0.092000  | -0.045000 |
| 4   | O    | 0.089000                | 0.911000 | 0.750000 | 0.000000                      | 0.000000  | 0.000000  | -0.091000                   | -0.091000 | -0.047000 |
| 5   | O    | 0.089000                | 0.339000 | 0.178000 | 0.000000                      | 0.000000  | 0.000000  | 0.090000                    | -0.091000 | -0.046000 |
| 6   | O    | 0.661000                | 0.911000 | 0.322000 | 0.000000                      | 0.000000  | 0.000000  | -0.090000                   | 0.091000  | -0.046000 |
| 7   | O    | 0.339000                | 0.661000 | 0.250000 | 0.000000                      | 0.000000  | 0.000000  | 0.092000                    | 0.092000  | -0.049000 |
| 8   | O    | 0.911000                | 0.089000 | 0.250000 | 0.000000                      | 0.000000  | 0.000000  | -0.094000                   | -0.093000 | -0.047000 |
| 9   | O    | 0.911000                | 0.661000 | 0.250000 | 0.000000                      | 0.000000  | 0.000000  | -0.002000                   | -0.001000 | -0.018000 |
| 10  | O    | 0.661000                | 0.911000 | 0.750000 | 0.000000                      | 0.000000  | 0.000000  | 0.001000                    | 0.003000  | -0.017000 |
| 11  | O    | 0.089000                | 0.339000 | 0.750000 | 0.000000                      | 0.000000  | 0.000000  | 0.002000                    | 0.001000  | -0.017000 |
| 12  | O    | 0.339000                | 0.089000 | 0.250000 | 0.000000                      | 0.000000  | 0.000000  | -0.000000                   | -0.003000 | -0.018000 |
| 13  | O    | 0.625000                | 0.375000 | 0.250000 | 0.000000                      | 0.000000  | 0.000000  | -0.000000                   | -0.001000 | -0.162000 |
| 14  | O    | 0.375000                | 0.625000 | 0.750000 | 0.000000                      | 0.000000  | 0.000000  | 0.001000                    | 0.001000  | -0.165000 |
| 15  | Ho   | 0.500000                | 0.500000 | 0.000000 | 0.000000                      | -6.025010 | 1.840010  | -0.001000                   | -7.106000 | 2.141000  |
| 16  | Ho   | 0.000000                | 0.500000 | 0.500000 | 0.000000                      | 6.025010  | 1.840010  | 0.002000                    | 7.104000  | 2.141000  |
| 17  | Ho   | 0.500000                | 0.000000 | 0.000000 | 0.000000                      | 6.025010  | 1.840010  | 7.106000                    | -0.002000 | 2.142000  |
| 18  | Ho   | 0.500000                | 0.500000 | 0.500000 | -6.025010                     | 0.000000  | 1.840010  | -7.104000                   | 0.001000  | 2.141000  |
| 19  | Ru   | 0.000000                | 0.000000 | 0.000000 | 0.000000                      | 0.311020  | -1.770030 | -0.000000                   | 0.405000  | -2.197000 |
| 20  | Ru   | 0.500000                | 0.000000 | 0.500000 | 0.000000                      | -0.311020 | -1.770030 | -0.000000                   | -0.405000 | -2.197000 |
| 21  | Ru   | 0.000000                | 0.500000 | 0.000000 | -0.311020                     | 0.000000  | -1.770030 | -0.405000                   | 0.000000  | -2.198000 |
| 22  | Ru   | 0.000000                | 0.000000 | 0.500000 | 0.311020                      | 0.000000  | -1.770030 | 0.405000                    | 0.000000  | -2.197000 |

FIG. 17. First-principles calculation results of 0.51 Ho<sub>2</sub>Ru<sub>2</sub>O<sub>7</sub>. The band structure is shown in the left panel, and the Fermi-level-dependent AHC is plotted in the right panel. In both plots, the Fermi level is set to 0 eV.

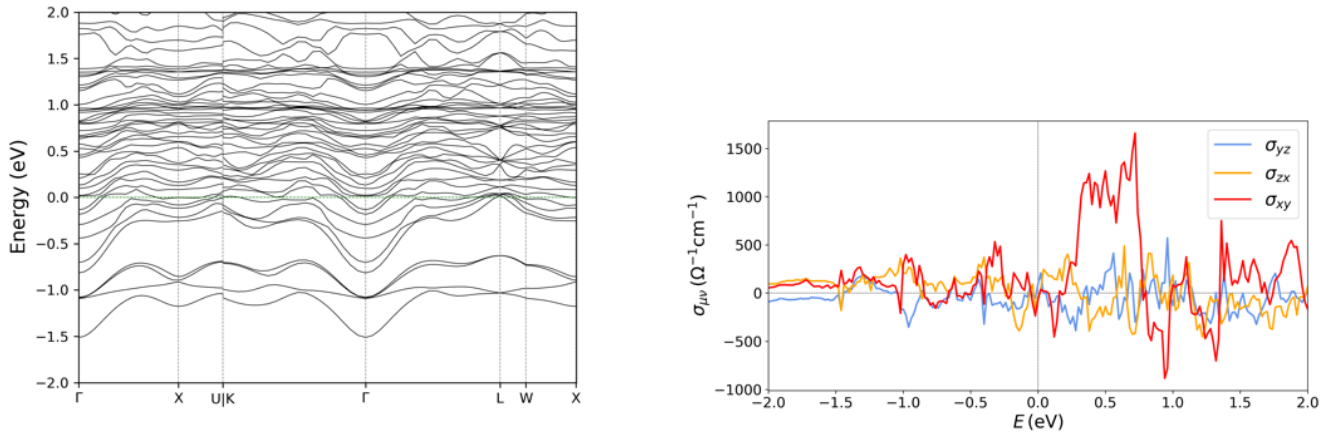

**0.593 UPSe** crystallizes in type III MSG 129.417, which hosts only FNSs. The symmetry-adapted AHC tensor of the MSG is  $(0, 0, \sigma_{xy})$ . Based on the first-principles calculation results, the comparison between the experimental and calculated magnetic moments is provided in Table SII20. The band structure is shown in the left panel of Fig. 18, and the Fermi-level-dependent AHC is plotted in the right panel.

TABLE SII20. The comparison between the experimental and calculated magnetic moments for 0.593 UPSe. The five columns contain the atom index in the structure file, the atom species, the fractional coordinates, the experimental magnetic moments, and the calculated magnetic moments. The lattice vectors are  $\vec{a}_1 = (3.951, 0.0, 0.0)$ ,  $\vec{a}_2 = (0.0, 3.951, 0.0)$ ,  $\vec{a}_3 = (0.0, 0.0, 8.185)$ .

| No. | Atom | Coordinates(fractional) |          |          | Experimental magnetic moments |          |          | Calculated magnetic moments |           |           |
|-----|------|-------------------------|----------|----------|-------------------------------|----------|----------|-----------------------------|-----------|-----------|
| 1   | U    | 0.250000                | 0.250000 | 0.739000 | 0.000000                      | 0.000000 | 1.350030 | 0.100000                    | 0.042000  | 1.801000  |
| 2   | U    | 0.750000                | 0.750000 | 0.261000 | 0.000000                      | 0.000000 | 1.350030 | -0.100000                   | -0.036000 | 1.801000  |
| 3   | Se   | 0.250000                | 0.250000 | 0.356500 | 0.000000                      | 0.000000 | 0.000000 | -0.000000                   | -0.001000 | -0.059000 |
| 4   | Se   | 0.750000                | 0.750000 | 0.643500 | 0.000000                      | 0.000000 | 0.000000 | -0.000000                   | -0.000000 | -0.059000 |
| 5   | P    | 0.750000                | 0.250000 | 0.000000 | 0.000000                      | 0.000000 | 0.000000 | 0.000000                    | -0.001000 | -0.036000 |
| 6   | P    | 0.250000                | 0.750000 | 0.000000 | 0.000000                      | 0.000000 | 0.000000 | -0.000000                   | -0.001000 | -0.036000 |

FIG. 18. First-principles calculation results of 0.593 UPSe. The band structure is shown in the left panel, and the Fermi-level-dependent AHC is plotted in the right panel. In both plots, the Fermi level is set to 0 eV.

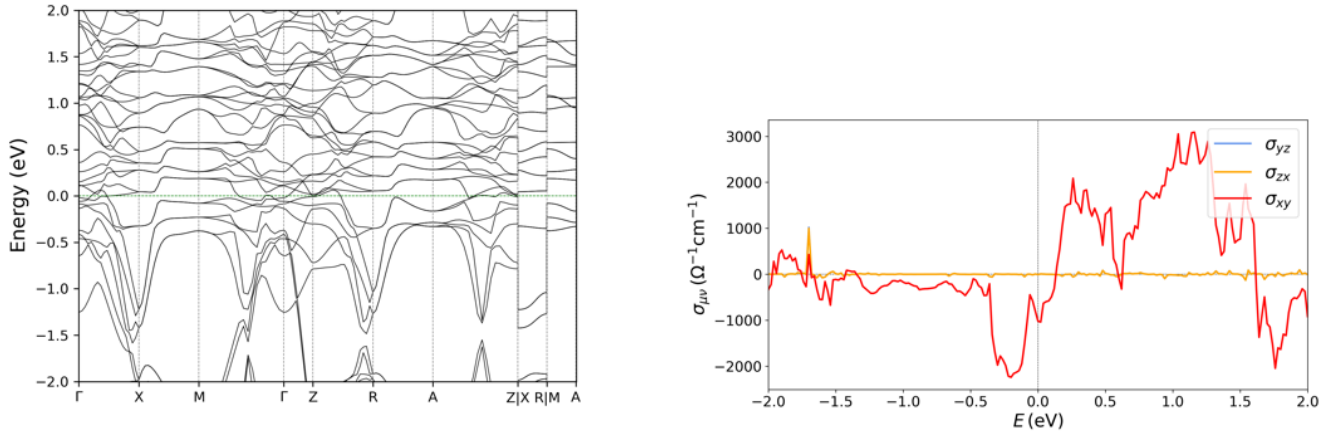

**0.594 UAsS** crystallizes in type III MSG 129.417, which hosts only FNSs. The symmetry-adapted AHC tensor of the MSG is  $(0, 0, \sigma_{xy})$ . Based on the first-principles calculation results, the comparison between the experimental and calculated magnetic moments is provided in Table SII21. The band structure is shown in the left panel of Fig. 19, and the Fermi-level-dependent AHC is plotted in the right panel.

TABLE SII21. The comparison between the experimental and calculated magnetic moments for 0.594 UAsS. The five columns contain the atom index in the structure file, the atom species, the fractional coordinates, the experimental magnetic moments, and the calculated magnetic moments. The lattice vectors are  $\vec{a}_1 = (3.884, 0.0, 0.0)$ ,  $\vec{a}_2 = (0.0, 3.884, 0.0)$ ,  $\vec{a}_3 = (0.0, 0.0, 8.176)$ .

| No. | Atom | Coordinates(fractional) |          |          | Experimental magnetic moments |          |          | Calculated magnetic moments |           |           |
|-----|------|-------------------------|----------|----------|-------------------------------|----------|----------|-----------------------------|-----------|-----------|
| 1   | U    | 0.250000                | 0.250000 | 0.716100 | 0.000000                      | 0.000000 | 1.239970 | 0.141000                    | 0.051000  | 1.689000  |
| 2   | U    | 0.750000                | 0.750000 | 0.283900 | 0.000000                      | 0.000000 | 1.239970 | -0.141000                   | -0.042000 | 1.689000  |
| 3   | S    | 0.250000                | 0.250000 | 0.368600 | 0.000000                      | 0.000000 | 0.000000 | -0.000000                   | 0.000000  | -0.050000 |
| 4   | S    | 0.750000                | 0.750000 | 0.631400 | 0.000000                      | 0.000000 | 0.000000 | 0.000000                    | -0.001000 | -0.050000 |
| 5   | As   | 0.750000                | 0.250000 | 0.000000 | 0.000000                      | 0.000000 | 0.000000 | -0.001000                   | -0.001000 | -0.029000 |
| 6   | As   | 0.250000                | 0.750000 | 0.000000 | 0.000000                      | 0.000000 | 0.000000 | 0.001000                    | -0.001000 | -0.029000 |

FIG. 19. First-principles calculation results of 0.594 UAsS. The band structure is shown in the left panel, and the Fermi-level-dependent AHC is plotted in the right panel. In both plots, the Fermi level is set to 0 eV.

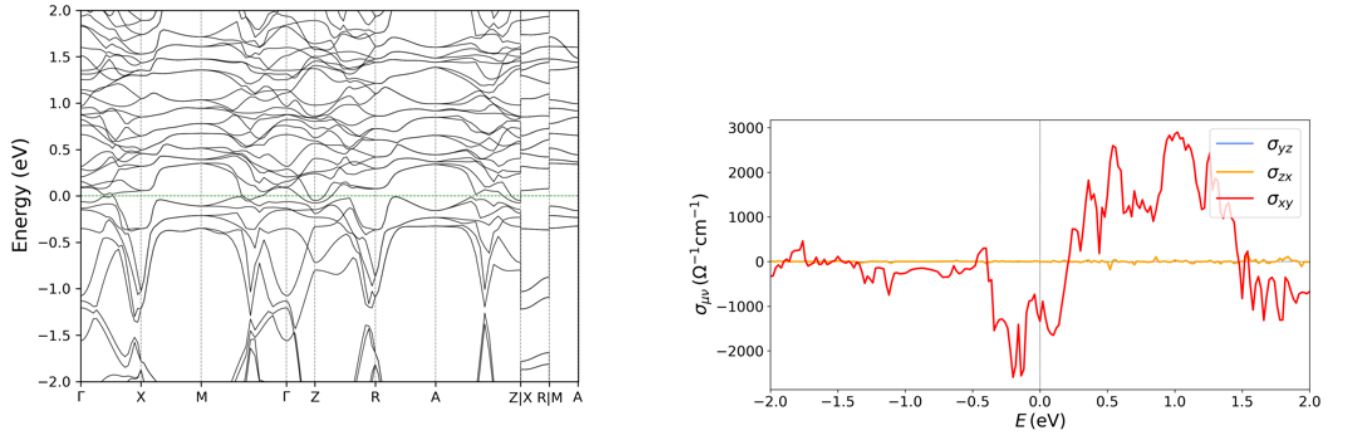

**0.664 Mn<sub>3</sub>Sn<sub>2</sub>** crystallizes in type III MSG 14.79, which hosts both SNLs and FNSs. The symmetry-adapted AHC tensor of the MSG is  $(\sigma_{yz}, \sigma_{zx}, 0)$ . Based on the first-principles calculation results, the comparison between the experimental and calculated magnetic moments is provided in Table SII22. The band structure is shown in the left panel of Fig. 20, and the Fermi-level-dependent AHC is plotted in the right panel.

TABLE SII22. The comparison between the experimental and calculated magnetic moments for 0.664 Mn<sub>3</sub>Sn<sub>2</sub>. The five columns contain the atom index in the structure file, the atom species, the fractional coordinates, the experimental magnetic moments, and the calculated magnetic moments. The lattice vectors are  $\vec{a}_1 = (5.5099, 0.0, 0.0)$ ,  $\vec{a}_2 = (0.0, 7.5646, 0.0)$ ,  $\vec{a}_3 = (-5.509899195, 0.0, 8.597497804)$ .

| No. | Atom | Coordinates(fractional) |          |          | Experimental magnetic moments |           |           | Calculated magnetic moments |           |           |
|-----|------|-------------------------|----------|----------|-------------------------------|-----------|-----------|-----------------------------|-----------|-----------|
| 1   | Mn   | 0.880700                | 0.224500 | 0.377100 | -0.000550                     | -2.319990 | -1.849750 | -0.000000                   | -3.316000 | -2.601000 |
| 2   | Mn   | 0.119300                | 0.775500 | 0.622900 | -0.000550                     | -2.319990 | -1.849750 | -0.001000                   | -3.315000 | -2.601000 |
| 3   | Mn   | 0.119300                | 0.724500 | 0.122900 | -0.000550                     | 2.319990  | -1.849750 | -0.001000                   | 3.315000  | -2.601000 |
| 4   | Mn   | 0.880700                | 0.275500 | 0.877100 | -0.000550                     | 2.319990  | -1.849750 | 0.000000                    | 3.315000  | -2.600000 |
| 5   | Mn   | 0.373500                | 0.275500 | 0.877100 | -0.000550                     | -2.319990 | -1.849750 | -0.000000                   | -3.315000 | -2.601000 |
| 6   | Mn   | 0.626500                | 0.724500 | 0.122900 | -0.000550                     | -2.319990 | -1.849750 | -0.001000                   | -3.316000 | -2.602000 |
| 7   | Mn   | 0.626500                | 0.775500 | 0.622900 | -0.000550                     | 2.319990  | -1.849750 | 0.000000                    | 3.316000  | -2.601000 |
| 8   | Mn   | 0.373500                | 0.224500 | 0.377100 | -0.000550                     | 2.319990  | -1.849750 | -0.002000                   | 3.316000  | -2.602000 |
| 9   | Mn   | 0.120100                | 0.907900 | 0.370100 | 0.000110                      | 0.000000  | -2.300170 | 0.005000                    | 0.000000  | -3.612000 |
| 10  | Mn   | 0.879900                | 0.092100 | 0.629900 | 0.000110                      | 0.000000  | -2.300170 | -0.005000                   | -0.000000 | -3.614000 |
| 11  | Mn   | 0.879900                | 0.407900 | 0.129900 | 0.000110                      | 0.000000  | -2.300170 | 0.004000                    | 0.000000  | -3.612000 |
| 12  | Mn   | 0.120100                | 0.592100 | 0.870100 | 0.000110                      | 0.000000  | -2.300170 | -0.003000                   | -0.000000 | -3.614000 |
| 13  | Sn   | 0.607400                | 0.596900 | 0.857400 | 0.000000                      | 0.000000  | 0.000000  | 0.001000                    | 0.000000  | 0.164000  |
| 14  | Sn   | 0.392600                | 0.403100 | 0.142600 | 0.000000                      | 0.000000  | 0.000000  | -0.002000                   | -0.001000 | 0.164000  |
| 15  | Sn   | 0.392600                | 0.096900 | 0.642600 | 0.000000                      | 0.000000  | 0.000000  | 0.000000                    | 0.000000  | 0.164000  |
| 16  | Sn   | 0.607400                | 0.903100 | 0.357400 | 0.000000                      | 0.000000  | 0.000000  | -0.001000                   | 0.000000  | 0.164000  |
| 17  | Sn   | 0.156800                | 0.561000 | 0.406800 | 0.000000                      | 0.000000  | 0.000000  | 0.001000                    | 0.000000  | 0.135000  |
| 18  | Sn   | 0.843200                | 0.439000 | 0.593200 | 0.000000                      | 0.000000  | 0.000000  | -0.001000                   | -0.000000 | 0.135000  |
| 19  | Sn   | 0.843200                | 0.061000 | 0.093200 | 0.000000                      | 0.000000  | 0.000000  | 0.002000                    | 0.000000  | 0.135000  |
| 20  | Sn   | 0.156800                | 0.939000 | 0.906800 | 0.000000                      | 0.000000  | 0.000000  | -0.002000                   | -0.000000 | 0.135000  |

FIG. 20. First-principles calculation results of 0.664 Mn<sub>3</sub>Sn<sub>2</sub>. The band structure is shown in the left panel, and the Fermi-level-dependent AHC is plotted in the right panel. In both plots, the Fermi level is set to 0 eV.

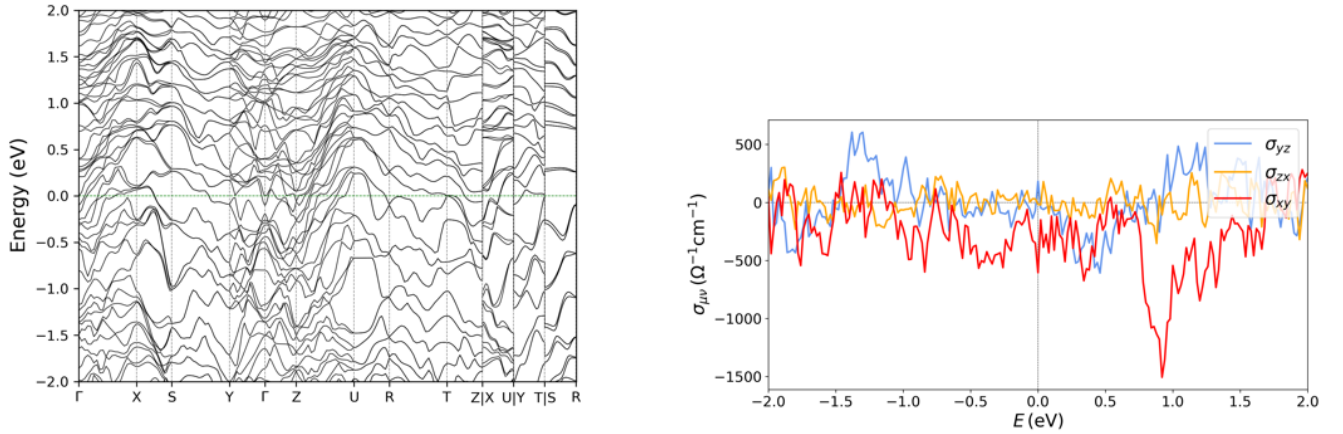



**0.685 ErPt** crystallizes in type III MSG 62.447, which hosts both SNLs and FNSs. The symmetry-adapted AHC tensor of the MSG is  $(\sigma_{yz}, 0, 0)$ . Based on the first-principles calculation results, the comparison between the experimental and calculated magnetic moments is provided in Table SII23. The band structure is shown in the left panel of Fig. 21, and the Fermi-level-dependent AHC is plotted in the right panel.

TABLE SII23. The comparison between the experimental and calculated magnetic moments for 0.685 ErPt. The five columns contain the atom index in the structure file, the atom species, the fractional coordinates, the experimental magnetic moments, and the calculated magnetic moments. The lattice vectors are  $\vec{a}_1 = (6.906, 0.0, 0.0)$ ,  $\vec{a}_2 = (0.0, 4.451, 0.0)$ ,  $\vec{a}_3 = (0.0, 0.0, 5.509)$ .

| No. | Atom | Coordinates(fractional) |          |          | Experimental magnetic moments |          |           | Calculated magnetic moments |           |           |
|-----|------|-------------------------|----------|----------|-------------------------------|----------|-----------|-----------------------------|-----------|-----------|
| 1   | Er   | 0.685000                | 0.250000 | 0.144000 | 7.699980                      | 0.000000 | 2.499980  | 6.260000                    | 0.004000  | 2.027000  |
| 2   | Er   | 0.185000                | 0.250000 | 0.356000 | 7.699980                      | 0.000000 | -2.499980 | 6.253000                    | 0.006000  | -2.026000 |
| 3   | Er   | 0.315000                | 0.750000 | 0.856000 | 7.699980                      | 0.000000 | 2.499980  | 6.257000                    | -0.004000 | 2.026000  |
| 4   | Er   | 0.815000                | 0.750000 | 0.644000 | 7.699980                      | 0.000000 | -2.499980 | 6.256000                    | -0.006000 | -2.026000 |
| 5   | Pt   | 0.548000                | 0.250000 | 0.653000 | 0.000000                      | 0.000000 | 0.000000  | -0.609000                   | 0.001000  | -0.048000 |
| 6   | Pt   | 0.048000                | 0.250000 | 0.847000 | 0.000000                      | 0.000000 | 0.000000  | -0.624000                   | 0.005000  | 0.036000  |
| 7   | Pt   | 0.452000                | 0.750000 | 0.347000 | 0.000000                      | 0.000000 | 0.000000  | -0.610000                   | -0.000000 | -0.046000 |
| 8   | Pt   | 0.952000                | 0.750000 | 0.153000 | 0.000000                      | 0.000000 | 0.000000  | -0.623000                   | -0.005000 | 0.039000  |

FIG. 21. First-principles calculation results of 0.685 ErPt. The band structure is shown in the left panel, and the Fermi-level-dependent AHC is plotted in the right panel. In both plots, the Fermi level is set to 0 eV.

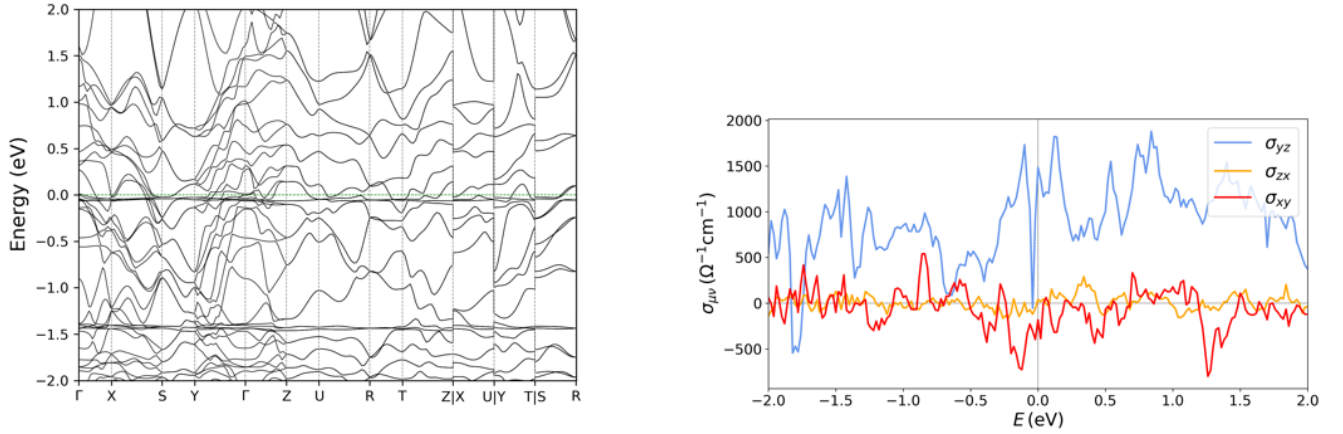



**0.687 DyPt** crystallizes in type III MSG 62.446, which hosts both SNLs and FNSs. The symmetry-adapted AHC tensor of the MSG is  $(0, 0, \sigma_{xy})$ . Based on the first-principles calculation results, the comparison between the experimental and calculated magnetic moments is provided in Table SII24. The band structure is shown in the left panel of Fig. 22, and the Fermi-level-dependent AHC is plotted in the right panel.

TABLE SII24. The comparison between the experimental and calculated magnetic moments for 0.687 DyPt. The five columns contain the atom index in the structure file, the atom species, the fractional coordinates, the experimental magnetic moments, and the calculated magnetic moments. The lattice vectors are  $\vec{a}_1 = (6.973, 0.0, 0.0)$ ,  $\vec{a}_2 = (0.0, 4.48, 0.0)$ ,  $\vec{a}_3 = (0.0, 0.0, 5.541)$ .

| No. | Atom | Coordinates(fractional) |          |          | Experimental magnetic moments |          |          | Calculated magnetic moments |           |           |
|-----|------|-------------------------|----------|----------|-------------------------------|----------|----------|-----------------------------|-----------|-----------|
| 1   | Dy   | 0.319000                | 0.250000 | 0.628000 | 4.929980                      | 0.000000 | 5.110020 | 5.320000                    | -0.013000 | 5.543000  |
| 2   | Dy   | 0.181000                | 0.750000 | 0.128000 | -4.929980                     | 0.000000 | 5.110020 | -5.315000                   | 0.009000  | 5.541000  |
| 3   | Dy   | 0.681000                | 0.750000 | 0.372000 | 4.929980                      | 0.000000 | 5.110020 | 5.318000                    | 0.011000  | 5.544000  |
| 4   | Dy   | 0.819000                | 0.250000 | 0.872000 | -4.929980                     | 0.000000 | 5.110020 | -5.317000                   | -0.010000 | 5.541000  |
| 5   | Pt   | 0.463000                | 0.250000 | 0.115000 | 0.000000                      | 0.000000 | 0.000000 | -0.033000                   | 0.004000  | -0.262000 |
| 6   | Pt   | 0.037000                | 0.750000 | 0.615000 | 0.000000                      | 0.000000 | 0.000000 | 0.030000                    | -0.007000 | -0.259000 |
| 7   | Pt   | 0.537000                | 0.750000 | 0.885000 | 0.000000                      | 0.000000 | 0.000000 | -0.027000                   | -0.005000 | -0.260000 |
| 8   | Pt   | 0.963000                | 0.250000 | 0.385000 | 0.000000                      | 0.000000 | 0.000000 | 0.035000                    | 0.006000  | -0.261000 |

FIG. 22. First-principles calculation results of 0.687 DyPt. The band structure is shown in the left panel, and the Fermi-level-dependent AHC is plotted in the right panel. In both plots, the Fermi level is set to 0 eV.

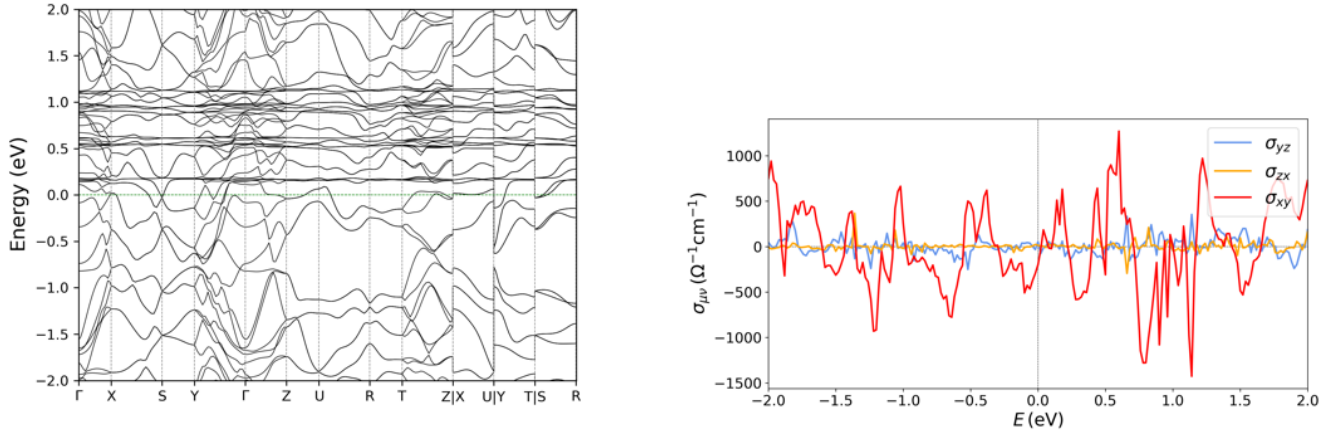

**0.707 Tb<sub>2</sub>Ir<sub>3</sub>Ga<sub>9</sub>** crystallizes in type III MSG 63.464, which hosts only FNSs. The symmetry-adapted AHC tensor of the MSG is  $(0, \sigma_{zx}, 0)$ . Based on the first-principles calculation results, the comparison between the experimental and calculated magnetic moments is provided in Table SII25. The band structure is shown in the left panel of Fig. 23, and the Fermi-level-dependent AHC is plotted in the right panel.

TABLE SII25. The comparison between the experimental and calculated magnetic moments for 0.707 Tb<sub>2</sub>Ir<sub>3</sub>Ga<sub>9</sub>. The five columns contain the atom index in the structure file, the atom species, the fractional coordinates, the experimental magnetic moments, and the calculated magnetic moments. The lattice vectors are  $\vec{a}_1 = (6.493, -3.76625, 0.0)$ ,  $\vec{a}_2 = (6.493, 3.76625, 0.0)$ ,  $\vec{a}_3 = (0.0, 0.0, 9.4349)$ .

| No. | Atom | Coordinates(fractional) |          |          | Experimental magnetic moments |          |          | Calculated magnetic moments |           |           |
|-----|------|-------------------------|----------|----------|-------------------------------|----------|----------|-----------------------------|-----------|-----------|
| 1   | Tb   | 0.004000                | 0.668000 | 0.250000 | 8.899960                      | 1.029990 | 0.000000 | 9.100000                    | 1.046000  | -0.000000 |
| 2   | Tb   | 0.332000                | 0.996000 | 0.250000 | -8.899960                     | 1.029990 | 0.000000 | -9.105000                   | 1.047000  | -0.000000 |
| 3   | Tb   | 0.996000                | 0.332000 | 0.750000 | 8.899960                      | 1.029990 | 0.000000 | 9.102000                    | 1.046000  | -0.000000 |
| 4   | Tb   | 0.668000                | 0.004000 | 0.750000 | -8.899960                     | 1.029990 | 0.000000 | -9.103000                   | 1.046000  | -0.000000 |
| 5   | Ir   | 0.328300                | 0.328300 | 0.000000 | 0.000000                      | 0.000000 | 0.000000 | 0.005000                    | -0.023000 | 0.004000  |
| 6   | Ir   | 0.671700                | 0.671700 | 0.500000 | 0.000000                      | 0.000000 | 0.000000 | 0.006000                    | -0.024000 | 0.001000  |
| 7   | Ir   | 0.671700                | 0.671700 | 0.000000 | 0.000000                      | 0.000000 | 0.000000 | 0.006000                    | -0.020000 | -0.002000 |
| 8   | Ir   | 0.328300                | 0.328300 | 0.500000 | 0.000000                      | 0.000000 | 0.000000 | 0.006000                    | -0.023000 | -0.001000 |
| 9   | Ir   | 0.000000                | 0.000000 | 0.000000 | 0.000000                      | 0.000000 | 0.000000 | -0.000000                   | -0.033000 | 0.001000  |
| 10  | Ir   | 0.000000                | 0.000000 | 0.500000 | 0.000000                      | 0.000000 | 0.000000 | -0.000000                   | -0.033000 | -0.003000 |
| 11  | Ga   | 0.999400                | 0.334800 | 0.078700 | 0.000000                      | 0.000000 | 0.000000 | 0.007000                    | -0.003000 | 0.001000  |
| 12  | Ga   | 0.665200                | 0.000600 | 0.421300 | 0.000000                      | 0.000000 | 0.000000 | -0.003000                   | -0.002000 | 0.000000  |
| 13  | Ga   | 0.000600                | 0.665200 | 0.921300 | 0.000000                      | 0.000000 | 0.000000 | 0.007000                    | -0.002000 | 0.001000  |
| 14  | Ga   | 0.334800                | 0.999400 | 0.578700 | 0.000000                      | 0.000000 | 0.000000 | -0.003000                   | -0.002000 | -0.001000 |
| 15  | Ga   | 0.334800                | 0.999400 | 0.921300 | 0.000000                      | 0.000000 | 0.000000 | -0.003000                   | -0.003000 | 0.001000  |
| 16  | Ga   | 0.000600                | 0.665200 | 0.578700 | 0.000000                      | 0.000000 | 0.000000 | 0.007000                    | -0.002000 | 0.000000  |
| 17  | Ga   | 0.665200                | 0.000600 | 0.078700 | 0.000000                      | 0.000000 | 0.000000 | -0.003000                   | -0.002000 | 0.000000  |
| 18  | Ga   | 0.999400                | 0.334800 | 0.421300 | 0.000000                      | 0.000000 | 0.000000 | 0.007000                    | -0.003000 | -0.001000 |
| 19  | Ga   | 0.661000                | 0.546400 | 0.250000 | 0.000000                      | 0.000000 | 0.000000 | -0.015000                   | -0.004000 | 0.001000  |
| 20  | Ga   | 0.453600                | 0.339000 | 0.250000 | 0.000000                      | 0.000000 | 0.000000 | 0.010000                    | -0.003000 | -0.001000 |
| 21  | Ga   | 0.339000                | 0.453600 | 0.750000 | 0.000000                      | 0.000000 | 0.000000 | -0.014000                   | -0.003000 | -0.001000 |
| 22  | Ga   | 0.546400                | 0.661000 | 0.750000 | 0.000000                      | 0.000000 | 0.000000 | 0.011000                    | -0.004000 | 0.001000  |
| 23  | Ga   | 0.666900                | 0.333100 | 0.563300 | 0.000000                      | 0.000000 | 0.000000 | 0.000000                    | -0.005000 | -0.001000 |
| 24  | Ga   | 0.666900                | 0.333100 | 0.936700 | 0.000000                      | 0.000000 | 0.000000 | 0.000000                    | -0.006000 | 0.001000  |
| 25  | Ga   | 0.333100                | 0.666900 | 0.436700 | 0.000000                      | 0.000000 | 0.000000 | 0.000000                    | -0.005000 | -0.001000 |
| 26  | Ga   | 0.333100                | 0.666900 | 0.063300 | 0.000000                      | 0.000000 | 0.000000 | 0.000000                    | -0.005000 | 0.001000  |
| 27  | Ga   | 0.870700                | 0.129300 | 0.250000 | 0.000000                      | 0.000000 | 0.000000 | 0.004000                    | -0.003000 | 0.000000  |
| 28  | Ga   | 0.129300                | 0.870700 | 0.750000 | 0.000000                      | 0.000000 | 0.000000 | 0.003000                    | -0.003000 | -0.000000 |

FIG. 23. First-principles calculation results of 0.707 Tb<sub>2</sub>Ir<sub>3</sub>Ga<sub>9</sub>. The band structure is shown in the left panel, and the Fermi-level-dependent AHC is plotted in the right panel. In both plots, the Fermi level is set to 0 eV.

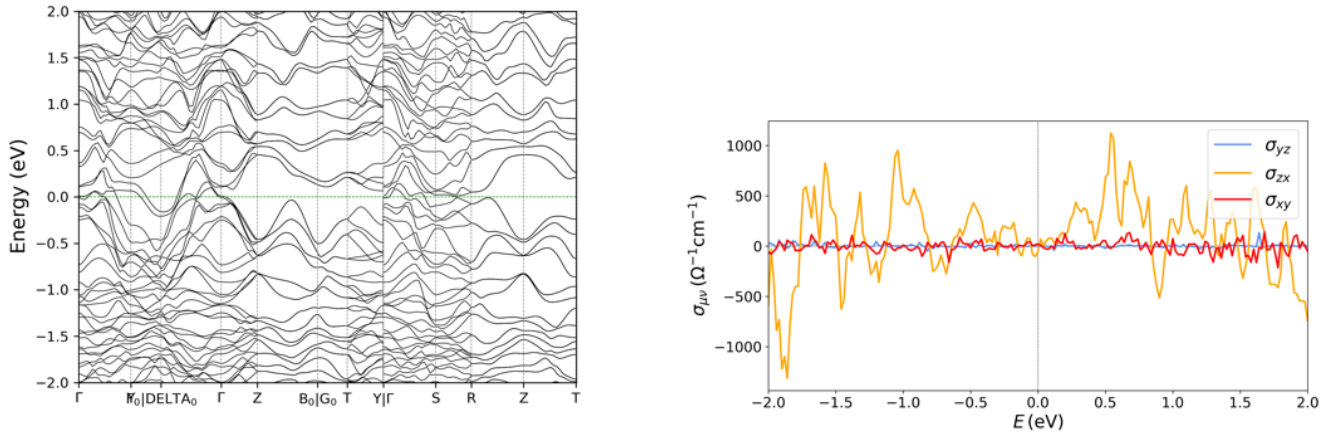

**0.772 PrMnSi<sub>2</sub>** crystallizes in type III MSG 63.464, which hosts only FNSs. The symmetry-adapted AHC tensor of the MSG is  $(0, \sigma_{zx}, 0)$ . Based on the first-principles calculation results, the comparison between the experimental and calculated magnetic moments is provided in Table SII26. The band structure is shown in the left panel of Fig. 24, and the Fermi-level-dependent AHC is plotted in the right panel.

TABLE SII26. The comparison between the experimental and calculated magnetic moments for 0.772 PrMnSi<sub>2</sub>. The five columns contain the atom index in the structure file, the atom species, the fractional coordinates, the experimental magnetic moments, and the calculated magnetic moments. The lattice vectors are  $\vec{a}_1 = (2.047, -8.775, 0.0)$ ,  $\vec{a}_2 = (2.047, 8.775, 0.0)$ ,  $\vec{a}_3 = (0.0, 0.0, 4.028)$ .

| No. | Atom | Coordinates(fractional) |          |          | Experimental magnetic moments |          |          | Calculated magnetic moments |           |           |
|-----|------|-------------------------|----------|----------|-------------------------------|----------|----------|-----------------------------|-----------|-----------|
| 1   | Pr   | 0.897400                | 0.102600 | 0.250000 | 0.000000                      | 0.000000 | 0.000000 | 0.006000                    | -0.042000 | 0.001000  |
| 2   | Pr   | 0.102600                | 0.897400 | 0.750000 | 0.000000                      | 0.000000 | 0.000000 | -0.005000                   | -0.042000 | 0.001000  |
| 3   | Mn   | 0.251200                | 0.748800 | 0.250000 | 0.000000                      | 1.929970 | 0.000000 | -0.010000                   | 3.258000  | 0.002000  |
| 4   | Mn   | 0.748800                | 0.251200 | 0.750000 | 0.000000                      | 1.929970 | 0.000000 | 0.010000                    | 3.258000  | -0.000000 |
| 5   | Si   | 0.673300                | 0.326700 | 0.250000 | 0.000000                      | 0.000000 | 0.000000 | -0.000000                   | -0.093000 | -0.000000 |
| 6   | Si   | 0.326700                | 0.673300 | 0.750000 | 0.000000                      | 0.000000 | 0.000000 | 0.000000                    | -0.093000 | 0.000000  |
| 7   | Si   | 0.534200                | 0.465800 | 0.250000 | 0.000000                      | 0.000000 | 0.000000 | 0.001000                    | -0.004000 | 0.000000  |
| 8   | Si   | 0.465800                | 0.534200 | 0.750000 | 0.000000                      | 0.000000 | 0.000000 | -0.000000                   | -0.004000 | 0.000000  |

FIG. 24. First-principles calculation results of 0.772 PrMnSi<sub>2</sub>. The band structure is shown in the left panel, and the Fermi-level-dependent AHC is plotted in the right panel. In both plots, the Fermi level is set to 0 eV.

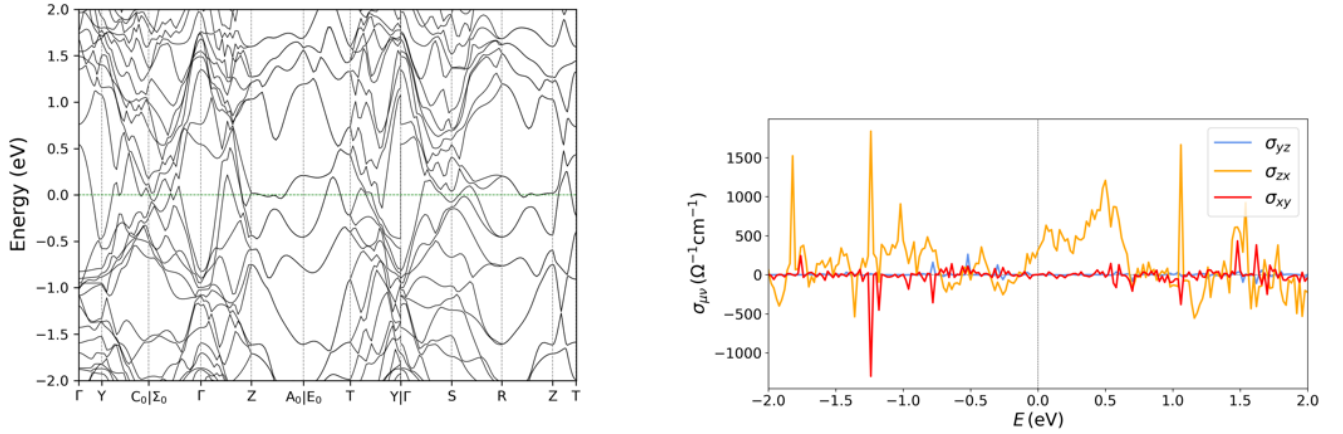

**0.789 CeCuSi** crystallizes in type III MSG 63.463, which hosts only FNSs. The symmetry-adapted AHC tensor of the MSG is  $(\sigma_{yz}, 0, 0)$ . Based on the first-principles calculation results, the comparison between the experimental and calculated magnetic moments is provided in Table SII27. The band structure is shown in the left panel of Fig. 25, and the Fermi-level-dependent AHC is plotted in the right panel.

TABLE SII27. The comparison between the experimental and calculated magnetic moments for 0.789 CeCuSi. The five columns contain the atom index in the structure file, the atom species, the fractional coordinates, the experimental magnetic moments, and the calculated magnetic moments. The lattice vectors are  $\vec{a}_1 = (2.114, -3.661555, 0.0)$ ,  $\vec{a}_2 = (2.114, 3.661555, 0.0)$ ,  $\vec{a}_3 = (0.0, 0.0, 7.926)$ .

| No. | Atom | Coordinates(fractional) |          |          | Experimental magnetic moments |          |          | Calculated magnetic moments |           |           |
|-----|------|-------------------------|----------|----------|-------------------------------|----------|----------|-----------------------------|-----------|-----------|
| 1   | Ce   | 0.000000                | 0.000000 | 0.000000 | 1.250010                      | 0.000000 | 0.000000 | 1.168000                    | -0.000000 | -0.000000 |
| 2   | Ce   | 0.000000                | 0.000000 | 0.500000 | 1.250010                      | 0.000000 | 0.000000 | 1.164000                    | 0.000000  | 0.000000  |
| 3   | Cu   | 0.333333                | 0.666667 | 0.250000 | 0.000000                      | 0.000000 | 0.000000 | -0.030000                   | 0.000000  | -0.000000 |
| 4   | Cu   | 0.666667                | 0.333333 | 0.750000 | 0.000000                      | 0.000000 | 0.000000 | -0.030000                   | -0.000000 | 0.000000  |
| 5   | Si   | 0.666667                | 0.333333 | 0.250000 | 0.000000                      | 0.000000 | 0.000000 | -0.071000                   | 0.000000  | -0.002000 |
| 6   | Si   | 0.333333                | 0.666667 | 0.750000 | 0.000000                      | 0.000000 | 0.000000 | -0.071000                   | -0.000000 | 0.002000  |

FIG. 25. First-principles calculation results of 0.789 CeCuSi. The band structure is shown in the left panel, and the Fermi-level-dependent AHC is plotted in the right panel. In both plots, the Fermi level is set to 0 eV.

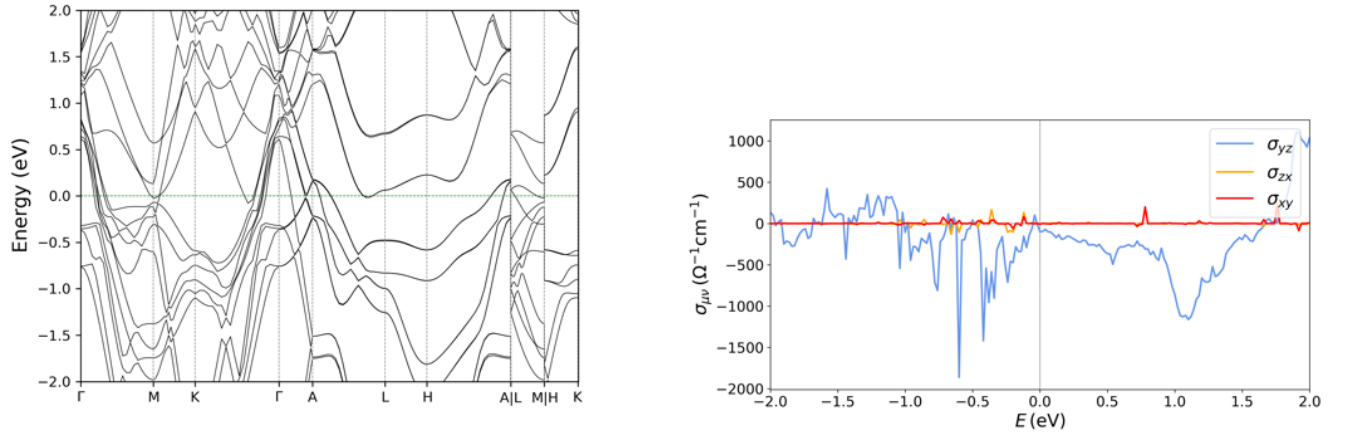

**0.79 CaIrO<sub>3</sub>** crystallizes in type III MSG 63.464, which hosts only FNSs. The symmetry-adapted AHC tensor of the MSG is  $(0, \sigma_{zx}, 0)$ . Based on the first-principles calculation results, the comparison between the experimental and calculated magnetic moments is provided in Table SII28. The band structure is shown in the left panel of Fig. 26, and the Fermi-level-dependent AHC is plotted in the right panel.

TABLE SII28. The comparison between the experimental and calculated magnetic moments for 0.79 CaIrO<sub>3</sub>. The five columns contain the atom index in the structure file, the atom species, the fractional coordinates, the experimental magnetic moments, and the calculated magnetic moments. The lattice vectors are  $\vec{a}_1 = (1.5736, -4.93275, 0.0)$ ,  $\vec{a}_2 = (1.5736, 4.93275, 0.0)$ ,  $\vec{a}_3 = (0.0, 0.0, 7.3018)$ .

| No. | Atom | Coordinates(fractional) |          |          | Experimental magnetic moments |          |           | Calculated magnetic moments |           |           |
|-----|------|-------------------------|----------|----------|-------------------------------|----------|-----------|-----------------------------|-----------|-----------|
| 1   | Ca   | 0.250800                | 0.749200 | 0.250000 | 0.000000                      | 0.000000 | 0.000000  | -0.001000                   | -0.000000 | 0.000000  |
| 2   | Ca   | 0.749200                | 0.250800 | 0.750000 | 0.000000                      | 0.000000 | 0.000000  | 0.001000                    | -0.000000 | 0.000000  |
| 3   | Ir   | 0.000000                | 0.000000 | 0.000000 | 0.000000                      | 0.000000 | 0.999980  | 0.000000                    | 0.006000  | 1.056000  |
| 4   | Ir   | 0.000000                | 0.000000 | 0.500000 | 0.000000                      | 0.000000 | -0.999980 | 0.000000                    | 0.007000  | -1.057000 |
| 5   | O    | 0.922100                | 0.077900 | 0.250000 | 0.000000                      | 0.000000 | 0.000000  | 0.004000                    | 0.000000  | -0.001000 |
| 6   | O    | 0.077900                | 0.922100 | 0.750000 | 0.000000                      | 0.000000 | 0.000000  | -0.003000                   | 0.000000  | -0.000000 |
| 7   | O    | 0.634200                | 0.365800 | 0.445200 | 0.000000                      | 0.000000 | 0.000000  | -0.004000                   | -0.002000 | 0.039000  |
| 8   | O    | 0.634200                | 0.365800 | 0.054800 | 0.000000                      | 0.000000 | 0.000000  | -0.001000                   | -0.003000 | -0.040000 |
| 9   | O    | 0.365800                | 0.634200 | 0.554800 | 0.000000                      | 0.000000 | 0.000000  | 0.004000                    | -0.003000 | 0.040000  |
| 10  | O    | 0.365800                | 0.634200 | 0.945200 | 0.000000                      | 0.000000 | 0.000000  | 0.001000                    | -0.002000 | -0.039000 |

FIG. 26. First-principles calculation results of 0.79 CaIrO<sub>3</sub>. The band structure is shown in the left panel, and the Fermi-level-dependent AHC is plotted in the right panel. In both plots, the Fermi level is set to 0 eV.

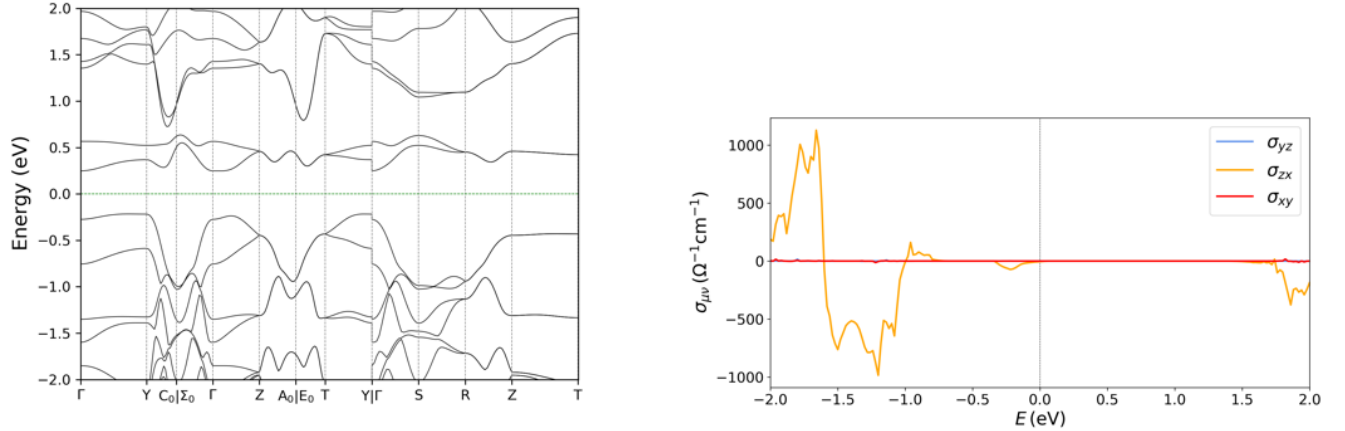

**0.832 CeAuGe** crystallizes in type III MSG 36.175, which hosts only FNSs. The symmetry-adapted AHC tensor of the MSG is  $(\sigma_{yz}, 0, 0)$ . Based on the first-principles calculation results, the comparison between the experimental and calculated magnetic moments is provided in Table SII29. The band structure is shown in the left panel of Fig. 27, and the Fermi-level-dependent AHC is plotted in the right panel.

TABLE SII29. The comparison between the experimental and calculated magnetic moments for 0.832 CeAuGe. The five columns contain the atom index in the structure file, the atom species, the fractional coordinates, the experimental magnetic moments, and the calculated magnetic moments. The lattice vectors are  $\vec{a}_1 = (2.228905, -3.860575, 0.0)$ ,  $\vec{a}_2 = (2.228905, 3.860575, 0.0)$ ,  $\vec{a}_3 = (0.0, 0.0, 7.8547)$ .

| No. | Atom | Coordinates(fractional) |          |          | Experimental magnetic moments |          |          | Calculated magnetic moments |           |           |
|-----|------|-------------------------|----------|----------|-------------------------------|----------|----------|-----------------------------|-----------|-----------|
| 1   | Ce   | 0.000000                | 0.000000 | 0.000000 | -1.059980                     | 0.000000 | 0.000000 | -0.791000                   | -0.001000 | -0.041000 |
| 2   | Ce   | 0.000000                | 0.000000 | 0.500000 | -1.059980                     | 0.000000 | 0.000000 | -0.791000                   | -0.001000 | 0.041000  |
| 3   | Au   | 0.666667                | 0.333333 | 0.800000 | 0.000000                      | 0.000000 | 0.000000 | -0.012000                   | -0.000000 | -0.011000 |
| 4   | Au   | 0.333333                | 0.666667 | 0.300000 | 0.000000                      | 0.000000 | 0.000000 | -0.012000                   | -0.000000 | 0.011000  |
| 5   | Ge   | 0.666667                | 0.333333 | 0.200000 | 0.000000                      | 0.000000 | 0.000000 | -0.007000                   | -0.000000 | -0.001000 |
| 6   | Ge   | 0.333333                | 0.666667 | 0.700000 | 0.000000                      | 0.000000 | 0.000000 | -0.007000                   | -0.000000 | 0.001000  |

FIG. 27. First-principles calculation results of 0.832 CeAuGe. The band structure is shown in the left panel, and the Fermi-level-dependent AHC is plotted in the right panel. In both plots, the Fermi level is set to 0 eV.

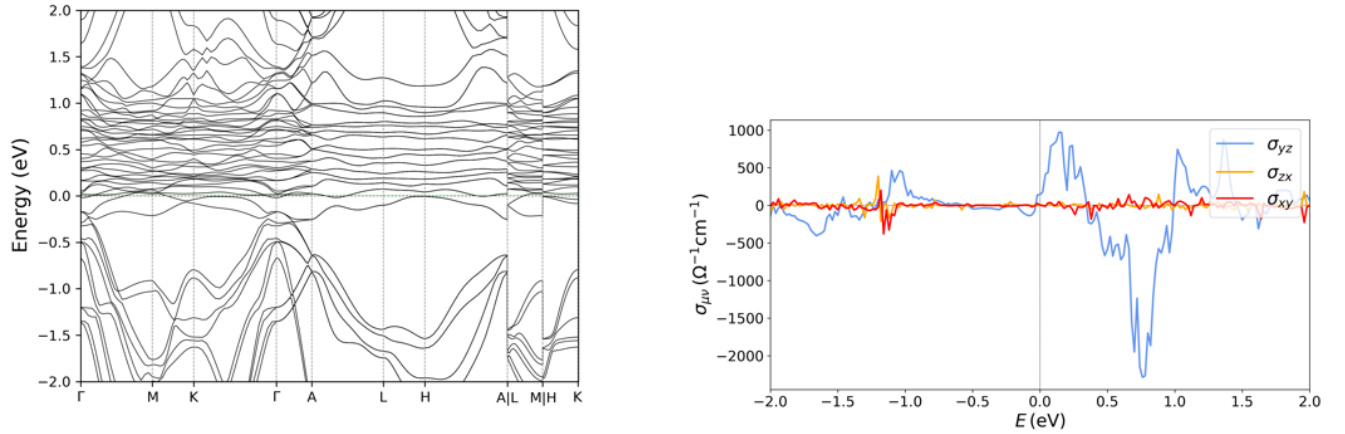

**2.28 NpNiGa<sub>5</sub>** crystallizes in type III MSG 74.559, which hosts only SNLs. The symmetry-adapted AHC tensor of the MSG is  $(\sigma_{yz}, 0, 0)$ . Based on the first-principles calculation results, the comparison between the experimental and calculated magnetic moments is provided in Table SII30. The band structure is shown in the left panel of Fig. 28, and the Fermi-level-dependent AHC is plotted in the right panel.

TABLE SII30. The comparison between the experimental and calculated magnetic moments for 2.28 NpNiGa<sub>5</sub>. The five columns contain the atom index in the structure file, the atom species, the fractional coordinates, the experimental magnetic moments, and the calculated magnetic moments. The lattice vectors are  $\vec{a}_1 = (-6.7858, 2.99481, 2.99481)$ ,  $\vec{a}_2 = (6.7858, -2.99481, 2.99481)$ ,  $\vec{a}_3 = (6.7858, 2.99481, -2.99481)$ .

| No. | Atom | Coordinates(fractional) |          |          | Experimental magnetic moments |          |           | Calculated magnetic moments |           |           |
|-----|------|-------------------------|----------|----------|-------------------------------|----------|-----------|-----------------------------|-----------|-----------|
| 1   | Np   | 0.000000                | 0.000000 | 0.500000 | -0.589960                     | 0.000000 | 0.593990  | -0.854000                   | 0.001000  | 0.859000  |
| 2   | Np   | 0.000000                | 0.500000 | 0.000000 | -0.589960                     | 0.000000 | -0.593990 | -0.848000                   | 0.001000  | -0.868000 |
| 3   | Ni   | 0.000000                | 0.750000 | 0.250000 | 0.000000                      | 0.000000 | 0.000000  | 0.002000                    | -0.001000 | -0.001000 |
| 4   | Ni   | 0.000000                | 0.250000 | 0.750000 | 0.000000                      | 0.000000 | 0.000000  | 0.002000                    | 0.001000  | -0.001000 |
| 5   | Ga   | 0.500000                | 0.500000 | 0.500000 | 0.000000                      | 0.000000 | 0.000000  | -0.004000                   | -0.000000 | 0.001000  |
| 6   | Ga   | 0.500000                | 0.000000 | 0.000000 | 0.000000                      | 0.000000 | 0.000000  | -0.004000                   | -0.000000 | -0.001000 |
| 7   | Ga   | 0.000000                | 0.903050 | 0.903050 | 0.000000                      | 0.000000 | 0.000000  | -0.001000                   | 0.000000  | -0.001000 |
| 8   | Ga   | 0.000000                | 0.096950 | 0.096950 | 0.000000                      | 0.000000 | 0.000000  | -0.001000                   | -0.001000 | -0.001000 |
| 9   | Ga   | 0.500000                | 0.096950 | 0.596950 | 0.000000                      | 0.000000 | 0.000000  | -0.001000                   | -0.000000 | -0.001000 |
| 10  | Ga   | 0.500000                | 0.903050 | 0.403050 | 0.000000                      | 0.000000 | 0.000000  | -0.001000                   | 0.000000  | 0.000000  |
| 11  | Ga   | 0.000000                | 0.596950 | 0.596950 | 0.000000                      | 0.000000 | 0.000000  | 0.001000                    | -0.000000 | -0.000000 |
| 12  | Ga   | 0.000000                | 0.403050 | 0.403050 | 0.000000                      | 0.000000 | 0.000000  | 0.001000                    | 0.001000  | 0.001000  |
| 13  | Ga   | 0.500000                | 0.403050 | 0.903050 | 0.000000                      | 0.000000 | 0.000000  | 0.001000                    | 0.000000  | 0.000000  |
| 14  | Ga   | 0.500000                | 0.596950 | 0.096950 | 0.000000                      | 0.000000 | 0.000000  | 0.001000                    | -0.000000 | -0.000000 |

FIG. 28. First-principles calculation results of 2.28 NpNiGa<sub>5</sub>. The band structure is shown in the left panel, and the Fermi-level-dependent AHC is plotted in the right panel. In both plots, the Fermi level is set to 0 eV.

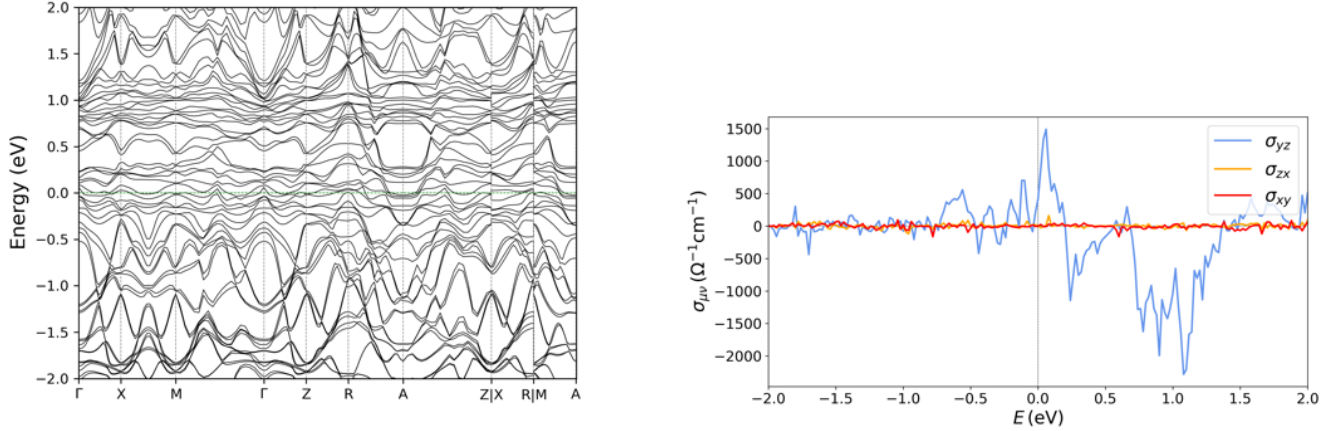



**2.57 TbMn<sub>2</sub>Si<sub>2</sub>** crystallizes in type III MSG 59.410, which hosts both SNLs and FNSs. The symmetry-adapted AHC tensor of the MSG is  $(\sigma_{yz}, 0, 0)$ . Based on the first-principles calculation results, the comparison between the experimental and calculated magnetic moments is provided in Table SII31. The band structure is shown in the left panel of Fig. 29, and the Fermi-level-dependent AHC is plotted in the right panel.

TABLE SII31. The comparison between the experimental and calculated magnetic moments for 2.57 TbMn<sub>2</sub>Si<sub>2</sub>. The five columns contain the atom index in the structure file, the atom species, the fractional coordinates, the experimental magnetic moments, and the calculated magnetic moments. The lattice vectors are  $\vec{a}_1 = (10.456, 0.0, 0.0)$ ,  $\vec{a}_2 = (0.0, 3.931, 0.0)$ ,  $\vec{a}_3 = (0.0, 0.0, 3.931)$ .

| No. | Atom | Coordinates(fractional) |          |          | Experimental magnetic moments |          |           | Calculated magnetic moments |           |           |
|-----|------|-------------------------|----------|----------|-------------------------------|----------|-----------|-----------------------------|-----------|-----------|
| 1   | Tb   | 0.250000                | 0.750000 | 0.750000 | -8.900040                     | 0.000000 | 0.000000  | -9.053000                   | 0.003000  | 0.000000  |
| 2   | Tb   | 0.750000                | 0.250000 | 0.250000 | -8.900040                     | 0.000000 | 0.000000  | -9.053000                   | -0.003000 | 0.000000  |
| 3   | Mn   | 0.000000                | 0.250000 | 0.750000 | 0.849970                      | 0.000000 | -1.269990 | 1.472000                    | -0.001000 | -2.084000 |
| 4   | Mn   | 0.500000                | 0.750000 | 0.250000 | 0.849970                      | 0.000000 | 1.269990  | 1.471000                    | -0.000000 | 2.084000  |
| 5   | Mn   | 0.000000                | 0.750000 | 0.250000 | 0.849970                      | 0.000000 | -1.269990 | 1.471000                    | 0.001000  | -2.084000 |
| 6   | Mn   | 0.500000                | 0.250000 | 0.750000 | 0.849970                      | 0.000000 | 1.269990  | 1.471000                    | 0.000000  | 2.084000  |
| 7   | Si   | 0.125000                | 0.250000 | 0.250000 | 0.000000                      | 0.000000 | 0.000000  | 0.057000                    | -0.001000 | 0.080000  |
| 8   | Si   | 0.625000                | 0.750000 | 0.750000 | 0.000000                      | 0.000000 | 0.000000  | 0.058000                    | 0.002000  | -0.080000 |
| 9   | Si   | 0.875000                | 0.750000 | 0.750000 | 0.000000                      | 0.000000 | 0.000000  | 0.058000                    | 0.001000  | 0.080000  |
| 10  | Si   | 0.375000                | 0.250000 | 0.250000 | 0.000000                      | 0.000000 | 0.000000  | 0.058000                    | -0.002000 | -0.080000 |

FIG. 29. First-principles calculation results of 2.57 TbMn<sub>2</sub>Si<sub>2</sub>. The band structure is shown in the left panel, and the Fermi-level-dependent AHC is plotted in the right panel. In both plots, the Fermi level is set to 0 eV.

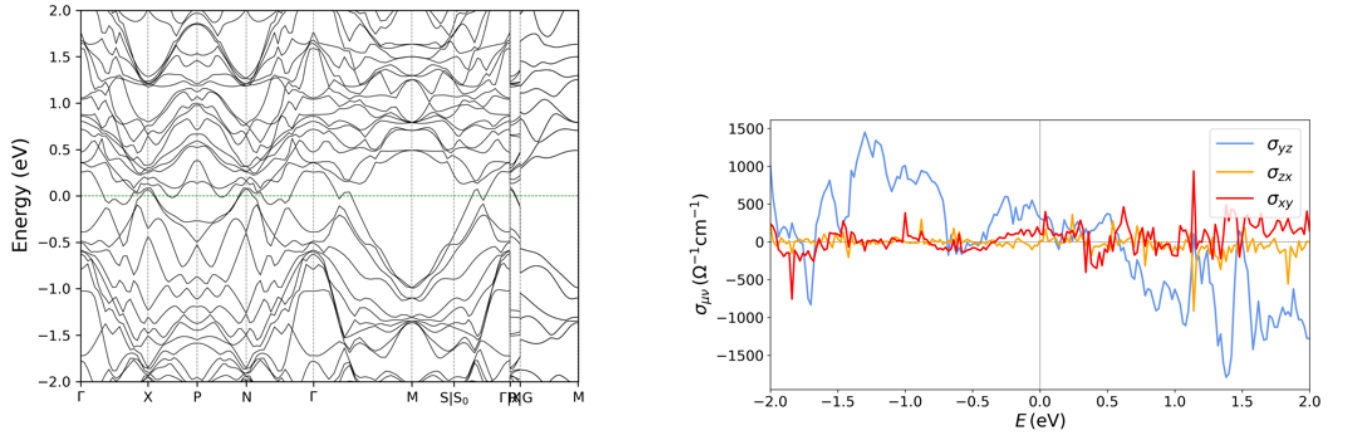



**2.70 GdMg** crystallizes in type III MSG 15.89, which hosts only SNLs. The symmetry-adapted AHC tensor of the MSG is  $(\sigma_{yz}, \sigma_{zx}, 0)$ . Based on the first-principles calculation results, the comparison between the experimental and calculated magnetic moments is provided in Table SII32. The band structure is shown in the left panel of Fig. 30, and the Fermi-level-dependent AHC is plotted in the right panel.

TABLE SII32. The comparison between the experimental and calculated magnetic moments for 2.70 GdMg. The five columns contain the atom index in the structure file, the atom species, the fractional coordinates, the experimental magnetic moments, and the calculated magnetic moments. The lattice vectors are  $\vec{a}_1 = (2.69549, -2.69549, 0.0)$ ,  $\vec{a}_2 = (2.69549, 2.69549, 0.0)$ ,  $\vec{a}_3 = (0.0, 0.0, 7.624)$ .

| No. | Atom | Coordinates(fractional) |          |          | Experimental magnetic moments |           |          | Calculated magnetic moments |           |          |
|-----|------|-------------------------|----------|----------|-------------------------------|-----------|----------|-----------------------------|-----------|----------|
| 1   | Gd   | 0.000000                | 0.000000 | 0.000000 | 4.031000                      | 5.162030  | 2.799990 | 4.475000                    | 5.739000  | 3.108000 |
| 2   | Gd   | 0.000000                | 0.000000 | 0.500000 | 4.031000                      | -5.162030 | 2.799990 | 4.475000                    | -5.739000 | 3.108000 |
| 3   | Mg   | 0.500000                | 0.500000 | 0.250000 | 0.000000                      | 0.000000  | 0.000000 | 0.006000                    | 0.000000  | 0.001000 |
| 4   | Mg   | 0.500000                | 0.500000 | 0.750000 | 0.000000                      | 0.000000  | 0.000000 | 0.003000                    | -0.000000 | 0.006000 |

FIG. 30. First-principles calculation results of 2.70 GdMg. The band structure is shown in the left panel, and the Fermi-level-dependent AHC is plotted in the right panel. In both plots, the Fermi level is set to 0 eV.

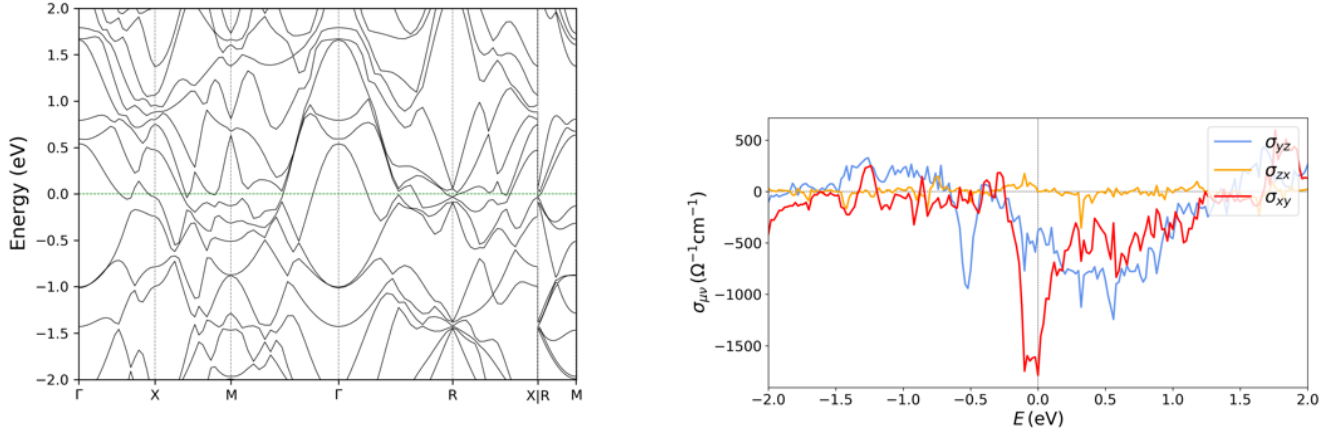

**0.1 LaMnO<sub>3</sub>** crystallizes in type III MSG 62.448, which hosts both SNLs and FNSs. The symmetry-adapted AHC tensor of the MSG is  $(0, \sigma_{zx}, 0)$ . Based on the first-principles calculation results, the comparison between the experimental and calculated magnetic moments is provided in Table SII33. The band structure is shown in the left panel of Fig. 31, and the Fermi-level-dependent AHC is plotted in the right panel.

TABLE SII33. The comparison between the experimental and calculated magnetic moments for 0.1 LaMnO<sub>3</sub>. The five columns contain the atom index in the structure file, the atom species, the fractional coordinates, the experimental magnetic moments, and the calculated magnetic moments. The lattice vectors are  $\vec{a}_1 = (5.7461, 0.0, 0.0)$ ,  $\vec{a}_2 = (0.0, 7.6637, 0.0)$ ,  $\vec{a}_3 = (0.0, 0.0, 5.5333)$ .

| No. | Atom | Coordinates(fractional) |          |          | Experimental magnetic moments |          |          | Calculated magnetic moments |           |           |
|-----|------|-------------------------|----------|----------|-------------------------------|----------|----------|-----------------------------|-----------|-----------|
| 1   | La   | 0.551300                | 0.250000 | 0.490500 | 0.000000                      | 0.000000 | 0.000000 | 0.000000                    | -0.000000 | -0.000000 |
| 2   | La   | 0.448700                | 0.750000 | 0.509500 | 0.000000                      | 0.000000 | 0.000000 | 0.000000                    | 0.000000  | 0.000000  |
| 3   | La   | 0.051300                | 0.250000 | 0.009500 | 0.000000                      | 0.000000 | 0.000000 | -0.000000                   | -0.000000 | -0.000000 |
| 4   | La   | 0.948700                | 0.750000 | 0.990500 | 0.000000                      | 0.000000 | 0.000000 | -0.000000                   | 0.000000  | 0.000000  |
| 5   | Mn   | 0.000000                | 0.000000 | 0.500000 | 3.870000                      | 0.000000 | 0.000000 | 4.321000                    | -0.000000 | -0.000000 |
| 6   | Mn   | 0.000000                | 0.500000 | 0.500000 | -3.870000                     | 0.000000 | 0.000000 | -4.322000                   | -0.000000 | 0.000000  |
| 7   | Mn   | 0.500000                | 0.500000 | 0.000000 | -3.870000                     | 0.000000 | 0.000000 | -4.321000                   | -0.000000 | -0.000000 |
| 8   | Mn   | 0.500000                | 0.000000 | 0.000000 | 3.870000                      | 0.000000 | 0.000000 | 4.322000                    | -0.000000 | 0.000000  |
| 9   | O    | 0.984930                | 0.250000 | 0.577700 | 0.000000                      | 0.000000 | 0.000000 | 0.001000                    | 0.001000  | 0.000000  |
| 10  | O    | 0.015070                | 0.750000 | 0.422300 | 0.000000                      | 0.000000 | 0.000000 | 0.001000                    | 0.002000  | -0.000000 |
| 11  | O    | 0.484930                | 0.250000 | 0.922300 | 0.000000                      | 0.000000 | 0.000000 | -0.000000                   | 0.000000  | 0.000000  |
| 12  | O    | 0.515070                | 0.750000 | 0.077700 | 0.000000                      | 0.000000 | 0.000000 | -0.001000                   | 0.000000  | -0.000000 |
| 13  | O    | 0.808500                | 0.040800 | 0.222700 | 0.000000                      | 0.000000 | 0.000000 | -0.111000                   | -0.000000 | 0.000000  |
| 14  | O    | 0.191500                | 0.540800 | 0.777300 | 0.000000                      | 0.000000 | 0.000000 | 0.111000                    | 0.000000  | 0.000000  |
| 15  | O    | 0.191500                | 0.959200 | 0.777300 | 0.000000                      | 0.000000 | 0.000000 | -0.111000                   | 0.000000  | -0.000000 |
| 16  | O    | 0.808500                | 0.459200 | 0.222700 | 0.000000                      | 0.000000 | 0.000000 | 0.111000                    | -0.000000 | -0.000000 |
| 17  | O    | 0.308500                | 0.459200 | 0.277300 | 0.000000                      | 0.000000 | 0.000000 | 0.111000                    | -0.000000 | 0.000000  |
| 18  | O    | 0.691500                | 0.959200 | 0.722700 | 0.000000                      | 0.000000 | 0.000000 | -0.111000                   | 0.000000  | 0.000000  |
| 19  | O    | 0.691500                | 0.540800 | 0.722700 | 0.000000                      | 0.000000 | 0.000000 | 0.111000                    | -0.000000 | -0.000000 |
| 20  | O    | 0.308500                | 0.040800 | 0.277300 | 0.000000                      | 0.000000 | 0.000000 | -0.111000                   | -0.000000 | -0.000000 |

FIG. 31. First-principles calculation results of 0.1 LaMnO<sub>3</sub>. The band structure is shown in the left panel, and the Fermi-level-dependent AHC is plotted in the right panel. In both plots, the Fermi level is set to 0 eV.

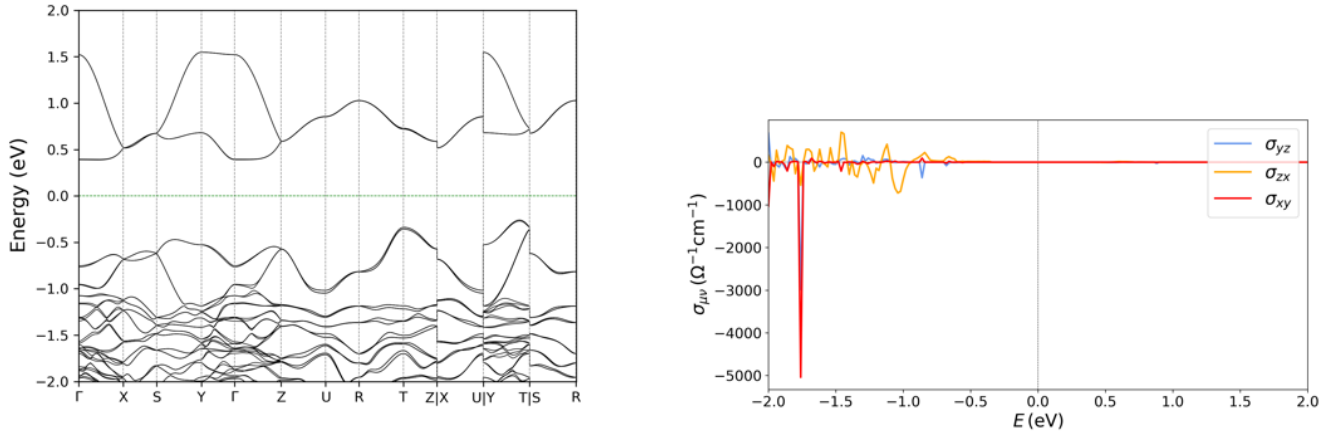

**0.106 DyVO<sub>3</sub>** crystallizes in type III MSG 11.54, which hosts only FNSs. The symmetry-adapted AHC tensor of the MSG is  $(\sigma_{yz}, \sigma_{zx}, 0)$ . Based on the first-principles calculation results, the comparison between the experimental and calculated magnetic moments is provided in Table SII34. The band structure is shown in the left panel of Fig. 32, and the Fermi-level-dependent AHC is plotted in the right panel.

TABLE SII34. The comparison between the experimental and calculated magnetic moments for 0.106 DyVO<sub>3</sub>. The five columns contain the atom index in the structure file, the atom species, the fractional coordinates, the experimental magnetic moments, and the calculated magnetic moments. The lattice vectors are  $\vec{a}_1 = (5.292, 0.0, 0.0)$ ,  $\vec{a}_2 = (0.0, 7.586, 0.0)$ ,  $\vec{a}_3 = (0.0, 0.0, 5.598)$ .

| No. | Atom | Coordinates(fractional) |          |          | Experimental magnetic moments |           |           | Calculated magnetic moments |           |           |
|-----|------|-------------------------|----------|----------|-------------------------------|-----------|-----------|-----------------------------|-----------|-----------|
| 1   | Dy   | 0.981400                | 0.250000 | 0.933000 | 4.800000                      | 0.000000  | -6.099970 | 4.882000                    | -0.001000 | -6.236000 |
| 2   | Dy   | 0.018600                | 0.750000 | 0.067000 | 4.800000                      | 0.000000  | -6.099970 | 4.883000                    | 0.001000  | -6.237000 |
| 3   | Dy   | 0.518600                | 0.250000 | 0.433000 | -4.800000                     | 0.000000  | -6.099970 | -4.849000                   | 0.002000  | -6.203000 |
| 4   | Dy   | 0.481400                | 0.750000 | 0.567000 | -4.800000                     | 0.000000  | -6.099970 | -4.848000                   | -0.002000 | -6.202000 |
| 5   | V    | 0.500000                | 0.000000 | 0.000000 | 0.000000                      | -1.449990 | 0.000000  | -0.004000                   | -1.939000 | -0.061000 |
| 6   | V    | 0.500000                | 0.500000 | 0.000000 | 0.000000                      | 1.449990  | 0.000000  | -0.004000                   | 1.940000  | -0.059000 |
| 7   | V    | 0.000000                | 0.000000 | 0.500000 | 0.000000                      | 1.449990  | 0.000000  | 0.006000                    | 1.935000  | -0.061000 |
| 8   | V    | 0.000000                | 0.500000 | 0.500000 | 0.000000                      | -1.449990 | 0.000000  | 0.006000                    | -1.942000 | -0.058000 |
| 9   | O    | 0.392600                | 0.250000 | 0.038200 | 0.000000                      | 0.000000  | 0.000000  | -0.003000                   | -0.005000 | 0.227000  |
| 10  | O    | 0.607400                | 0.750000 | 0.961800 | 0.000000                      | 0.000000  | 0.000000  | -0.003000                   | 0.003000  | 0.227000  |
| 11  | O    | 0.107400                | 0.250000 | 0.538200 | 0.000000                      | 0.000000  | 0.000000  | 0.003000                    | 0.004000  | 0.223000  |
| 12  | O    | 0.892600                | 0.750000 | 0.461800 | 0.000000                      | 0.000000  | 0.000000  | 0.003000                    | -0.002000 | 0.222000  |
| 13  | O    | 0.192300                | 0.554900 | 0.803100 | 0.000000                      | 0.000000  | 0.000000  | -0.072000                   | 0.015000  | 0.236000  |
| 14  | O    | 0.807700                | 0.445100 | 0.196900 | 0.000000                      | 0.000000  | 0.000000  | -0.071000                   | 0.014000  | 0.237000  |
| 15  | O    | 0.807700                | 0.054900 | 0.196900 | 0.000000                      | 0.000000  | 0.000000  | -0.072000                   | -0.014000 | 0.238000  |
| 16  | O    | 0.192300                | 0.945100 | 0.803100 | 0.000000                      | 0.000000  | 0.000000  | -0.071000                   | -0.014000 | 0.239000  |
| 17  | O    | 0.692308                | 0.445100 | 0.696900 | 0.000000                      | 0.000000  | 0.000000  | 0.067000                    | -0.015000 | 0.238000  |
| 18  | O    | 0.307692                | 0.554900 | 0.303100 | 0.000000                      | 0.000000  | 0.000000  | 0.069000                    | -0.015000 | 0.238000  |
| 19  | O    | 0.307692                | 0.945100 | 0.303100 | 0.000000                      | 0.000000  | 0.000000  | 0.067000                    | 0.015000  | 0.240000  |
| 20  | O    | 0.692308                | 0.054900 | 0.696900 | 0.000000                      | 0.000000  | 0.000000  | 0.069000                    | 0.014000  | 0.240000  |

FIG. 32. First-principles calculation results of 0.106 DyVO<sub>3</sub>. The band structure is shown in the left panel, and the Fermi-level-dependent AHC is plotted in the right panel. In both plots, the Fermi level is set to 0 eV.

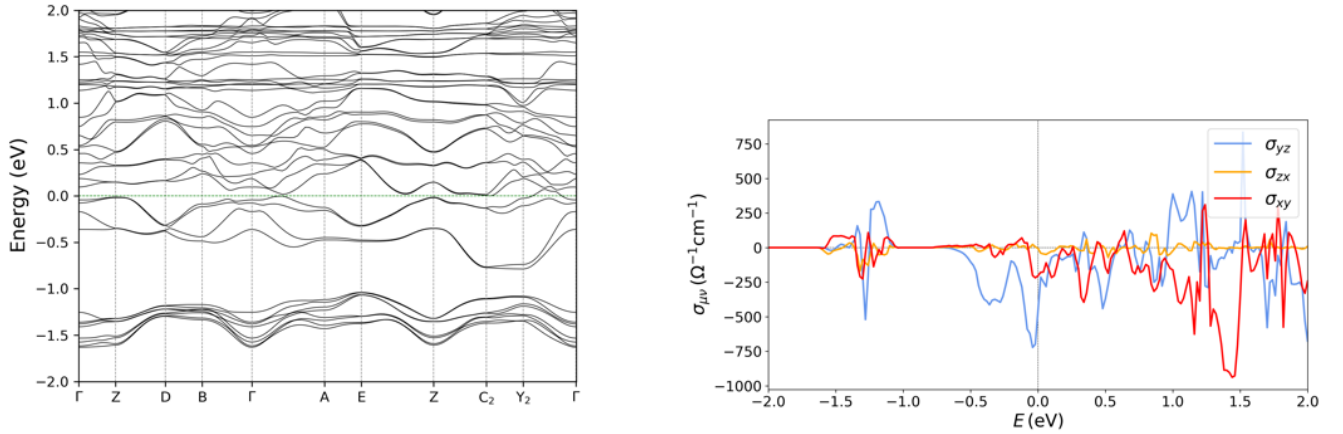

**0.174 Pr<sub>3</sub>Ru<sub>4</sub>Al<sub>12</sub>** crystallizes in type III MSG 15.89, which hosts only SNLs. The symmetry-adapted AHC tensor of the MSG is  $(\sigma_{yz}, \sigma_{zx}, 0)$ . Based on the first-principles calculation results, the comparison between the experimental and calculated magnetic moments is provided in Table SII35. The band structure is shown in the left panel of Fig. 33, and the Fermi-level-dependent AHC is plotted in the right panel.

TABLE SII35. The comparison between the experimental and calculated magnetic moments for 0.174 Pr<sub>3</sub>Ru<sub>4</sub>Al<sub>12</sub>. The five columns contain the atom index in the structure file, the atom species, the fractional coordinates, the experimental magnetic moments, and the calculated magnetic moments. The lattice vectors are  $\vec{a}_1 = (4.42935, -7.67186, 0.0)$ ,  $\vec{a}_2 = (4.42935, 7.67186, 0.0)$ ,  $\vec{a}_3 = (0.0, 0.0, 9.6244)$ .

| No. | Atom | Coordinates(fractional) |          |          | Experimental magnetic moments |          |          | Calculated magnetic moments |           |           |
|-----|------|-------------------------|----------|----------|-------------------------------|----------|----------|-----------------------------|-----------|-----------|
| 1   | Pr   | 0.811500                | 0.188500 | 0.250000 | 0.000000                      | 0.000000 | 3.200020 | -0.000000                   | 0.001000  | 2.880000  |
| 2   | Pr   | 0.188500                | 0.811500 | 0.750000 | 0.000000                      | 0.000000 | 3.200020 | 0.002000                    | 0.001000  | 2.878000  |
| 3   | Pr   | 0.188500                | 0.377000 | 0.750000 | 0.499990                      | 0.000000 | 1.299970 | 0.621000                    | 0.006000  | 1.603000  |
| 4   | Pr   | 0.811500                | 0.623000 | 0.250000 | 0.499990                      | 0.000000 | 1.299970 | 0.621000                    | 0.004000  | 1.604000  |
| 5   | Pr   | 0.623000                | 0.811500 | 0.750000 | 0.499990                      | 0.000000 | 1.299970 | 0.624000                    | -0.008000 | 1.606000  |
| 6   | Pr   | 0.377000                | 0.188500 | 0.250000 | 0.499990                      | 0.000000 | 1.299970 | 0.624000                    | -0.006000 | 1.605000  |
| 7   | Ru   | 0.000000                | 0.000000 | 0.000000 | 0.000000                      | 0.000000 | 0.000000 | -0.001000                   | 0.001000  | -0.062000 |
| 8   | Ru   | 0.000000                | 0.000000 | 0.500000 | 0.000000                      | 0.000000 | 0.000000 | -0.001000                   | -0.001000 | -0.060000 |
| 9   | Ru   | 0.000000                | 0.500000 | 0.500000 | 0.000000                      | 0.000000 | 0.000000 | 0.001000                    | -0.002000 | -0.153000 |
| 10  | Ru   | 0.500000                | 0.000000 | 0.000000 | 0.000000                      | 0.000000 | 0.000000 | 0.002000                    | 0.001000  | -0.153000 |
| 11  | Ru   | 0.000000                | 0.500000 | 0.000000 | 0.000000                      | 0.000000 | 0.000000 | -0.004000                   | 0.003000  | -0.150000 |
| 12  | Ru   | 0.500000                | 0.000000 | 0.500000 | 0.000000                      | 0.000000 | 0.000000 | -0.004000                   | -0.003000 | -0.151000 |
| 13  | Ru   | 0.500000                | 0.500000 | 0.000000 | 0.000000                      | 0.000000 | 0.000000 | -0.004000                   | 0.001000  | -0.040000 |
| 14  | Ru   | 0.500000                | 0.500000 | 0.500000 | 0.000000                      | 0.000000 | 0.000000 | -0.004000                   | -0.001000 | -0.038000 |
| 15  | Al   | 0.880600                | 0.440300 | 0.750000 | 0.000000                      | 0.000000 | 0.000000 | 0.000000                    | 0.000000  | 0.002000  |
| 16  | Al   | 0.119400                | 0.559700 | 0.250000 | 0.000000                      | 0.000000 | 0.000000 | -0.000000                   | -0.001000 | 0.002000  |
| 17  | Al   | 0.559700                | 0.119400 | 0.750000 | 0.000000                      | 0.000000 | 0.000000 | 0.000000                    | -0.000000 | 0.002000  |
| 18  | Al   | 0.440300                | 0.880600 | 0.250000 | 0.000000                      | 0.000000 | 0.000000 | -0.000000                   | 0.001000  | 0.002000  |
| 19  | Al   | 0.440300                | 0.559700 | 0.250000 | 0.000000                      | 0.000000 | 0.000000 | 0.000000                    | -0.000000 | -0.001000 |
| 20  | Al   | 0.559700                | 0.440300 | 0.750000 | 0.000000                      | 0.000000 | 0.000000 | -0.001000                   | -0.000000 | -0.001000 |
| 21  | Al   | 0.000000                | 0.000000 | 0.250000 | 0.000000                      | 0.000000 | 0.000000 | 0.000000                    | -0.000000 | 0.008000  |
| 22  | Al   | 0.000000                | 0.000000 | 0.750000 | 0.000000                      | 0.000000 | 0.000000 | 0.000000                    | -0.000000 | 0.008000  |
| 23  | Al   | 0.836900                | 0.673800 | 0.572000 | 0.000000                      | 0.000000 | 0.000000 | -0.000000                   | -0.000000 | -0.002000 |
| 24  | Al   | 0.163100                | 0.326200 | 0.428000 | 0.000000                      | 0.000000 | 0.000000 | -0.000000                   | -0.000000 | -0.002000 |
| 25  | Al   | 0.326200                | 0.163100 | 0.928000 | 0.000000                      | 0.000000 | 0.000000 | -0.000000                   | 0.000000  | -0.002000 |
| 26  | Al   | 0.673800                | 0.836900 | 0.072000 | 0.000000                      | 0.000000 | 0.000000 | -0.000000                   | 0.000000  | -0.002000 |
| 27  | Al   | 0.163100                | 0.326200 | 0.072000 | 0.000000                      | 0.000000 | 0.000000 | -0.000000                   | 0.000000  | -0.003000 |
| 28  | Al   | 0.836900                | 0.673800 | 0.928000 | 0.000000                      | 0.000000 | 0.000000 | -0.000000                   | -0.000000 | -0.002000 |
| 29  | Al   | 0.673800                | 0.836900 | 0.428000 | 0.000000                      | 0.000000 | 0.000000 | -0.000000                   | -0.000000 | -0.002000 |
| 30  | Al   | 0.326200                | 0.163100 | 0.572000 | 0.000000                      | 0.000000 | 0.000000 | -0.000000                   | 0.000000  | -0.002000 |
| 31  | Al   | 0.836900                | 0.163100 | 0.572000 | 0.000000                      | 0.000000 | 0.000000 | -0.000000                   | 0.000000  | 0.001000  |
| 32  | Al   | 0.163100                | 0.836900 | 0.428000 | 0.000000                      | 0.000000 | 0.000000 | 0.000000                    | 0.000000  | 0.001000  |
| 33  | Al   | 0.836900                | 0.163100 | 0.928000 | 0.000000                      | 0.000000 | 0.000000 | -0.000000                   | 0.000000  | 0.001000  |
| 34  | Al   | 0.163100                | 0.836900 | 0.072000 | 0.000000                      | 0.000000 | 0.000000 | -0.000000                   | 0.000000  | 0.001000  |
| 35  | Al   | 0.666667                | 0.333333 | 0.515000 | 0.000000                      | 0.000000 | 0.000000 | 0.000000                    | -0.000000 | 0.008000  |
| 36  | Al   | 0.333333                | 0.666667 | 0.485000 | 0.000000                      | 0.000000 | 0.000000 | 0.000000                    | -0.000000 | 0.008000  |
| 37  | Al   | 0.666667                | 0.333333 | 0.985000 | 0.000000                      | 0.000000 | 0.000000 | 0.000000                    | 0.000000  | 0.008000  |
| 38  | Al   | 0.333333                | 0.666667 | 0.015000 | 0.000000                      | 0.000000 | 0.000000 | 0.000000                    | 0.000000  | 0.008000  |

FIG. 33. First-principles calculation results of  $0.174 \text{ Pr}_3\text{Ru}_4\text{Al}_{12}$ . The band structure is shown in the left panel, and the Fermi-level-dependent AHC is plotted in the right panel. In both plots, the Fermi level is set to 0 eV.

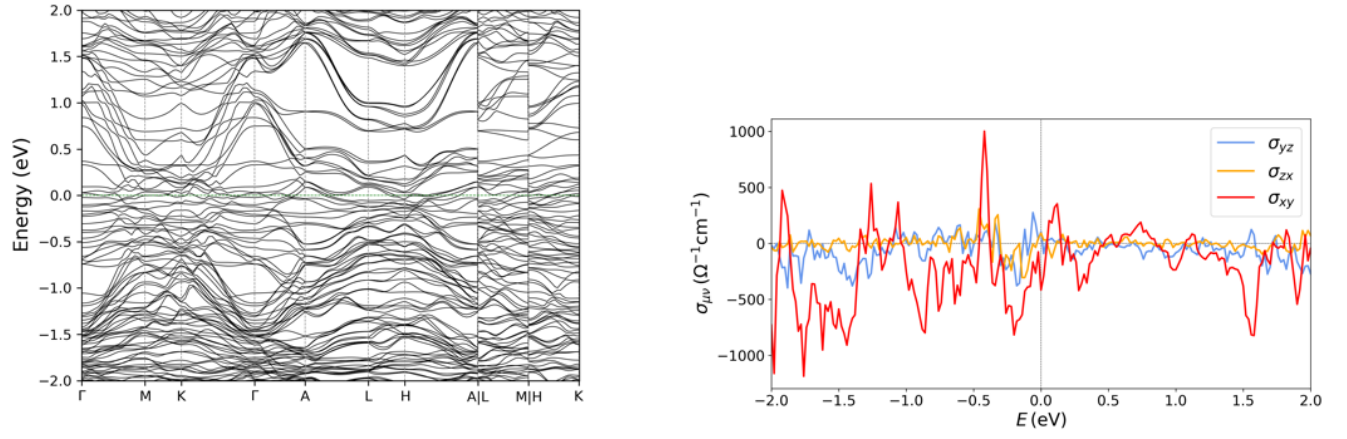

**0.279 Mn<sub>3</sub>As** crystallizes in type III MSG 63.463, which hosts only FNSs. The symmetry-adapted AHC tensor of the MSG is  $(\sigma_{yz}, 0, 0)$ . Based on the first-principles calculation results, the comparison between the experimental and calculated magnetic moments is provided in Table SII36. The band structure is shown in the left panel of Fig. 34, and the Fermi-level-dependent AHC is plotted in the right panel.

TABLE SII36. The comparison between the experimental and calculated magnetic moments for 0.279 Mn<sub>3</sub>As. The five columns contain the atom index in the structure file, the atom species, the fractional coordinates, the experimental magnetic moments, and the calculated magnetic moments. The lattice vectors are  $\vec{a}_1 = (2.8325, -4.906035, 0.0)$ ,  $\vec{a}_2 = (2.8325, 4.906035, 0.0)$ ,  $\vec{a}_3 = (0.0, 0.0, 4.531)$ .

| No. | Atom | Coordinates(fractional) |          |          | Experimental magnetic moments |           |          | Calculated magnetic moments |           |           |
|-----|------|-------------------------|----------|----------|-------------------------------|-----------|----------|-----------------------------|-----------|-----------|
| 1   | Mn   | 0.838800                | 0.677600 | 0.250000 | 1.499980                      | 2.598040  | 0.000000 | 2.155000                    | 3.735000  | -0.002000 |
| 2   | Mn   | 0.677600                | 0.838800 | 0.750000 | 1.499980                      | -2.598040 | 0.000000 | 2.150000                    | -3.722000 | 0.003000  |
| 3   | Mn   | 0.161200                | 0.322400 | 0.750000 | 1.499980                      | 2.598040  | 0.000000 | 2.155000                    | 3.736000  | 0.002000  |
| 4   | Mn   | 0.322400                | 0.161200 | 0.250000 | 1.499980                      | -2.598040 | 0.000000 | 2.150000                    | -3.722000 | -0.003000 |
| 5   | Mn   | 0.838800                | 0.161200 | 0.250000 | -3.000010                     | 0.000000  | 0.000000 | -4.306000                   | 0.003000  | -0.002000 |
| 6   | Mn   | 0.161200                | 0.838800 | 0.750000 | -3.000010                     | 0.000000  | 0.000000 | -4.305000                   | 0.003000  | 0.002000  |
| 7   | As   | 0.333333                | 0.666667 | 0.250000 | 0.000000                      | 0.000000  | 0.000000 | 0.000000                    | 0.000000  | -0.004000 |
| 8   | As   | 0.666667                | 0.333333 | 0.750000 | 0.000000                      | 0.000000  | 0.000000 | -0.000000                   | 0.000000  | 0.004000  |

FIG. 34. First-principles calculation results of 0.279 Mn<sub>3</sub>As. The band structure is shown in the left panel, and the Fermi-level-dependent AHC is plotted in the right panel. In both plots, the Fermi level is set to 0 eV.

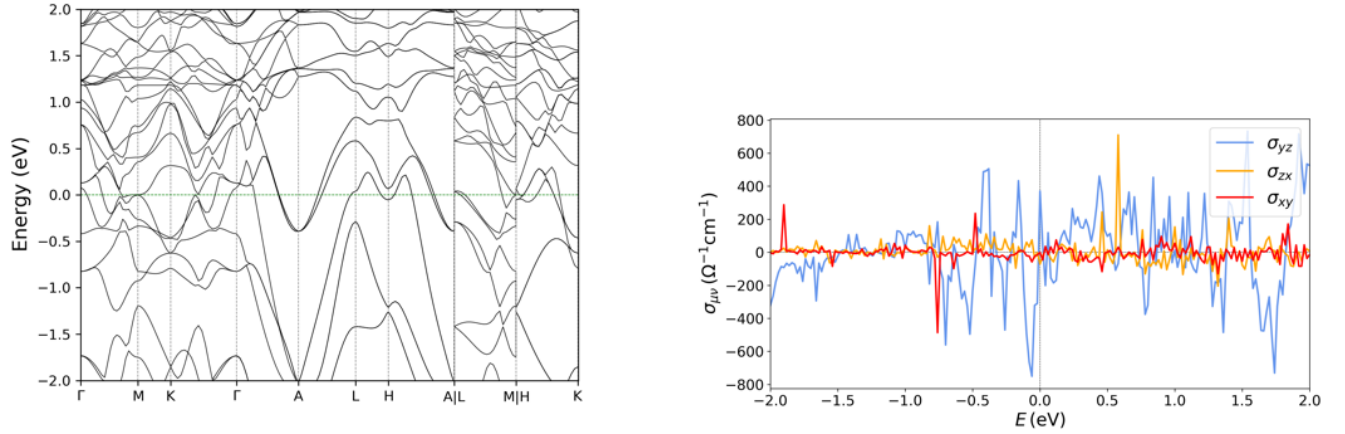

**0.280 Mn<sub>3</sub>As** crystallizes in type III MSG 63.464, which hosts only FNSs. The symmetry-adapted AHC tensor of the MSG is  $(0, \sigma_{zx}, 0)$ . Based on the first-principles calculation results, the comparison between the experimental and calculated magnetic moments is provided in Table SII37. The band structure is shown in the left panel of Fig. 35, and the Fermi-level-dependent AHC is plotted in the right panel.

TABLE SII37. The comparison between the experimental and calculated magnetic moments for 0.280 Mn<sub>3</sub>As. The five columns contain the atom index in the structure file, the atom species, the fractional coordinates, the experimental magnetic moments, and the calculated magnetic moments. The lattice vectors are  $\vec{a}_1 = (2.8325, -4.906035, 0.0)$ ,  $\vec{a}_2 = (2.8325, 4.906035, 0.0)$ ,  $\vec{a}_3 = (0.0, 0.0, 4.531)$ .

| No. | Atom | Coordinates(fractional) |          |          | Experimental magnetic moments |           |          | Calculated magnetic moments |           |           |
|-----|------|-------------------------|----------|----------|-------------------------------|-----------|----------|-----------------------------|-----------|-----------|
| 1   | Mn   | 0.677600                | 0.838800 | 0.250000 | 4.499990                      | 2.598040  | 0.000000 | 4.260000                    | 2.462000  | 0.001000  |
| 2   | Mn   | 0.161200                | 0.322400 | 0.250000 | -4.499990                     | 2.598040  | 0.000000 | -4.264000                   | 2.459000  | -0.000000 |
| 3   | Mn   | 0.322400                | 0.161200 | 0.750000 | 4.499990                      | 2.598040  | 0.000000 | 4.261000                    | 2.462000  | -0.001000 |
| 4   | Mn   | 0.838800                | 0.677600 | 0.750000 | -4.499990                     | 2.598040  | 0.000000 | -4.263000                   | 2.459000  | 0.000000  |
| 5   | Mn   | 0.161200                | 0.838800 | 0.250000 | 0.000000                      | -5.195980 | 0.000000 | -0.004000                   | -4.921000 | 0.000000  |
| 6   | Mn   | 0.838800                | 0.161200 | 0.750000 | 0.000000                      | -5.195980 | 0.000000 | -0.004000                   | -4.921000 | -0.000000 |
| 7   | As   | 0.666667                | 0.333333 | 0.250000 | 0.000000                      | 0.000000  | 0.000000 | 0.001000                    | -0.000000 | 0.000000  |
| 8   | As   | 0.333333                | 0.666667 | 0.750000 | 0.000000                      | 0.000000  | 0.000000 | 0.001000                    | 0.000000  | 0.000000  |

FIG. 35. First-principles calculation results of 0.280 Mn<sub>3</sub>As. The band structure is shown in the left panel, and the Fermi-level-dependent AHC is plotted in the right panel. In both plots, the Fermi level is set to 0 eV.

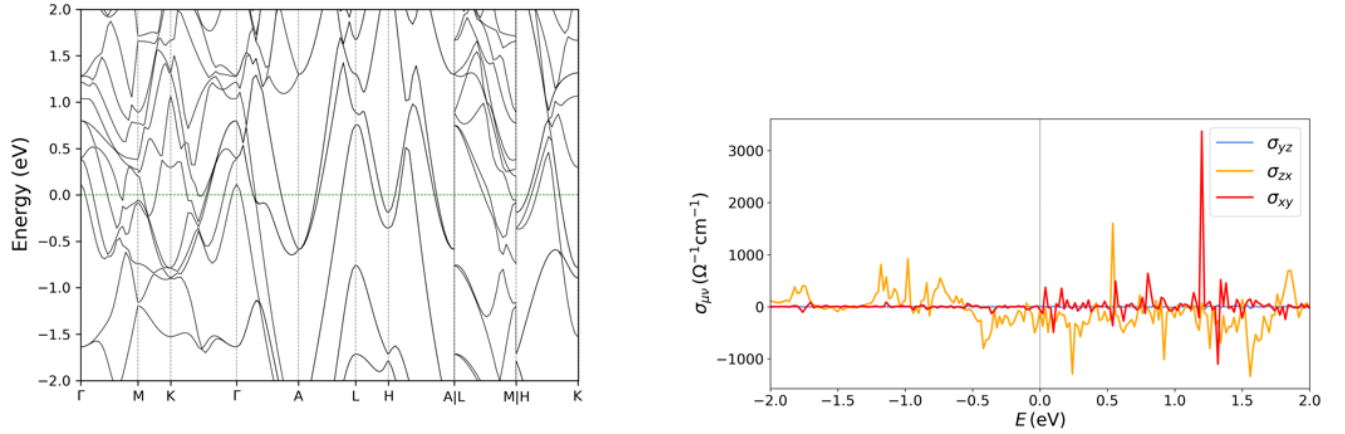

**0.288 NdMnO<sub>3</sub>** crystallizes in type III MSG 62.448, which hosts both SNLs and FNSs. The symmetry-adapted AHC tensor of the MSG is  $(0, \sigma_{zx}, 0)$ . Based on the first-principles calculation results, the comparison between the experimental and calculated magnetic moments is provided in Table SII38. The band structure is shown in the left panel of Fig. 36, and the Fermi-level-dependent AHC is plotted in the right panel.

TABLE SII38. The comparison between the experimental and calculated magnetic moments for 0.288 NdMnO<sub>3</sub>. The five columns contain the atom index in the structure file, the atom species, the fractional coordinates, the experimental magnetic moments, and the calculated magnetic moments. The lattice vectors are  $\vec{a}_1 = (5.7119, 0.0, 0.0)$ ,  $\vec{a}_2 = (0.0, 7.589, 0.0)$ ,  $\vec{a}_3 = (0.0, 0.0, 5.4119)$ .

| No. | Atom | Coordinates(fractional) |          |          | Experimental magnetic moments |           |          | Calculated magnetic moments |           |           |
|-----|------|-------------------------|----------|----------|-------------------------------|-----------|----------|-----------------------------|-----------|-----------|
| 1   | Nd   | 0.559700                | 0.250000 | 0.490900 | 0.000000                      | 0.000000  | 0.000000 | 0.000000                    | 0.260000  | 0.000000  |
| 2   | Nd   | 0.440300                | 0.750000 | 0.509100 | 0.000000                      | 0.000000  | 0.000000 | 0.000000                    | 0.264000  | -0.000000 |
| 3   | Nd   | 0.059700                | 0.250000 | 0.009100 | 0.000000                      | 0.000000  | 0.000000 | -0.000000                   | 0.240000  | 0.000000  |
| 4   | Nd   | 0.940300                | 0.750000 | 0.990900 | 0.000000                      | 0.000000  | 0.000000 | -0.000000                   | 0.244000  | -0.000000 |
| 5   | Mn   | 0.000000                | 0.000000 | 0.500000 | 2.799970                      | -1.079990 | 0.000000 | 3.721000                    | -1.436000 | -0.000000 |
| 6   | Mn   | 0.000000                | 0.500000 | 0.500000 | -2.799970                     | -1.079990 | 0.000000 | -3.721000                   | -1.437000 | 0.000000  |
| 7   | Mn   | 0.500000                | 0.500000 | 0.000000 | -2.799970                     | -1.079990 | 0.000000 | -3.721000                   | -1.437000 | -0.000000 |
| 8   | Mn   | 0.500000                | 0.000000 | 0.000000 | 2.799970                      | -1.079990 | 0.000000 | 3.722000                    | -1.437000 | 0.000000  |
| 9   | O    | 0.983700                | 0.250000 | 0.581700 | 0.000000                      | 0.000000  | 0.000000 | 0.000000                    | 0.019000  | 0.001000  |
| 10  | O    | 0.016300                | 0.750000 | 0.418300 | 0.000000                      | 0.000000  | 0.000000 | 0.000000                    | 0.019000  | -0.001000 |
| 11  | O    | 0.483700                | 0.250000 | 0.918300 | 0.000000                      | 0.000000  | 0.000000 | 0.000000                    | 0.019000  | 0.001000  |
| 12  | O    | 0.516300                | 0.750000 | 0.081700 | 0.000000                      | 0.000000  | 0.000000 | -0.000000                   | 0.019000  | -0.001000 |
| 13  | O    | 0.810600                | 0.040500 | 0.210800 | 0.000000                      | 0.000000  | 0.000000 | -0.027000                   | 0.010000  | 0.000000  |
| 14  | O    | 0.189400                | 0.540500 | 0.789200 | 0.000000                      | 0.000000  | 0.000000 | 0.028000                    | 0.010000  | 0.000000  |
| 15  | O    | 0.189400                | 0.959500 | 0.789200 | 0.000000                      | 0.000000  | 0.000000 | -0.028000                   | 0.010000  | -0.000000 |
| 16  | O    | 0.810600                | 0.459500 | 0.210800 | 0.000000                      | 0.000000  | 0.000000 | 0.028000                    | 0.010000  | 0.000000  |
| 17  | O    | 0.310600                | 0.459500 | 0.289200 | 0.000000                      | 0.000000  | 0.000000 | 0.027000                    | 0.010000  | 0.001000  |
| 18  | O    | 0.689400                | 0.959500 | 0.710800 | 0.000000                      | 0.000000  | 0.000000 | -0.028000                   | 0.009000  | -0.000000 |
| 19  | O    | 0.689400                | 0.540500 | 0.710800 | 0.000000                      | 0.000000  | 0.000000 | 0.028000                    | 0.010000  | 0.000000  |
| 20  | O    | 0.310600                | 0.040500 | 0.289200 | 0.000000                      | 0.000000  | 0.000000 | -0.027000                   | 0.009000  | -0.001000 |

FIG. 36. First-principles calculation results of 0.288 NdMnO<sub>3</sub>. The band structure is shown in the left panel, and the Fermi-level-dependent AHC is plotted in the right panel. In both plots, the Fermi level is set to 0 eV.

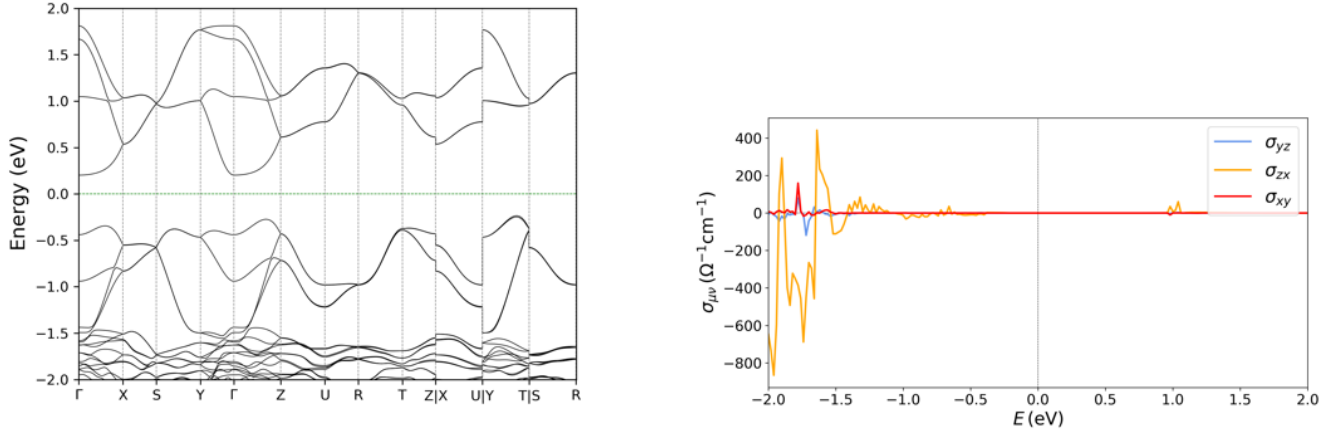



**0.289 NdMnO<sub>3</sub>** crystallizes in type III MSG 62.448, which hosts both SNLs and FNSs. The symmetry-adapted AHC tensor of the MSG is  $(0, \sigma_{zx}, 0)$ . Based on the first-principles calculation results, the comparison between the experimental and calculated magnetic moments is provided in Table SII39. The band structure is shown in the left panel of Fig. 37, and the Fermi-level-dependent AHC is plotted in the right panel.

TABLE SII39. The comparison between the experimental and calculated magnetic moments for 0.289 NdMnO<sub>3</sub>. The five columns contain the atom index in the structure file, the atom species, the fractional coordinates, the experimental magnetic moments, and the calculated magnetic moments. The lattice vectors are  $\vec{a}_1 = (5.7119, 0.0, 0.0)$ ,  $\vec{a}_2 = (0.0, 7.589, 0.0)$ ,  $\vec{a}_3 = (0.0, 0.0, 5.4119)$ .

| No. | Atom | Coordinates(fractional) |          |          | Experimental magnetic moments |           |          | Calculated magnetic moments |           |           |
|-----|------|-------------------------|----------|----------|-------------------------------|-----------|----------|-----------------------------|-----------|-----------|
| 1   | Nd   | 0.559700                | 0.250000 | 0.490900 | 0.000000                      | -1.199970 | 0.000000 | 0.000000                    | -1.549000 | -0.000000 |
| 2   | Nd   | 0.440300                | 0.750000 | 0.509100 | 0.000000                      | -1.199970 | 0.000000 | 0.000000                    | -1.547000 | -0.000000 |
| 3   | Nd   | 0.059700                | 0.250000 | 0.009100 | 0.000000                      | -1.199970 | 0.000000 | -0.000000                   | -1.548000 | 0.000000  |
| 4   | Nd   | 0.940300                | 0.750000 | 0.990900 | 0.000000                      | -1.199970 | 0.000000 | -0.000000                   | -1.547000 | -0.000000 |
| 5   | Mn   | 0.000000                | 0.000000 | 0.500000 | 2.799970                      | -1.599990 | 0.000000 | 3.548000                    | -2.029000 | -0.000000 |
| 6   | Mn   | 0.000000                | 0.500000 | 0.500000 | -2.799970                     | -1.599990 | 0.000000 | -3.548000                   | -2.029000 | 0.000000  |
| 7   | Mn   | 0.500000                | 0.500000 | 0.000000 | -2.799970                     | -1.599990 | 0.000000 | -3.547000                   | -2.029000 | -0.000000 |
| 8   | Mn   | 0.500000                | 0.000000 | 0.000000 | 2.799970                      | -1.599990 | 0.000000 | 3.548000                    | -2.029000 | 0.000000  |
| 9   | O    | 0.983700                | 0.250000 | 0.581700 | 0.000000                      | 0.000000  | 0.000000 | -0.000000                   | 0.039000  | 0.002000  |
| 10  | O    | 0.016300                | 0.750000 | 0.418300 | 0.000000                      | 0.000000  | 0.000000 | 0.000000                    | 0.038000  | -0.002000 |
| 11  | O    | 0.483700                | 0.250000 | 0.918300 | 0.000000                      | 0.000000  | 0.000000 | 0.000000                    | 0.039000  | 0.002000  |
| 12  | O    | 0.516300                | 0.750000 | 0.081700 | 0.000000                      | 0.000000  | 0.000000 | 0.000000                    | 0.038000  | -0.002000 |
| 13  | O    | 0.810600                | 0.040500 | 0.210800 | 0.000000                      | 0.000000  | 0.000000 | -0.047000                   | 0.024000  | 0.001000  |
| 14  | O    | 0.189400                | 0.540500 | 0.789200 | 0.000000                      | 0.000000  | 0.000000 | 0.046000                    | 0.024000  | -0.000000 |
| 15  | O    | 0.189400                | 0.959500 | 0.789200 | 0.000000                      | 0.000000  | 0.000000 | -0.046000                   | 0.024000  | -0.000000 |
| 16  | O    | 0.810600                | 0.459500 | 0.210800 | 0.000000                      | 0.000000  | 0.000000 | 0.047000                    | 0.024000  | -0.000000 |
| 17  | O    | 0.310600                | 0.459500 | 0.289200 | 0.000000                      | 0.000000  | 0.000000 | 0.046000                    | 0.024000  | 0.001000  |
| 18  | O    | 0.689400                | 0.959500 | 0.710800 | 0.000000                      | 0.000000  | 0.000000 | -0.046000                   | 0.024000  | -0.000000 |
| 19  | O    | 0.689400                | 0.540500 | 0.710800 | 0.000000                      | 0.000000  | 0.000000 | 0.046000                    | 0.024000  | -0.000000 |
| 20  | O    | 0.310600                | 0.040500 | 0.289200 | 0.000000                      | 0.000000  | 0.000000 | -0.047000                   | 0.024000  | -0.000000 |

FIG. 37. First-principles calculation results of 0.289 NdMnO<sub>3</sub>. The band structure is shown in the left panel, and the Fermi-level-dependent AHC is plotted in the right panel. In both plots, the Fermi level is set to 0 eV.

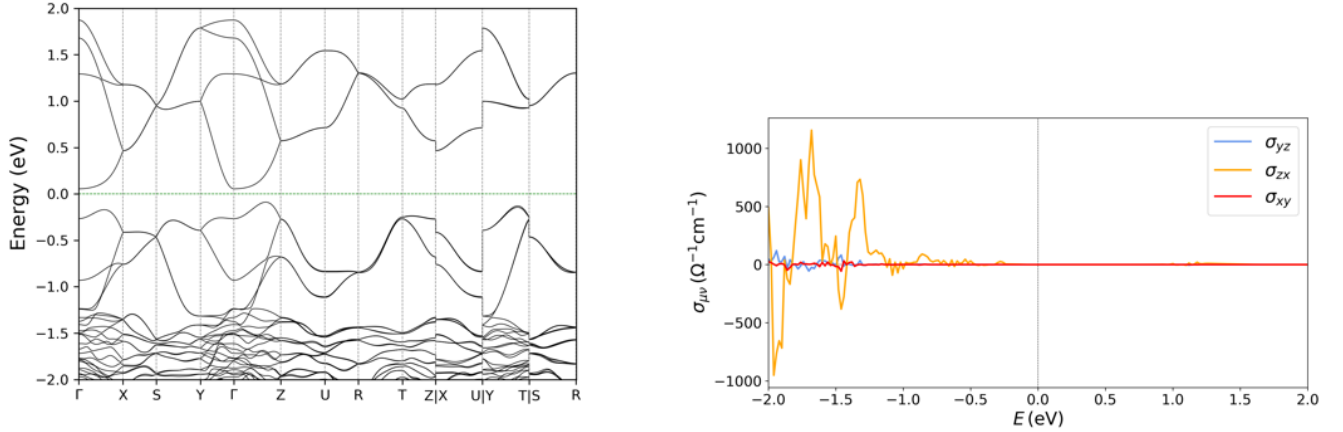

**0.377 Mn<sub>3</sub>Ge** crystallizes in type III MSG 63.464, which hosts only FNSs. The symmetry-adapted AHC tensor of the MSG is  $(0, \sigma_{zx}, 0)$ . Based on the first-principles calculation results, the comparison between the experimental and calculated magnetic moments is provided in Table SII40. The band structure is shown in the left panel of Fig. 38, and the Fermi-level-dependent AHC is plotted in the right panel.

TABLE SII40. The comparison between the experimental and calculated magnetic moments for 0.377 Mn<sub>3</sub>Ge. The five columns contain the atom index in the structure file, the atom species, the fractional coordinates, the experimental magnetic moments, and the calculated magnetic moments. The lattice vectors are  $\vec{a}_1 = (2.651, -4.591665, 0.0)$ ,  $\vec{a}_2 = (2.651, 4.591665, 0.0)$ ,  $\vec{a}_3 = (0.0, 0.0, 4.289)$ .

| No. | Atom | Coordinates(fractional) |          |          | Experimental magnetic moments |           |          | Calculated magnetic moments |           |           |
|-----|------|-------------------------|----------|----------|-------------------------------|-----------|----------|-----------------------------|-----------|-----------|
| 1   | Ge   | 0.333333                | 0.666667 | 0.250000 | 0.000000                      | 0.000000  | 0.000000 | -0.010000                   | -0.000000 | -0.000000 |
| 2   | Ge   | 0.666667                | 0.333333 | 0.750000 | 0.000000                      | 0.000000  | 0.000000 | -0.010000                   | 0.000000  | 0.001000  |
| 3   | Mn   | 0.834000                | 0.668000 | 0.250000 | 2.295020                      | -1.324970 | 0.000000 | 3.395000                    | -1.954000 | -0.012000 |
| 4   | Mn   | 0.332000                | 0.166000 | 0.250000 | -2.295020                     | -1.324970 | 0.000000 | -3.388000                   | -1.963000 | 0.011000  |
| 5   | Mn   | 0.166000                | 0.332000 | 0.750000 | 2.295020                      | -1.324970 | 0.000000 | 3.395000                    | -1.953000 | 0.012000  |
| 6   | Mn   | 0.668000                | 0.834000 | 0.750000 | -2.295020                     | -1.324970 | 0.000000 | -3.388000                   | -1.963000 | -0.012000 |
| 7   | Mn   | 0.834000                | 0.166000 | 0.250000 | 0.000000                      | 2.650030  | 0.000000 | 0.011000                    | 3.916000  | -0.001000 |
| 8   | Mn   | 0.166000                | 0.834000 | 0.750000 | 0.000000                      | 2.650030  | 0.000000 | 0.012000                    | 3.916000  | 0.001000  |

FIG. 38. First-principles calculation results of 0.377 Mn<sub>3</sub>Ge. The band structure is shown in the left panel, and the Fermi-level-dependent AHC is plotted in the right panel. In both plots, the Fermi level is set to 0 eV.

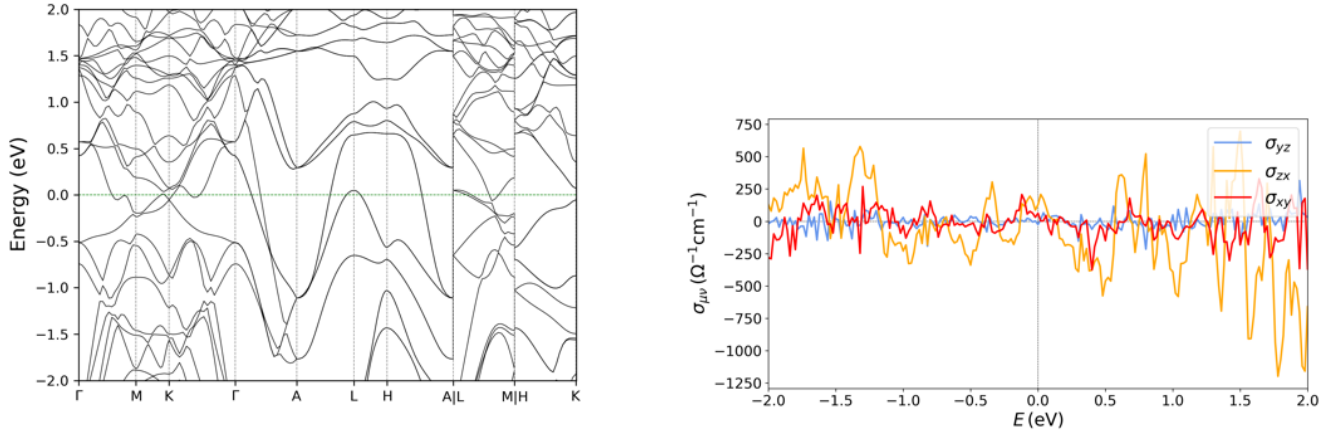

**0.38 GaFeO<sub>3</sub>** crystallizes in type III MSG 33.147, which hosts both SNLs and FNSs. The symmetry-adapted AHC tensor of the MSG is  $(\sigma_{yz}, 0, 0)$ . Based on the first-principles calculation results, the comparison between the experimental and calculated magnetic moments is provided in Table SII41. The band structure is shown in the left panel of Fig. 39, and the Fermi-level-dependent AHC is plotted in the right panel.

TABLE SII41. The comparison between the experimental and calculated magnetic moments for 0.38 GaFeO<sub>3</sub>. The five columns contain the atom index in the structure file, the atom species, the fractional coordinates, the experimental magnetic moments, and the calculated magnetic moments. The lattice vectors are  $\vec{a}_1 = (5.0672, 0.0, 0.0)$ ,  $\vec{a}_2 = (0.0, 8.7193, 0.0)$ ,  $\vec{a}_3 = (0.0, 0.0, 9.3684)$ .

| No. | Atom | Coordinates(fractional) |          |          | Experimental magnetic moments |          |          | Calculated magnetic moments |           |           |
|-----|------|-------------------------|----------|----------|-------------------------------|----------|----------|-----------------------------|-----------|-----------|
| 1   | Ga   | 0.678100                | 0.650000 | 0.000000 | 0.000000                      | 0.000000 | 0.000000 | -0.039000                   | -0.000000 | -0.000000 |
| 2   | Ga   | 0.821900                | 0.150000 | 0.500000 | 0.000000                      | 0.000000 | 0.000000 | -0.039000                   | 0.000000  | -0.000000 |
| 3   | Ga   | 0.321900                | 0.350000 | 0.500000 | 0.000000                      | 0.000000 | 0.000000 | -0.039000                   | -0.000000 | 0.000000  |
| 4   | Ga   | 0.178100                | 0.850000 | 0.000000 | 0.000000                      | 0.000000 | 0.000000 | -0.039000                   | 0.000000  | 0.000000  |
| 5   | Ga   | 0.310600                | 0.659300 | 0.307300 | -4.699980                     | 0.000000 | 0.000000 | -6.965000                   | -0.000000 | -0.000000 |
| 6   | Ga   | 0.189400                | 0.159300 | 0.807300 | -4.699980                     | 0.000000 | 0.000000 | -6.961000                   | -0.000000 | -0.000000 |
| 7   | Ga   | 0.689400                | 0.340700 | 0.807300 | -4.699980                     | 0.000000 | 0.000000 | -6.965000                   | -0.000000 | 0.000000  |
| 8   | Ga   | 0.810600                | 0.840700 | 0.307300 | -4.699980                     | 0.000000 | 0.000000 | -6.961000                   | -0.000000 | 0.000000  |
| 9   | Fe   | 0.688600                | 0.653800 | 0.583100 | 3.900020                      | 0.000000 | 0.000000 | 3.105000                    | -0.001000 | -0.000000 |
| 10  | Fe   | 0.811400                | 0.153800 | 0.083100 | 3.900020                      | 0.000000 | 0.000000 | 3.095000                    | -0.000000 | -0.000000 |
| 11  | Fe   | 0.311400                | 0.346200 | 0.083100 | 3.900020                      | 0.000000 | 0.000000 | 3.105000                    | -0.001000 | 0.000000  |
| 12  | Fe   | 0.188600                | 0.846200 | 0.583100 | 3.900020                      | 0.000000 | 0.000000 | 3.095000                    | -0.000000 | 0.000000  |
| 13  | Fe   | 0.179500                | 0.534600 | 0.799800 | -4.499980                     | 0.000000 | 0.000000 | -5.031000                   | 0.000000  | -0.000000 |
| 14  | Fe   | 0.320500                | 0.034600 | 0.299800 | -4.499980                     | 0.000000 | 0.000000 | -5.030000                   | -0.000000 | -0.000000 |
| 15  | Fe   | 0.820500                | 0.465400 | 0.299800 | -4.499980                     | 0.000000 | 0.000000 | -5.031000                   | 0.000000  | 0.000000  |
| 16  | Fe   | 0.679500                | 0.965400 | 0.799800 | -4.499980                     | 0.000000 | 0.000000 | -5.030000                   | -0.000000 | 0.000000  |
| 17  | O    | 0.471600                | 0.822800 | 0.426200 | 0.000000                      | 0.000000 | 0.000000 | 0.077000                    | -0.000000 | -0.000000 |
| 18  | O    | 0.028400                | 0.322800 | 0.926200 | 0.000000                      | 0.000000 | 0.000000 | 0.079000                    | -0.000000 | 0.000000  |
| 19  | O    | 0.528400                | 0.177200 | 0.926200 | 0.000000                      | 0.000000 | 0.000000 | 0.077000                    | -0.000000 | 0.000000  |
| 20  | O    | 0.971600                | 0.677200 | 0.426200 | 0.000000                      | 0.000000 | 0.000000 | 0.079000                    | -0.000000 | -0.000000 |
| 21  | O    | 0.014200                | 0.986400 | 0.431100 | 0.000000                      | 0.000000 | 0.000000 | 0.035000                    | 0.000000  | -0.000000 |
| 22  | O    | 0.485800                | 0.486400 | 0.931100 | 0.000000                      | 0.000000 | 0.000000 | 0.034000                    | -0.000000 | -0.000000 |
| 23  | O    | 0.985800                | 0.013600 | 0.931100 | 0.000000                      | 0.000000 | 0.000000 | 0.035000                    | 0.000000  | 0.000000  |
| 24  | O    | 0.514200                | 0.513600 | 0.431100 | 0.000000                      | 0.000000 | 0.000000 | 0.034000                    | -0.000000 | 0.000000  |
| 25  | O    | 0.154100                | 0.497900 | 0.202200 | 0.000000                      | 0.000000 | 0.000000 | 0.085000                    | -0.000000 | 0.000000  |
| 26  | O    | 0.345900                | 0.997900 | 0.702200 | 0.000000                      | 0.000000 | 0.000000 | 0.085000                    | 0.000000  | -0.000000 |
| 27  | O    | 0.845900                | 0.502100 | 0.702200 | 0.000000                      | 0.000000 | 0.000000 | 0.085000                    | -0.000000 | -0.000000 |
| 28  | O    | 0.654100                | 0.002100 | 0.202200 | 0.000000                      | 0.000000 | 0.000000 | 0.085000                    | 0.000000  | 0.000000  |
| 29  | O    | 0.648000                | 0.659300 | 0.197400 | 0.000000                      | 0.000000 | 0.000000 | 0.037000                    | -0.000000 | -0.000000 |
| 30  | O    | 0.852000                | 0.159300 | 0.697400 | 0.000000                      | 0.000000 | 0.000000 | 0.035000                    | -0.000000 | -0.000000 |
| 31  | O    | 0.352000                | 0.340700 | 0.697400 | 0.000000                      | 0.000000 | 0.000000 | 0.037000                    | -0.000000 | 0.000000  |
| 32  | O    | 0.148000                | 0.840700 | 0.197400 | 0.000000                      | 0.000000 | 0.000000 | 0.035000                    | -0.000000 | 0.000000  |
| 33  | O    | 0.343700                | 0.669500 | 0.671700 | 0.000000                      | 0.000000 | 0.000000 | 0.035000                    | -0.000000 | 0.000000  |
| 34  | O    | 0.156300                | 0.169500 | 0.171700 | 0.000000                      | 0.000000 | 0.000000 | 0.034000                    | -0.000000 | -0.000000 |
| 35  | O    | 0.656300                | 0.330500 | 0.171700 | 0.000000                      | 0.000000 | 0.000000 | 0.035000                    | -0.000000 | -0.000000 |
| 36  | O    | 0.843700                | 0.830500 | 0.671700 | 0.000000                      | 0.000000 | 0.000000 | 0.034000                    | -0.000000 | -0.000000 |
| 37  | O    | 0.016600                | 0.673600 | 0.938300 | 0.000000                      | 0.000000 | 0.000000 | -0.008000                   | -0.000000 | 0.000000  |
| 38  | O    | 0.483400                | 0.173600 | 0.438300 | 0.000000                      | 0.000000 | 0.000000 | -0.008000                   | 0.000000  | -0.000000 |
| 39  | O    | 0.983400                | 0.326400 | 0.438300 | 0.000000                      | 0.000000 | 0.000000 | -0.008000                   | -0.000000 | -0.000000 |
| 40  | O    | 0.516600                | 0.826400 | 0.938300 | 0.000000                      | 0.000000 | 0.000000 | -0.008000                   | 0.000000  | 0.000000  |

FIG. 39. First-principles calculation results of 0.38 GaFeO<sub>3</sub>. The band structure is shown in the left panel, and the Fermi-level-dependent AHC is plotted in the right panel. In both plots, the Fermi level is set to 0 eV.

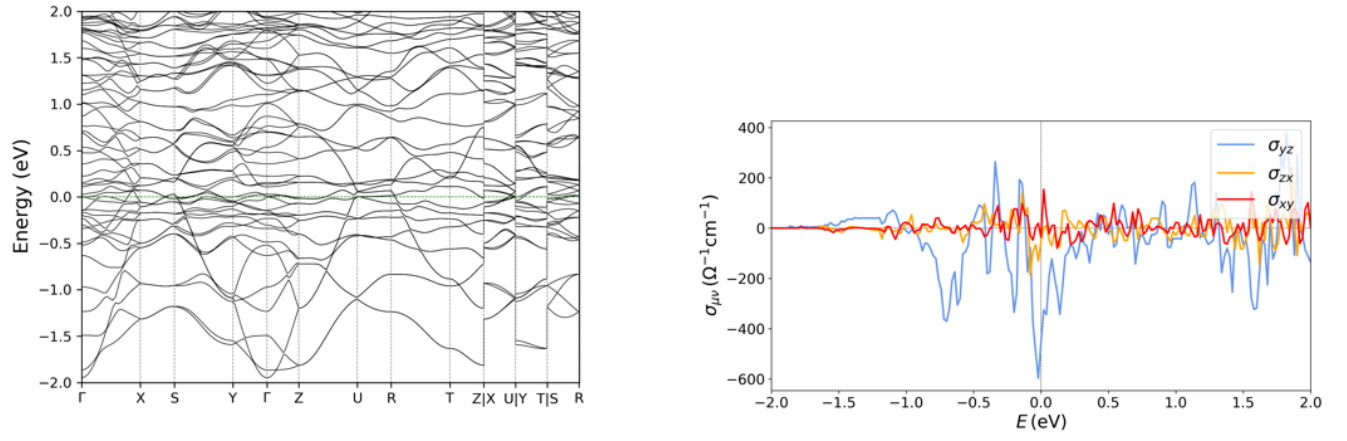

0.642  $\text{LaMnO}_3$  crystallizes in type III MSG 62.448, which hosts both SNLs and FNSs. The symmetry-adapted AHC tensor of the MSG is  $(0, \sigma_{zx}, 0)$ . Based on the first-principles calculation results, the comparison between the experimental and calculated magnetic moments is provided in Table SII70. The band structure is shown in the left panel of Fig. 68, and the Fermi-level-dependent AHC is plotted in the right panel.

TABLE SII42. The comparison between the experimental and calculated magnetic moments for 0.642  $\text{LaMnO}_3$ . The five columns contain the atom index in the structure file, the atom species, the fractional coordinates, the experimental magnetic moments, and the calculated magnetic moments. The lattice vectors are  $\vec{a}_1 = (5.742, 0.0, 0.0)$ ,  $\vec{a}_2 = (0.0, 7.668, 0.0)$ ,  $\vec{a}_3 = (0.0, 0.0, 5.532)$ .

| No. | Atom | Coordinates(fractional) |          |          | Experimental magnetic moments |          |          | Calculated magnetic moments |           |           |
|-----|------|-------------------------|----------|----------|-------------------------------|----------|----------|-----------------------------|-----------|-----------|
| 1   | La   | 0.049000                | 0.250000 | 0.510000 | 0.000000                      | 0.000000 | 0.000000 | -0.000000                   | -0.000000 | -0.000000 |
| 2   | La   | 0.951000                | 0.750000 | 0.490000 | 0.000000                      | 0.000000 | 0.000000 | -0.000000                   | 0.000000  | 0.000000  |
| 3   | La   | 0.549000                | 0.250000 | 0.990000 | 0.000000                      | 0.000000 | 0.000000 | 0.000000                    | -0.000000 | -0.000000 |
| 4   | La   | 0.451000                | 0.750000 | 0.010000 | 0.000000                      | 0.000000 | 0.000000 | 0.000000                    | 0.000000  | 0.000000  |
| 5   | Mn   | 0.000000                | 0.000000 | 0.000000 | 3.699970                      | 0.000000 | 0.000000 | 4.259000                    | 0.000000  | -0.000000 |
| 6   | Mn   | 0.000000                | 0.500000 | 0.000000 | -3.699970                     | 0.000000 | 0.000000 | -4.259000                   | 0.000000  | 0.000000  |
| 7   | Mn   | 0.500000                | 0.500000 | 0.500000 | -3.699970                     | 0.000000 | 0.000000 | -4.259000                   | 0.000000  | -0.000000 |
| 8   | Mn   | 0.500000                | 0.000000 | 0.500000 | 3.699970                      | 0.000000 | 0.000000 | 4.259000                    | 0.000000  | 0.000000  |
| 9   | O    | 0.486000                | 0.250000 | 0.430000 | 0.000000                      | 0.000000 | 0.000000 | -0.001000                   | -0.001000 | 0.000000  |
| 10  | O    | 0.514000                | 0.750000 | 0.570000 | 0.000000                      | 0.000000 | 0.000000 | -0.001000                   | -0.001000 | -0.000000 |
| 11  | O    | 0.986000                | 0.250000 | 0.070000 | 0.000000                      | 0.000000 | 0.000000 | 0.001000                    | 0.000000  | 0.000000  |
| 12  | O    | 0.014000                | 0.750000 | 0.930000 | 0.000000                      | 0.000000 | 0.000000 | 0.001000                    | 0.001000  | -0.000000 |
| 13  | O    | 0.809000                | 0.039000 | 0.724000 | 0.000000                      | 0.000000 | 0.000000 | -0.095000                   | -0.000000 | 0.000000  |
| 14  | O    | 0.191000                | 0.539000 | 0.276000 | 0.000000                      | 0.000000 | 0.000000 | 0.095000                    | 0.000000  | -0.000000 |
| 15  | O    | 0.191000                | 0.961000 | 0.276000 | 0.000000                      | 0.000000 | 0.000000 | -0.095000                   | 0.000000  | -0.000000 |
| 16  | O    | 0.809000                | 0.461000 | 0.724000 | 0.000000                      | 0.000000 | 0.000000 | 0.095000                    | -0.000000 | -0.000000 |
| 17  | O    | 0.309000                | 0.461000 | 0.776000 | 0.000000                      | 0.000000 | 0.000000 | 0.095000                    | 0.000000  | 0.000000  |
| 18  | O    | 0.691000                | 0.961000 | 0.224000 | 0.000000                      | 0.000000 | 0.000000 | -0.095000                   | 0.000000  | 0.000000  |
| 19  | O    | 0.691000                | 0.539000 | 0.224000 | 0.000000                      | 0.000000 | 0.000000 | 0.095000                    | 0.000000  | -0.000000 |
| 20  | O    | 0.309000                | 0.039000 | 0.776000 | 0.000000                      | 0.000000 | 0.000000 | -0.095000                   | 0.000000  | -0.000000 |

FIG. 40. First-principles calculation results of 0.642  $\text{LaMnO}_3$ . The band structure is shown in the left panel, and the Fermi-level-dependent AHC is plotted in the right panel. In both plots, the Fermi level is set to 0 eV.

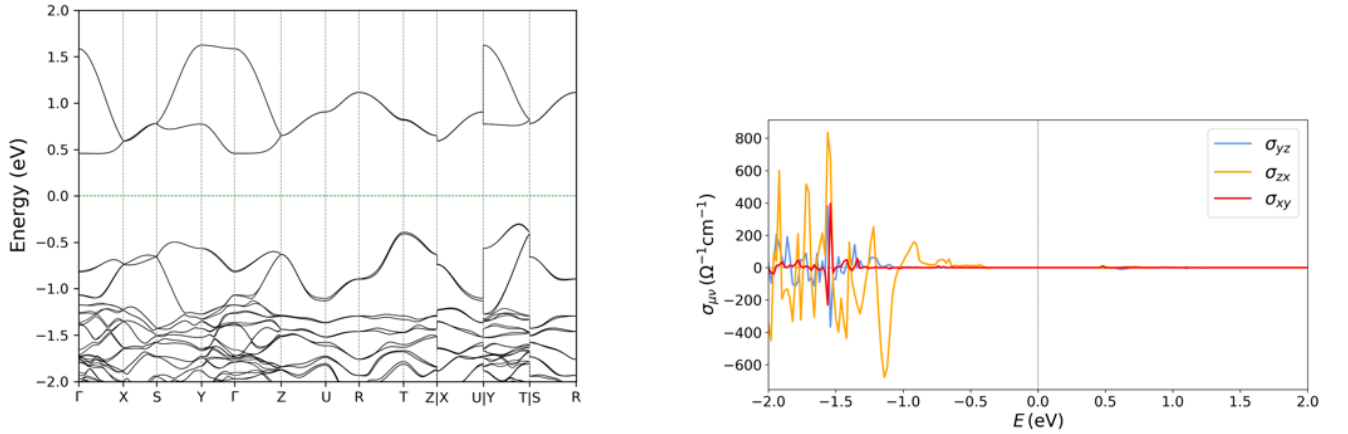

**0.662 Mn<sub>3</sub>Sn<sub>2</sub>** crystallizes in type III MSG 62.448, which hosts both SNLs and FNSs. The symmetry-adapted AHC tensor of the MSG is  $(0, \sigma_{zx}, 0)$ . Based on the first-principles calculation results, the comparison between the experimental and calculated magnetic moments is provided in Table SII43. The band structure is shown in the left panel of Fig. 41, and the Fermi-level-dependent AHC is plotted in the right panel.

TABLE SII43. The comparison between the experimental and calculated magnetic moments for 0.662 Mn<sub>3</sub>Sn<sub>2</sub>. The five columns contain the atom index in the structure file, the atom species, the fractional coordinates, the experimental magnetic moments, and the calculated magnetic moments. The lattice vectors are  $\vec{a}_1 = (7.5646, 0.0, 0.0)$ ,  $\vec{a}_2 = (0.0, 5.5099, 0.0)$ ,  $\vec{a}_3 = (0.0, 0.0, 8.5975)$ .

| No. | Atom | Coordinates(fractional) |          |          | Experimental magnetic moments |          |          | Calculated magnetic moments |           |           |
|-----|------|-------------------------|----------|----------|-------------------------------|----------|----------|-----------------------------|-----------|-----------|
| 1   | Mn   | 0.724500                | 0.003600 | 0.622900 | 0.000000                      | 0.830010 | 0.000000 | -0.001000                   | 1.355000  | -0.001000 |
| 2   | Mn   | 0.275500                | 0.503600 | 0.377100 | 0.000000                      | 0.830010 | 0.000000 | -0.000000                   | 1.361000  | 0.000000  |
| 3   | Mn   | 0.275500                | 0.996400 | 0.377100 | 0.000000                      | 0.830010 | 0.000000 | 0.001000                    | 1.355000  | 0.001000  |
| 4   | Mn   | 0.724500                | 0.496400 | 0.622900 | 0.000000                      | 0.830010 | 0.000000 | 0.000000                    | 1.358000  | -0.002000 |
| 5   | Mn   | 0.224500                | 0.496400 | 0.877100 | 0.000000                      | 0.830010 | 0.000000 | 0.001000                    | 1.352000  | -0.001000 |
| 6   | Mn   | 0.775500                | 0.996400 | 0.122900 | 0.000000                      | 0.830010 | 0.000000 | 0.000000                    | 1.364000  | -0.000000 |
| 7   | Mn   | 0.775500                | 0.503600 | 0.122900 | 0.000000                      | 0.830010 | 0.000000 | -0.001000                   | 1.351000  | 0.001000  |
| 8   | Mn   | 0.224500                | 0.003600 | 0.877100 | 0.000000                      | 0.830010 | 0.000000 | -0.001000                   | 1.362000  | -0.002000 |
| 9   | Mn   | 0.407900                | 0.250000 | 0.629900 | 0.000000                      | 1.529990 | 0.000000 | -0.001000                   | 2.795000  | 0.000000  |
| 10  | Mn   | 0.592100                | 0.750000 | 0.370100 | 0.000000                      | 1.529990 | 0.000000 | -0.001000                   | 2.794000  | -0.000000 |
| 11  | Mn   | 0.907900                | 0.250000 | 0.870100 | 0.000000                      | 1.529990 | 0.000000 | -0.000000                   | 2.795000  | 0.001000  |
| 12  | Mn   | 0.092100                | 0.750000 | 0.129900 | 0.000000                      | 1.529990 | 0.000000 | -0.000000                   | 2.794000  | 0.000000  |
| 13  | Sn   | 0.096900                | 0.250000 | 0.142600 | 0.000000                      | 0.000000 | 0.000000 | 0.000000                    | -0.138000 | -0.000000 |
| 14  | Sn   | 0.903100                | 0.750000 | 0.857400 | 0.000000                      | 0.000000 | 0.000000 | -0.001000                   | -0.139000 | 0.001000  |
| 15  | Sn   | 0.596900                | 0.250000 | 0.357400 | 0.000000                      | 0.000000 | 0.000000 | -0.001000                   | -0.139000 | -0.000000 |
| 16  | Sn   | 0.403100                | 0.750000 | 0.642600 | 0.000000                      | 0.000000 | 0.000000 | 0.001000                    | -0.138000 | 0.001000  |
| 17  | Sn   | 0.061000                | 0.250000 | 0.593200 | 0.000000                      | 0.000000 | 0.000000 | -0.001000                   | -0.052000 | 0.001000  |
| 18  | Sn   | 0.939000                | 0.750000 | 0.406800 | 0.000000                      | 0.000000 | 0.000000 | 0.000000                    | -0.053000 | -0.001000 |
| 19  | Sn   | 0.561000                | 0.250000 | 0.906800 | 0.000000                      | 0.000000 | 0.000000 | 0.001000                    | -0.052000 | 0.001000  |
| 20  | Sn   | 0.439000                | 0.750000 | 0.093200 | 0.000000                      | 0.000000 | 0.000000 | -0.001000                   | -0.053000 | -0.000000 |

FIG. 41. First-principles calculation results of 0.662 Mn<sub>3</sub>Sn<sub>2</sub>. The band structure is shown in the left panel, and the Fermi-level-dependent AHC is plotted in the right panel. In both plots, the Fermi level is set to 0 eV.

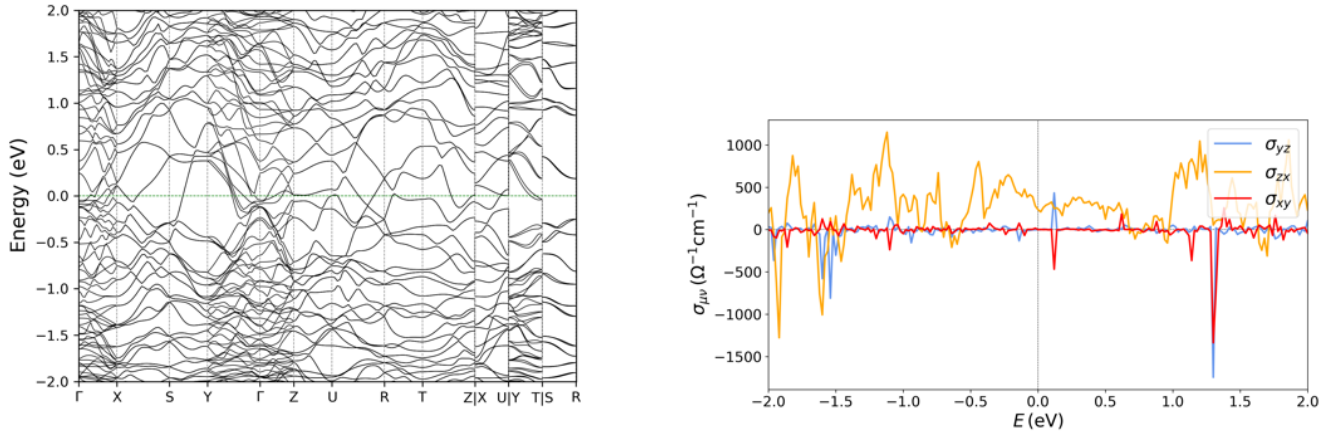

**0.663 Mn<sub>3</sub>Sn<sub>2</sub>** crystallizes in type III MSG 62.448, which hosts both SNLs and FNSs. The symmetry-adapted AHC tensor of the MSG is  $(0, \sigma_{zx}, 0)$ . Based on the first-principles calculation results, the comparison between the experimental and calculated magnetic moments is provided in Table SII44. The band structure is shown in the left panel of Fig. 42, and the Fermi-level-dependent AHC is plotted in the right panel.

TABLE SII44. The comparison between the experimental and calculated magnetic moments for 0.663 Mn<sub>3</sub>Sn<sub>2</sub>. The five columns contain the atom index in the structure file, the atom species, the fractional coordinates, the experimental magnetic moments, and the calculated magnetic moments. The lattice vectors are  $\vec{a}_1 = (7.5646, 0.0, 0.0)$ ,  $\vec{a}_2 = (0.0, 5.5099, 0.0)$ ,  $\vec{a}_3 = (0.0, 0.0, 8.5975)$ .

| No. | Atom | Coordinates(fractional) |          |          | Experimental magnetic moments |          |          | Calculated magnetic moments |           |           |
|-----|------|-------------------------|----------|----------|-------------------------------|----------|----------|-----------------------------|-----------|-----------|
| 1   | Mn   | 0.724500                | 0.003600 | 0.622900 | -1.490000                     | 1.180000 | 0.000000 | -2.554000                   | 1.983000  | -0.019000 |
| 2   | Mn   | 0.275500                | 0.503600 | 0.377100 | 1.490000                      | 1.180000 | 0.000000 | 2.560000                    | 1.982000  | 0.017000  |
| 3   | Mn   | 0.275500                | 0.996400 | 0.377100 | -1.490000                     | 1.180000 | 0.000000 | -2.550000                   | 1.982000  | 0.018000  |
| 4   | Mn   | 0.724500                | 0.496400 | 0.622900 | 1.490000                      | 1.180000 | 0.000000 | 2.560000                    | 1.981000  | -0.018000 |
| 5   | Mn   | 0.224500                | 0.496400 | 0.877100 | 1.490000                      | 1.180000 | 0.000000 | 2.556000                    | 1.993000  | -0.018000 |
| 6   | Mn   | 0.775500                | 0.996400 | 0.122900 | -1.490000                     | 1.180000 | 0.000000 | -2.558000                   | 1.972000  | 0.018000  |
| 7   | Mn   | 0.775500                | 0.503600 | 0.122900 | 1.490000                      | 1.180000 | 0.000000 | 2.554000                    | 1.992000  | 0.017000  |
| 8   | Mn   | 0.224500                | 0.003600 | 0.877100 | -1.490000                     | 1.180000 | 0.000000 | -2.556000                   | 1.971000  | -0.019000 |
| 9   | Mn   | 0.407900                | 0.250000 | 0.629900 | 0.000000                      | 1.790000 | 0.000000 | -0.001000                   | 3.068000  | 0.013000  |
| 10  | Mn   | 0.592100                | 0.750000 | 0.370100 | 0.000000                      | 1.790000 | 0.000000 | 0.007000                    | 3.062000  | -0.015000 |
| 11  | Mn   | 0.907900                | 0.250000 | 0.870100 | 0.000000                      | 1.790000 | 0.000000 | 0.008000                    | 3.068000  | 0.014000  |
| 12  | Mn   | 0.092100                | 0.750000 | 0.129900 | 0.000000                      | 1.790000 | 0.000000 | 0.000000                    | 3.062000  | -0.013000 |
| 13  | Sn   | 0.096900                | 0.250000 | 0.142600 | 0.000000                      | 0.000000 | 0.000000 | 0.002000                    | -0.178000 | 0.003000  |
| 14  | Sn   | 0.903100                | 0.750000 | 0.857400 | 0.000000                      | 0.000000 | 0.000000 | 0.002000                    | -0.177000 | -0.004000 |
| 15  | Sn   | 0.596900                | 0.250000 | 0.357400 | 0.000000                      | 0.000000 | 0.000000 | 0.002000                    | -0.178000 | 0.003000  |
| 16  | Sn   | 0.403100                | 0.750000 | 0.642600 | 0.000000                      | 0.000000 | 0.000000 | 0.001000                    | -0.177000 | -0.004000 |
| 17  | Sn   | 0.061000                | 0.250000 | 0.593200 | 0.000000                      | 0.000000 | 0.000000 | 0.000000                    | -0.131000 | 0.013000  |
| 18  | Sn   | 0.939000                | 0.750000 | 0.406800 | 0.000000                      | 0.000000 | 0.000000 | 0.002000                    | -0.132000 | -0.012000 |
| 19  | Sn   | 0.561000                | 0.250000 | 0.906800 | 0.000000                      | 0.000000 | 0.000000 | 0.001000                    | -0.131000 | 0.013000  |
| 20  | Sn   | 0.439000                | 0.750000 | 0.093200 | 0.000000                      | 0.000000 | 0.000000 | -0.001000                   | -0.132000 | -0.012000 |

FIG. 42. First-principles calculation results of 0.663 Mn<sub>3</sub>Sn<sub>2</sub>. The band structure is shown in the left panel, and the Fermi-level-dependent AHC is plotted in the right panel. In both plots, the Fermi level is set to 0 eV.

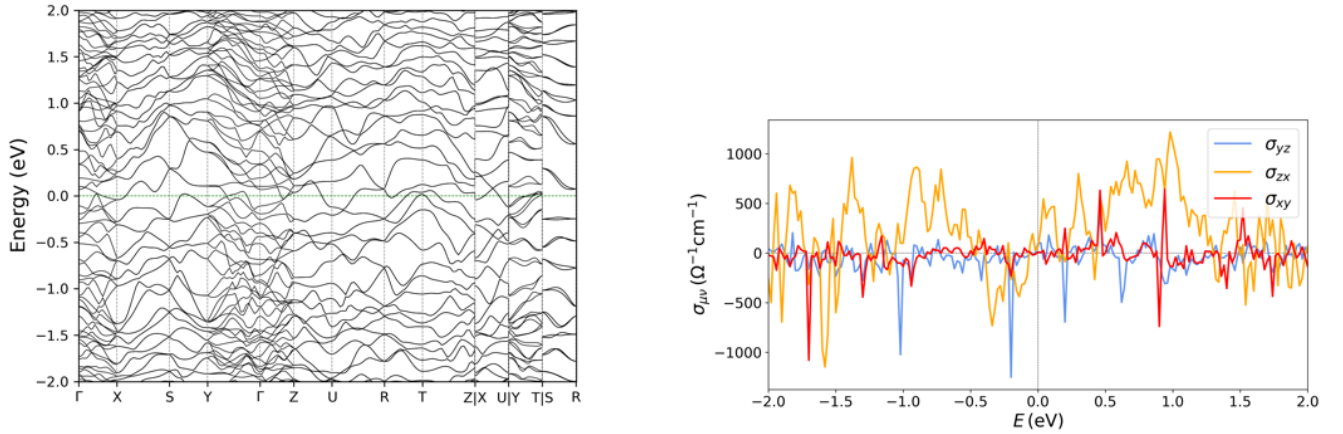



**0.684 TbPt** crystallizes in type III MSG 62.446, which hosts both SNLs and FNSs. The symmetry-adapted AHC tensor of the MSG is  $(0, 0, \sigma_{xy})$ . Based on the first-principles calculation results, the comparison between the experimental and calculated magnetic moments is provided in Table SII45. The band structure is shown in the left panel of Fig. 43, and the Fermi-level-dependent AHC is plotted in the right panel.

TABLE SII45. The comparison between the experimental and calculated magnetic moments for 0.684 TbPt. The five columns contain the atom index in the structure file, the atom species, the fractional coordinates, the experimental magnetic moments, and the calculated magnetic moments. The lattice vectors are  $\vec{a}_1 = (7.013, 0.0, 0.0)$ ,  $\vec{a}_2 = (0.0, 4.49, 0.0)$ ,  $\vec{a}_3 = (0.0, 0.0, 5.564)$ .

| No. | Atom | Coordinates(fractional) |          |          | Experimental magnetic moments |          |          | Calculated magnetic moments |           |           |
|-----|------|-------------------------|----------|----------|-------------------------------|----------|----------|-----------------------------|-----------|-----------|
| 1   | Pt   | 0.466600                | 0.250000 | 0.162000 | 0.000000                      | 0.000000 | 0.000000 | -0.083000                   | 0.004000  | -0.335000 |
| 2   | Pt   | 0.033400                | 0.750000 | 0.662000 | 0.000000                      | 0.000000 | 0.000000 | 0.106000                    | -0.006000 | -0.320000 |
| 3   | Pt   | 0.533400                | 0.750000 | 0.838000 | 0.000000                      | 0.000000 | 0.000000 | -0.104000                   | -0.003000 | -0.323000 |
| 4   | Pt   | 0.966600                | 0.250000 | 0.338000 | 0.000000                      | 0.000000 | 0.000000 | 0.085000                    | 0.008000  | -0.332000 |
| 5   | Tb   | 0.323000                | 0.250000 | 0.648000 | 4.990030                      | 0.000000 | 6.380020 | 5.388000                    | -0.011000 | 6.930000  |
| 6   | Tb   | 0.177000                | 0.750000 | 0.148000 | -4.990030                     | 0.000000 | 6.380020 | -5.387000                   | 0.009000  | 6.932000  |
| 7   | Tb   | 0.677000                | 0.750000 | 0.352000 | 4.990030                      | 0.000000 | 6.380020 | 5.388000                    | 0.011000  | 6.934000  |
| 8   | Tb   | 0.823000                | 0.250000 | 0.852000 | -4.990030                     | 0.000000 | 6.380020 | -5.387000                   | -0.009000 | 6.928000  |

FIG. 43. First-principles calculation results of 0.684 TbPt. The band structure is shown in the left panel, and the Fermi-level-dependent AHC is plotted in the right panel. In both plots, the Fermi level is set to 0 eV.

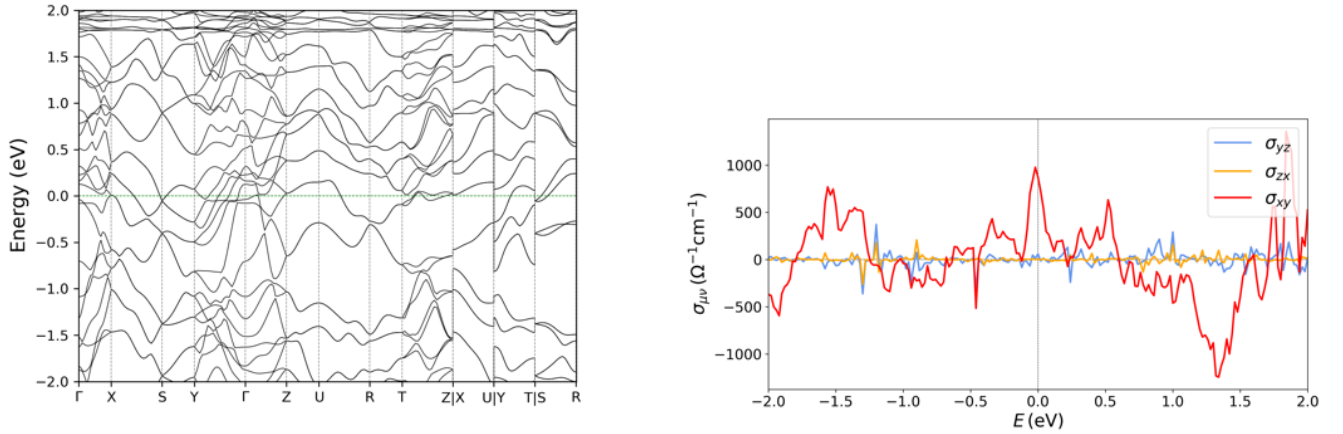

**0.686 HoPt** crystallizes in type III MSG 62.447, which hosts both SNLs and FNSs. The symmetry-adapted AHC tensor of the MSG is  $(\sigma_{yz}, 0, 0)$ . Based on the first-principles calculation results, the comparison between the experimental and calculated magnetic moments is provided in Table SII46. The band structure is shown in the left panel of Fig. 44, and the Fermi-level-dependent AHC is plotted in the right panel.

TABLE SII46. The comparison between the experimental and calculated magnetic moments for 0.686 HoPt. The five columns contain the atom index in the structure file, the atom species, the fractional coordinates, the experimental magnetic moments, and the calculated magnetic moments. The lattice vectors are  $\vec{a}_1 = (6.947, 0.0, 0.0)$ ,  $\vec{a}_2 = (0.0, 4.462, 0.0)$ ,  $\vec{a}_3 = (0.0, 0.0, 5.526)$ .

| No. | Atom | Coordinates(fractional) |          |          | Experimental magnetic moments |          |           | Calculated magnetic moments |           |           |
|-----|------|-------------------------|----------|----------|-------------------------------|----------|-----------|-----------------------------|-----------|-----------|
| 1   | Ho   | 0.681000                | 0.250000 | 0.128000 | 7.550000                      | 0.000000 | -3.200000 | 7.092000                    | 0.008000  | -2.988000 |
| 2   | Ho   | 0.181000                | 0.250000 | 0.372000 | 7.550000                      | 0.000000 | 3.200000  | 7.071000                    | 0.003000  | 2.980000  |
| 3   | Ho   | 0.319000                | 0.750000 | 0.872000 | 7.550000                      | 0.000000 | -3.200000 | 7.091000                    | -0.008000 | -2.988000 |
| 4   | Ho   | 0.819000                | 0.750000 | 0.628000 | 7.550000                      | 0.000000 | 3.200000  | 7.071000                    | -0.003000 | 2.981000  |
| 5   | Pt   | 0.527000                | 0.250000 | 0.615000 | 0.000000                      | 0.000000 | 0.000000  | -0.507000                   | -0.012000 | 0.032000  |
| 6   | Pt   | 0.027000                | 0.250000 | 0.885000 | 0.000000                      | 0.000000 | 0.000000  | -0.529000                   | 0.002000  | -0.030000 |
| 7   | Pt   | 0.473000                | 0.750000 | 0.385000 | 0.000000                      | 0.000000 | 0.000000  | -0.507000                   | 0.010000  | 0.033000  |
| 8   | Pt   | 0.973000                | 0.750000 | 0.115000 | 0.000000                      | 0.000000 | 0.000000  | -0.529000                   | -0.004000 | -0.029000 |

FIG. 44. First-principles calculation results of 0.686 HoPt. The band structure is shown in the left panel, and the Fermi-level-dependent AHC is plotted in the right panel. In both plots, the Fermi level is set to 0 eV.

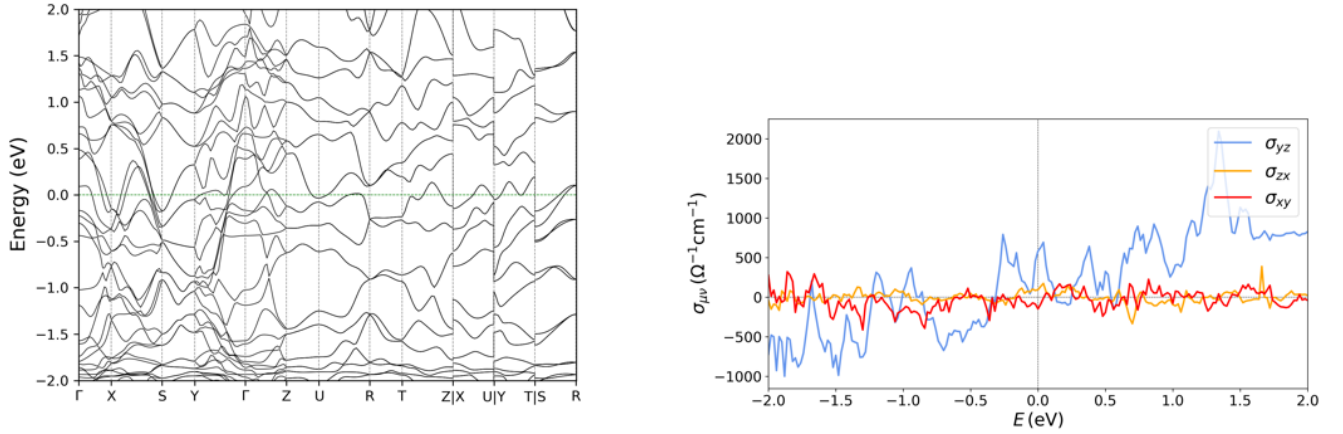

0.688 TmPt crystallizes in type III MSG 62.447, which hosts both SNLs and FNSs. The symmetry-adapted AHC tensor of the MSG is  $(\sigma_{yz}, 0, 0)$ . Based on the first-principles calculation results, the comparison between the experimental and calculated magnetic moments is provided in Table SII47. The band structure is shown in the left panel of Fig. 45, and the Fermi-level-dependent AHC is plotted in the right panel.

TABLE SII47. The comparison between the experimental and calculated magnetic moments for 0.688 TmPt. The five columns contain the atom index in the structure file, the atom species, the fractional coordinates, the experimental magnetic moments, and the calculated magnetic moments. The lattice vectors are  $\vec{a}_1 = (6.855, 0.0, 0.0)$ ,  $\vec{a}_2 = (0.0, 4.446, 0.0)$ ,  $\vec{a}_3 = (0.0, 0.0, 5.496)$ .

| No. | Atom | Coordinates(fractional) |          |          | Experimental magnetic moments |          |           | Calculated magnetic moments |           |           |
|-----|------|-------------------------|----------|----------|-------------------------------|----------|-----------|-----------------------------|-----------|-----------|
| 1   | Tm   | 0.685000                | 0.250000 | 0.144000 | 3.590030                      | 0.000000 | 2.710020  | 3.028000                    | 0.003000  | 2.255000  |
| 2   | Tm   | 0.185000                | 0.250000 | 0.356000 | 3.590030                      | 0.000000 | -2.710020 | 3.037000                    | 0.011000  | -2.263000 |
| 3   | Tm   | 0.315000                | 0.750000 | 0.856000 | 3.590030                      | 0.000000 | 2.710020  | 3.029000                    | -0.004000 | 2.256000  |
| 4   | Tm   | 0.815000                | 0.750000 | 0.644000 | 3.590030                      | 0.000000 | -2.710020 | 3.036000                    | -0.011000 | -2.262000 |
| 5   | Pt   | 0.540000                | 0.250000 | 0.653000 | 0.000000                      | 0.000000 | 0.000000  | -0.369000                   | 0.003000  | -0.070000 |
| 6   | Pt   | 0.040000                | 0.250000 | 0.847000 | 0.000000                      | 0.000000 | 0.000000  | -0.363000                   | 0.003000  | 0.061000  |
| 7   | Pt   | 0.460000                | 0.750000 | 0.347000 | 0.000000                      | 0.000000 | 0.000000  | -0.370000                   | -0.004000 | -0.069000 |
| 8   | Pt   | 0.960000                | 0.750000 | 0.153000 | 0.000000                      | 0.000000 | 0.000000  | -0.362000                   | -0.004000 | 0.063000  |

FIG. 45. First-principles calculation results of 0.688 TmPt. The band structure is shown in the left panel, and the Fermi-level-dependent AHC is plotted in the right panel. In both plots, the Fermi level is set to 0 eV.

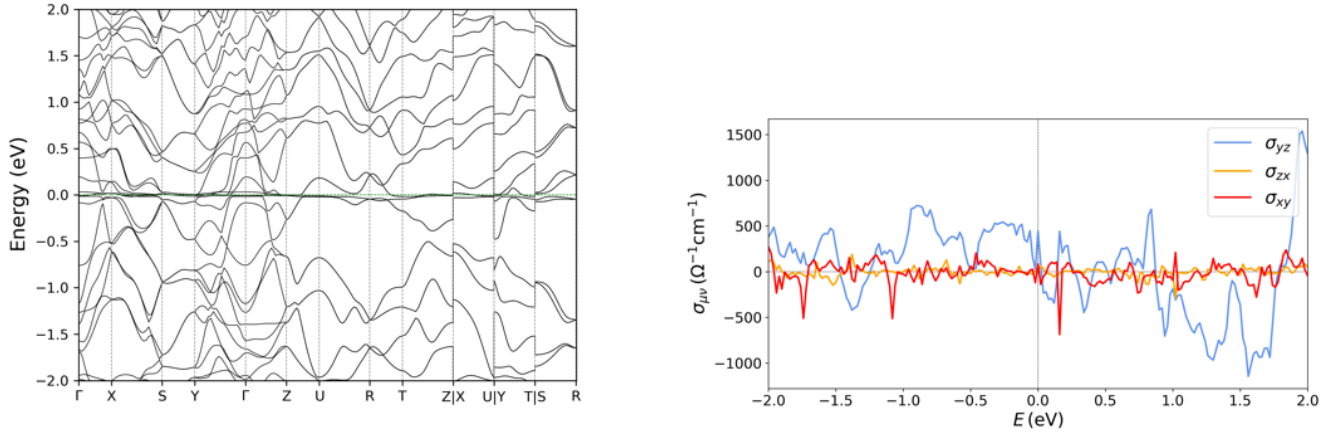

**0.689 PrPt** crystallizes in type III MSG 63.462, which hosts only SNLs. The symmetry-adapted AHC tensor of the MSG is  $(0, 0, \sigma_{xy})$ . Based on the first-principles calculation results, the comparison between the experimental and calculated magnetic moments is provided in Table SII48. The band structure is shown in the left panel of Fig. 46, and the Fermi-level-dependent AHC is plotted in the right panel.

TABLE SII48. The comparison between the experimental and calculated magnetic moments for 0.689 PrPt. The five columns contain the atom index in the structure file, the atom species, the fractional coordinates, the experimental magnetic moments, and the calculated magnetic moments. The lattice vectors are  $\vec{a}_1 = (1.9455, -5.4495, 0.0)$ ,  $\vec{a}_2 = (1.9455, 5.4495, 0.0)$ ,  $\vec{a}_3 = (0.0, 0.0, 4.569)$ .

| No. | Atom | Coordinates(fractional) |          |          | Experimental magnetic moments |          |          | Calculated magnetic moments |           |           |
|-----|------|-------------------------|----------|----------|-------------------------------|----------|----------|-----------------------------|-----------|-----------|
| 1   | Pt   | 0.591000                | 0.409000 | 0.250000 | 0.000000                      | 0.000000 | 0.000000 | 0.003000                    | -0.001000 | -0.105000 |
| 2   | Pt   | 0.409000                | 0.591000 | 0.750000 | 0.000000                      | 0.000000 | 0.000000 | -0.007000                   | -0.001000 | -0.092000 |
| 3   | Pr   | 0.868000                | 0.132000 | 0.250000 | 0.000000                      | 0.000000 | 2.200020 | 0.003000                    | -0.000000 | 2.324000  |
| 4   | Pr   | 0.132000                | 0.868000 | 0.750000 | 0.000000                      | 0.000000 | 2.200020 | -0.004000                   | -0.000000 | 2.346000  |

FIG. 46. First-principles calculation results of 0.689 PrPt. The band structure is shown in the left panel, and the Fermi-level-dependent AHC is plotted in the right panel. In both plots, the Fermi level is set to 0 eV.

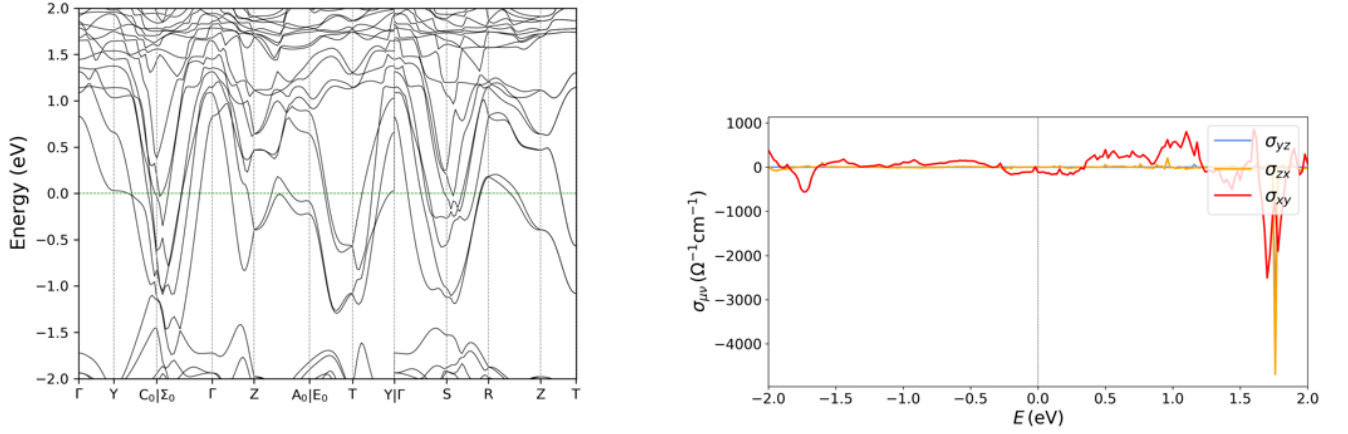

**0.690 NdPt** crystallizes in type III MSG 15.89, which hosts only SNLs. The symmetry-adapted AHC tensor of the MSG is  $(\sigma_{yz}, \sigma_{zx}, 0)$ . Based on the first-principles calculation results, the comparison between the experimental and calculated magnetic moments is provided in Table SII49. The band structure is shown in the left panel of Fig. 47, and the Fermi-level-dependent AHC is plotted in the right panel.

TABLE SII49. The comparison between the experimental and calculated magnetic moments for 0.690 NdPt. The five columns contain the atom index in the structure file, the atom species, the fractional coordinates, the experimental magnetic moments, and the calculated magnetic moments. The lattice vectors are  $\vec{a}_1 = (1.923, -5.3845, 0.0)$ ,  $\vec{a}_2 = (1.923, 5.3845, 0.0)$ ,  $\vec{a}_3 = (0.0, 0.0, 4.542)$ .

| No. | Atom | Coordinates(fractional) |          |          | Experimental magnetic moments |          | Calculated magnetic moments |           |           |          |
|-----|------|-------------------------|----------|----------|-------------------------------|----------|-----------------------------|-----------|-----------|----------|
| 1   | Nd   | 0.131000                | 0.869000 | 0.250000 | 2.169990                      | 0.000000 | 0.880010                    | 2.321000  | -0.035000 | 0.955000 |
| 2   | Nd   | 0.869000                | 0.131000 | 0.750000 | 2.169990                      | 0.000000 | 0.880010                    | 2.308000  | -0.036000 | 0.950000 |
| 3   | Pt   | 0.416000                | 0.584000 | 0.250000 | 0.000000                      | 0.000000 | 0.000000                    | -0.000000 | 0.000000  | 0.005000 |
| 4   | Pt   | 0.584000                | 0.416000 | 0.750000 | 0.000000                      | 0.000000 | 0.000000                    | 0.010000  | 0.001000  | 0.003000 |

FIG. 47. First-principles calculation results of 0.690 NdPt. The band structure is shown in the left panel, and the Fermi-level-dependent AHC is plotted in the right panel. In both plots, the Fermi level is set to 0 eV.

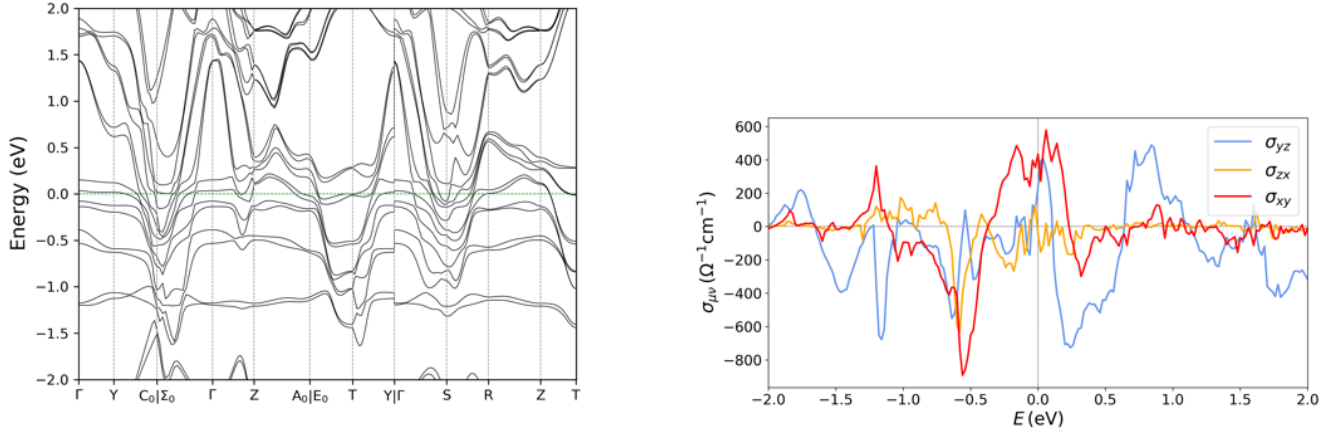

**0.732 SrRuO<sub>3</sub>** crystallizes in type III MSG 62.446, which hosts both SNLs and FNSs. The symmetry-adapted AHC tensor of the MSG is  $(0, 0, \sigma_{xy})$ . Based on the first-principles calculation results, the comparison between the experimental and calculated magnetic moments is provided in Table SII50. The band structure is shown in the left panel of Fig. 48, and the Fermi-level-dependent AHC is plotted in the right panel.

TABLE SII50. The comparison between the experimental and calculated magnetic moments for 0.732 SrRuO<sub>3</sub>. The five columns contain the atom index in the structure file, the atom species, the fractional coordinates, the experimental magnetic moments, and the calculated magnetic moments. The lattice vectors are  $\vec{a}_1 = (5.52421, 0.0, 0.0)$ ,  $\vec{a}_2 = (0.0, 7.8348, 0.0)$ ,  $\vec{a}_3 = (0.0, 0.0, 5.55907)$ .

| No. | Atom | Coordinates(fractional) |          |          | Experimental magnetic moments |          | Calculated magnetic moments |           |           |          |
|-----|------|-------------------------|----------|----------|-------------------------------|----------|-----------------------------|-----------|-----------|----------|
| 1   | Sr   | 0.020200                | 0.250000 | 0.996900 | 0.000000                      | 0.000000 | 0.000000                    | -0.000000 | 0.000000  | 0.008000 |
| 2   | Sr   | 0.479800                | 0.750000 | 0.496900 | 0.000000                      | 0.000000 | 0.000000                    | 0.000000  | -0.000000 | 0.008000 |
| 3   | Sr   | 0.979800                | 0.750000 | 0.003100 | 0.000000                      | 0.000000 | 0.000000                    | -0.000000 | -0.000000 | 0.008000 |
| 4   | Sr   | 0.520200                | 0.250000 | 0.503100 | 0.000000                      | 0.000000 | 0.000000                    | 0.000000  | 0.000000  | 0.008000 |
| 5   | Ru   | 0.000000                | 0.000000 | 0.500000 | 0.000000                      | 0.000000 | 1.629970                    | -0.061000 | -0.069000 | 1.420000 |
| 6   | Ru   | 0.500000                | 0.000000 | 0.000000 | 0.000000                      | 0.000000 | 1.629970                    | 0.061000  | 0.071000  | 1.425000 |
| 7   | Ru   | 0.500000                | 0.500000 | 0.000000 | 0.000000                      | 0.000000 | 1.629970                    | 0.061000  | -0.069000 | 1.420000 |
| 8   | Ru   | 0.000000                | 0.500000 | 0.500000 | 0.000000                      | 0.000000 | 1.629970                    | -0.061000 | 0.071000  | 1.425000 |
| 9   | O    | 0.996000                | 0.250000 | 0.444300 | 0.000000                      | 0.000000 | 0.000000                    | -0.005000 | -0.000000 | 0.150000 |
| 10  | O    | 0.504000                | 0.750000 | 0.944300 | 0.000000                      | 0.000000 | 0.000000                    | 0.005000  | 0.000000  | 0.149000 |
| 11  | O    | 0.004000                | 0.750000 | 0.555700 | 0.000000                      | 0.000000 | 0.000000                    | -0.005000 | 0.000000  | 0.149000 |
| 12  | O    | 0.496000                | 0.250000 | 0.055700 | 0.000000                      | 0.000000 | 0.000000                    | 0.005000  | -0.000000 | 0.150000 |
| 13  | O    | 0.221100                | 0.971900 | 0.221800 | 0.000000                      | 0.000000 | 0.000000                    | 0.002000  | 0.000000  | 0.148000 |
| 14  | O    | 0.278900                | 0.028100 | 0.721800 | 0.000000                      | 0.000000 | 0.000000                    | -0.001000 | 0.001000  | 0.149000 |
| 15  | O    | 0.778900                | 0.028100 | 0.778200 | 0.000000                      | 0.000000 | 0.000000                    | 0.002000  | -0.001000 | 0.146000 |
| 16  | O    | 0.721100                | 0.971900 | 0.278200 | 0.000000                      | 0.000000 | 0.000000                    | -0.002000 | 0.000000  | 0.146000 |
| 17  | O    | 0.721100                | 0.528100 | 0.278200 | 0.000000                      | 0.000000 | 0.000000                    | -0.002000 | 0.000000  | 0.148000 |
| 18  | O    | 0.778900                | 0.471900 | 0.778200 | 0.000000                      | 0.000000 | 0.000000                    | 0.001000  | 0.001000  | 0.149000 |
| 19  | O    | 0.278900                | 0.471900 | 0.721800 | 0.000000                      | 0.000000 | 0.000000                    | -0.002000 | -0.001000 | 0.146000 |
| 20  | O    | 0.221100                | 0.528100 | 0.221800 | 0.000000                      | 0.000000 | 0.000000                    | 0.002000  | 0.000000  | 0.146000 |

FIG. 48. First-principles calculation results of 0.732 SrRuO<sub>3</sub>. The band structure is shown in the left panel, and the Fermi-level-dependent AHC is plotted in the right panel. In both plots, the Fermi level is set to 0 eV.

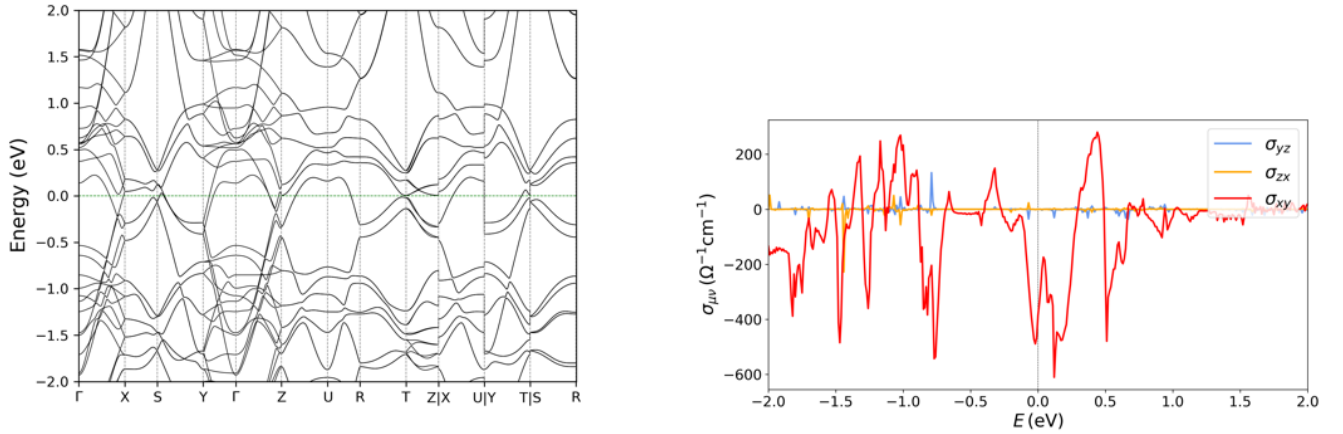

**0.778 LaMnSi<sub>2</sub>** crystallizes in type III MSG 63.464, which hosts only FNSs. The symmetry-adapted AHC tensor of the MSG is  $(0, \sigma_{zx}, 0)$ . Based on the first-principles calculation results, the comparison between the experimental and calculated magnetic moments is provided in Table SII51. The band structure is shown in the left panel of Fig. 49, and the Fermi-level-dependent AHC is plotted in the right panel.

TABLE SII51. The comparison between the experimental and calculated magnetic moments for 0.778 LaMnSi<sub>2</sub>. The five columns contain the atom index in the structure file, the atom species, the fractional coordinates, the experimental magnetic moments, and the calculated magnetic moments. The lattice vectors are  $\vec{a}_1 = (2.0955, -8.84, 0.0)$ ,  $\vec{a}_2 = (2.0955, 8.84, 0.0)$ ,  $\vec{a}_3 = (0.0, 0.0, 4.073)$ .

| No. | Atom | Coordinates(fractional) |          |          | Experimental magnetic moments |          |          | Calculated magnetic moments |           |           |
|-----|------|-------------------------|----------|----------|-------------------------------|----------|----------|-----------------------------|-----------|-----------|
| 1   | La   | 0.899000                | 0.101000 | 0.250000 | 0.000000                      | 0.000000 | 0.000000 | 0.000000                    | -0.014000 | -0.000000 |
| 2   | La   | 0.101000                | 0.899000 | 0.750000 | 0.000000                      | 0.000000 | 0.000000 | -0.000000                   | -0.014000 | -0.000000 |
| 3   | Mn   | 0.249000                | 0.751000 | 0.250000 | 0.000000                      | 2.069970 | 0.000000 | -0.006000                   | 2.092000  | -0.000000 |
| 4   | Mn   | 0.751000                | 0.249000 | 0.750000 | 0.000000                      | 2.069970 | 0.000000 | 0.006000                    | 2.092000  | -0.000000 |
| 5   | Si   | 0.676000                | 0.324000 | 0.250000 | 0.000000                      | 0.000000 | 0.000000 | -0.000000                   | -0.081000 | -0.000000 |
| 6   | Si   | 0.324000                | 0.676000 | 0.750000 | 0.000000                      | 0.000000 | 0.000000 | 0.000000                    | -0.081000 | -0.000000 |
| 7   | Si   | 0.535000                | 0.465000 | 0.250000 | 0.000000                      | 0.000000 | 0.000000 | 0.001000                    | -0.003000 | -0.000000 |
| 8   | Si   | 0.465000                | 0.535000 | 0.750000 | 0.000000                      | 0.000000 | 0.000000 | -0.001000                   | -0.003000 | -0.000000 |

FIG. 49. First-principles calculation results of 0.778 LaMnSi<sub>2</sub>. The band structure is shown in the left panel, and the Fermi-level-dependent AHC is plotted in the right panel. In both plots, the Fermi level is set to 0 eV.

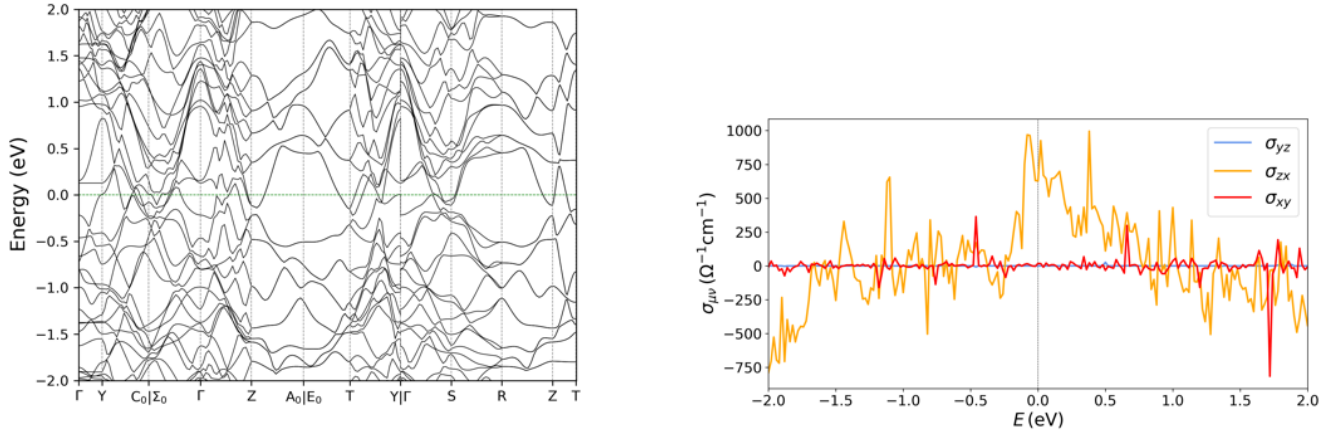



**0.779 LaMnSi<sub>2</sub>** crystallizes in type III MSG 63.464, which hosts only FNSs. The symmetry-adapted AHC tensor of the MSG is  $(0, \sigma_{zx}, 0)$ . Based on the first-principles calculation results, the comparison between the experimental and calculated magnetic moments is provided in Table SII52. The band structure is shown in the left panel of Fig. 50, and the Fermi-level-dependent AHC is plotted in the right panel.

TABLE SII52. The comparison between the experimental and calculated magnetic moments for 0.779 LaMnSi<sub>2</sub>. The five columns contain the atom index in the structure file, the atom species, the fractional coordinates, the experimental magnetic moments, and the calculated magnetic moments. The lattice vectors are  $\vec{a}_1 = (2.0955, -8.84, 0.0)$ ,  $\vec{a}_2 = (2.0955, 8.84, 0.0)$ ,  $\vec{a}_3 = (0.0, 0.0, 4.073)$ .

| No. | Atom | Coordinates(fractional) |          |          | Experimental magnetic moments |          |          | Calculated magnetic moments |           |           |
|-----|------|-------------------------|----------|----------|-------------------------------|----------|----------|-----------------------------|-----------|-----------|
| 1   | La   | 0.899000                | 0.101000 | 0.250000 | 0.000000                      | 0.000000 | 0.000000 | 0.000000                    | -0.014000 | -0.000000 |
| 2   | La   | 0.101000                | 0.899000 | 0.750000 | 0.000000                      | 0.000000 | 0.000000 | -0.000000                   | -0.014000 | -0.000000 |
| 3   | Mn   | 0.249000                | 0.751000 | 0.250000 | 0.000000                      | 2.030020 | 0.000000 | -0.006000                   | 2.092000  | -0.000000 |
| 4   | Mn   | 0.751000                | 0.249000 | 0.750000 | 0.000000                      | 2.030020 | 0.000000 | 0.006000                    | 2.092000  | -0.000000 |
| 5   | Si   | 0.676000                | 0.324000 | 0.250000 | 0.000000                      | 0.000000 | 0.000000 | -0.000000                   | -0.081000 | -0.000000 |
| 6   | Si   | 0.324000                | 0.676000 | 0.750000 | 0.000000                      | 0.000000 | 0.000000 | 0.000000                    | -0.081000 | -0.000000 |
| 7   | Si   | 0.535000                | 0.465000 | 0.250000 | 0.000000                      | 0.000000 | 0.000000 | 0.001000                    | -0.003000 | -0.000000 |
| 8   | Si   | 0.465000                | 0.535000 | 0.750000 | 0.000000                      | 0.000000 | 0.000000 | -0.001000                   | -0.003000 | -0.000000 |

FIG. 50. First-principles calculation results of 0.779 LaMnSi<sub>2</sub>. The band structure is shown in the left panel, and the Fermi-level-dependent AHC is plotted in the right panel. In both plots, the Fermi level is set to 0 eV.

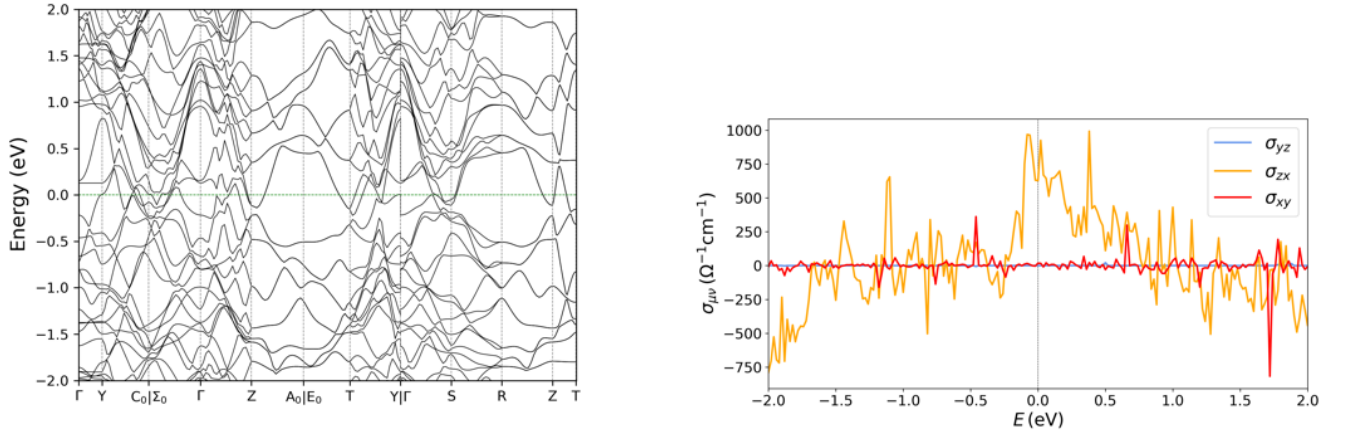

**0.780 LaMnSi<sub>2</sub>** crystallizes in type III MSG 63.464, which hosts only FNSs. The symmetry-adapted AHC tensor of the MSG is  $(0, \sigma_{zx}, 0)$ . Based on the first-principles calculation results, the comparison between the experimental and calculated magnetic moments is provided in Table SII53. The band structure is shown in the left panel of Fig. 51, and the Fermi-level-dependent AHC is plotted in the right panel.

TABLE SII53. The comparison between the experimental and calculated magnetic moments for 0.780 LaMnSi<sub>2</sub>. The five columns contain the atom index in the structure file, the atom species, the fractional coordinates, the experimental magnetic moments, and the calculated magnetic moments. The lattice vectors are  $\vec{a}_1 = (2.0955, -8.84, 0.0)$ ,  $\vec{a}_2 = (2.0955, 8.84, 0.0)$ ,  $\vec{a}_3 = (0.0, 0.0, 4.073)$ .

| No. | Atom | Coordinates(fractional) |          |          | Experimental magnetic moments |          |          | Calculated magnetic moments |           |           |
|-----|------|-------------------------|----------|----------|-------------------------------|----------|----------|-----------------------------|-----------|-----------|
| 1   | La   | 0.899000                | 0.101000 | 0.250000 | 0.000000                      | 0.000000 | 0.000000 | 0.000000                    | -0.014000 | -0.000000 |
| 2   | La   | 0.101000                | 0.899000 | 0.750000 | 0.000000                      | 0.000000 | 0.000000 | -0.000000                   | -0.014000 | -0.000000 |
| 3   | Mn   | 0.249000                | 0.751000 | 0.250000 | 0.000000                      | 1.769940 | 0.000000 | -0.006000                   | 2.092000  | -0.000000 |
| 4   | Mn   | 0.751000                | 0.249000 | 0.750000 | 0.000000                      | 1.769940 | 0.000000 | 0.006000                    | 2.092000  | -0.000000 |
| 5   | Si   | 0.676000                | 0.324000 | 0.250000 | 0.000000                      | 0.000000 | 0.000000 | -0.000000                   | -0.081000 | -0.000000 |
| 6   | Si   | 0.324000                | 0.676000 | 0.750000 | 0.000000                      | 0.000000 | 0.000000 | 0.000000                    | -0.081000 | -0.000000 |
| 7   | Si   | 0.535000                | 0.465000 | 0.250000 | 0.000000                      | 0.000000 | 0.000000 | 0.001000                    | -0.003000 | -0.000000 |
| 8   | Si   | 0.465000                | 0.535000 | 0.750000 | 0.000000                      | 0.000000 | 0.000000 | -0.001000                   | -0.003000 | -0.000000 |

FIG. 51. First-principles calculation results of 0.780 LaMnSi<sub>2</sub>. The band structure is shown in the left panel, and the Fermi-level-dependent AHC is plotted in the right panel. In both plots, the Fermi level is set to 0 eV.

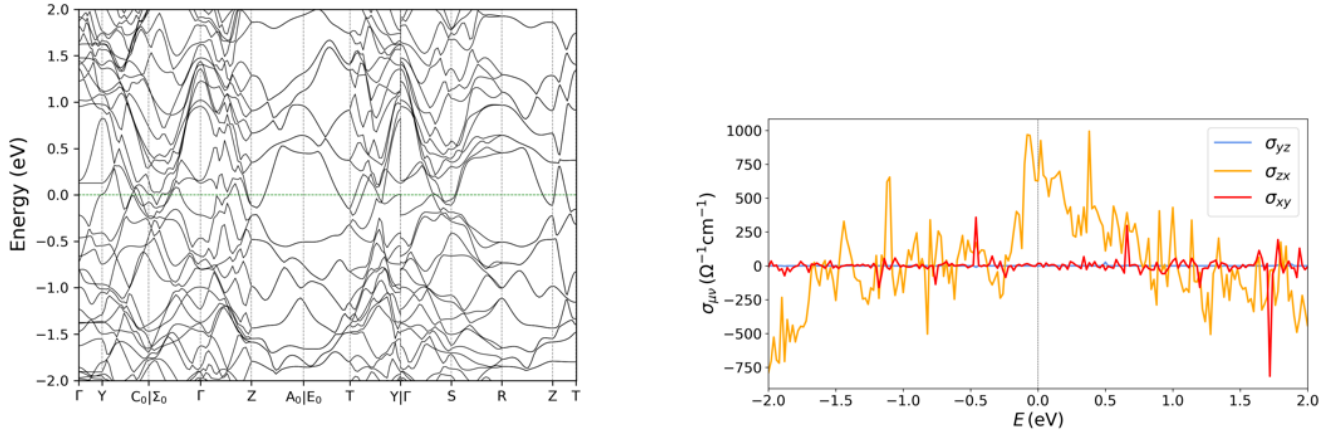

**0.781 CeMnSi<sub>2</sub>** crystallizes in type III MSG 63.464, which hosts only FNSs. The symmetry-adapted AHC tensor of the MSG is  $(0, \sigma_{zx}, 0)$ . Based on the first-principles calculation results, the comparison between the experimental and calculated magnetic moments is provided in Table SII54. The band structure is shown in the left panel of Fig. 52, and the Fermi-level-dependent AHC is plotted in the right panel.

TABLE SII54. The comparison between the experimental and calculated magnetic moments for 0.781 CeMnSi<sub>2</sub>. The five columns contain the atom index in the structure file, the atom species, the fractional coordinates, the experimental magnetic moments, and the calculated magnetic moments. The lattice vectors are  $\vec{a}_1 = (2.0517, -8.7445, 0.0)$ ,  $\vec{a}_2 = (2.0517, 8.7445, 0.0)$ ,  $\vec{a}_3 = (0.0, 0.0, 4.0267)$ .

| No. | Atom | Coordinates(fractional) |          |          | Experimental magnetic moments |           |          | Calculated magnetic moments |           |           |
|-----|------|-------------------------|----------|----------|-------------------------------|-----------|----------|-----------------------------|-----------|-----------|
| 1   | Ce   | 0.898700                | 0.101300 | 0.250000 | 0.000000                      | -0.100040 | 0.000000 | 0.005000                    | -0.139000 | 0.000000  |
| 2   | Ce   | 0.101300                | 0.898700 | 0.750000 | 0.000000                      | -0.100040 | 0.000000 | -0.004000                   | -0.139000 | -0.000000 |
| 3   | Mn   | 0.249000                | 0.751000 | 0.250000 | 0.000000                      | 2.699950  | 0.000000 | -0.005000                   | 3.925000  | 0.001000  |
| 4   | Mn   | 0.751000                | 0.249000 | 0.750000 | 0.000000                      | 2.699950  | 0.000000 | 0.005000                    | 3.925000  | -0.000000 |
| 5   | Si   | 0.535000                | 0.465000 | 0.250000 | 0.000000                      | 0.000000  | 0.000000 | 0.001000                    | -0.016000 | -0.000000 |
| 6   | Si   | 0.465000                | 0.535000 | 0.750000 | 0.000000                      | 0.000000  | 0.000000 | -0.001000                   | -0.016000 | -0.000000 |
| 7   | Si   | 0.675400                | 0.324600 | 0.250000 | 0.000000                      | 0.000000  | 0.000000 | 0.001000                    | -0.119000 | -0.000000 |
| 8   | Si   | 0.324600                | 0.675400 | 0.750000 | 0.000000                      | 0.000000  | 0.000000 | -0.001000                   | -0.119000 | -0.000000 |

FIG. 52. First-principles calculation results of 0.781 CeMnSi<sub>2</sub>. The band structure is shown in the left panel, and the Fermi-level-dependent AHC is plotted in the right panel. In both plots, the Fermi level is set to 0 eV.

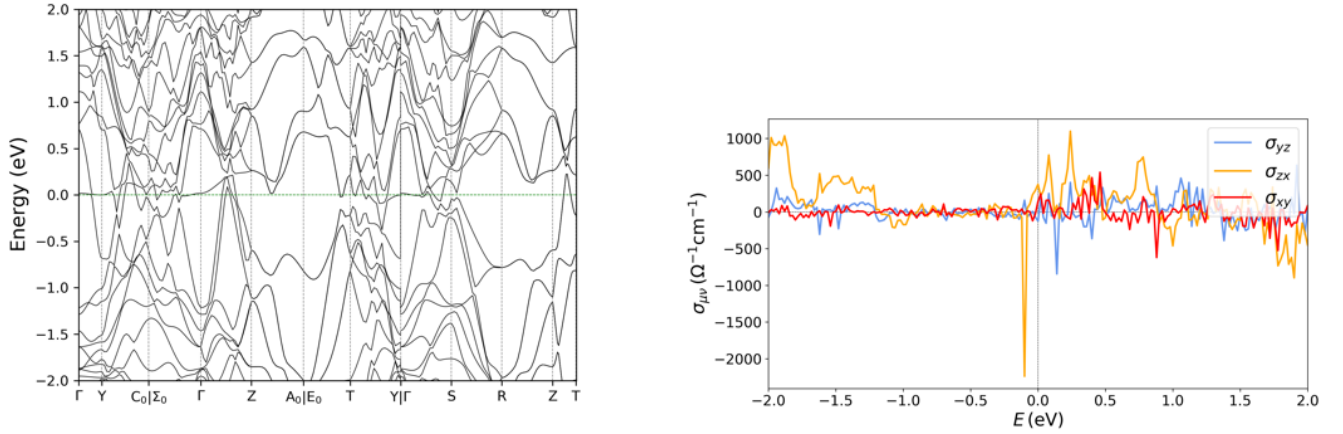

0.796  $\text{Ca}_2\text{NiOsO}_6$  crystallizes in type III MSG 14.79, which hosts both SNLs and FNSs. The symmetry-adapted AHC tensor of the MSG is  $(\sigma_{yz}, \sigma_{zx}, 0)$ . Based on the first-principles calculation results, the comparison between the experimental and calculated magnetic moments is provided in Table SII55. The band structure is shown in the left panel of Fig. 53, and the Fermi-level-dependent AHC is plotted in the right panel.

TABLE SII55. The comparison between the experimental and calculated magnetic moments for 0.796  $\text{Ca}_2\text{NiOsO}_6$ . The five columns contain the atom index in the structure file, the atom species, the fractional coordinates, the experimental magnetic moments, and the calculated magnetic moments. The lattice vectors are  $\vec{a}_1 = (5.3608, 0.0, 0.0)$ ,  $\vec{a}_2 = (0.0, 5.543, 0.0)$ ,  $\vec{a}_3 = (-5.322243315, 0.0, 7.617501343)$ .

| No. | Atom | Coordinates(fractional) |          |          | Experimental magnetic moments |          |          | Calculated magnetic moments |           |           |
|-----|------|-------------------------|----------|----------|-------------------------------|----------|----------|-----------------------------|-----------|-----------|
| 1   | Ca   | 0.738600                | 0.443300 | 0.250900 | 0.000000                      | 0.000000 | 0.000000 | -0.011000                   | -0.001000 | -0.001000 |
| 2   | Ca   | 0.261400                | 0.556700 | 0.749100 | 0.000000                      | 0.000000 | 0.000000 | -0.010000                   | -0.001000 | -0.001000 |
| 3   | Ca   | 0.261400                | 0.943300 | 0.249100 | 0.000000                      | 0.000000 | 0.000000 | -0.011000                   | 0.001000  | -0.001000 |
| 4   | Ca   | 0.738600                | 0.056700 | 0.750900 | 0.000000                      | 0.000000 | 0.000000 | -0.011000                   | 0.001000  | -0.001000 |
| 5   | Ni   | 0.500000                | 0.000000 | 0.000000 | 2.599990                      | 0.000000 | 0.000000 | 2.074000                    | -0.001000 | 0.001000  |
| 6   | Ni   | 0.500000                | 0.500000 | 0.500000 | 2.599990                      | 0.000000 | 0.000000 | 2.074000                    | 0.001000  | 0.001000  |
| 7   | Os   | 0.000000                | 0.000000 | 0.500000 | -1.410000                     | 0.000000 | 0.000000 | -2.005000                   | -0.001000 | 0.000000  |
| 8   | Os   | 0.000000                | 0.500000 | 0.000000 | -1.410000                     | 0.000000 | 0.000000 | -2.005000                   | 0.001000  | 0.000000  |
| 9   | O    | 0.851600                | 0.027000 | 0.258400 | 0.000000                      | 0.000000 | 0.000000 | -0.000000                   | -0.001000 | -0.000000 |
| 10  | O    | 0.148400                | 0.973000 | 0.741600 | 0.000000                      | 0.000000 | 0.000000 | -0.000000                   | -0.001000 | -0.000000 |
| 11  | O    | 0.148400                | 0.527000 | 0.241600 | 0.000000                      | 0.000000 | 0.000000 | -0.000000                   | 0.001000  | -0.000000 |
| 12  | O    | 0.851600                | 0.473000 | 0.758400 | 0.000000                      | 0.000000 | 0.000000 | -0.000000                   | 0.001000  | -0.000000 |
| 13  | O    | 0.665200                | 0.194000 | 0.454700 | 0.000000                      | 0.000000 | 0.000000 | -0.009000                   | 0.004000  | -0.001000 |
| 14  | O    | 0.334800                | 0.806000 | 0.545300 | 0.000000                      | 0.000000 | 0.000000 | -0.010000                   | 0.004000  | -0.002000 |
| 15  | O    | 0.334800                | 0.694000 | 0.045300 | 0.000000                      | 0.000000 | 0.000000 | -0.010000                   | -0.004000 | -0.002000 |
| 16  | O    | 0.665200                | 0.306000 | 0.954700 | 0.000000                      | 0.000000 | 0.000000 | -0.009000                   | -0.004000 | -0.001000 |
| 17  | O    | 0.238800                | 0.285500 | 0.548000 | 0.000000                      | 0.000000 | 0.000000 | -0.004000                   | -0.004000 | 0.000000  |
| 18  | O    | 0.761200                | 0.714500 | 0.452000 | 0.000000                      | 0.000000 | 0.000000 | -0.004000                   | -0.005000 | 0.001000  |
| 19  | O    | 0.761200                | 0.785500 | 0.952000 | 0.000000                      | 0.000000 | 0.000000 | -0.003000                   | 0.004000  | 0.001000  |
| 20  | O    | 0.238800                | 0.214500 | 0.048000 | 0.000000                      | 0.000000 | 0.000000 | -0.005000                   | 0.005000  | 0.000000  |

FIG. 53. First-principles calculation results of 0.796  $\text{Ca}_2\text{NiOsO}_6$ . The band structure is shown in the left panel, and the Fermi-level-dependent AHC is plotted in the right panel. In both plots, the Fermi level is set to 0 eV.

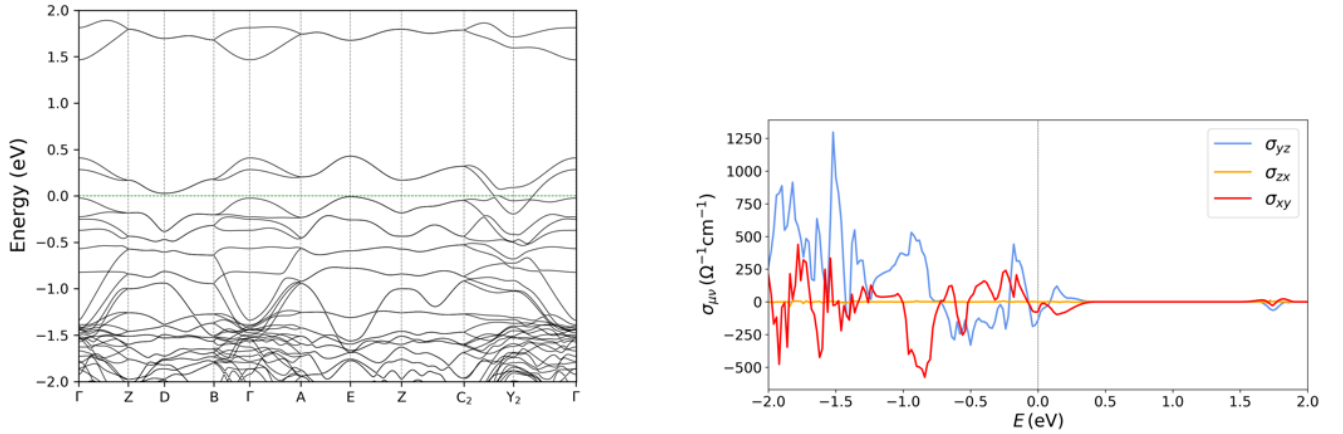

**0.803 NbMnP** crystallizes in type III MSG 31.125, which hosts both SNLs and FNSs. The symmetry-adapted AHC tensor of the MSG is  $(0, \sigma_{zx}, 0)$ . Based on the first-principles calculation results, the comparison between the experimental and calculated magnetic moments is provided in Table SII56. The band structure is shown in the left panel of Fig. 54, and the Fermi-level-dependent AHC is plotted in the right panel.

TABLE SII56. The comparison between the experimental and calculated magnetic moments for 0.803 NbMnP. The five columns contain the atom index in the structure file, the atom species, the fractional coordinates, the experimental magnetic moments, and the calculated magnetic moments. The lattice vectors are  $\vec{a}_1 = (3.5325, 0.0, 0.0)$ ,  $\vec{a}_2 = (0.0, 6.1661, 0.0)$ ,  $\vec{a}_3 = (0.0, 0.0, 7.2199)$ .

| No. | Atom | Coordinates(fractional) |          |          | Experimental magnetic moments |           |           | Calculated magnetic moments |           |           |
|-----|------|-------------------------|----------|----------|-------------------------------|-----------|-----------|-----------------------------|-----------|-----------|
| 1   | Mn   | 0.000000                | 0.108900 | 0.559500 | 0.000000                      | -0.830020 | 0.880030  | 0.010000                    | -1.394000 | 1.492000  |
| 2   | Mn   | 0.500000                | 0.891100 | 0.059500 | 0.000000                      | -0.830020 | -0.880030 | 0.010000                    | -1.394000 | -1.492000 |
| 3   | Mn   | 0.000000                | 0.608900 | 0.940500 | 0.000000                      | 0.830020  | -0.880030 | 0.007000                    | 1.393000  | -1.493000 |
| 4   | Mn   | 0.500000                | 0.391100 | 0.440500 | 0.000000                      | 0.830020  | 0.880030  | 0.007000                    | 1.393000  | 1.493000  |
| 5   | Nb   | 0.000000                | 0.218300 | 0.171500 | 0.000000                      | 0.000000  | 0.000000  | -0.001000                   | 0.044000  | -0.056000 |
| 6   | Nb   | 0.500000                | 0.781700 | 0.671500 | 0.000000                      | 0.000000  | 0.000000  | -0.001000                   | 0.044000  | 0.056000  |
| 7   | Nb   | 0.000000                | 0.718300 | 0.328500 | 0.000000                      | 0.000000  | 0.000000  | -0.003000                   | -0.044000 | 0.055000  |
| 8   | Nb   | 0.500000                | 0.281700 | 0.828500 | 0.000000                      | 0.000000  | 0.000000  | -0.003000                   | -0.044000 | -0.055000 |
| 9   | P    | 0.000000                | 0.982600 | 0.868800 | 0.000000                      | 0.000000  | 0.000000  | 0.000000                    | 0.006000  | 0.013000  |
| 10  | P    | 0.500000                | 0.017400 | 0.368800 | 0.000000                      | 0.000000  | 0.000000  | 0.000000                    | 0.006000  | -0.013000 |
| 11  | P    | 0.000000                | 0.482600 | 0.631200 | 0.000000                      | 0.000000  | 0.000000  | 0.000000                    | -0.006000 | -0.013000 |
| 12  | P    | 0.500000                | 0.517400 | 0.131200 | 0.000000                      | 0.000000  | 0.000000  | 0.000000                    | -0.006000 | 0.013000  |

FIG. 54. First-principles calculation results of 0.803 NbMnP. The band structure is shown in the left panel, and the Fermi-level-dependent AHC is plotted in the right panel. In both plots, the Fermi level is set to 0 eV.

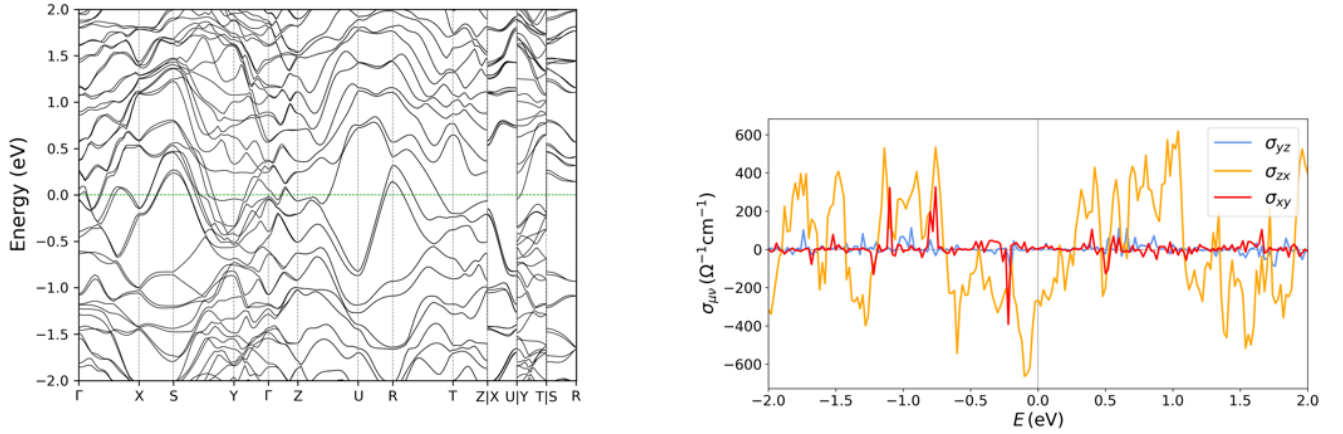

**0.834 CrSbSe<sub>3</sub>** crystallizes in type III MSG 62.447, which hosts both SNLs and FNSs. The symmetry-adapted AHC tensor of the MSG is  $(\sigma_{yz}, 0, 0)$ . Based on the first-principles calculation results, the comparison between the experimental and calculated magnetic moments is provided in Table SII57. The band structure is shown in the left panel of Fig. 55, and the Fermi-level-dependent AHC is plotted in the right panel.

TABLE SII57. The comparison of experimental magnetic moments and calculated magnetic moments for 0.834 CrSbSe<sub>3</sub>. The five columns contain the sequence number of the atom in the structure data, the atom name, the fractional coordinates, the experimental magnetic moments, and the calculated magnetic moments.

| No. | Atom | Coordinates(fractional) |          |          | Experimental magnetic moments |          |          | Calculated magnetic moments |           |           |
|-----|------|-------------------------|----------|----------|-------------------------------|----------|----------|-----------------------------|-----------|-----------|
| 1   | Cr   | 0.656850                | 0.250000 | 0.043890 | 3.060020                      | 0.000000 | 0.000000 | 3.772000                    | -0.000000 | 0.000000  |
| 2   | Cr   | 0.156850                | 0.250000 | 0.456110 | 3.060020                      | 0.000000 | 0.000000 | 3.775000                    | 0.000000  | 0.000000  |
| 3   | Cr   | 0.343150                | 0.750000 | 0.956110 | 3.060020                      | 0.000000 | 0.000000 | 3.772000                    | 0.000000  | -0.000000 |
| 4   | Cr   | 0.843150                | 0.750000 | 0.543890 | 3.060020                      | 0.000000 | 0.000000 | 3.775000                    | -0.000000 | -0.000000 |
| 5   | Sb   | 0.528840                | 0.250000 | 0.658490 | 0.000000                      | 0.000000 | 0.000000 | 0.014000                    | -0.000000 | -0.000000 |
| 6   | Sb   | 0.028840                | 0.250000 | 0.841510 | 0.000000                      | 0.000000 | 0.000000 | 0.015000                    | -0.000000 | -0.000000 |
| 7   | Sb   | 0.471160                | 0.750000 | 0.341510 | 0.000000                      | 0.000000 | 0.000000 | 0.015000                    | 0.000000  | 0.000000  |
| 8   | Sb   | 0.971160                | 0.750000 | 0.158490 | 0.000000                      | 0.000000 | 0.000000 | 0.015000                    | 0.000000  | -0.000000 |
| 9   | Se   | 0.000760                | 0.250000 | 0.608230 | 0.000000                      | 0.000000 | 0.000000 | -0.380000                   | -0.001000 | -0.001000 |
| 10  | Se   | 0.500760                | 0.250000 | 0.891770 | 0.000000                      | 0.000000 | 0.000000 | -0.381000                   | 0.000000  | -0.000000 |
| 11  | Se   | 0.999240                | 0.750000 | 0.391770 | 0.000000                      | 0.000000 | 0.000000 | -0.380000                   | 0.001000  | 0.001000  |
| 12  | Se   | 0.499240                | 0.750000 | 0.108230 | 0.000000                      | 0.000000 | 0.000000 | -0.380000                   | -0.000000 | 0.001000  |
| 13  | Se   | 0.785860                | 0.250000 | 0.213920 | 0.000000                      | 0.000000 | 0.000000 | -0.129000                   | -0.000000 | -0.002000 |
| 14  | Se   | 0.285860                | 0.250000 | 0.286080 | 0.000000                      | 0.000000 | 0.000000 | -0.128000                   | 0.000000  | -0.002000 |
| 15  | Se   | 0.214140                | 0.750000 | 0.786080 | 0.000000                      | 0.000000 | 0.000000 | -0.129000                   | 0.000000  | 0.002000  |
| 16  | Se   | 0.714140                | 0.750000 | 0.713920 | 0.000000                      | 0.000000 | 0.000000 | -0.128000                   | -0.000000 | 0.002000  |
| 17  | Se   | 0.671140                | 0.250000 | 0.484030 | 0.000000                      | 0.000000 | 0.000000 | -0.188000                   | -0.000000 | 0.001000  |
| 18  | Se   | 0.171140                | 0.250000 | 0.015970 | 0.000000                      | 0.000000 | 0.000000 | -0.187000                   | 0.000000  | 0.000000  |
| 19  | Se   | 0.328860                | 0.750000 | 0.515970 | 0.000000                      | 0.000000 | 0.000000 | -0.187000                   | -0.000000 | -0.000000 |
| 20  | Se   | 0.828860                | 0.750000 | 0.984030 | 0.000000                      | 0.000000 | 0.000000 | -0.188000                   | -0.000000 | -0.001000 |

FIG. 55. First-principles calculation results of 0.834 CrSbSe<sub>3</sub>. The band structure is shown in the left panel, and the Fermi-level-dependent AHC is plotted in the right panel. In both plots, the Fermi level is set to 0 eV.

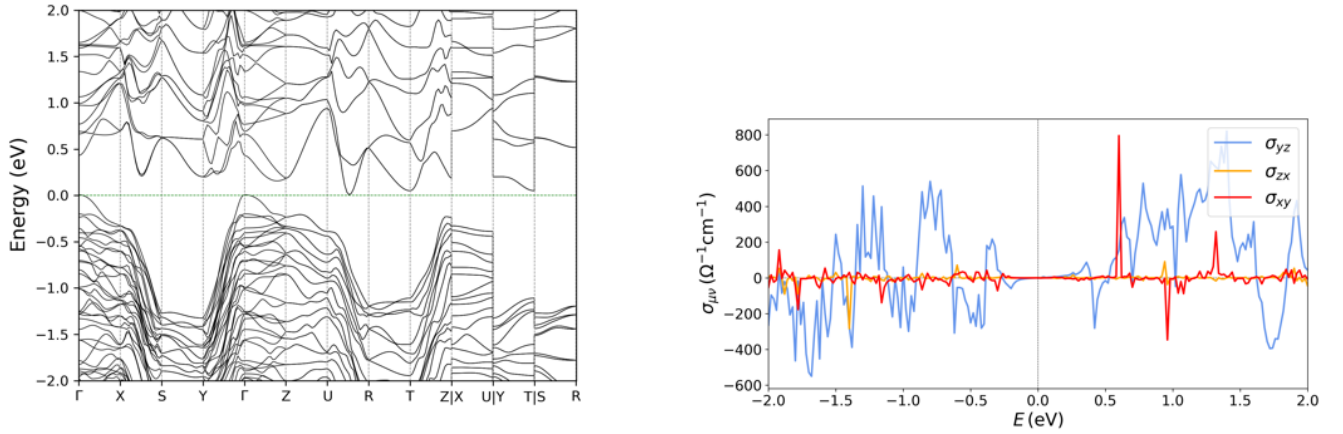

**0.855 Mn<sub>2</sub>Sb** crystallizes in type III MSG 129.417, which hosts only FNSs. The symmetry-adapted AHC tensor of the MSG is  $(0, 0, \sigma_{xy})$ . Based on the first-principles calculation results, the comparison between the experimental and calculated magnetic moments is provided in Table SII58. The band structure is shown in the left panel of Fig. 56, and the Fermi-level-dependent AHC is plotted in the right panel.

TABLE SII58. The comparison between the experimental and calculated magnetic moments for 0.855 Mn<sub>2</sub>Sb. The five columns contain the atom index in the structure file, the atom species, the fractional coordinates, the experimental magnetic moments, and the calculated magnetic moments. The lattice vectors are  $\vec{a}_1 = (4.078, 0.0, 0.0)$ ,  $\vec{a}_2 = (0.0, 4.078, 0.0)$ ,  $\vec{a}_3 = (0.0, 0.0, 6.557)$ .

| No. | Atom | Coordinates(fractional) |          |          | Experimental magnetic moments |          |           | Calculated magnetic moments |           |           |
|-----|------|-------------------------|----------|----------|-------------------------------|----------|-----------|-----------------------------|-----------|-----------|
| 1   | Mn   | 0.750000                | 0.250000 | 0.000000 | 0.000000                      | 0.000000 | 2.100010  | -0.000000                   | -0.001000 | 3.514000  |
| 2   | Mn   | 0.250000                | 0.750000 | 0.000000 | 0.000000                      | 0.000000 | 2.100010  | 0.000000                    | 0.001000  | 3.513000  |
| 3   | Mn   | 0.250000                | 0.250000 | 0.705000 | 0.000000                      | 0.000000 | -3.899970 | 0.000000                    | -0.000000 | -4.678000 |
| 4   | Mn   | 0.750000                | 0.750000 | 0.295000 | 0.000000                      | 0.000000 | -3.899970 | -0.000000                   | 0.000000  | -4.678000 |
| 5   | Sb   | 0.250000                | 0.250000 | 0.280000 | 0.000000                      | 0.000000 | 0.000000  | 0.002000                    | 0.000000  | 0.040000  |
| 6   | Sb   | 0.750000                | 0.750000 | 0.720000 | 0.000000                      | 0.000000 | 0.000000  | -0.002000                   | 0.001000  | 0.040000  |

FIG. 56. First-principles calculation results of 0.855 Mn<sub>2</sub>Sb. The band structure is shown in the left panel, and the Fermi-level-dependent AHC is plotted in the right panel. In both plots, the Fermi level is set to 0 eV.

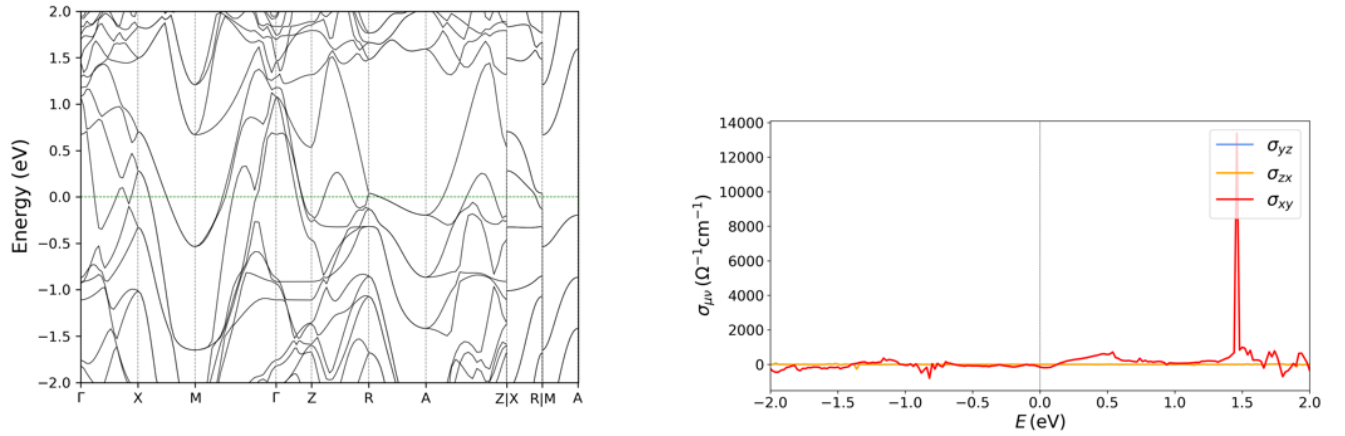



**0.985 EuPd<sub>3</sub>Si<sub>2</sub>** crystallizes in type III MSG 74.559, which hosts only SNLs. The symmetry-adapted AHC tensor of the MSG is  $(\sigma_{yz}, 0, 0)$ . Based on the first-principles calculation results, the comparison between the experimental and calculated magnetic moments is provided in Table SII59. The band structure is shown in the left panel of Fig. 57, and the Fermi-level-dependent AHC is plotted in the right panel.

TABLE SII59. The comparison between the experimental and calculated magnetic moments for 0.985 EuPd<sub>3</sub>Si<sub>2</sub>. The five columns contain the atom index in the structure file, the atom species, the fractional coordinates, the experimental magnetic moments, and the calculated magnetic moments. The lattice vectors are  $\vec{a}_1 = (-3.57415, 5.03715, 2.8753)$ ,  $\vec{a}_2 = (3.57415, -5.03715, 2.8753)$ ,  $\vec{a}_3 = (3.57415, 5.03715, -2.8753)$ .

| No. | Atom | Coordinates(fractional) |          |          | Experimental magnetic moments |          |          | Calculated magnetic moments |           |           |
|-----|------|-------------------------|----------|----------|-------------------------------|----------|----------|-----------------------------|-----------|-----------|
| 1   | Eu   | 0.034600                | 0.784600 | 0.250000 | 8.000020                      | 0.000000 | 0.000000 | 7.632000                    | -0.000000 | 0.000000  |
| 2   | Eu   | 0.965400                | 0.215400 | 0.750000 | 8.000020                      | 0.000000 | 0.000000 | 7.632000                    | 0.000000  | -0.000000 |
| 3   | Pd   | 0.000000                | 0.795000 | 0.795000 | 0.000000                      | 0.000000 | 0.000000 | -0.023000                   | -0.000000 | -0.000000 |
| 4   | Pd   | 0.000000                | 0.205000 | 0.205000 | 0.000000                      | 0.000000 | 0.000000 | -0.022000                   | 0.000000  | 0.000000  |
| 5   | Pd   | 0.500000                | 0.205000 | 0.705000 | 0.000000                      | 0.000000 | 0.000000 | -0.022000                   | -0.001000 | -0.001000 |
| 6   | Pd   | 0.500000                | 0.795000 | 0.295000 | 0.000000                      | 0.000000 | 0.000000 | -0.022000                   | 0.001000  | 0.000000  |
| 7   | Pd   | 0.500000                | 0.500000 | 0.500000 | 0.000000                      | 0.000000 | 0.000000 | -0.014000                   | 0.000000  | 0.001000  |
| 8   | Pd   | 0.500000                | 0.000000 | 0.000000 | 0.000000                      | 0.000000 | 0.000000 | -0.014000                   | 0.000000  | -0.001000 |
| 9   | Si   | 0.263800                | 0.685200 | 0.578600 | 0.000000                      | 0.000000 | 0.000000 | -0.010000                   | 0.000000  | 0.001000  |
| 10  | Si   | 0.736200                | 0.314800 | 0.421400 | 0.000000                      | 0.000000 | 0.000000 | -0.009000                   | -0.000000 | -0.001000 |
| 11  | Si   | 0.393400                | 0.314800 | 0.078600 | 0.000000                      | 0.000000 | 0.000000 | -0.010000                   | -0.000000 | -0.000000 |
| 12  | Si   | 0.606600                | 0.685200 | 0.921400 | 0.000000                      | 0.000000 | 0.000000 | -0.010000                   | 0.000000  | 0.000000  |

FIG. 57. First-principles calculation results of 0.985 EuPd<sub>3</sub>Si<sub>2</sub>. The band structure is shown in the left panel, and the Fermi-level-dependent AHC is plotted in the right panel. In both plots, the Fermi level is set to 0 eV.

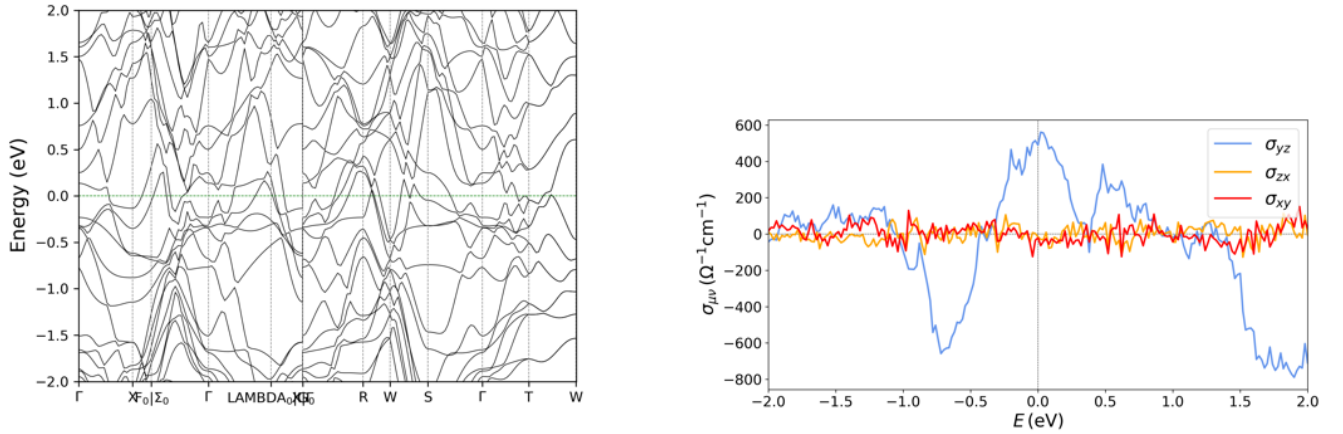

**2.12 TbMg** crystallizes in type III MSG 49.270, which hosts only SNLs. The symmetry-adapted AHC tensor of the MSG is  $(0, \sigma_{zx}, 0)$ . Based on the first-principles calculation results, the comparison between the experimental and calculated magnetic moments is provided in Table SII60. The band structure is shown in the left panel of Fig. 58, and the Fermi-level-dependent AHC is plotted in the right panel.

TABLE SII60. The comparison between the experimental and calculated magnetic moments for 2.12 TbMg. The five columns contain the atom index in the structure file, the atom species, the fractional coordinates, the experimental magnetic moments, and the calculated magnetic moments. The lattice vectors are  $\vec{a}_1 = (3.778, 0.0, 0.0)$ ,  $\vec{a}_2 = (0.0, 3.778, 0.0)$ ,  $\vec{a}_3 = (0.0, 0.0, 7.556)$ .

| No. | Atom | Coordinates(fractional) |          |          | Experimental magnetic moments |          |          | Calculated magnetic moments |          |           |
|-----|------|-------------------------|----------|----------|-------------------------------|----------|----------|-----------------------------|----------|-----------|
| 1   | Mg   | 0.500000                | 0.500000 | 0.250000 | 0.000000                      | 0.000000 | 0.000000 | 0.000000                    | 0.005000 | -0.003000 |
| 2   | Mg   | 0.500000                | 0.500000 | 0.750000 | 0.000000                      | 0.000000 | 0.000000 | -0.000000                   | 0.005000 | 0.003000  |
| 3   | Tb   | 0.000000                | 0.000000 | 0.000000 | -5.180020                     | 5.200000 | 0.000000 | -5.754000                   | 5.762000 | 0.000000  |
| 4   | Tb   | 0.000000                | 0.000000 | 0.500000 | 5.180020                      | 5.200000 | 0.000000 | 5.754000                    | 5.763000 | -0.000000 |

FIG. 58. First-principles calculation results of 2.12 TbMg. The band structure is shown in the left panel, and the Fermi-level-dependent AHC is plotted in the right panel. In both plots, the Fermi level is set to 0 eV.

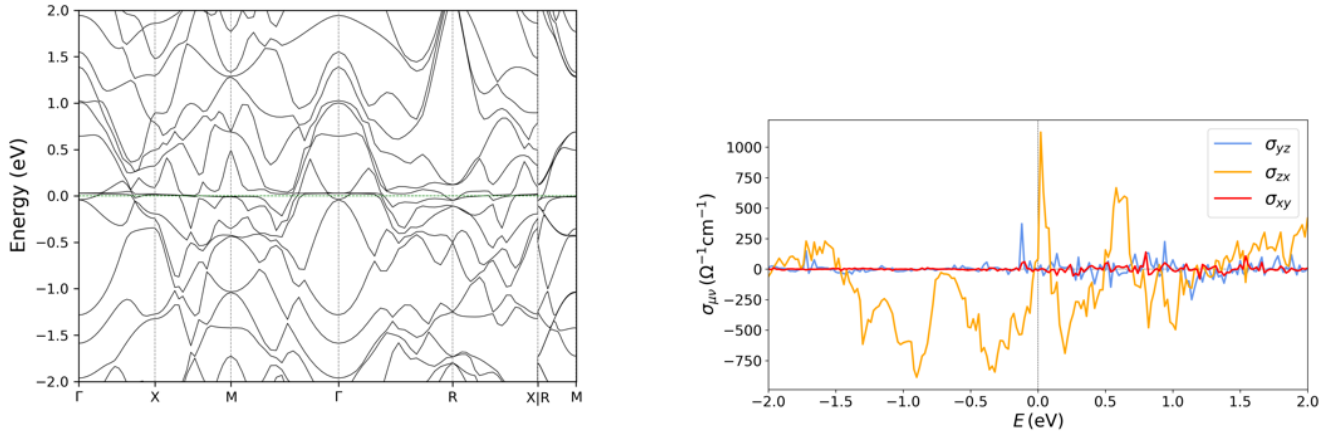

**2.97 GdMn<sub>2</sub>Si<sub>2</sub>** crystallizes in type III MSG 59.409, which hosts only FNSs. The symmetry-adapted AHC tensor of the MSG is  $(0, 0, \sigma_{xy})$ . Based on the first-principles calculation results, the comparison between the experimental and calculated magnetic moments is provided in Table SII61. The band structure is shown in the left panel of Fig. 59, and the Fermi-level-dependent AHC is plotted in the right panel.

TABLE SII61. The comparison between the experimental and calculated magnetic moments for 2.97 GdMn<sub>2</sub>Si<sub>2</sub>. The five columns contain the atom index in the structure file, the atom species, the fractional coordinates, the experimental magnetic moments, and the calculated magnetic moments. The lattice vectors are  $\vec{a}_1 = (10.489, 0.0, 0.0)$ ,  $\vec{a}_2 = (0.0, 3.954, 0.0)$ ,  $\vec{a}_3 = (0.0, 0.0, 3.954)$ .

| No. | Atom | Coordinates(fractional) |          |          | Experimental magnetic moments |          |           | Calculated magnetic moments |           |           |
|-----|------|-------------------------|----------|----------|-------------------------------|----------|-----------|-----------------------------|-----------|-----------|
| 1   | Gd   | 0.250000                | 0.250000 | 0.250000 | 0.000000                      | 0.000000 | 6.700010  | 0.002000                    | -0.001000 | 7.529000  |
| 2   | Gd   | 0.750000                | 0.750000 | 0.750000 | 0.000000                      | 0.000000 | 6.700010  | -0.002000                   | 0.001000  | 7.529000  |
| 3   | Mn   | 0.500000                | 0.250000 | 0.750000 | 1.899980                      | 0.000000 | -1.000010 | 3.019000                    | -0.008000 | -1.613000 |
| 4   | Mn   | 0.000000                | 0.250000 | 0.750000 | -1.899980                     | 0.000000 | -1.000010 | -3.023000                   | 0.006000  | -1.603000 |
| 5   | Mn   | 0.500000                | 0.750000 | 0.250000 | 1.899980                      | 0.000000 | -1.000010 | 3.023000                    | 0.008000  | -1.603000 |
| 6   | Mn   | 0.000000                | 0.750000 | 0.250000 | -1.899980                     | 0.000000 | -1.000010 | -3.018000                   | -0.006000 | -1.613000 |
| 7   | Si   | 0.633200                | 0.250000 | 0.250000 | 0.000000                      | 0.000000 | 0.000000  | -0.094000                   | 0.001000  | 0.009000  |
| 8   | Si   | 0.866800                | 0.250000 | 0.250000 | 0.000000                      | 0.000000 | 0.000000  | 0.095000                    | -0.001000 | 0.010000  |
| 9   | Si   | 0.366800                | 0.750000 | 0.750000 | 0.000000                      | 0.000000 | 0.000000  | -0.095000                   | -0.001000 | 0.010000  |
| 10  | Si   | 0.133200                | 0.750000 | 0.750000 | 0.000000                      | 0.000000 | 0.000000  | 0.094000                    | 0.001000  | 0.009000  |

FIG. 59. First-principles calculation results of 2.97 GdMn<sub>2</sub>Si<sub>2</sub>. The band structure is shown in the left panel, and the Fermi-level-dependent AHC is plotted in the right panel. In both plots, the Fermi level is set to 0 eV.

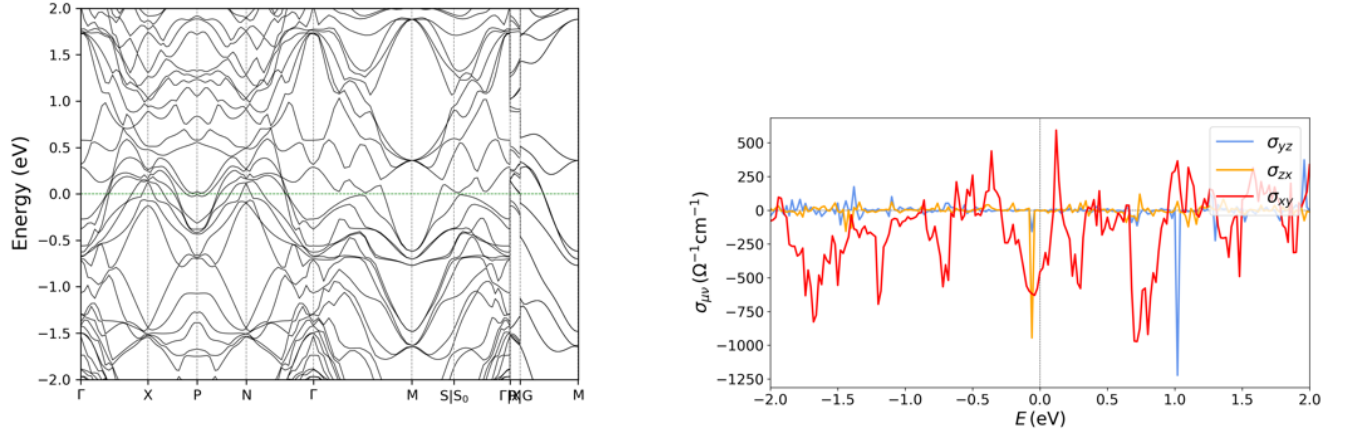

**0.11 DyFeO<sub>3</sub>** crystallizes in type III MSG 33.148, which hosts only SNLs. The symmetry-adapted AHC tensor of the MSG is  $(0, 0, \sigma_{xy})$ . Based on the first-principles calculation results, the comparison between the experimental and calculated magnetic moments is provided in Table SII62. The band structure is shown in the left panel of Fig. 60, and the Fermi-level-dependent AHC is plotted in the right panel.

TABLE SII62. The comparison between the experimental and calculated magnetic moments for 0.11 DyFeO<sub>3</sub>. The five columns contain the atom index in the structure file, the atom species, the fractional coordinates, the experimental magnetic moments, and the calculated magnetic moments. The lattice vectors are  $\vec{a}_1 = (5.5957, 0.0, 0.0)$ ,  $\vec{a}_2 = (0.0, 5.3009, 0.0)$ ,  $\vec{a}_3 = (0.0, 0.0, 7.629)$ .

| No. | Atom | Coordinates(fractional) |          |          | Experimental magnetic moments |          |          | Calculated magnetic moments |           |           |
|-----|------|-------------------------|----------|----------|-------------------------------|----------|----------|-----------------------------|-----------|-----------|
| 1   | Dy   | 0.933350                | 0.482750 | 0.250000 | -1.000010                     | 0.000000 | 0.000000 | -1.387000                   | 0.001000  | 0.008000  |
| 2   | Dy   | 0.066650                | 0.517250 | 0.750000 | 1.000010                      | 0.000000 | 0.000000 | 1.388000                    | -0.001000 | -0.000000 |
| 3   | Dy   | 0.566650                | 0.982750 | 0.750000 | 1.000010                      | 0.000000 | 0.000000 | 1.360000                    | -0.002000 | -0.007000 |
| 4   | Dy   | 0.433350                | 0.017250 | 0.250000 | -1.000010                     | 0.000000 | 0.000000 | -1.361000                   | 0.002000  | 0.002000  |
| 5   | Fe   | 0.000000                | 0.000000 | 0.000000 | -1.000010                     | 0.000000 | 0.299970 | -1.570000                   | 0.004000  | 0.478000  |
| 6   | Fe   | 0.000000                | 0.000000 | 0.500000 | 1.000010                      | 0.000000 | 0.299970 | 1.570000                    | -0.005000 | 0.478000  |
| 7   | Fe   | 0.500000                | 0.500000 | 0.500000 | 1.000010                      | 0.000000 | 0.299970 | 1.574000                    | 0.005000  | 0.478000  |
| 8   | Fe   | 0.500000                | 0.500000 | 0.000000 | -1.000010                     | 0.000000 | 0.299970 | -1.574000                   | -0.005000 | 0.478000  |
| 9   | O    | 0.537400                | 0.608100 | 0.250000 | 0.000000                      | 0.000000 | 0.000000 | -0.004000                   | -0.000000 | 0.003000  |
| 10  | O    | 0.462600                | 0.391900 | 0.750000 | 0.000000                      | 0.000000 | 0.000000 | 0.004000                    | 0.000000  | 0.004000  |
| 11  | O    | 0.962600                | 0.108100 | 0.750000 | 0.000000                      | 0.000000 | 0.000000 | 0.005000                    | -0.001000 | 0.003000  |
| 12  | O    | 0.037400                | 0.891900 | 0.250000 | 0.000000                      | 0.000000 | 0.000000 | -0.005000                   | 0.001000  | 0.002000  |
| 13  | O    | 0.303300                | 0.807500 | 0.944300 | 0.000000                      | 0.000000 | 0.000000 | -0.009000                   | 0.005000  | -0.018000 |
| 14  | O    | 0.696700                | 0.192500 | 0.444300 | 0.000000                      | 0.000000 | 0.000000 | 0.008000                    | -0.007000 | -0.019000 |
| 15  | O    | 0.196700                | 0.307500 | 0.444300 | 0.000000                      | 0.000000 | 0.000000 | 0.009000                    | 0.006000  | -0.019000 |
| 16  | O    | 0.803300                | 0.692500 | 0.944300 | 0.000000                      | 0.000000 | 0.000000 | -0.010000                   | -0.004000 | -0.018000 |
| 17  | O    | 0.196700                | 0.307500 | 0.055700 | 0.000000                      | 0.000000 | 0.000000 | -0.011000                   | -0.005000 | -0.018000 |
| 18  | O    | 0.803300                | 0.692500 | 0.555700 | 0.000000                      | 0.000000 | 0.000000 | 0.012000                    | 0.003000  | -0.017000 |
| 19  | O    | 0.303300                | 0.807500 | 0.555700 | 0.000000                      | 0.000000 | 0.000000 | 0.012000                    | -0.005000 | -0.017000 |
| 20  | O    | 0.696700                | 0.192500 | 0.055700 | 0.000000                      | 0.000000 | 0.000000 | -0.011000                   | 0.006000  | -0.018000 |

FIG. 60. First-principles calculation results of 0.11 DyFeO<sub>3</sub>. The band structure is shown in the left panel, and the Fermi-level-dependent AHC is plotted in the right panel. In both plots, the Fermi level is set to 0 eV.

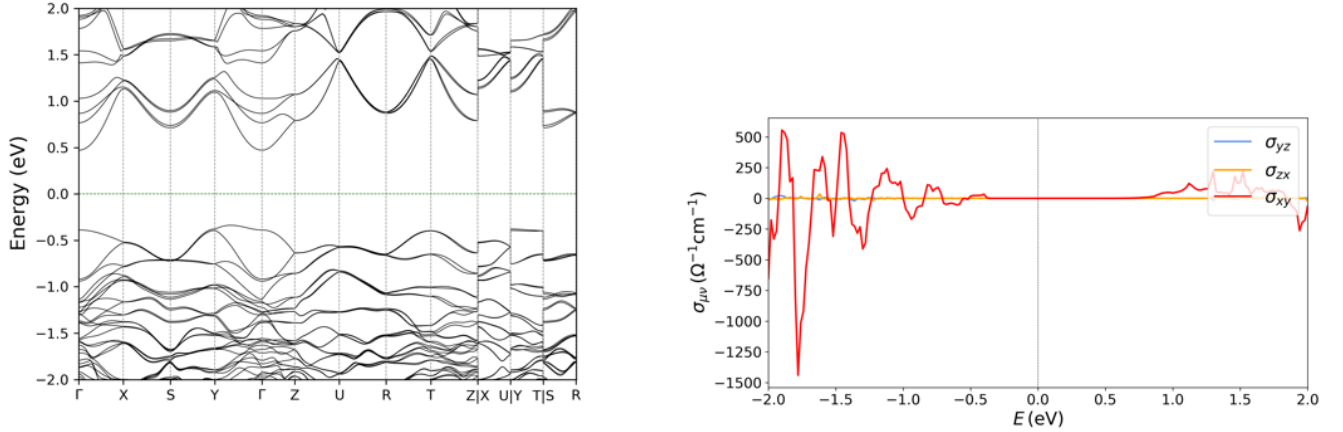

**0.205 Sr<sub>2</sub>MnReO<sub>6</sub>** crystallizes in type III MSG 14.79, which hosts both SNLs and FNSs. The symmetry-adapted AHC tensor of the MSG is  $(\sigma_{yz}, \sigma_{zx}, 0)$ . Based on the first-principles calculation results, the comparison between the experimental and calculated magnetic moments is provided in Table SII63. The band structure is shown in the left panel of Fig. 61, and the Fermi-level-dependent AHC is plotted in the right panel.

TABLE SII63. The comparison between the experimental and calculated magnetic moments for 0.205 Sr<sub>2</sub>MnReO<sub>6</sub>. The five columns contain the atom index in the structure file, the atom species, the fractional coordinates, the experimental magnetic moments, and the calculated magnetic moments. The lattice vectors are  $\vec{a}_1 = (5.6514, 0.0, 0.0)$ ,  $\vec{a}_2 = (0.0, 5.6378, 0.0)$ ,  $\vec{a}_3 = (-5.623571654, 0.0, 7.9730554)$ .

| No. | Atom | Coordinates(fractional) |          |          | Experimental magnetic moments |           |           | Calculated magnetic moments |           |           |
|-----|------|-------------------------|----------|----------|-------------------------------|-----------|-----------|-----------------------------|-----------|-----------|
| 1   | Sr   | 0.254200                | 0.976100 | 0.249800 | 0.000000                      | 0.000000  | 0.000000  | 0.000000                    | -0.000000 | 0.005000  |
| 2   | Sr   | 0.745800                | 0.023900 | 0.750200 | 0.000000                      | 0.000000  | 0.000000  | 0.000000                    | 0.000000  | 0.005000  |
| 3   | Sr   | 0.745800                | 0.476100 | 0.250200 | 0.000000                      | 0.000000  | 0.000000  | 0.000000                    | 0.000000  | 0.005000  |
| 4   | Sr   | 0.254200                | 0.523900 | 0.749800 | 0.000000                      | 0.000000  | 0.000000  | 0.000000                    | -0.000000 | 0.005000  |
| 5   | Mn   | 0.000000                | 0.000000 | 0.500000 | 4.155820                      | -1.270030 | -1.099960 | 4.416000                    | -1.350000 | -1.171000 |
| 6   | Mn   | 0.000000                | 0.500000 | 0.000000 | 4.155820                      | 1.270030  | -1.099960 | 4.416000                    | 1.350000  | -1.171000 |
| 7   | Re   | 0.500000                | 0.000000 | 0.000000 | 0.203430                      | -0.070020 | 0.899680  | 0.241000                    | -0.084000 | 1.111000  |
| 8   | Re   | 0.500000                | 0.500000 | 0.500000 | 0.203430                      | 0.070020  | 0.899680  | 0.241000                    | 0.084000  | 1.111000  |
| 9   | O    | 0.264500                | 0.294300 | 0.527500 | 0.000000                      | 0.000000  | 0.000000  | -0.008000                   | -0.003000 | -0.037000 |
| 10  | O    | 0.735500                | 0.705700 | 0.472500 | 0.000000                      | 0.000000  | 0.000000  | -0.008000                   | -0.003000 | -0.037000 |
| 11  | O    | 0.735500                | 0.794300 | 0.972500 | 0.000000                      | 0.000000  | 0.000000  | -0.008000                   | 0.003000  | -0.037000 |
| 12  | O    | 0.264500                | 0.205700 | 0.027500 | 0.000000                      | 0.000000  | 0.000000  | -0.008000                   | 0.002000  | -0.037000 |
| 13  | O    | 0.324900                | 0.769400 | 0.532400 | 0.000000                      | 0.000000  | 0.000000  | -0.007000                   | -0.002000 | -0.029000 |
| 14  | O    | 0.675100                | 0.230600 | 0.467600 | 0.000000                      | 0.000000  | 0.000000  | -0.007000                   | -0.001000 | -0.029000 |
| 15  | O    | 0.675100                | 0.269400 | 0.967600 | 0.000000                      | 0.000000  | 0.000000  | -0.007000                   | 0.001000  | -0.030000 |
| 16  | O    | 0.324900                | 0.730600 | 0.032400 | 0.000000                      | 0.000000  | 0.000000  | -0.007000                   | 0.002000  | -0.029000 |
| 17  | O    | 0.203600                | 0.509400 | 0.263200 | 0.000000                      | 0.000000  | 0.000000  | -0.007000                   | -0.002000 | -0.025000 |
| 18  | O    | 0.796400                | 0.490600 | 0.736800 | 0.000000                      | 0.000000  | 0.000000  | -0.007000                   | -0.003000 | -0.025000 |
| 19  | O    | 0.796400                | 0.009400 | 0.236800 | 0.000000                      | 0.000000  | 0.000000  | -0.007000                   | 0.002000  | -0.026000 |
| 20  | O    | 0.203600                | 0.990600 | 0.763200 | 0.000000                      | 0.000000  | 0.000000  | -0.007000                   | 0.003000  | -0.025000 |

FIG. 61. First-principles calculation results of 0.205 Sr<sub>2</sub>MnReO<sub>6</sub>. The band structure is shown in the left panel, and the Fermi-level-dependent AHC is plotted in the right panel. In both plots, the Fermi level is set to 0 eV.

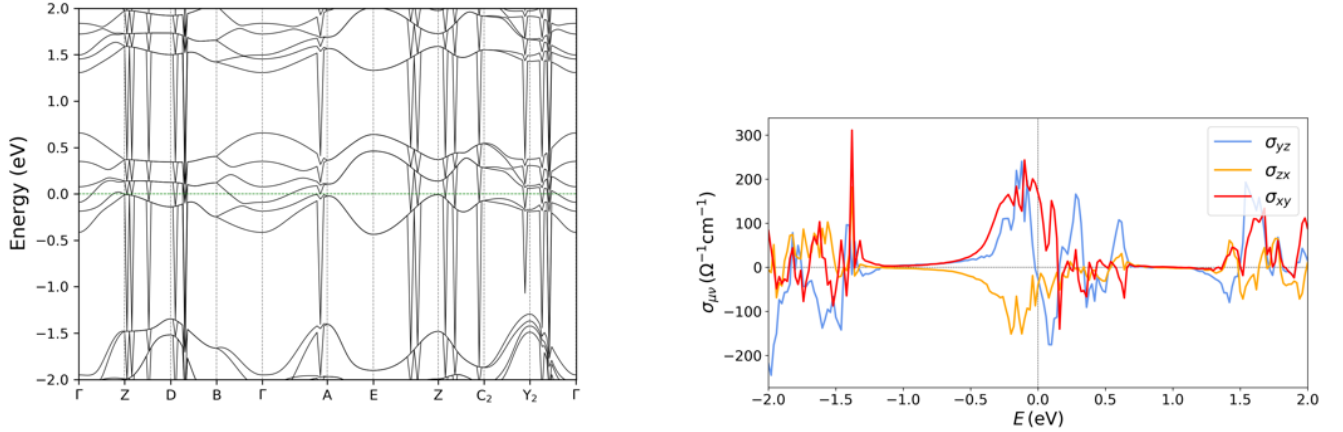

$0.25 \text{ NaOsO}_3$  crystallizes in type III MSG 62.448, which hosts both SNLs and FNSs. The symmetry-adapted AHC tensor of the MSG is  $(0, \sigma_{zx}, 0)$ . Based on the first-principles calculation results, the comparison between the experimental and calculated magnetic moments is provided in Table SII64. The band structure is shown in the left panel of Fig. 62, and the Fermi-level-dependent AHC is plotted in the right panel.

TABLE SII64. The comparison between the experimental and calculated magnetic moments for  $0.25 \text{ NaOsO}_3$ . The five columns contain the atom index in the structure file, the atom species, the fractional coordinates, the experimental magnetic moments, and the calculated magnetic moments. The lattice vectors are  $\vec{a}_1 = (5.3842, 0.0, 0.0)$ ,  $\vec{a}_2 = (0.0, 7.5804, 0.0)$ ,  $\vec{a}_3 = (0.0, 0.0, 5.3282)$ .

| No. | Atom | Coordinates(fractional) |          |          | Experimental magnetic moments |          |           | Calculated magnetic moments |           |           |
|-----|------|-------------------------|----------|----------|-------------------------------|----------|-----------|-----------------------------|-----------|-----------|
| 1   | Na   | 0.532800                | 0.250000 | 0.499350 | 0.000000                      | 0.000000 | 0.000000  | 0.000000                    | 0.000000  | 0.000000  |
| 2   | Na   | 0.467200                | 0.750000 | 0.500650 | 0.000000                      | 0.000000 | 0.000000  | 0.000000                    | 0.000000  | -0.000000 |
| 3   | Na   | 0.032800                | 0.250000 | 0.000650 | 0.000000                      | 0.000000 | 0.000000  | -0.000000                   | 0.000000  | 0.000000  |
| 4   | Na   | 0.967200                | 0.750000 | 0.999350 | 0.000000                      | 0.000000 | 0.000000  | -0.000000                   | 0.000000  | -0.000000 |
| 5   | Os   | 0.000000                | 0.000000 | 0.500000 | 0.000000                      | 0.000000 | -1.000000 | -0.094000                   | -0.046000 | -1.578000 |
| 6   | Os   | 0.000000                | 0.500000 | 0.500000 | 0.000000                      | 0.000000 | 1.000000  | 0.094000                    | -0.047000 | 1.576000  |
| 7   | Os   | 0.500000                | 0.500000 | 0.000000 | 0.000000                      | 0.000000 | -1.000000 | 0.094000                    | -0.046000 | -1.578000 |
| 8   | Os   | 0.500000                | 0.000000 | 0.000000 | 0.000000                      | 0.000000 | 1.000000  | -0.094000                   | -0.047000 | 1.576000  |
| 9   | O    | 0.983400                | 0.250000 | 0.580800 | 0.000000                      | 0.000000 | 0.000000  | -0.001000                   | 0.002000  | -0.000000 |
| 10  | O    | 0.016600                | 0.750000 | 0.419200 | 0.000000                      | 0.000000 | 0.000000  | 0.001000                    | 0.002000  | 0.000000  |
| 11  | O    | 0.483400                | 0.250000 | 0.919200 | 0.000000                      | 0.000000 | 0.000000  | 0.001000                    | 0.002000  | -0.000000 |
| 12  | O    | 0.516600                | 0.750000 | 0.080800 | 0.000000                      | 0.000000 | 0.000000  | -0.001000                   | 0.002000  | 0.000000  |
| 13  | O    | 0.788100                | 0.039400 | 0.211200 | 0.000000                      | 0.000000 | 0.000000  | -0.009000                   | -0.003000 | 0.003000  |
| 14  | O    | 0.211900                | 0.539400 | 0.788800 | 0.000000                      | 0.000000 | 0.000000  | 0.006000                    | -0.002000 | -0.003000 |
| 15  | O    | 0.211900                | 0.960600 | 0.788800 | 0.000000                      | 0.000000 | 0.000000  | -0.010000                   | -0.003000 | 0.003000  |
| 16  | O    | 0.788100                | 0.460600 | 0.211200 | 0.000000                      | 0.000000 | 0.000000  | 0.007000                    | -0.003000 | -0.003000 |
| 17  | O    | 0.288100                | 0.460600 | 0.288800 | 0.000000                      | 0.000000 | 0.000000  | 0.009000                    | -0.003000 | 0.003000  |
| 18  | O    | 0.711900                | 0.960600 | 0.711200 | 0.000000                      | 0.000000 | 0.000000  | -0.006000                   | -0.002000 | -0.003000 |
| 19  | O    | 0.711900                | 0.539400 | 0.711200 | 0.000000                      | 0.000000 | 0.000000  | 0.010000                    | -0.003000 | 0.003000  |
| 20  | O    | 0.288100                | 0.039400 | 0.288800 | 0.000000                      | 0.000000 | 0.000000  | -0.007000                   | -0.003000 | -0.003000 |

FIG. 62. First-principles calculation results of  $0.25 \text{ NaOsO}_3$ . The band structure is shown in the left panel, and the Fermi-level-dependent AHC is plotted in the right panel. In both plots, the Fermi level is set to 0 eV.

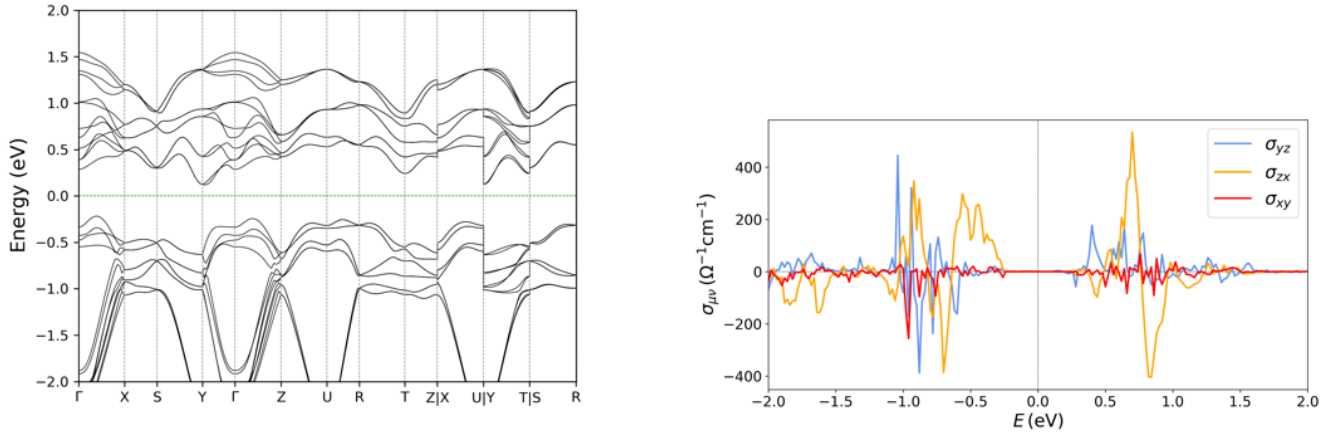

**0.286 Mn<sub>5</sub>Ge<sub>3</sub>** crystallizes in type III MSG 193.260, which hosts only SNLs. The symmetry-adapted AHC tensor of the MSG is  $(0, 0, \sigma_{xy})$ . Based on the first-principles calculation results, the comparison between the experimental and calculated magnetic moments is provided in Table SII65. The band structure is shown in the left panel of Fig. 63, and the Fermi-level-dependent AHC is plotted in the right panel.

TABLE SII65. The comparison between the experimental and calculated magnetic moments for 0.286 Mn<sub>5</sub>Ge<sub>3</sub>. The five columns contain the atom index in the structure file, the atom species, the fractional coordinates, the experimental magnetic moments, and the calculated magnetic moments. The lattice vectors are  $\vec{a}_1 = (7.184, 0.0, 0.0)$ ,  $\vec{a}_2 = (-3.592, 6.221526501, 0.0)$ ,  $\vec{a}_3 = (0.0, 0.0, 5.053)$ .

| No. | Atom | Coordinates(fractional) |          |          | Experimental magnetic moments |          |          | Calculated magnetic moments |           |           |
|-----|------|-------------------------|----------|----------|-------------------------------|----------|----------|-----------------------------|-----------|-----------|
| 1   | Ge   | 0.603000                | 0.000000 | 0.250000 | 0.000000                      | 0.000000 | 0.000000 | -0.000000                   | -0.000000 | -0.228000 |
| 2   | Ge   | 0.603000                | 0.603000 | 0.750000 | 0.000000                      | 0.000000 | 0.000000 | 0.000000                    | 0.000000  | -0.230000 |
| 3   | Ge   | 0.000000                | 0.603000 | 0.250000 | 0.000000                      | 0.000000 | 0.000000 | -0.000000                   | -0.000000 | -0.205000 |
| 4   | Ge   | 0.397000                | 0.000000 | 0.750000 | 0.000000                      | 0.000000 | 0.000000 | -0.000000                   | -0.000000 | -0.228000 |
| 5   | Ge   | 0.397000                | 0.397000 | 0.250000 | 0.000000                      | 0.000000 | 0.000000 | 0.000000                    | 0.000000  | -0.230000 |
| 6   | Ge   | 0.000000                | 0.397000 | 0.750000 | 0.000000                      | 0.000000 | 0.000000 | 0.000000                    | 0.000000  | -0.205000 |
| 7   | Mn   | 0.333333                | 0.666667 | 0.000000 | 0.000000                      | 0.000000 | 1.960010 | -0.000000                   | -0.000000 | 3.828000  |
| 8   | Mn   | 0.666667                | 0.333333 | 0.500000 | 0.000000                      | 0.000000 | 1.960010 | -0.000000                   | -0.000000 | 3.807000  |
| 9   | Mn   | 0.666667                | 0.333333 | 0.000000 | 0.000000                      | 0.000000 | 1.960010 | 0.000000                    | 0.001000  | 3.825000  |
| 10  | Mn   | 0.333333                | 0.666667 | 0.500000 | 0.000000                      | 0.000000 | 1.960010 | 0.000000                    | -0.000000 | 3.807000  |
| 11  | Mn   | 0.239700                | 0.000000 | 0.250000 | 0.000000                      | 0.000000 | 3.229980 | 0.000000                    | -0.001000 | 4.027000  |
| 12  | Mn   | 0.239700                | 0.239700 | 0.750000 | 0.000000                      | 0.000000 | 3.229980 | 0.001000                    | -0.001000 | 4.029000  |
| 13  | Mn   | 0.000000                | 0.239700 | 0.250000 | 0.000000                      | 0.000000 | 3.229980 | 0.001000                    | 0.000000  | 4.028000  |
| 14  | Mn   | 0.760300                | 0.000000 | 0.750000 | 0.000000                      | 0.000000 | 3.229980 | 0.000000                    | 0.001000  | 4.027000  |
| 15  | Mn   | 0.760300                | 0.760300 | 0.250000 | 0.000000                      | 0.000000 | 3.229980 | -0.001000                   | 0.001000  | 4.030000  |
| 16  | Mn   | 0.000000                | 0.760300 | 0.750000 | 0.000000                      | 0.000000 | 3.229980 | -0.001000                   | -0.000000 | 4.028000  |

FIG. 63. First-principles calculation results of 0.286 Mn<sub>5</sub>Ge<sub>3</sub>. The band structure is shown in the left panel, and the Fermi-level-dependent AHC is plotted in the right panel. In both plots, the Fermi level is set to 0 eV.

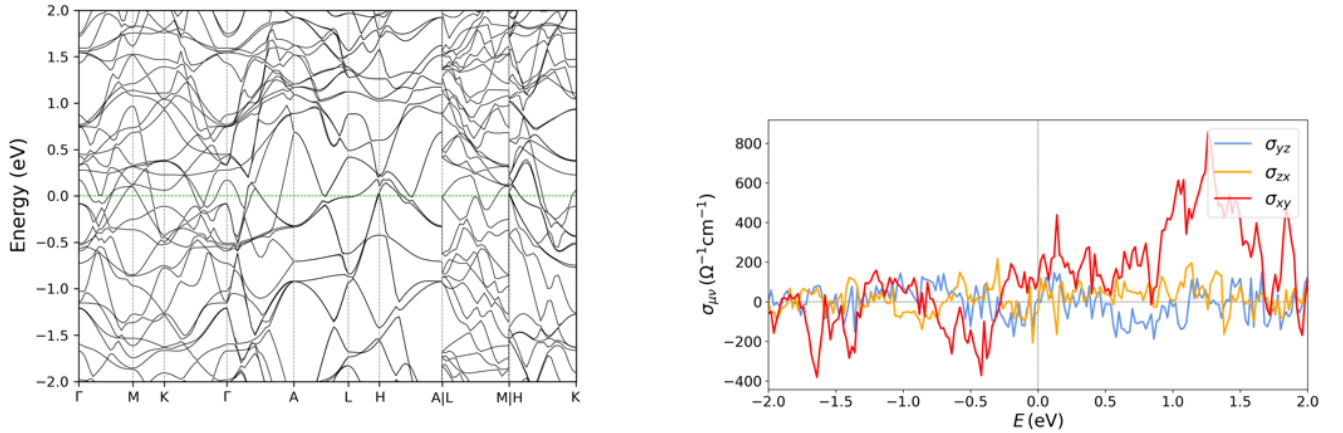



0.319  $\text{Tm}_2\text{CoMnO}_6$  crystallizes in type III MSG 14.79, which hosts both SNLs and FNSs. The symmetry-adapted AHC tensor of the MSG is  $(\sigma_{yz}, \sigma_{zx}, 0)$ . Based on the first-principles calculation results, the comparison between the experimental and calculated magnetic moments is provided in Table SII66. The band structure is shown in the left panel of Fig. 64, and the Fermi-level-dependent AHC is plotted in the right panel.

TABLE SII66. The comparison between the experimental and calculated magnetic moments for 0.319  $\text{Tm}_2\text{CoMnO}_6$ . The five columns contain the atom index in the structure file, the atom species, the fractional coordinates, the experimental magnetic moments, and the calculated magnetic moments. The lattice vectors are  $\vec{a}_1 = (5.18906, 0.0, 0.0)$ ,  $\vec{a}_2 = (0.0, 5.54327, 0.0)$ ,  $\vec{a}_3 = (-5.146075488, 0.0, 7.418628786)$ .

| No. | Atom | Coordinates(fractional) |          |          | Experimental magnetic moments |          | Calculated magnetic moments |           |           |           |
|-----|------|-------------------------|----------|----------|-------------------------------|----------|-----------------------------|-----------|-----------|-----------|
| 1   | Tm   | 0.272100                | 0.573100 | 0.752200 | -0.576650                     | 0.000000 | 0.529990                    | -0.715000 | 0.014000  | 0.669000  |
| 2   | Tm   | 0.727900                | 0.426900 | 0.247800 | -0.576650                     | 0.000000 | 0.529990                    | -0.715000 | 0.015000  | 0.669000  |
| 3   | Tm   | 0.727900                | 0.073100 | 0.747800 | -0.576650                     | 0.000000 | 0.529990                    | -0.723000 | -0.013000 | 0.678000  |
| 4   | Tm   | 0.272100                | 0.926900 | 0.252200 | -0.576650                     | 0.000000 | 0.529990                    | -0.723000 | -0.013000 | 0.678000  |
| 5   | Co   | 0.000000                | 0.000000 | 0.500000 | 1.006140                      | 0.000000 | -2.350000                   | 1.300000  | 0.001000  | -3.037000 |
| 6   | Co   | 0.000000                | 0.500000 | 0.000000 | 1.006140                      | 0.000000 | -2.350000                   | 1.300000  | -0.000000 | -3.037000 |
| 7   | Mn   | 0.500000                | 0.000000 | 0.000000 | 1.006140                      | 0.000000 | -2.350000                   | 1.514000  | 0.000000  | -3.538000 |
| 8   | Mn   | 0.500000                | 0.500000 | 0.500000 | 1.006140                      | 0.000000 | -2.350000                   | 1.514000  | -0.000000 | -3.537000 |
| 9   | O    | 0.355300                | 0.817200 | 0.553800 | 0.000000                      | 0.000000 | 0.000000                    | 0.063000  | -0.001000 | -0.143000 |
| 10  | O    | 0.644700                | 0.182800 | 0.446200 | 0.000000                      | 0.000000 | 0.000000                    | 0.063000  | -0.001000 | -0.143000 |
| 11  | O    | 0.644700                | 0.317200 | 0.946200 | 0.000000                      | 0.000000 | 0.000000                    | 0.064000  | 0.001000  | -0.146000 |
| 12  | O    | 0.355300                | 0.682800 | 0.053800 | 0.000000                      | 0.000000 | 0.000000                    | 0.064000  | 0.001000  | -0.146000 |
| 13  | O    | 0.765400                | 0.793300 | 0.942000 | 0.000000                      | 0.000000 | 0.000000                    | 0.036000  | -0.000000 | -0.083000 |
| 14  | O    | 0.234600                | 0.206700 | 0.058000 | 0.000000                      | 0.000000 | 0.000000                    | 0.036000  | -0.000000 | -0.083000 |
| 15  | O    | 0.234600                | 0.293300 | 0.558000 | 0.000000                      | 0.000000 | 0.000000                    | 0.035000  | 0.000000  | -0.080000 |
| 16  | O    | 0.765400                | 0.706700 | 0.442000 | 0.000000                      | 0.000000 | 0.000000                    | 0.035000  | 0.000000  | -0.080000 |
| 17  | O    | 0.868600                | 0.461100 | 0.756700 | 0.000000                      | 0.000000 | 0.000000                    | 0.021000  | 0.000000  | -0.051000 |
| 18  | O    | 0.131400                | 0.538900 | 0.243300 | 0.000000                      | 0.000000 | 0.000000                    | 0.021000  | -0.000000 | -0.051000 |
| 19  | O    | 0.131400                | 0.961100 | 0.743300 | 0.000000                      | 0.000000 | 0.000000                    | 0.021000  | 0.000000  | -0.053000 |
| 20  | O    | 0.868600                | 0.038900 | 0.256700 | 0.000000                      | 0.000000 | 0.000000                    | 0.021000  | 0.000000  | -0.053000 |

FIG. 64. First-principles calculation results of 0.319  $\text{Tm}_2\text{CoMnO}_6$ . The band structure is shown in the left panel, and the Fermi-level-dependent AHC is plotted in the right panel. In both plots, the Fermi level is set to 0 eV.

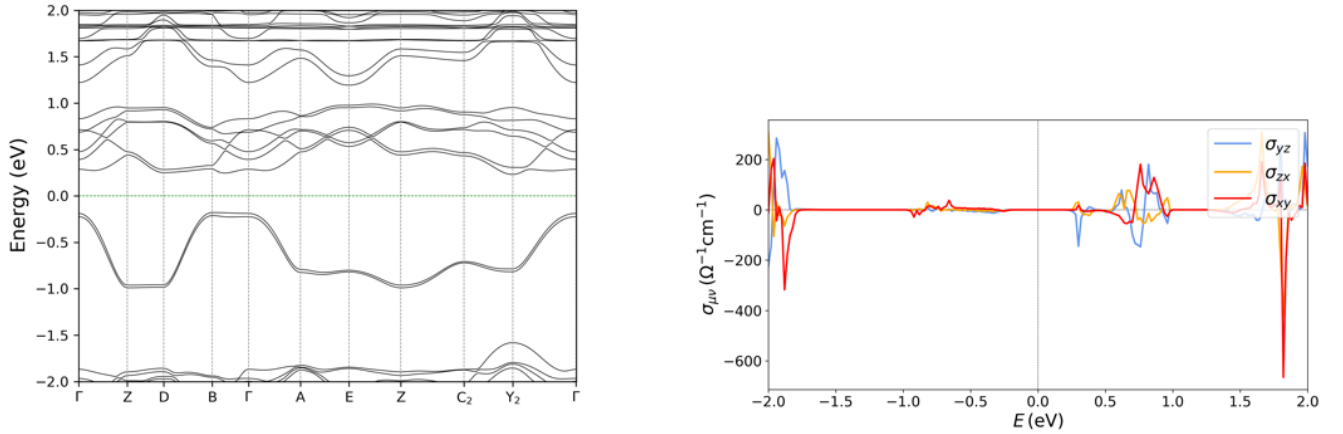

**0.358 CaFe<sub>5</sub>O<sub>7</sub>** crystallizes in type III MSG 11.54, which hosts only FNSs. The symmetry-adapted AHC tensor of the MSG is  $(\sigma_{yz}, \sigma_{zx}, 0)$ . Based on the first-principles calculation results, the comparison between the experimental and calculated magnetic moments is provided in Table SII67. The band structure is shown in the left panel of Fig. 65, and the Fermi-level-dependent AHC is plotted in the right panel.

TABLE SII67. The comparison between the experimental and calculated magnetic moments for 0.358 CaFe<sub>5</sub>O<sub>7</sub>. The five columns contain the atom index in the structure file, the atom species, the fractional coordinates, the experimental magnetic moments, and the calculated magnetic moments. The lattice vectors are  $\vec{a}_1 = (3.0454, 0.0, 0.0)$ ,  $\vec{a}_2 = (0.0, 17.9659, 0.0)$ ,  $\vec{a}_3 = (-1.510098119, 0.0, 5.018608059)$ .

| No. | Atom | Coordinates(fractional) |          |          | Experimental magnetic moments |           |          | Calculated magnetic moments |           |           |
|-----|------|-------------------------|----------|----------|-------------------------------|-----------|----------|-----------------------------|-----------|-----------|
| 1   | Ca   | 0.212500                | 0.250000 | 0.428500 | 0.000000                      | 0.000000  | 0.000000 | -0.000000                   | -0.005000 | 0.000000  |
| 2   | Ca   | 0.787500                | 0.750000 | 0.571500 | 0.000000                      | 0.000000  | 0.000000 | -0.000000                   | -0.005000 | 0.000000  |
| 3   | Fe   | 0.726200                | 0.075200 | 0.452000 | 0.000000                      | 3.799970  | 0.000000 | 0.083000                    | 3.724000  | 0.017000  |
| 4   | Fe   | 0.273800                | 0.924800 | 0.548000 | 0.000000                      | 3.799970  | 0.000000 | 0.083000                    | 3.725000  | 0.016000  |
| 5   | Fe   | 0.273800                | 0.575200 | 0.548000 | 0.000000                      | -3.799970 | 0.000000 | 0.033000                    | -4.047000 | -0.006000 |
| 6   | Fe   | 0.726200                | 0.424800 | 0.452000 | 0.000000                      | -3.799970 | 0.000000 | 0.033000                    | -4.048000 | -0.007000 |
| 7   | Fe   | 0.544700                | 0.846300 | 0.074300 | 0.000000                      | -3.900040 | 0.000000 | -0.056000                   | -4.152000 | -0.032000 |
| 8   | Fe   | 0.455300                | 0.153700 | 0.925700 | 0.000000                      | -3.900040 | 0.000000 | -0.056000                   | -4.152000 | -0.031000 |
| 9   | Fe   | 0.455300                | 0.346300 | 0.925700 | 0.000000                      | 3.900040  | 0.000000 | -0.108000                   | 3.822000  | -0.047000 |
| 10  | Fe   | 0.544700                | 0.653700 | 0.074300 | 0.000000                      | 3.900040  | 0.000000 | -0.108000                   | 3.822000  | -0.047000 |
| 11  | Fe   | 0.000000                | 0.000000 | 0.000000 | 0.000000                      | -3.499940 | 0.000000 | -0.119000                   | -3.718000 | 0.180000  |
| 12  | Fe   | 0.000000                | 0.500000 | 0.000000 | 0.000000                      | 3.499940  | 0.000000 | -0.022000                   | 3.678000  | 0.064000  |
| 13  | O    | 0.737600                | 0.250000 | 0.085600 | 0.000000                      | 0.000000  | 0.000000 | -0.004000                   | -0.100000 | -0.003000 |
| 14  | O    | 0.262400                | 0.750000 | 0.914400 | 0.000000                      | 0.000000  | 0.000000 | -0.004000                   | -0.100000 | -0.003000 |
| 15  | O    | 0.080800                | 0.393500 | 0.175700 | 0.000000                      | 0.000000  | 0.000000 | -0.000000                   | -0.041000 | -0.001000 |
| 16  | O    | 0.919200                | 0.606500 | 0.824300 | 0.000000                      | 0.000000  | 0.000000 | -0.000000                   | -0.041000 | -0.001000 |
| 17  | O    | 0.919200                | 0.893500 | 0.824300 | 0.000000                      | 0.000000  | 0.000000 | -0.003000                   | -0.142000 | -0.000000 |
| 18  | O    | 0.080800                | 0.106500 | 0.175700 | 0.000000                      | 0.000000  | 0.000000 | -0.003000                   | -0.142000 | -0.000000 |
| 19  | O    | 0.377100                | 0.468200 | 0.716400 | 0.000000                      | 0.000000  | 0.000000 | 0.001000                    | -0.098000 | 0.001000  |
| 20  | O    | 0.622900                | 0.531800 | 0.283600 | 0.000000                      | 0.000000  | 0.000000 | 0.001000                    | -0.098000 | 0.001000  |
| 21  | O    | 0.622900                | 0.968200 | 0.283600 | 0.000000                      | 0.000000  | 0.000000 | -0.001000                   | -0.027000 | 0.003000  |
| 22  | O    | 0.377100                | 0.031800 | 0.716400 | 0.000000                      | 0.000000  | 0.000000 | -0.001000                   | -0.028000 | 0.003000  |
| 23  | O    | 0.831000                | 0.331800 | 0.650000 | 0.000000                      | 0.000000  | 0.000000 | -0.001000                   | -0.032000 | -0.001000 |
| 24  | O    | 0.169000                | 0.668200 | 0.350000 | 0.000000                      | 0.000000  | 0.000000 | -0.000000                   | -0.032000 | -0.001000 |
| 25  | O    | 0.169000                | 0.831800 | 0.350000 | 0.000000                      | 0.000000  | 0.000000 | -0.002000                   | -0.135000 | -0.001000 |
| 26  | O    | 0.831000                | 0.168200 | 0.650000 | 0.000000                      | 0.000000  | 0.000000 | -0.002000                   | -0.135000 | -0.001000 |

FIG. 65. First-principles calculation results of 0.358 CaFe<sub>5</sub>O<sub>7</sub>. The band structure is shown in the left panel, and the Fermi-level-dependent AHC is plotted in the right panel. In both plots, the Fermi level is set to 0 eV.

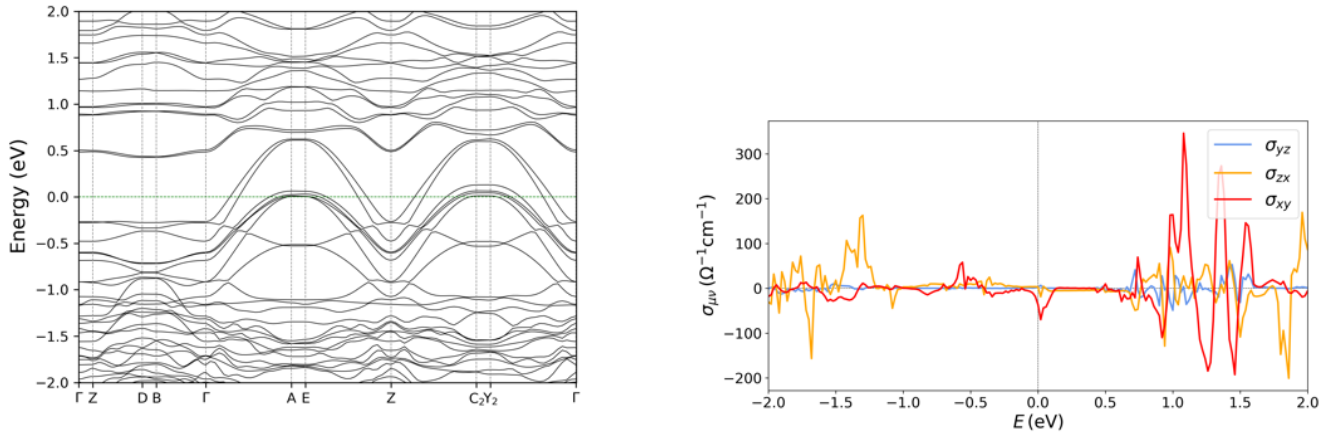

**0.445 MnCoGe** crystallizes in type III MSG 62.446, which hosts both SNLs and FNSs. The symmetry-adapted AHC tensor of the MSG is  $(0, 0, \sigma_{xy})$ . Based on the first-principles calculation results, the comparison between the experimental and calculated magnetic moments is provided in Table SII68. The band structure is shown in the left panel of Fig. 66, and the Fermi-level-dependent AHC is plotted in the right panel.

TABLE SII68. The comparison between the experimental and calculated magnetic moments for 0.445 MnCoGe. The five columns contain the atom index in the structure file, the atom species, the fractional coordinates, the experimental magnetic moments, and the calculated magnetic moments. The lattice vectors are  $\vec{a}_1 = (5.9192, 0.0, 0.0)$ ,  $\vec{a}_2 = (0.0, 3.8132, 0.0)$ ,  $\vec{a}_3 = (0.0, 0.0, 7.0621)$ .

| No. | Atom | Coordinates(fractional) |          |          | Experimental magnetic moments |          |          | Calculated magnetic moments |           |           |
|-----|------|-------------------------|----------|----------|-------------------------------|----------|----------|-----------------------------|-----------|-----------|
| 1   | Co   | 0.347500                | 0.250000 | 0.083200 | 0.000000                      | 0.000000 | 0.630010 | 0.006000                    | -0.002000 | 0.889000  |
| 2   | Co   | 0.152500                | 0.750000 | 0.583200 | 0.000000                      | 0.000000 | 0.630010 | 0.006000                    | 0.002000  | 0.885000  |
| 3   | Co   | 0.652500                | 0.750000 | 0.916800 | 0.000000                      | 0.000000 | 0.630010 | -0.006000                   | 0.002000  | 0.885000  |
| 4   | Co   | 0.847500                | 0.250000 | 0.416800 | 0.000000                      | 0.000000 | 0.630010 | -0.006000                   | -0.003000 | 0.890000  |
| 5   | Mn   | 0.467900                | 0.250000 | 0.698800 | 0.000000                      | 0.000000 | 3.540020 | -0.000000                   | -0.000000 | 4.417000  |
| 6   | Mn   | 0.032100                | 0.750000 | 0.198800 | 0.000000                      | 0.000000 | 3.540020 | -0.000000                   | 0.000000  | 4.419000  |
| 7   | Mn   | 0.532100                | 0.750000 | 0.301200 | 0.000000                      | 0.000000 | 3.540020 | 0.000000                    | 0.000000  | 4.419000  |
| 8   | Mn   | 0.967900                | 0.250000 | 0.801200 | 0.000000                      | 0.000000 | 3.540020 | 0.000000                    | -0.000000 | 4.417000  |
| 9   | Ge   | 0.725800                | 0.250000 | 0.120400 | 0.000000                      | 0.000000 | 0.000000 | -0.002000                   | -0.000000 | -0.178000 |
| 10  | Ge   | 0.774200                | 0.750000 | 0.620400 | 0.000000                      | 0.000000 | 0.000000 | -0.001000                   | -0.000000 | -0.179000 |
| 11  | Ge   | 0.274200                | 0.750000 | 0.879600 | 0.000000                      | 0.000000 | 0.000000 | 0.001000                    | -0.000000 | -0.180000 |
| 12  | Ge   | 0.225800                | 0.250000 | 0.379600 | 0.000000                      | 0.000000 | 0.000000 | 0.002000                    | -0.000000 | -0.177000 |

FIG. 66. First-principles calculation results of 0.445 MnCoGe. The band structure is shown in the left panel, and the Fermi-level-dependent AHC is plotted in the right panel. In both plots, the Fermi level is set to 0 eV.

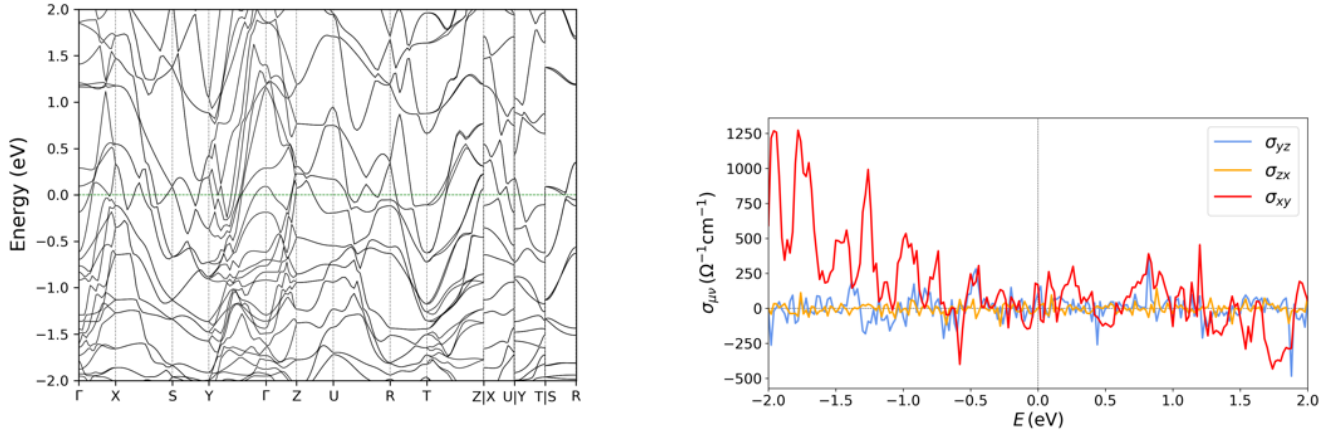

**0.513 YRuO<sub>3</sub>** crystallizes in type III MSG 62.448, which hosts both SNLs and FNSs. The symmetry-adapted AHC tensor of the MSG is  $(0, \sigma_{zx}, 0)$ . Based on the first-principles calculation results, the comparison between the experimental and calculated magnetic moments is provided in Table SII69. The band structure is shown in the left panel of Fig. 67, and the Fermi-level-dependent AHC is plotted in the right panel.

TABLE SII69. The comparison between the experimental and calculated magnetic moments for 0.513 YRuO<sub>3</sub>. The five columns contain the atom index in the structure file, the atom species, the fractional coordinates, the experimental magnetic moments, and the calculated magnetic moments. The lattice vectors are  $\vec{a}_1 = (5.839, 0.0, 0.0)$ ,  $\vec{a}_2 = (0.0, 7.523, 0.0)$ ,  $\vec{a}_3 = (0.0, 0.0, 5.192)$ .

| No. | Atom | Coordinates(fractional) |          |          | Experimental magnetic moments |          |           | Calculated magnetic moments |           |           |
|-----|------|-------------------------|----------|----------|-------------------------------|----------|-----------|-----------------------------|-----------|-----------|
| 1   | Y    | 0.583900                | 0.250000 | 0.474000 | 0.000000                      | 0.000000 | 0.000000  | -0.000000                   | -0.001000 | 0.000000  |
| 2   | Y    | 0.416100                | 0.750000 | 0.526000 | 0.000000                      | 0.000000 | 0.000000  | 0.000000                    | -0.002000 | -0.000000 |
| 3   | Y    | 0.083900                | 0.250000 | 0.026000 | 0.000000                      | 0.000000 | 0.000000  | 0.000000                    | -0.001000 | 0.001000  |
| 4   | Y    | 0.916100                | 0.750000 | 0.974000 | 0.000000                      | 0.000000 | 0.000000  | -0.000000                   | -0.002000 | -0.000000 |
| 5   | Ru   | 0.000000                | 0.000000 | 0.500000 | 0.000000                      | 0.000000 | -0.330000 | 0.009000                    | 0.006000  | -0.576000 |
| 6   | Ru   | 0.000000                | 0.500000 | 0.500000 | 0.000000                      | 0.000000 | 0.330000  | -0.008000                   | 0.007000  | 0.577000  |
| 7   | Ru   | 0.500000                | 0.500000 | 0.000000 | 0.000000                      | 0.000000 | -0.330000 | -0.009000                   | 0.007000  | -0.575000 |
| 8   | Ru   | 0.500000                | 0.000000 | 0.000000 | 0.000000                      | 0.000000 | 0.330000  | 0.008000                    | 0.006000  | 0.577000  |
| 9   | O    | 0.805200                | 0.061700 | 0.168900 | 0.000000                      | 0.000000 | 0.000000  | -0.004000                   | 0.008000  | 0.020000  |
| 10  | O    | 0.194800                | 0.561700 | 0.831100 | 0.000000                      | 0.000000 | 0.000000  | 0.005000                    | 0.010000  | -0.018000 |
| 11  | O    | 0.194800                | 0.938300 | 0.831100 | 0.000000                      | 0.000000 | 0.000000  | -0.005000                   | 0.008000  | 0.017000  |
| 12  | O    | 0.805200                | 0.438300 | 0.168900 | 0.000000                      | 0.000000 | 0.000000  | 0.004000                    | 0.006000  | -0.020000 |
| 13  | O    | 0.305200                | 0.438300 | 0.331100 | 0.000000                      | 0.000000 | 0.000000  | 0.005000                    | 0.007000  | 0.021000  |
| 14  | O    | 0.694800                | 0.938300 | 0.668900 | 0.000000                      | 0.000000 | 0.000000  | -0.005000                   | 0.010000  | -0.017000 |
| 15  | O    | 0.694800                | 0.561700 | 0.668900 | 0.000000                      | 0.000000 | 0.000000  | 0.005000                    | 0.008000  | 0.017000  |
| 16  | O    | 0.305200                | 0.061700 | 0.331100 | 0.000000                      | 0.000000 | 0.000000  | -0.004000                   | 0.005000  | -0.020000 |
| 17  | O    | 0.947800                | 0.250000 | 0.641400 | 0.000000                      | 0.000000 | 0.000000  | -0.000000                   | -0.004000 | 0.001000  |
| 18  | O    | 0.052200                | 0.750000 | 0.358600 | 0.000000                      | 0.000000 | 0.000000  | 0.000000                    | -0.000000 | 0.001000  |
| 19  | O    | 0.447800                | 0.250000 | 0.858600 | 0.000000                      | 0.000000 | 0.000000  | 0.000000                    | -0.003000 | 0.000000  |
| 20  | O    | 0.552200                | 0.750000 | 0.141400 | 0.000000                      | 0.000000 | 0.000000  | -0.000000                   | -0.001000 | 0.000000  |

FIG. 67. First-principles calculation results of 0.513 YRuO<sub>3</sub>. The band structure is shown in the left panel, and the Fermi-level-dependent AHC is plotted in the right panel. In both plots, the Fermi level is set to 0 eV.

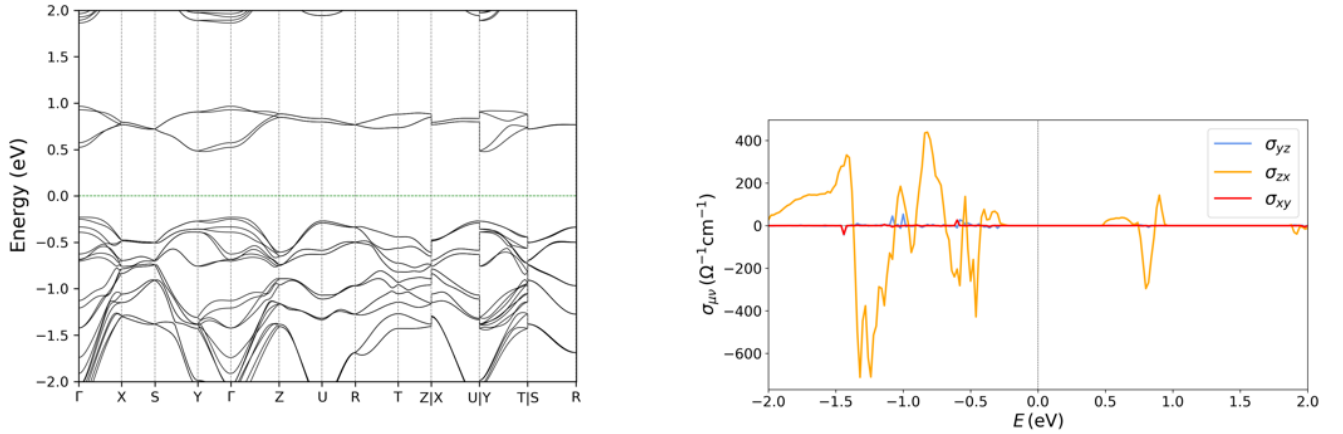

**0.642 LaMnO<sub>3</sub>** crystallizes in type III MSG 62.448, which hosts both SNLs and FNSs. The symmetry-adapted AHC tensor of the MSG is  $(0, \sigma_{zx}, 0)$ . Based on the first-principles calculation results, the comparison between the experimental and calculated magnetic moments is provided in Table SII70. The band structure is shown in the left panel of Fig. 68, and the Fermi-level-dependent AHC is plotted in the right panel.

TABLE SII70. The comparison between the experimental and calculated magnetic moments for 0.642 LaMnO<sub>3</sub>. The five columns contain the atom index in the structure file, the atom species, the fractional coordinates, the experimental magnetic moments, and the calculated magnetic moments. The lattice vectors are  $\vec{a}_1 = (5.742, 0.0, 0.0)$ ,  $\vec{a}_2 = (0.0, 7.668, 0.0)$ ,  $\vec{a}_3 = (0.0, 0.0, 5.532)$ .

| No. | Atom | Coordinates(fractional) |          |          | Experimental magnetic moments |          |          | Calculated magnetic moments |           |           |
|-----|------|-------------------------|----------|----------|-------------------------------|----------|----------|-----------------------------|-----------|-----------|
| 1   | La   | 0.049000                | 0.250000 | 0.510000 | 0.000000                      | 0.000000 | 0.000000 | -0.000000                   | -0.000000 | -0.000000 |
| 2   | La   | 0.951000                | 0.750000 | 0.490000 | 0.000000                      | 0.000000 | 0.000000 | -0.000000                   | 0.000000  | 0.000000  |
| 3   | La   | 0.549000                | 0.250000 | 0.990000 | 0.000000                      | 0.000000 | 0.000000 | 0.000000                    | -0.000000 | -0.000000 |
| 4   | La   | 0.451000                | 0.750000 | 0.010000 | 0.000000                      | 0.000000 | 0.000000 | 0.000000                    | 0.000000  | 0.000000  |
| 5   | Mn   | 0.000000                | 0.000000 | 0.000000 | 3.699970                      | 0.000000 | 0.000000 | 4.259000                    | 0.000000  | -0.000000 |
| 6   | Mn   | 0.000000                | 0.500000 | 0.000000 | -3.699970                     | 0.000000 | 0.000000 | -4.259000                   | 0.000000  | 0.000000  |
| 7   | Mn   | 0.500000                | 0.500000 | 0.500000 | -3.699970                     | 0.000000 | 0.000000 | -4.259000                   | 0.000000  | -0.000000 |
| 8   | Mn   | 0.500000                | 0.000000 | 0.500000 | 3.699970                      | 0.000000 | 0.000000 | 4.259000                    | 0.000000  | 0.000000  |
| 9   | O    | 0.486000                | 0.250000 | 0.430000 | 0.000000                      | 0.000000 | 0.000000 | -0.001000                   | -0.001000 | 0.000000  |
| 10  | O    | 0.514000                | 0.750000 | 0.570000 | 0.000000                      | 0.000000 | 0.000000 | -0.001000                   | -0.001000 | -0.000000 |
| 11  | O    | 0.986000                | 0.250000 | 0.070000 | 0.000000                      | 0.000000 | 0.000000 | 0.001000                    | 0.000000  | 0.000000  |
| 12  | O    | 0.014000                | 0.750000 | 0.930000 | 0.000000                      | 0.000000 | 0.000000 | 0.001000                    | 0.001000  | -0.000000 |
| 13  | O    | 0.809000                | 0.039000 | 0.724000 | 0.000000                      | 0.000000 | 0.000000 | -0.095000                   | -0.000000 | 0.000000  |
| 14  | O    | 0.191000                | 0.539000 | 0.276000 | 0.000000                      | 0.000000 | 0.000000 | 0.095000                    | 0.000000  | -0.000000 |
| 15  | O    | 0.191000                | 0.961000 | 0.276000 | 0.000000                      | 0.000000 | 0.000000 | -0.095000                   | 0.000000  | -0.000000 |
| 16  | O    | 0.809000                | 0.461000 | 0.724000 | 0.000000                      | 0.000000 | 0.000000 | 0.095000                    | -0.000000 | -0.000000 |
| 17  | O    | 0.309000                | 0.461000 | 0.776000 | 0.000000                      | 0.000000 | 0.000000 | 0.095000                    | 0.000000  | 0.000000  |
| 18  | O    | 0.691000                | 0.961000 | 0.224000 | 0.000000                      | 0.000000 | 0.000000 | -0.095000                   | 0.000000  | 0.000000  |
| 19  | O    | 0.691000                | 0.539000 | 0.224000 | 0.000000                      | 0.000000 | 0.000000 | 0.095000                    | 0.000000  | -0.000000 |
| 20  | O    | 0.309000                | 0.039000 | 0.776000 | 0.000000                      | 0.000000 | 0.000000 | -0.095000                   | 0.000000  | -0.000000 |

FIG. 68. First-principles calculation results of 0.642 LaMnO<sub>3</sub>. The band structure is shown in the left panel, and the Fermi-level-dependent AHC is plotted in the right panel. In both plots, the Fermi level is set to 0 eV.

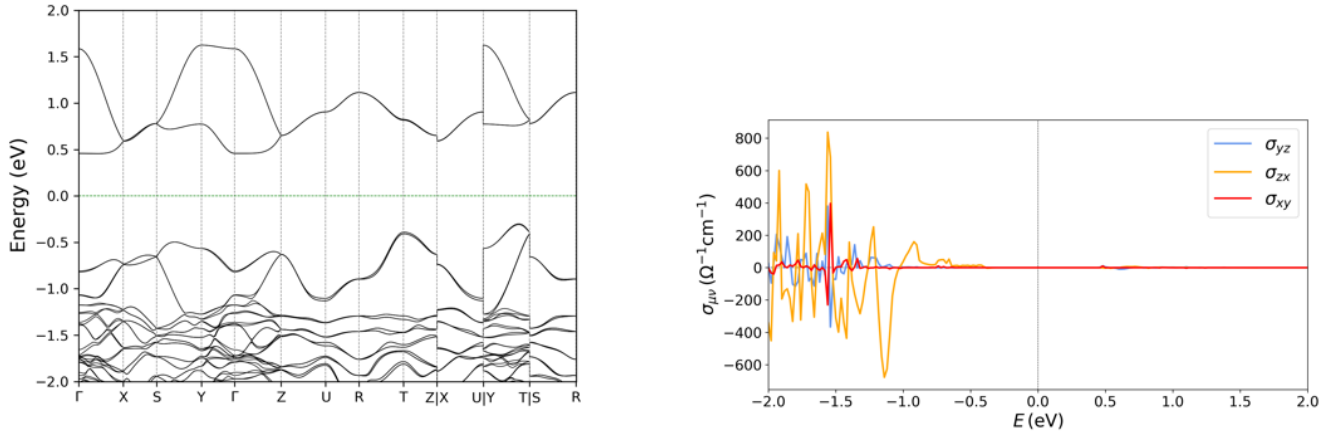

0.726 CsMn<sub>2</sub>F<sub>6</sub> crystallizes in type III MSG 62.447, which hosts both SNLs and FNSs. The symmetry-adapted AHC tensor of the MSG is ( $\sigma_{yz}$ , 0, 0). Based on the first-principles calculation results, the comparison between the experimental and calculated magnetic moments is provided in Table SII71. The band structure is shown in the left panel of Fig. 69, and the Fermi-level-dependent AHC is plotted in the right panel.

TABLE SII71. The comparison between the experimental and calculated magnetic moments for 0.726 CsMn<sub>2</sub>F<sub>6</sub>. The five columns contain the atom index in the structure file, the atom species, the fractional coordinates, the experimental magnetic moments, and the calculated magnetic moments. The lattice vectors are  $\vec{a}_1 = (7.3013, 0.0, 0.0)$ ,  $\vec{a}_2 = (0.0, 7.7141, 0.0)$ ,  $\vec{a}_3 = (0.0, 0.0, 10.1926)$ .

| No. | Atom | Coordinates(fractional) |          |          | Experimental magnetic moments |           |           | Calculated magnetic moments |           |           |
|-----|------|-------------------------|----------|----------|-------------------------------|-----------|-----------|-----------------------------|-----------|-----------|
| 1   | Mn   | 0.000000                | 0.000000 | 0.000000 | 0.047970                      | 3.233980  | 0.360000  | 0.057000                    | 4.065000  | 0.451000  |
| 2   | Mn   | 0.500000                | 0.500000 | 0.500000 | 0.047970                      | -3.233980 | -0.360000 | 0.056000                    | -4.064000 | -0.451000 |
| 3   | Mn   | 0.000000                | 0.500000 | 0.000000 | 0.047970                      | -3.233980 | 0.360000  | 0.057000                    | -4.064000 | 0.451000  |
| 4   | Mn   | 0.500000                | 0.000000 | 0.500000 | 0.047970                      | 3.233980  | -0.360000 | 0.056000                    | 4.064000  | -0.450000 |
| 5   | Mn   | 0.292000                | 0.250000 | 0.763000 | 0.159020                      | 0.000000  | 0.574050  | 0.279000                    | 0.001000  | 0.992000  |
| 6   | Mn   | 0.792000                | 0.250000 | 0.737000 | 0.159020                      | 0.000000  | -0.574050 | 0.280000                    | 0.000000  | -0.996000 |
| 7   | Mn   | 0.708000                | 0.750000 | 0.237000 | 0.159020                      | 0.000000  | 0.574050  | 0.279000                    | 0.000000  | 0.992000  |
| 8   | Mn   | 0.208000                | 0.750000 | 0.263000 | 0.159020                      | 0.000000  | -0.574050 | 0.280000                    | -0.000000 | -0.996000 |
| 9   | Cs   | 0.494080                | 0.250000 | 0.128890 | 0.000000                      | 0.000000  | 0.000000  | 0.000000                    | 0.000000  | -0.000000 |
| 10  | Cs   | 0.994080                | 0.250000 | 0.371110 | 0.000000                      | 0.000000  | 0.000000  | 0.000000                    | -0.000000 | -0.000000 |
| 11  | Cs   | 0.505920                | 0.750000 | 0.871110 | 0.000000                      | 0.000000  | 0.000000  | 0.000000                    | -0.000000 | -0.000000 |
| 12  | Cs   | 0.005920                | 0.750000 | 0.628890 | 0.000000                      | 0.000000  | 0.000000  | 0.000000                    | 0.000000  | -0.000000 |
| 13  | F    | 0.435700                | 0.250000 | 0.453200 | 0.000000                      | 0.000000  | 0.000000  | 0.001000                    | -0.000000 | -0.007000 |
| 14  | F    | 0.935700                | 0.250000 | 0.046800 | 0.000000                      | 0.000000  | 0.000000  | 0.001000                    | 0.000000  | 0.007000  |
| 15  | F    | 0.564300                | 0.750000 | 0.546800 | 0.000000                      | 0.000000  | 0.000000  | 0.001000                    | 0.000000  | -0.007000 |
| 16  | F    | 0.064300                | 0.750000 | 0.953200 | 0.000000                      | 0.000000  | 0.000000  | 0.001000                    | -0.000000 | 0.007000  |
| 17  | F    | 0.137230                | 0.518900 | 0.154030 | 0.000000                      | 0.000000  | 0.000000  | -0.001000                   | 0.037000  | -0.002000 |
| 18  | F    | 0.637230                | 0.981100 | 0.345970 | 0.000000                      | 0.000000  | 0.000000  | -0.000000                   | -0.036000 | 0.002000  |
| 19  | F    | 0.862770                | 0.481100 | 0.845970 | 0.000000                      | 0.000000  | 0.000000  | -0.001000                   | 0.036000  | -0.002000 |
| 20  | F    | 0.362770                | 0.018900 | 0.654030 | 0.000000                      | 0.000000  | 0.000000  | -0.001000                   | -0.036000 | 0.002000  |
| 21  | F    | 0.862770                | 0.018900 | 0.845970 | 0.000000                      | 0.000000  | 0.000000  | -0.001000                   | -0.037000 | -0.002000 |
| 22  | F    | 0.362770                | 0.481100 | 0.654030 | 0.000000                      | 0.000000  | 0.000000  | -0.000000                   | 0.037000  | 0.002000  |
| 23  | F    | 0.137230                | 0.981100 | 0.154030 | 0.000000                      | 0.000000  | 0.000000  | -0.001000                   | -0.036000 | -0.002000 |
| 24  | F    | 0.637230                | 0.518900 | 0.345970 | 0.000000                      | 0.000000  | 0.000000  | -0.001000                   | 0.036000  | 0.002000  |
| 25  | F    | 0.789520                | 0.567020 | 0.089310 | 0.000000                      | 0.000000  | 0.000000  | 0.001000                    | 0.036000  | 0.001000  |
| 26  | F    | 0.289520                | 0.932980 | 0.410690 | 0.000000                      | 0.000000  | 0.000000  | 0.001000                    | -0.037000 | -0.001000 |
| 27  | F    | 0.210480                | 0.432980 | 0.910690 | 0.000000                      | 0.000000  | 0.000000  | 0.002000                    | 0.036000  | 0.001000  |
| 28  | F    | 0.710480                | 0.067020 | 0.589310 | 0.000000                      | 0.000000  | 0.000000  | 0.002000                    | -0.037000 | -0.001000 |
| 29  | F    | 0.210480                | 0.067020 | 0.910690 | 0.000000                      | 0.000000  | 0.000000  | 0.001000                    | -0.036000 | 0.001000  |
| 30  | F    | 0.710480                | 0.432980 | 0.589310 | 0.000000                      | 0.000000  | 0.000000  | 0.001000                    | 0.037000  | -0.001000 |
| 31  | F    | 0.789520                | 0.932980 | 0.089310 | 0.000000                      | 0.000000  | 0.000000  | 0.002000                    | -0.036000 | 0.001000  |
| 32  | F    | 0.289520                | 0.567020 | 0.410690 | 0.000000                      | 0.000000  | 0.000000  | 0.002000                    | 0.037000  | -0.001000 |
| 33  | F    | 0.545000                | 0.250000 | 0.836520 | 0.000000                      | 0.000000  | 0.000000  | 0.007000                    | -0.000000 | 0.008000  |
| 34  | F    | 0.045000                | 0.250000 | 0.663480 | 0.000000                      | 0.000000  | 0.000000  | 0.007000                    | -0.000000 | -0.007000 |
| 35  | F    | 0.455000                | 0.750000 | 0.163480 | 0.000000                      | 0.000000  | 0.000000  | 0.007000                    | -0.000000 | 0.008000  |
| 36  | F    | 0.955000                | 0.750000 | 0.336520 | 0.000000                      | 0.000000  | 0.000000  | 0.007000                    | 0.000000  | -0.007000 |

FIG. 69. First-principles calculation results of 0.726 CsMn<sub>2</sub>F<sub>6</sub>. The band structure is shown in the left panel, and the Fermi-level-dependent AHC is plotted in the right panel. In both plots, the Fermi level is set to 0 eV.

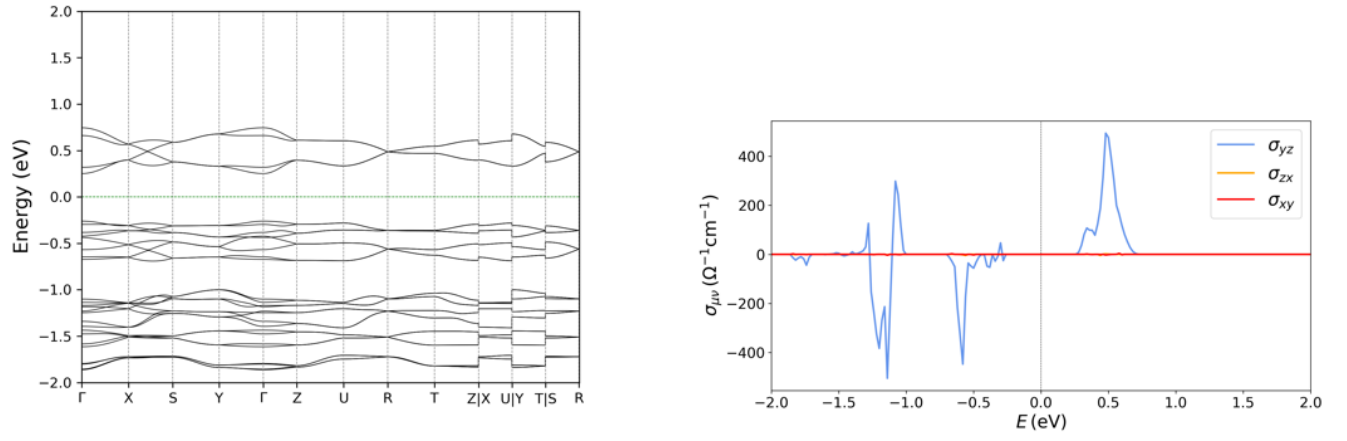



**0.810 Fe<sub>2</sub>WO<sub>6</sub>** crystallizes in type III MSG 60.423, which hosts both SNLs and FNSs. The symmetry-adapted AHC tensor of the MSG is ( $\sigma_{yz}$ , 0, 0). Based on the first-principles calculation results, the comparison between the experimental and calculated magnetic moments is provided in Table SII72. The band structure is shown in the left panel of Fig. 70, and the Fermi-level-dependent AHC is plotted in the right panel.

TABLE SII72. The comparison between the experimental and calculated magnetic moments for 0.810 Fe<sub>2</sub>WO<sub>6</sub>. The five columns contain the atom index in the structure file, the atom species, the fractional coordinates, the experimental magnetic moments, and the calculated magnetic moments. The lattice vectors are  $\vec{a}_1 = (4.576, 0.0, 0.0)$ ,  $\vec{a}_2 = (0.0, 16.766, 0.0)$ ,  $\vec{a}_3 = (0.0, 0.0, 4.967)$ .

| No. | Atom | Coordinates(fractional) |          |          | Experimental magnetic moments |          |           | Calculated magnetic moments |           |           |
|-----|------|-------------------------|----------|----------|-------------------------------|----------|-----------|-----------------------------|-----------|-----------|
| 1   | Fe   | 0.000000                | 0.943600 | 0.250000 | 0.900010                      | 0.000000 | -2.659980 | 1.347000                    | 0.000000  | -3.987000 |
| 2   | Fe   | 0.500000                | 0.556400 | 0.750000 | 0.900010                      | 0.000000 | 2.659980  | 1.349000                    | -0.000000 | 3.986000  |
| 3   | Fe   | 0.000000                | 0.056400 | 0.750000 | 0.900010                      | 0.000000 | -2.659980 | 1.346000                    | 0.000000  | -3.984000 |
| 4   | Fe   | 0.500000                | 0.443600 | 0.250000 | 0.900010                      | 0.000000 | 2.659980  | 1.348000                    | -0.000000 | 3.987000  |
| 5   | Fe   | 0.000000                | 0.275800 | 0.250000 | 0.000000                      | 0.000000 | -1.959980 | -0.003000                   | 0.000000  | -3.303000 |
| 6   | Fe   | 0.500000                | 0.224200 | 0.750000 | 0.000000                      | 0.000000 | 1.959980  | 0.003000                    | -0.000000 | 3.305000  |
| 7   | Fe   | 0.000000                | 0.724200 | 0.750000 | 0.000000                      | 0.000000 | -1.959980 | 0.015000                    | 0.000000  | -3.369000 |
| 8   | Fe   | 0.500000                | 0.775800 | 0.250000 | 0.000000                      | 0.000000 | 1.959980  | 0.005000                    | -0.000000 | 3.280000  |
| 9   | W    | 0.000000                | 0.612750 | 0.250000 | 0.000000                      | 0.000000 | 0.000000  | 0.026000                    | 0.000000  | 0.073000  |
| 10  | W    | 0.500000                | 0.887250 | 0.750000 | 0.000000                      | 0.000000 | 0.000000  | 0.025000                    | -0.000000 | -0.082000 |
| 11  | W    | 0.000000                | 0.387250 | 0.750000 | 0.000000                      | 0.000000 | 0.000000  | 0.024000                    | 0.000000  | 0.078000  |
| 12  | W    | 0.500000                | 0.112750 | 0.250000 | 0.000000                      | 0.000000 | 0.000000  | 0.025000                    | -0.000000 | -0.080000 |
| 13  | O    | 0.740000                | 0.540900 | 0.095800 | 0.000000                      | 0.000000 | 0.000000  | 0.044000                    | -0.001000 | 0.128000  |
| 14  | O    | 0.240000                | 0.959100 | 0.904200 | 0.000000                      | 0.000000 | 0.000000  | 0.042000                    | 0.000000  | -0.123000 |
| 15  | O    | 0.260000                | 0.459100 | 0.904200 | 0.000000                      | 0.000000 | 0.000000  | 0.043000                    | 0.001000  | 0.124000  |
| 16  | O    | 0.760000                | 0.040900 | 0.095800 | 0.000000                      | 0.000000 | 0.000000  | 0.042000                    | -0.001000 | -0.121000 |
| 17  | O    | 0.260000                | 0.540900 | 0.404200 | 0.000000                      | 0.000000 | 0.000000  | 0.044000                    | 0.001000  | 0.128000  |
| 18  | O    | 0.760000                | 0.959100 | 0.595800 | 0.000000                      | 0.000000 | 0.000000  | 0.042000                    | -0.000000 | -0.123000 |
| 19  | O    | 0.740000                | 0.459100 | 0.595800 | 0.000000                      | 0.000000 | 0.000000  | 0.043000                    | -0.001000 | 0.124000  |
| 20  | O    | 0.240000                | 0.040900 | 0.404200 | 0.000000                      | 0.000000 | 0.000000  | 0.042000                    | 0.001000  | -0.121000 |
| 21  | O    | 0.773400                | 0.627100 | 0.569200 | 0.000000                      | 0.000000 | 0.000000  | 0.036000                    | 0.003000  | 0.074000  |
| 22  | O    | 0.273400                | 0.872900 | 0.430800 | 0.000000                      | 0.000000 | 0.000000  | 0.035000                    | -0.002000 | -0.073000 |
| 23  | O    | 0.226600                | 0.372900 | 0.430800 | 0.000000                      | 0.000000 | 0.000000  | 0.036000                    | 0.000000  | 0.074000  |
| 24  | O    | 0.726600                | 0.127100 | 0.569200 | 0.000000                      | 0.000000 | 0.000000  | 0.036000                    | 0.000000  | -0.074000 |
| 25  | O    | 0.226600                | 0.627100 | 0.930800 | 0.000000                      | 0.000000 | 0.000000  | 0.036000                    | -0.003000 | 0.074000  |
| 26  | O    | 0.726600                | 0.872900 | 0.069200 | 0.000000                      | 0.000000 | 0.000000  | 0.035000                    | 0.002000  | -0.073000 |
| 27  | O    | 0.773400                | 0.372900 | 0.069200 | 0.000000                      | 0.000000 | 0.000000  | 0.036000                    | -0.000000 | 0.074000  |
| 28  | O    | 0.273400                | 0.127100 | 0.930800 | 0.000000                      | 0.000000 | 0.000000  | 0.036000                    | -0.000000 | -0.074000 |
| 29  | O    | 0.776000                | 0.703500 | 0.081700 | 0.000000                      | 0.000000 | 0.000000  | 0.013000                    | 0.017000  | 0.030000  |
| 30  | O    | 0.276000                | 0.796500 | 0.918300 | 0.000000                      | 0.000000 | 0.000000  | 0.011000                    | -0.014000 | -0.034000 |
| 31  | O    | 0.224000                | 0.296500 | 0.918300 | 0.000000                      | 0.000000 | 0.000000  | 0.009000                    | 0.019000  | 0.033000  |
| 32  | O    | 0.724000                | 0.203500 | 0.081700 | 0.000000                      | 0.000000 | 0.000000  | 0.008000                    | -0.013000 | -0.039000 |
| 33  | O    | 0.224000                | 0.703500 | 0.418300 | 0.000000                      | 0.000000 | 0.000000  | 0.013000                    | -0.017000 | 0.030000  |
| 34  | O    | 0.724000                | 0.796500 | 0.581700 | 0.000000                      | 0.000000 | 0.000000  | 0.011000                    | 0.014000  | -0.034000 |
| 35  | O    | 0.776000                | 0.296500 | 0.581700 | 0.000000                      | 0.000000 | 0.000000  | 0.009000                    | -0.019000 | 0.033000  |
| 36  | O    | 0.276000                | 0.203500 | 0.418300 | 0.000000                      | 0.000000 | 0.000000  | 0.008000                    | 0.013000  | -0.038000 |

FIG. 70. First-principles calculation results of 0.810 Fe<sub>2</sub>WO<sub>6</sub>. The band structure is shown in the left panel, and the Fermi-level-dependent AHC is plotted in the right panel. In both plots, the Fermi level is set to 0 eV.

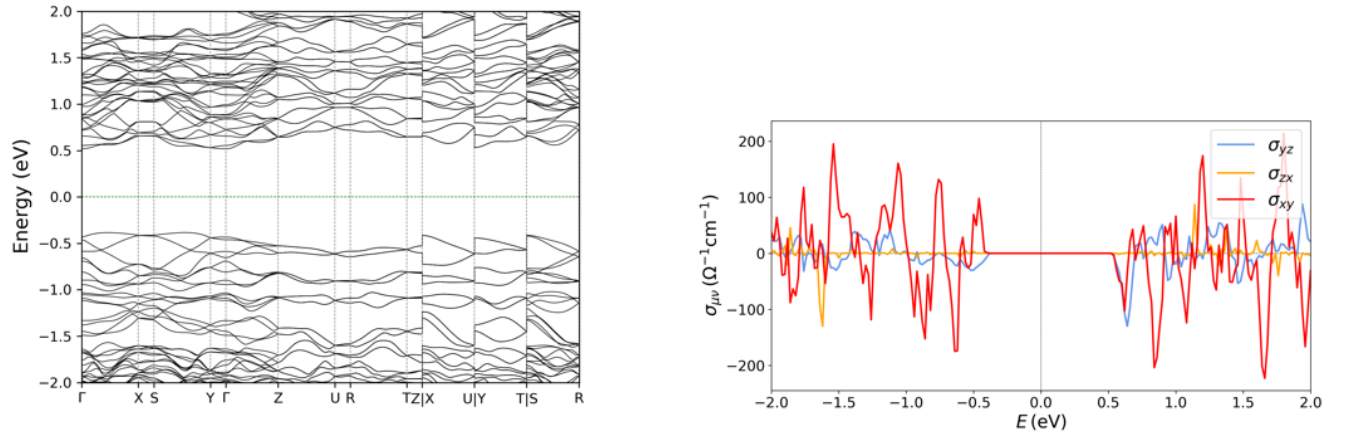

0.811  $\text{Fe}_2\text{WO}_6$  crystallizes in type III MSG 60.423, which hosts both SNLs and FNSs. The symmetry-adapted AHC tensor of the MSG is  $(\sigma_{yz}, 0, 0)$ . Based on the first-principles calculation results, the comparison between the experimental and calculated magnetic moments is provided in Table SII73. The band structure is shown in the left panel of Fig. 71, and the Fermi-level-dependent AHC is plotted in the right panel.

TABLE SII73. The comparison between the experimental and calculated magnetic moments for 0.811  $\text{Fe}_2\text{WO}_6$ . The five columns contain the atom index in the structure file, the atom species, the fractional coordinates, the experimental magnetic moments, and the calculated magnetic moments. The lattice vectors are  $\vec{a}_1 = (4.576, 0.0, 0.0)$ ,  $\vec{a}_2 = (0.0, 16.766, 0.0)$ ,  $\vec{a}_3 = (0.0, 0.0, 4.967)$ .

| No. | Atom | Coordinates(fractional) |          |          | Experimental magnetic moments |          |           | Calculated magnetic moments |           |           |
|-----|------|-------------------------|----------|----------|-------------------------------|----------|-----------|-----------------------------|-----------|-----------|
| 1   | Fe   | 0.000000                | 0.943600 | 0.250000 | 0.000000                      | 0.000000 | -2.550010 | -0.002000                   | -0.001000 | -3.846000 |
| 2   | Fe   | 0.500000                | 0.556400 | 0.750000 | 0.000000                      | 0.000000 | 2.550010  | -0.002000                   | 0.001000  | 3.884000  |
| 3   | Fe   | 0.000000                | 0.056400 | 0.750000 | 0.000000                      | 0.000000 | -2.550010 | 0.002000                    | -0.001000 | -3.842000 |
| 4   | Fe   | 0.500000                | 0.443600 | 0.250000 | 0.000000                      | 0.000000 | 2.550010  | 0.003000                    | 0.001000  | 3.885000  |
| 5   | Fe   | 0.000000                | 0.275800 | 0.250000 | 0.000000                      | 0.000000 | -2.150020 | -0.001000                   | -0.000000 | -3.628000 |
| 6   | Fe   | 0.500000                | 0.224200 | 0.750000 | 0.000000                      | 0.000000 | 2.150020  | 0.001000                    | 0.000000  | 3.591000  |
| 7   | Fe   | 0.000000                | 0.724200 | 0.750000 | 0.000000                      | 0.000000 | -2.150020 | -0.000000                   | -0.000000 | -3.627000 |
| 8   | Fe   | 0.500000                | 0.775800 | 0.250000 | 0.000000                      | 0.000000 | 2.150020  | -0.003000                   | 0.000000  | 3.589000  |
| 9   | W    | 0.000000                | 0.612750 | 0.250000 | 0.000000                      | 0.000000 | 0.000000  | 0.001000                    | 0.000000  | 0.117000  |
| 10  | W    | 0.500000                | 0.887250 | 0.750000 | 0.000000                      | 0.000000 | 0.000000  | -0.002000                   | -0.000000 | -0.120000 |
| 11  | W    | 0.000000                | 0.387250 | 0.750000 | 0.000000                      | 0.000000 | 0.000000  | -0.002000                   | 0.000000  | 0.120000  |
| 12  | W    | 0.500000                | 0.112750 | 0.250000 | 0.000000                      | 0.000000 | 0.000000  | 0.001000                    | -0.000000 | -0.121000 |
| 13  | O    | 0.740000                | 0.540900 | 0.095800 | 0.000000                      | 0.000000 | 0.000000  | 0.000000                    | -0.001000 | 0.145000  |
| 14  | O    | 0.240000                | 0.959100 | 0.904200 | 0.000000                      | 0.000000 | 0.000000  | 0.000000                    | 0.001000  | -0.137000 |
| 15  | O    | 0.260000                | 0.459100 | 0.904200 | 0.000000                      | 0.000000 | 0.000000  | 0.001000                    | 0.000000  | 0.141000  |
| 16  | O    | 0.760000                | 0.040900 | 0.095800 | 0.000000                      | 0.000000 | 0.000000  | 0.001000                    | -0.001000 | -0.135000 |
| 17  | O    | 0.260000                | 0.540900 | 0.404200 | 0.000000                      | 0.000000 | 0.000000  | 0.000000                    | 0.001000  | 0.145000  |
| 18  | O    | 0.760000                | 0.959100 | 0.595800 | 0.000000                      | 0.000000 | 0.000000  | 0.001000                    | -0.001000 | -0.137000 |
| 19  | O    | 0.740000                | 0.459100 | 0.595800 | 0.000000                      | 0.000000 | 0.000000  | 0.001000                    | -0.000000 | 0.141000  |
| 20  | O    | 0.240000                | 0.040900 | 0.404200 | 0.000000                      | 0.000000 | 0.000000  | 0.001000                    | 0.001000  | -0.135000 |
| 21  | O    | 0.773400                | 0.627100 | 0.569200 | 0.000000                      | 0.000000 | 0.000000  | -0.002000                   | 0.002000  | 0.097000  |
| 22  | O    | 0.273400                | 0.872900 | 0.430800 | 0.000000                      | 0.000000 | 0.000000  | -0.001000                   | -0.001000 | -0.098000 |
| 23  | O    | 0.226600                | 0.372900 | 0.430800 | 0.000000                      | 0.000000 | 0.000000  | -0.001000                   | -0.001000 | 0.097000  |
| 24  | O    | 0.726600                | 0.127100 | 0.569200 | 0.000000                      | 0.000000 | 0.000000  | -0.002000                   | 0.002000  | -0.099000 |
| 25  | O    | 0.226600                | 0.627100 | 0.930800 | 0.000000                      | 0.000000 | 0.000000  | -0.002000                   | -0.002000 | 0.097000  |
| 26  | O    | 0.726600                | 0.872900 | 0.069200 | 0.000000                      | 0.000000 | 0.000000  | -0.001000                   | 0.001000  | -0.098000 |
| 27  | O    | 0.773400                | 0.372900 | 0.069200 | 0.000000                      | 0.000000 | 0.000000  | -0.001000                   | 0.001000  | 0.097000  |
| 28  | O    | 0.273400                | 0.127100 | 0.930800 | 0.000000                      | 0.000000 | 0.000000  | -0.002000                   | -0.002000 | -0.099000 |
| 29  | O    | 0.776000                | 0.703500 | 0.081700 | 0.000000                      | 0.000000 | 0.000000  | 0.000000                    | -0.001000 | 0.038000  |
| 30  | O    | 0.276000                | 0.796500 | 0.918300 | 0.000000                      | 0.000000 | 0.000000  | 0.000000                    | 0.001000  | -0.042000 |
| 31  | O    | 0.224000                | 0.296500 | 0.918300 | 0.000000                      | 0.000000 | 0.000000  | 0.001000                    | 0.000000  | 0.038000  |
| 32  | O    | 0.724000                | 0.203500 | 0.081700 | 0.000000                      | 0.000000 | 0.000000  | 0.000000                    | 0.000000  | -0.043000 |
| 33  | O    | 0.224000                | 0.703500 | 0.418300 | 0.000000                      | 0.000000 | 0.000000  | 0.000000                    | 0.001000  | 0.038000  |
| 34  | O    | 0.724000                | 0.796500 | 0.581700 | 0.000000                      | 0.000000 | 0.000000  | 0.000000                    | -0.001000 | -0.042000 |
| 35  | O    | 0.776000                | 0.296500 | 0.581700 | 0.000000                      | 0.000000 | 0.000000  | 0.001000                    | -0.000000 | 0.038000  |
| 36  | O    | 0.276000                | 0.203500 | 0.418300 | 0.000000                      | 0.000000 | 0.000000  | 0.000000                    | -0.000000 | -0.043000 |

FIG. 71. First-principles calculation results of 0.811 Fe<sub>2</sub>WO<sub>6</sub>. The band structure is shown in the left panel, and the Fermi-level-dependent AHC is plotted in the right panel. In both plots, the Fermi level is set to 0 eV.

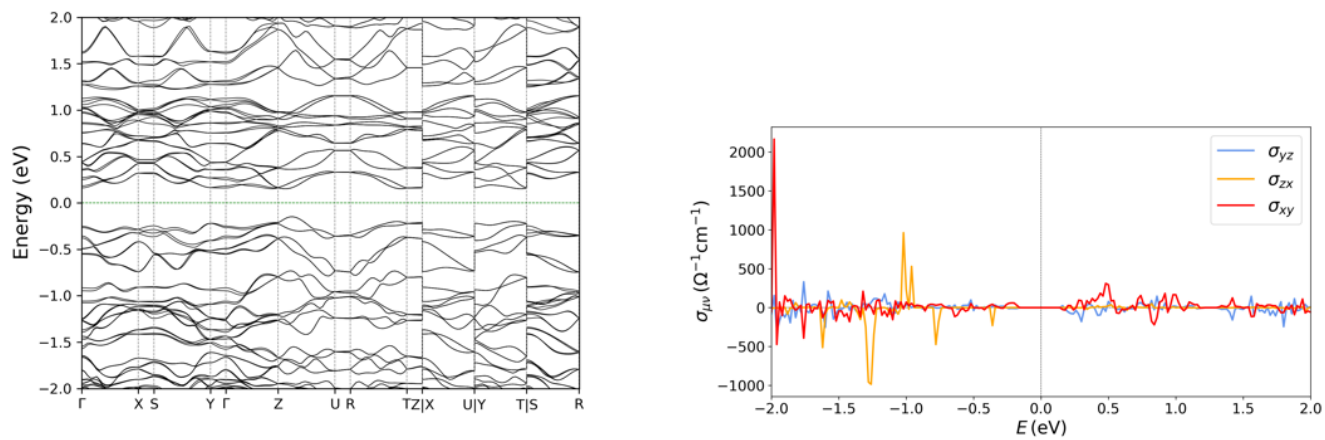

**0.812 Fe<sub>2</sub>WO<sub>6</sub>** crystallizes in type III MSG 30.113, which hosts only SNLs. The symmetry-adapted AHC tensor of the MSG is  $(0, \sigma_{zx}, 0)$ . Based on the first-principles calculation results, the comparison between the experimental and calculated magnetic moments is provided in Table SII74. The band structure is shown in the left panel of Fig. 72, and the Fermi-level-dependent AHC is plotted in the right panel.

TABLE SII74. The comparison between the experimental and calculated magnetic moments for 0.812 Fe<sub>2</sub>WO<sub>6</sub>. The five columns contain the atom index in the structure file, the atom species, the fractional coordinates, the experimental magnetic moments, and the calculated magnetic moments. The lattice vectors are  $\vec{a}_1 = (4.967, 0.0, 0.0)$ ,  $\vec{a}_2 = (0.0, 4.576, 0.0)$ ,  $\vec{a}_3 = (0.0, 0.0, 16.766)$ .

| No. | Atom | Coordinates(fractional) |          |          | Experimental magnetic moments |           |          | Calculated magnetic moments |           |           |
|-----|------|-------------------------|----------|----------|-------------------------------|-----------|----------|-----------------------------|-----------|-----------|
| 1   | Fe   | 0.000000                | 0.000000 | 0.556400 | -3.120020                     | 1.359990  | 0.000000 | -3.460000                   | 1.708000  | -0.026000 |
| 2   | Fe   | 0.000000                | 0.500000 | 0.056400 | 3.120020                      | 1.359990  | 0.000000 | 3.465000                    | 1.705000  | 0.026000  |
| 3   | Fe   | 0.500000                | 0.000000 | 0.443600 | -3.120020                     | -1.359990 | 0.000000 | -3.433000                   | -1.758000 | -0.008000 |
| 4   | Fe   | 0.500000                | 0.500000 | 0.943600 | 3.120020                      | -1.359990 | 0.000000 | 3.434000                    | -1.756000 | 0.008000  |
| 5   | Fe   | 0.000000                | 0.000000 | 0.224200 | -3.120020                     | -1.359990 | 0.000000 | -3.332000                   | -1.391000 | -0.064000 |
| 6   | Fe   | 0.000000                | 0.500000 | 0.724200 | 3.120020                      | -1.359990 | 0.000000 | 3.335000                    | -1.392000 | 0.065000  |
| 7   | Fe   | 0.500000                | 0.000000 | 0.775800 | -3.120020                     | 1.359990  | 0.000000 | -3.325000                   | 1.406000  | -0.063000 |
| 8   | Fe   | 0.500000                | 0.500000 | 0.275800 | 3.120020                      | 1.359990  | 0.000000 | 3.326000                    | 1.404000  | 0.063000  |
| 9   | W    | 0.000000                | 0.000000 | 0.887250 | 0.000000                      | 0.000000  | 0.000000 | 0.108000                    | -0.025000 | 0.001000  |
| 10  | W    | 0.000000                | 0.500000 | 0.387250 | 0.000000                      | 0.000000  | 0.000000 | -0.106000                   | -0.026000 | -0.001000 |
| 11  | W    | 0.500000                | 0.000000 | 0.112750 | 0.000000                      | 0.000000  | 0.000000 | 0.104000                    | 0.023000  | 0.001000  |
| 12  | W    | 0.500000                | 0.500000 | 0.612750 | 0.000000                      | 0.000000  | 0.000000 | -0.107000                   | 0.023000  | -0.001000 |
| 13  | O    | 0.345800                | 0.740000 | 0.040900 | 0.000000                      | 0.000000  | 0.000000 | 0.125000                    | 0.013000  | -0.001000 |
| 14  | O    | 0.345800                | 0.760000 | 0.540900 | 0.000000                      | 0.000000  | 0.000000 | -0.121000                   | 0.014000  | -0.001000 |
| 15  | O    | 0.654200                | 0.260000 | 0.040900 | 0.000000                      | 0.000000  | 0.000000 | 0.125000                    | 0.013000  | 0.002000  |
| 16  | O    | 0.654200                | 0.240000 | 0.540900 | 0.000000                      | 0.000000  | 0.000000 | -0.121000                   | 0.014000  | -0.001000 |
| 17  | O    | 0.845800                | 0.760000 | 0.459100 | 0.000000                      | 0.000000  | 0.000000 | -0.125000                   | -0.014000 | -0.001000 |
| 18  | O    | 0.845800                | 0.740000 | 0.959100 | 0.000000                      | 0.000000  | 0.000000 | 0.123000                    | -0.014000 | -0.001000 |
| 19  | O    | 0.154200                | 0.240000 | 0.459100 | 0.000000                      | 0.000000  | 0.000000 | -0.125000                   | -0.014000 | -0.000000 |
| 20  | O    | 0.154200                | 0.260000 | 0.959100 | 0.000000                      | 0.000000  | 0.000000 | 0.123000                    | -0.014000 | 0.002000  |
| 21  | O    | 0.819200                | 0.773400 | 0.127100 | 0.000000                      | 0.000000  | 0.000000 | 0.086000                    | 0.039000  | 0.002000  |
| 22  | O    | 0.819200                | 0.726600 | 0.627100 | 0.000000                      | 0.000000  | 0.000000 | -0.086000                   | 0.039000  | 0.001000  |
| 23  | O    | 0.180800                | 0.226600 | 0.127100 | 0.000000                      | 0.000000  | 0.000000 | 0.086000                    | 0.039000  | -0.001000 |
| 24  | O    | 0.180800                | 0.273400 | 0.627100 | 0.000000                      | 0.000000  | 0.000000 | -0.086000                   | 0.039000  | -0.002000 |
| 25  | O    | 0.319200                | 0.726600 | 0.372900 | 0.000000                      | 0.000000  | 0.000000 | -0.085000                   | -0.043000 | 0.001000  |
| 26  | O    | 0.319200                | 0.773400 | 0.872900 | 0.000000                      | 0.000000  | 0.000000 | 0.085000                    | -0.043000 | 0.001000  |
| 27  | O    | 0.680800                | 0.273400 | 0.372900 | 0.000000                      | 0.000000  | 0.000000 | -0.085000                   | -0.043000 | -0.001000 |
| 28  | O    | 0.680800                | 0.226600 | 0.872900 | 0.000000                      | 0.000000  | 0.000000 | 0.085000                    | -0.043000 | -0.002000 |
| 29  | O    | 0.331700                | 0.776000 | 0.203500 | 0.000000                      | 0.000000  | 0.000000 | 0.036000                    | 0.013000  | -0.001000 |
| 30  | O    | 0.331700                | 0.724000 | 0.703500 | 0.000000                      | 0.000000  | 0.000000 | -0.036000                   | 0.013000  | -0.001000 |
| 31  | O    | 0.668300                | 0.224000 | 0.203500 | 0.000000                      | 0.000000  | 0.000000 | 0.036000                    | 0.013000  | 0.001000  |
| 32  | O    | 0.668300                | 0.276000 | 0.703500 | 0.000000                      | 0.000000  | 0.000000 | -0.036000                   | 0.013000  | 0.000000  |
| 33  | O    | 0.831700                | 0.724000 | 0.296500 | 0.000000                      | 0.000000  | 0.000000 | -0.036000                   | -0.012000 | -0.001000 |
| 34  | O    | 0.831700                | 0.776000 | 0.796500 | 0.000000                      | 0.000000  | 0.000000 | 0.037000                    | -0.012000 | 0.001000  |
| 35  | O    | 0.168300                | 0.276000 | 0.296500 | 0.000000                      | 0.000000  | 0.000000 | -0.036000                   | -0.012000 | 0.000000  |
| 36  | O    | 0.168300                | 0.224000 | 0.796500 | 0.000000                      | 0.000000  | 0.000000 | 0.037000                    | -0.012000 | 0.000000  |

FIG. 72. First-principles calculation results of 0.812 Fe<sub>2</sub>WO<sub>6</sub>. The band structure is shown in the left panel, and the Fermi-level-dependent AHC is plotted in the right panel. In both plots, the Fermi level is set to 0 eV.

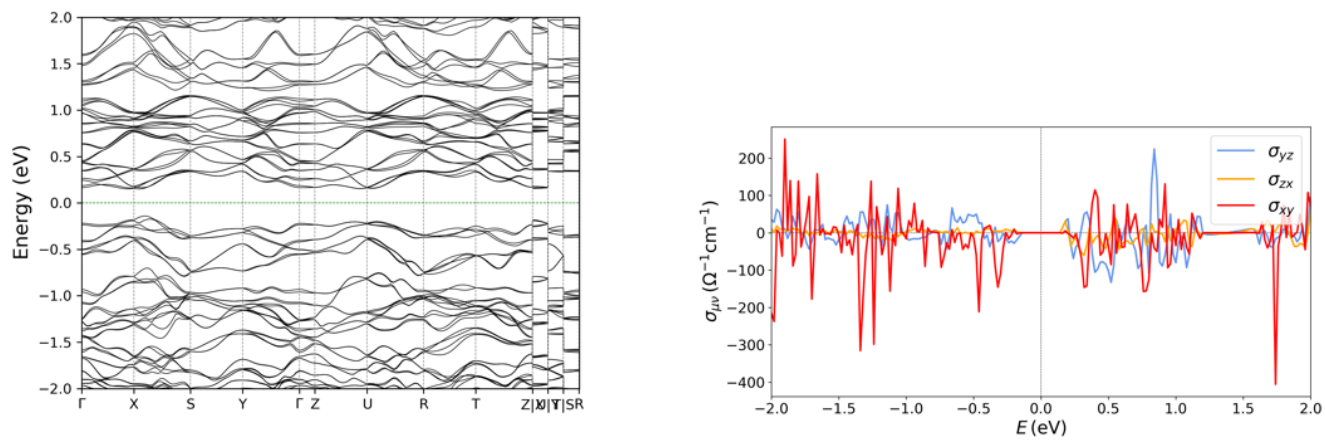

0.813  $\text{Fe}_2\text{WO}_6$  crystallizes in type III MSG 60.423, which hosts both SNLs and FNSs. The symmetry-adapted AHC tensor of the MSG is  $(\sigma_{yz}, 0, 0)$ . Based on the first-principles calculation results, the comparison between the experimental and calculated magnetic moments is provided in Table SII75. The band structure is shown in the left panel of Fig. 73, and the Fermi-level-dependent AHC is plotted in the right panel.

TABLE SII75. The comparison between the experimental and calculated magnetic moments for 0.813  $\text{Fe}_2\text{WO}_6$ . The five columns contain the atom index in the structure file, the atom species, the fractional coordinates, the experimental magnetic moments, and the calculated magnetic moments. The lattice vectors are  $\vec{a}_1 = (4.562, 0.0, 0.0)$ ,  $\vec{a}_2 = (0.0, 16.699, 0.0)$ ,  $\vec{a}_3 = (0.0, 0.0, 4.953)$ .

| No. | Atom | Coordinates(fractional) |          |          | Experimental magnetic moments |          |           | Calculated magnetic moments |           |           |
|-----|------|-------------------------|----------|----------|-------------------------------|----------|-----------|-----------------------------|-----------|-----------|
| 1   | Fe   | 0.000000                | 0.942800 | 0.250000 | 0.000000                      | 0.000000 | -3.599990 | 0.046000                    | 0.000000  | -3.840000 |
| 2   | Fe   | 0.500000                | 0.557200 | 0.750000 | 0.000000                      | 0.000000 | 3.599990  | 0.047000                    | -0.000000 | 3.875000  |
| 3   | Fe   | 0.000000                | 0.057200 | 0.750000 | 0.000000                      | 0.000000 | -3.599990 | 0.050000                    | 0.000000  | -3.835000 |
| 4   | Fe   | 0.500000                | 0.442800 | 0.250000 | 0.000000                      | 0.000000 | 3.599990  | 0.050000                    | -0.000000 | 3.877000  |
| 5   | Fe   | 0.000000                | 0.274300 | 0.250000 | 0.000000                      | 0.000000 | -4.500000 | -0.013000                   | 0.000000  | -3.614000 |
| 6   | Fe   | 0.500000                | 0.225700 | 0.750000 | 0.000000                      | 0.000000 | 4.500000  | -0.009000                   | -0.000000 | 3.579000  |
| 7   | Fe   | 0.000000                | 0.725700 | 0.750000 | 0.000000                      | 0.000000 | -4.500000 | -0.010000                   | 0.000000  | -3.611000 |
| 8   | Fe   | 0.500000                | 0.774300 | 0.250000 | 0.000000                      | 0.000000 | 4.500000  | -0.014000                   | -0.000000 | 3.577000  |
| 9   | W    | 0.000000                | 0.612900 | 0.250000 | 0.000000                      | 0.000000 | 0.000000  | 0.002000                    | -0.000000 | 0.120000  |
| 10  | W    | 0.500000                | 0.887100 | 0.750000 | 0.000000                      | 0.000000 | 0.000000  | -0.001000                   | 0.000000  | -0.123000 |
| 11  | W    | 0.000000                | 0.387100 | 0.750000 | 0.000000                      | 0.000000 | 0.000000  | -0.001000                   | -0.000000 | 0.124000  |
| 12  | W    | 0.500000                | 0.112900 | 0.250000 | 0.000000                      | 0.000000 | 0.000000  | 0.003000                    | 0.000000  | -0.125000 |
| 13  | O    | 0.750000                | 0.541800 | 0.081000 | 0.000000                      | 0.000000 | 0.000000  | 0.002000                    | -0.001000 | 0.142000  |
| 14  | O    | 0.250000                | 0.958200 | 0.919000 | 0.000000                      | 0.000000 | 0.000000  | 0.002000                    | 0.001000  | -0.135000 |
| 15  | O    | 0.250000                | 0.458200 | 0.919000 | 0.000000                      | 0.000000 | 0.000000  | 0.003000                    | -0.000000 | 0.138000  |
| 16  | O    | 0.750000                | 0.041800 | 0.081000 | 0.000000                      | 0.000000 | 0.000000  | 0.002000                    | -0.001000 | -0.133000 |
| 17  | O    | 0.250000                | 0.541800 | 0.419000 | 0.000000                      | 0.000000 | 0.000000  | 0.002000                    | 0.001000  | 0.142000  |
| 18  | O    | 0.750000                | 0.958200 | 0.581000 | 0.000000                      | 0.000000 | 0.000000  | 0.002000                    | -0.001000 | -0.135000 |
| 19  | O    | 0.750000                | 0.458200 | 0.581000 | 0.000000                      | 0.000000 | 0.000000  | 0.003000                    | 0.000000  | 0.138000  |
| 20  | O    | 0.250000                | 0.041800 | 0.419000 | 0.000000                      | 0.000000 | 0.000000  | 0.002000                    | 0.001000  | -0.133000 |
| 21  | O    | 0.770000                | 0.628100 | 0.568000 | 0.000000                      | 0.000000 | 0.000000  | 0.000000                    | 0.002000  | 0.109000  |
| 22  | O    | 0.270000                | 0.871900 | 0.432000 | 0.000000                      | 0.000000 | 0.000000  | 0.001000                    | -0.000000 | -0.110000 |
| 23  | O    | 0.230000                | 0.371900 | 0.432000 | 0.000000                      | 0.000000 | 0.000000  | 0.001000                    | -0.001000 | 0.109000  |
| 24  | O    | 0.730000                | 0.128100 | 0.568000 | 0.000000                      | 0.000000 | 0.000000  | -0.000000                   | 0.002000  | -0.111000 |
| 25  | O    | 0.230000                | 0.628100 | 0.932000 | 0.000000                      | 0.000000 | 0.000000  | 0.000000                    | -0.002000 | 0.109000  |
| 26  | O    | 0.730000                | 0.871900 | 0.068000 | 0.000000                      | 0.000000 | 0.000000  | 0.001000                    | 0.001000  | -0.110000 |
| 27  | O    | 0.770000                | 0.371900 | 0.068000 | 0.000000                      | 0.000000 | 0.000000  | 0.001000                    | 0.001000  | 0.109000  |
| 28  | O    | 0.270000                | 0.128100 | 0.932000 | 0.000000                      | 0.000000 | 0.000000  | -0.000000                   | -0.002000 | -0.111000 |
| 29  | O    | 0.785000                | 0.705700 | 0.094000 | 0.000000                      | 0.000000 | 0.000000  | 0.000000                    | -0.000000 | 0.057000  |
| 30  | O    | 0.285000                | 0.794300 | 0.906000 | 0.000000                      | 0.000000 | 0.000000  | -0.000000                   | 0.001000  | -0.060000 |
| 31  | O    | 0.215000                | 0.294300 | 0.906000 | 0.000000                      | 0.000000 | 0.000000  | 0.001000                    | 0.000000  | 0.056000  |
| 32  | O    | 0.715000                | 0.205700 | 0.094000 | 0.000000                      | 0.000000 | 0.000000  | 0.000000                    | -0.000000 | -0.061000 |
| 33  | O    | 0.215000                | 0.705700 | 0.406000 | 0.000000                      | 0.000000 | 0.000000  | 0.000000                    | 0.000000  | 0.057000  |
| 34  | O    | 0.715000                | 0.794300 | 0.594000 | 0.000000                      | 0.000000 | 0.000000  | -0.000000                   | -0.001000 | -0.060000 |
| 35  | O    | 0.785000                | 0.294300 | 0.594000 | 0.000000                      | 0.000000 | 0.000000  | 0.001000                    | -0.000000 | 0.056000  |
| 36  | O    | 0.285000                | 0.205700 | 0.406000 | 0.000000                      | 0.000000 | 0.000000  | 0.000000                    | 0.000000  | -0.061000 |



FIG. 73. First-principles calculation results of 0.813  $\text{Fe}_2\text{WO}_6$ . The band structure is shown in the left panel, and the Fermi-level-dependent AHC is plotted in the right panel. In both plots, the Fermi level is set to 0 eV.

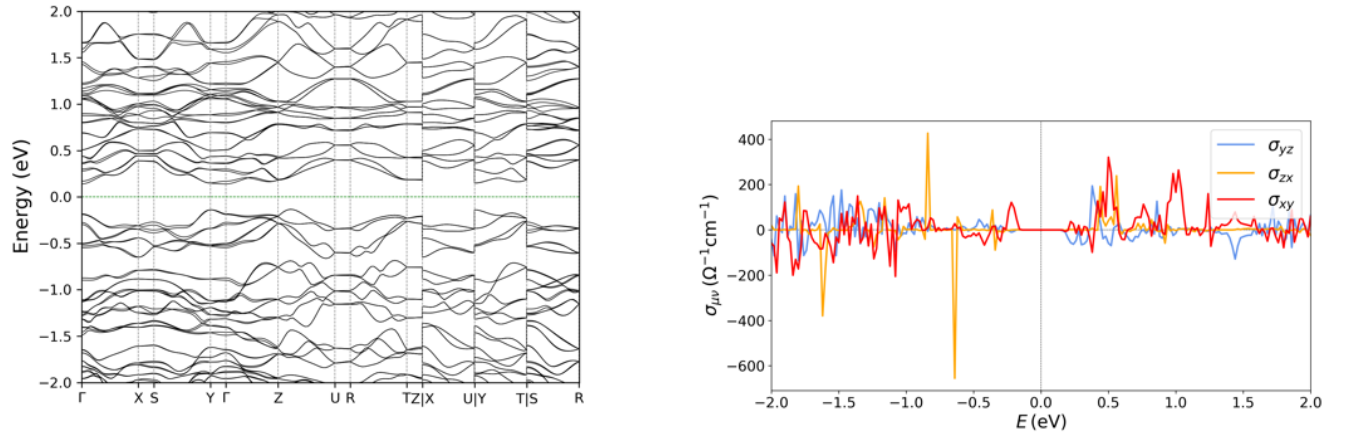

**0.886 SnCo<sub>2</sub>O<sub>4</sub>** crystallizes in type III MSG 141.557, which hosts only SNLs. The symmetry-adapted AHC tensor of the MSG is  $(0, 0, \sigma_{xy})$ . Based on the first-principles calculation results, the comparison between the experimental and calculated magnetic moments is provided in Table SII76. The band structure is shown in the left panel of Fig. 74, and the Fermi-level-dependent AHC is plotted in the right panel.

TABLE SII76. The comparison between the experimental and calculated magnetic moments for 0.886 SnCo<sub>2</sub>O<sub>4</sub>. The five columns contain the atom index in the structure file, the atom species, the fractional coordinates, the experimental magnetic moments, and the calculated magnetic moments. The lattice vectors are  $\vec{a}_1 = (-3.056115, 3.056115, 4.322)$ ,  $\vec{a}_2 = (3.056115, -3.056115, 4.322)$ ,  $\vec{a}_3 = (3.056115, 3.056115, -4.322)$ .

| No. | Atom | Coordinates(fractional) |          |          | Experimental magnetic moments |          |           | Calculated magnetic moments |           |           |
|-----|------|-------------------------|----------|----------|-------------------------------|----------|-----------|-----------------------------|-----------|-----------|
| 1   | Co   | 0.500000                | 0.500000 | 0.000000 | 0.000000                      | 0.000000 | -2.570030 | 0.003000                    | 0.000000  | -3.151000 |
| 2   | Co   | 0.000000                | 0.500000 | 0.500000 | 0.000000                      | 0.000000 | -2.570030 | 0.001000                    | 0.002000  | -3.009000 |
| 3   | Co   | 0.500000                | 0.000000 | 0.000000 | 0.000000                      | 0.000000 | -2.570030 | 0.000000                    | -0.001000 | -3.228000 |
| 4   | Co   | 0.500000                | 0.500000 | 0.500000 | 0.000000                      | 0.000000 | -2.570030 | -0.004000                   | 0.002000  | -3.153000 |
| 5   | Sn   | 0.875000                | 0.125000 | 0.750000 | 0.000000                      | 0.000000 | 0.000000  | -0.000000                   | -0.001000 | -0.046000 |
| 6   | Sn   | 0.125000                | 0.875000 | 0.250000 | 0.000000                      | 0.000000 | 0.000000  | 0.000000                    | -0.000000 | 0.011000  |
| 7   | Sn   | 0.262000                | 0.254000 | 0.008000 | 0.000000                      | 0.000000 | 0.000000  | -0.000000                   | -0.000000 | 0.073000  |
| 8   | O    | 0.746000                | 0.254000 | 0.492000 | 0.000000                      | 0.000000 | 0.000000  | 0.001000                    | 0.001000  | -0.027000 |
| 9   | O    | 0.254000                | 0.746000 | 0.992000 | 0.000000                      | 0.000000 | 0.000000  | 0.000000                    | -0.000000 | -0.017000 |
| 10  | O    | 0.254000                | 0.262000 | 0.508000 | 0.000000                      | 0.000000 | 0.000000  | 0.000000                    | 0.001000  | -0.018000 |
| 11  | O    | 0.738000                | 0.746000 | 0.992000 | 0.000000                      | 0.000000 | 0.000000  | -0.000000                   | -0.000000 | -0.001000 |
| 12  | O    | 0.254000                | 0.746000 | 0.508000 | 0.000000                      | 0.000000 | 0.000000  | 0.000000                    | -0.000000 | -0.017000 |
| 13  | O    | 0.746000                | 0.254000 | 0.008000 | 0.000000                      | 0.000000 | 0.000000  | -0.001000                   | 0.000000  | -0.027000 |

FIG. 74. First-principles calculation results of 0.886 SnCo<sub>2</sub>O<sub>4</sub>. The band structure is shown in the left panel, and the Fermi-level-dependent AHC is plotted in the right panel. In both plots, the Fermi level is set to 0 eV.

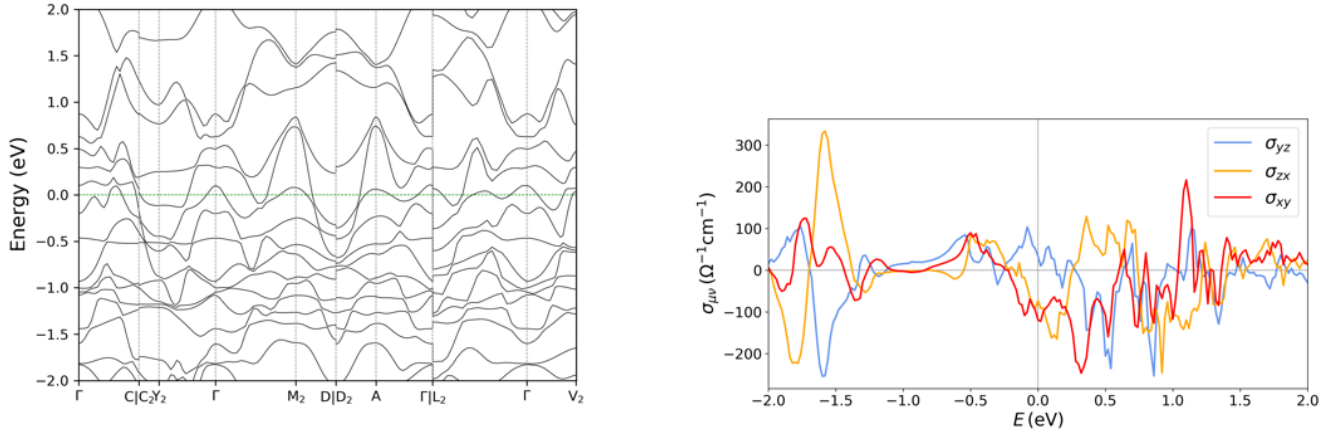

**0.137 Cu<sub>2</sub>V<sub>2</sub>O<sub>7</sub>** crystallizes in type III MSG 141.557, which hosts only SNLs. The symmetry-adapted AHC tensor of the MSG is  $(0, 0, \sigma_{xy})$ . Based on the first-principles calculation results, the comparison between the experimental and calculated magnetic moments is provided in Table SII77. The band structure is shown in the left panel of Fig. 75, and the Fermi-level-dependent AHC is plotted in the right panel.

TABLE SII77. The comparison between the experimental and calculated magnetic moments for 0.137 Cu<sub>2</sub>V<sub>2</sub>O<sub>7</sub>. The five columns contain the atom index in the structure file, the atom species, the fractional coordinates, the experimental magnetic moments, and the calculated magnetic moments. The lattice vectors are  $\vec{a}_1 = (0.0, 4.2025, 3.223)$ ,  $\vec{a}_2 = (10.339, 0.0, 3.223)$ ,  $\vec{a}_3 = (10.339, 4.2025, 0.0)$ .

| No. | Atom | Coordinates(fractional) |          |          | Experimental magnetic moments |          |          | Calculated magnetic moments |           |           |
|-----|------|-------------------------|----------|----------|-------------------------------|----------|----------|-----------------------------|-----------|-----------|
| 1   | Cu   | 0.701090                | 0.302910 | 0.028110 | 0.930100                      | 0.000000 | 0.000000 | 0.734000                    | -0.011000 | -0.006000 |
| 2   | Cu   | 0.302910                | 0.701090 | 0.967890 | -0.930100                     | 0.000000 | 0.000000 | -0.729000                   | 0.013000  | -0.004000 |
| 3   | Cu   | 0.282110                | 0.221890 | 0.947090 | -0.930100                     | 0.000000 | 0.000000 | -0.724000                   | -0.007000 | -0.010000 |
| 4   | Cu   | 0.221890                | 0.282110 | 0.548910 | 0.930100                      | 0.000000 | 0.000000 | 0.731000                    | 0.008000  | -0.008000 |
| 5   | V    | 0.192600                | 0.781400 | 0.616600 | 0.000000                      | 0.000000 | 0.000000 | 0.012000                    | -0.011000 | 0.004000  |
| 6   | V    | 0.781400                | 0.192600 | 0.409400 | 0.000000                      | 0.000000 | 0.000000 | 0.013000                    | -0.010000 | -0.002000 |
| 7   | V    | 0.840600                | 0.633400 | 0.468600 | 0.000000                      | 0.000000 | 0.000000 | -0.014000                   | -0.004000 | 0.015000  |
| 8   | V    | 0.633400                | 0.840600 | 0.057400 | 0.000000                      | 0.000000 | 0.000000 | -0.021000                   | 0.001000  | -0.009000 |
| 9   | O    | 0.337900                | 0.706700 | 0.785400 | 0.000000                      | 0.000000 | 0.000000 | -0.028000                   | -0.001000 | -0.003000 |
| 10  | O    | 0.706700                | 0.337900 | 0.170000 | 0.000000                      | 0.000000 | 0.000000 | 0.022000                    | 0.003000  | -0.002000 |
| 11  | O    | 0.080000                | 0.464600 | 0.543300 | 0.000000                      | 0.000000 | 0.000000 | 0.037000                    | 0.002000  | -0.010000 |
| 12  | O    | 0.464600                | 0.080000 | 0.912100 | 0.000000                      | 0.000000 | 0.000000 | -0.032000                   | -0.002000 | -0.006000 |
| 13  | O    | 0.072080                | 0.485120 | 0.803440 | 0.000000                      | 0.000000 | 0.000000 | 0.004000                    | -0.000000 | -0.008000 |
| 14  | O    | 0.485120                | 0.072080 | 0.639360 | 0.000000                      | 0.000000 | 0.000000 | -0.006000                   | 0.002000  | 0.006000  |
| 15  | O    | 0.610640                | 0.446560 | 0.764880 | 0.000000                      | 0.000000 | 0.000000 | 0.002000                    | -0.000000 | -0.002000 |
| 16  | O    | 0.446560                | 0.610640 | 0.177920 | 0.000000                      | 0.000000 | 0.000000 | 0.001000                    | 0.001000  | 0.003000  |
| 17  | O    | 0.389180                | 0.021020 | 0.302980 | 0.000000                      | 0.000000 | 0.000000 | 0.012000                    | 0.005000  | 0.003000  |
| 18  | O    | 0.021020                | 0.389180 | 0.286820 | 0.000000                      | 0.000000 | 0.000000 | -0.039000                   | 0.004000  | -0.001000 |
| 19  | O    | 0.963180                | 0.947020 | 0.228980 | 0.000000                      | 0.000000 | 0.000000 | -0.031000                   | -0.000000 | -0.006000 |
| 20  | O    | 0.947020                | 0.963180 | 0.860820 | 0.000000                      | 0.000000 | 0.000000 | 0.041000                    | -0.001000 | 0.003000  |
| 21  | O    | 0.650700                | 0.650700 | 0.349300 | 0.000000                      | 0.000000 | 0.000000 | 0.013000                    | 0.001000  | -0.001000 |
| 22  | O    | 0.900700                | 0.900700 | 0.599300 | 0.000000                      | 0.000000 | 0.000000 | -0.005000                   | 0.005000  | -0.001000 |

FIG. 75. First-principles calculation results of 0.137 Cu<sub>2</sub>V<sub>2</sub>O<sub>7</sub>. The band structure is shown in the left panel, and the Fermi-level-dependent AHC is plotted in the right panel. In both plots, the Fermi level is set to 0 eV.

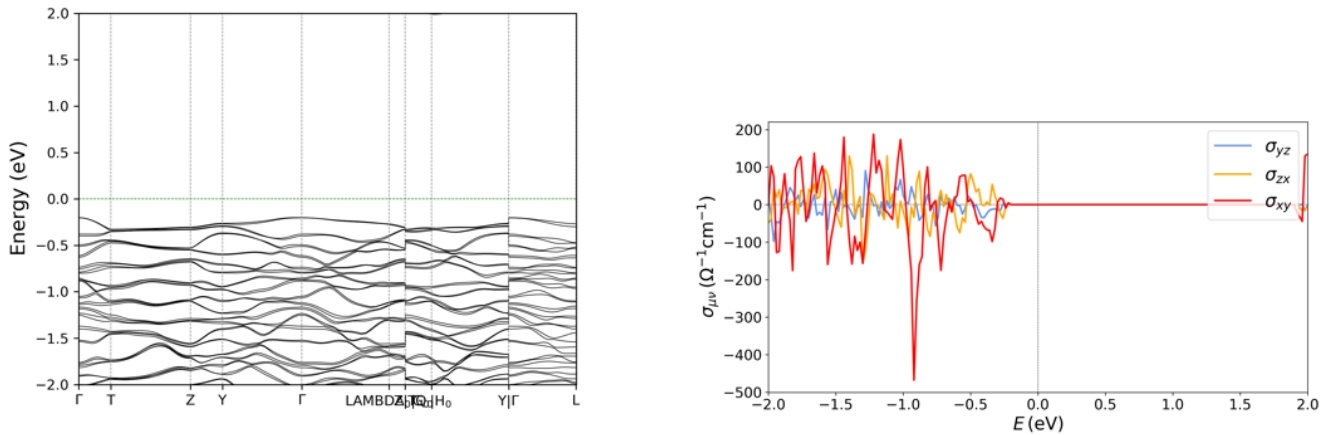

**0.164 Y<sub>2</sub>MnCoO<sub>6</sub>** crystallizes in type III MSG 141.557, which hosts only SNLs. The symmetry-adapted AHC tensor of the MSG is  $(0, 0, \sigma_{xy})$ . Based on the first-principles calculation results, the comparison between the experimental and calculated magnetic moments is provided in Table SII78. The band structure is shown in the left panel of Fig. 76, and the Fermi-level-dependent AHC is plotted in the right panel.

TABLE SII78. The comparison between the experimental and calculated magnetic moments for 0.164 Y<sub>2</sub>MnCoO<sub>6</sub>. The five columns contain the atom index in the structure file, the atom species, the fractional coordinates, the experimental magnetic moments, and the calculated magnetic moments. The lattice vectors are  $\vec{a}_1 = (5.21683, 0.0, 0.0)$ ,  $\vec{a}_2 = (0.0, 5.56803, 0.0)$ ,  $\vec{a}_3 = (-5.18562513, 0.0, 7.44889068)$ .

| No. | Atom | Coordinates(fractional) |          |          | Experimental magnetic moments |           |           | Calculated magnetic moments |           |           |
|-----|------|-------------------------|----------|----------|-------------------------------|-----------|-----------|-----------------------------|-----------|-----------|
| 1   | Y    | 0.270500                | 0.572900 | 0.751200 | 0.000000                      | 0.000000  | 0.000000  | 0.003000                    | 0.000000  | -0.010000 |
| 2   | Y    | 0.729500                | 0.427100 | 0.248800 | 0.000000                      | 0.000000  | 0.000000  | 0.003000                    | 0.000000  | -0.010000 |
| 3   | Y    | 0.729500                | 0.072900 | 0.748800 | 0.000000                      | 0.000000  | 0.000000  | 0.003000                    | -0.000000 | -0.010000 |
| 4   | Y    | 0.270500                | 0.927100 | 0.251200 | 0.000000                      | 0.000000  | 0.000000  | 0.003000                    | -0.000000 | -0.010000 |
| 5   | Co   | 0.500000                | 0.000000 | 0.000000 | 0.838180                      | -0.330020 | -2.779780 | 1.036000                    | -0.384000 | -3.444000 |
| 6   | Co   | 0.500000                | 0.500000 | 0.500000 | 0.838180                      | 0.330020  | -2.779780 | 1.035000                    | 0.385000  | -3.444000 |
| 7   | Mn   | 0.000000                | 0.000000 | 0.500000 | 0.838180                      | 0.330020  | -2.779780 | 1.110000                    | 0.448000  | -3.675000 |
| 8   | Mn   | 0.000000                | 0.500000 | 0.000000 | 0.838180                      | -0.330020 | -2.779780 | 1.110000                    | -0.449000 | -3.676000 |
| 9   | O    | 0.350100                | 0.815400 | 0.551500 | 0.000000                      | 0.000000  | 0.000000  | 0.010000                    | 0.001000  | -0.033000 |
| 10  | O    | 0.649900                | 0.184600 | 0.448500 | 0.000000                      | 0.000000  | 0.000000  | 0.010000                    | 0.001000  | -0.033000 |
| 11  | O    | 0.649900                | 0.315400 | 0.948500 | 0.000000                      | 0.000000  | 0.000000  | 0.010000                    | -0.001000 | -0.033000 |
| 12  | O    | 0.350100                | 0.684600 | 0.051500 | 0.000000                      | 0.000000  | 0.000000  | 0.010000                    | -0.001000 | -0.033000 |
| 13  | O    | 0.764000                | 0.792400 | 0.944300 | 0.000000                      | 0.000000  | 0.000000  | 0.018000                    | -0.005000 | -0.058000 |
| 14  | O    | 0.236000                | 0.207600 | 0.055700 | 0.000000                      | 0.000000  | 0.000000  | 0.017000                    | -0.005000 | -0.058000 |
| 15  | O    | 0.236000                | 0.292400 | 0.555700 | 0.000000                      | 0.000000  | 0.000000  | 0.018000                    | 0.006000  | -0.058000 |
| 16  | O    | 0.764000                | 0.707600 | 0.444300 | 0.000000                      | 0.000000  | 0.000000  | 0.017000                    | 0.006000  | -0.058000 |
| 17  | O    | 0.861600                | 0.466100 | 0.755700 | 0.000000                      | 0.000000  | 0.000000  | 0.019000                    | 0.004000  | -0.064000 |
| 18  | O    | 0.138400                | 0.533900 | 0.244300 | 0.000000                      | 0.000000  | 0.000000  | 0.020000                    | 0.004000  | -0.064000 |
| 19  | O    | 0.138400                | 0.966100 | 0.744300 | 0.000000                      | 0.000000  | 0.000000  | 0.019000                    | -0.004000 | -0.064000 |
| 20  | O    | 0.861600                | 0.033900 | 0.255700 | 0.000000                      | 0.000000  | 0.000000  | 0.020000                    | -0.004000 | -0.064000 |

FIG. 76. First-principles calculation results of 0.164 Y<sub>2</sub>MnCoO<sub>6</sub>. The band structure is shown in the left panel, and the Fermi-level-dependent AHC is plotted in the right panel. In both plots, the Fermi level is set to 0 eV.

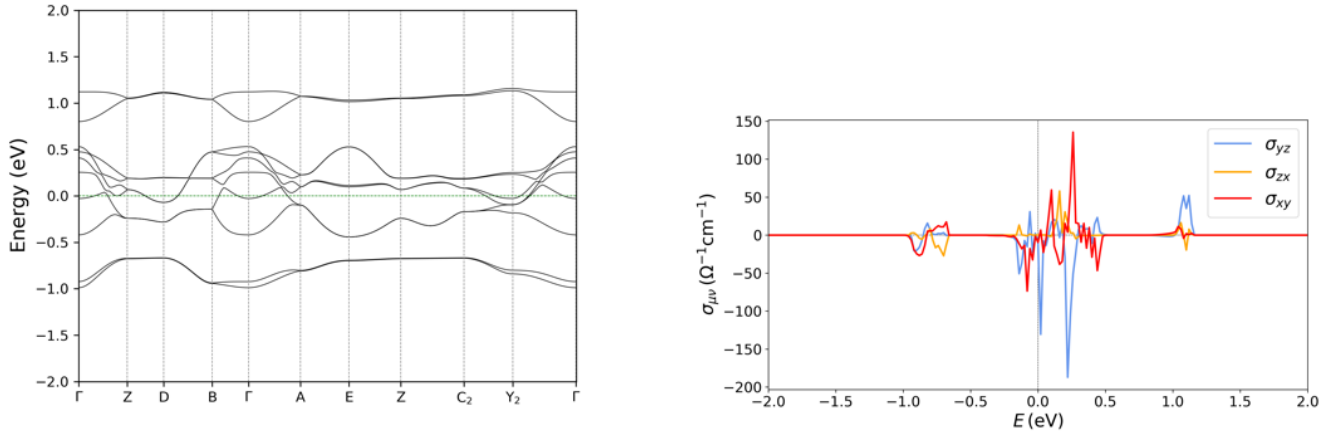

**0.306 GaFeO<sub>3</sub>** crystallizes in type III MSG 141.557, which hosts only SNLs. The symmetry-adapted AHC tensor of the MSG is  $(0, 0, \sigma_{xy})$ . Based on the first-principles calculation results, the comparison between the experimental and calculated magnetic moments is provided in Table SII79. The band structure is shown in the left panel of Fig. 77, and the Fermi-level-dependent AHC is plotted in the right panel.

TABLE SII79. The comparison between the experimental and calculated magnetic moments for 0.306 GaFeO<sub>3</sub>. The five columns contain the atom index in the structure file, the atom species, the fractional coordinates, the experimental magnetic moments, and the calculated magnetic moments. The lattice vectors are  $\vec{a}_1 = (4.34632, -2.50935, 0.0)$ ,  $\vec{a}_2 = (4.34632, 2.50935, 0.0)$ ,  $\vec{a}_3 = (-2.897546143, 0.0, 4.529296546)$ .

| No. | Atom | Coordinates(fractional) |          |          | Experimental magnetic moments |           |          | Calculated magnetic moments |           |           |
|-----|------|-------------------------|----------|----------|-------------------------------|-----------|----------|-----------------------------|-----------|-----------|
| 1   | Ga   | 0.500000                | 0.000000 | 0.500000 | 0.000000                      | 0.000000  | 0.000000 | -0.000000                   | 0.047000  | 0.001000  |
| 2   | Ga   | 0.000000                | 0.500000 | 0.000000 | 0.000000                      | 0.000000  | 0.000000 | -0.000000                   | -0.047000 | 0.001000  |
| 3   | Fe   | 0.789190                | 0.289190 | 0.367570 | 0.000000                      | -2.150010 | 0.000000 | 0.028000                    | -3.618000 | -0.040000 |
| 4   | Fe   | 0.289190                | 0.789190 | 0.867570 | 0.000000                      | 2.150010  | 0.000000 | 0.028000                    | 3.618000  | -0.040000 |
| 5   | O    | 0.694630                | 0.584770 | 0.176000 | 0.000000                      | 0.000000  | 0.000000 | 0.000000                    | -0.005000 | 0.000000  |
| 6   | O    | 0.584770                | 0.694630 | 0.676000 | 0.000000                      | 0.000000  | 0.000000 | 0.000000                    | 0.005000  | 0.000000  |
| 7   | O    | 0.396610                | 0.194630 | 0.176000 | 0.000000                      | 0.000000  | 0.000000 | 0.000000                    | -0.002000 | -0.000000 |
| 8   | O    | 0.194630                | 0.396610 | 0.676000 | 0.000000                      | 0.000000  | 0.000000 | 0.000000                    | 0.002000  | -0.000000 |

FIG. 77. First-principles calculation results of 0.306 GaFeO<sub>3</sub>. The band structure is shown in the left panel, and the Fermi-level-dependent AHC is plotted in the right panel. In both plots, the Fermi level is set to 0 eV.

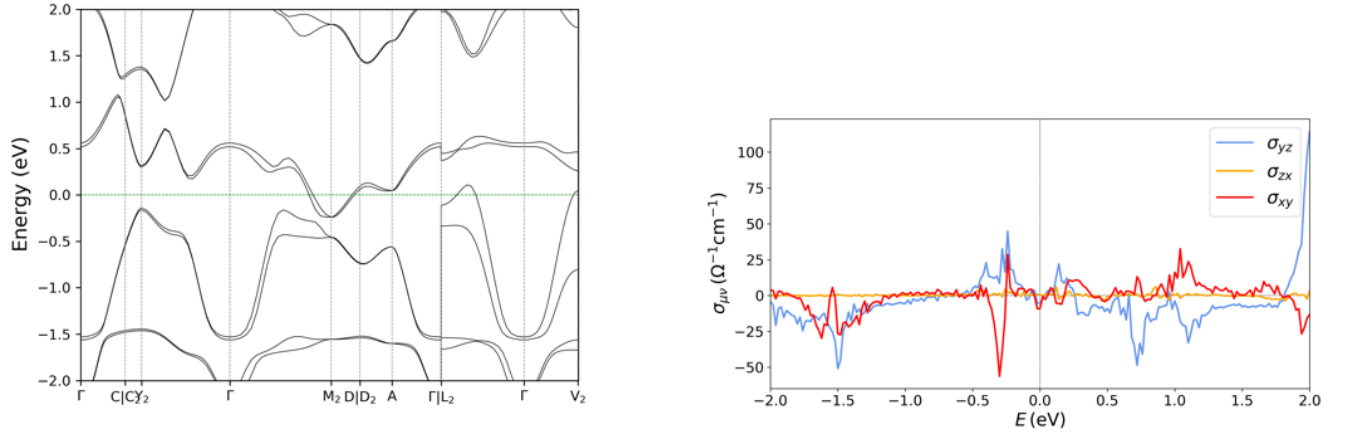

**0.314 ZrCo<sub>2</sub>Ge<sub>4</sub>O<sub>12</sub>** crystallizes in type III MSG 141.557, which hosts only SNLs. The symmetry-adapted AHC tensor of the MSG is  $(0, 0, \sigma_{xy})$ . Based on the first-principles calculation results, the comparison between the experimental and calculated magnetic moments is provided in Table SII80. The band structure is shown in the left panel of Fig. 78, and the Fermi-level-dependent AHC is plotted in the right panel.

TABLE SII80. The comparison between the experimental and calculated magnetic moments for 0.314 ZrCo<sub>2</sub>Ge<sub>4</sub>O<sub>12</sub>. The five columns contain the atom index in the structure file, the atom species, the fractional coordinates, the experimental magnetic moments, and the calculated magnetic moments. The lattice vectors are  $\vec{a}_1 = (9.5477, 0.0, 0.0)$ ,  $\vec{a}_2 = (0.0, 9.5477, 0.0)$ ,  $\vec{a}_3 = (0.0, 0.0, 4.7791)$ .

| No. | Atom | Coordinates(fractional) |          |          | Experimental magnetic moments |          |          | Calculated magnetic moments |          |           |
|-----|------|-------------------------|----------|----------|-------------------------------|----------|----------|-----------------------------|----------|-----------|
| 1   | Zr   | 0.750000                | 0.250000 | 0.500000 | 0.000000                      | 0.000000 | 0.000000 | -0.000000                   | 0.006000 | -0.000000 |
| 2   | Zr   | 0.250000                | 0.750000 | 0.500000 | 0.000000                      | 0.000000 | 0.000000 | 0.000000                    | 0.006000 | 0.000000  |
| 3   | Co   | 0.000000                | 0.000000 | 0.500000 | -2.100020                     | 1.450010 | 0.000000 | -2.134000                   | 1.473000 | 0.038000  |
| 4   | Co   | 0.500000                | 0.000000 | 0.500000 | 2.100020                      | 1.450010 | 0.000000 | 2.124000                    | 1.465000 | -0.037000 |
| 5   | Co   | 0.000000                | 0.500000 | 0.500000 | 2.100020                      | 1.450010 | 0.000000 | 2.170000                    | 1.418000 | 0.060000  |
| 6   | Co   | 0.500000                | 0.500000 | 0.500000 | -2.100020                     | 1.450010 | 0.000000 | -2.176000                   | 1.421000 | -0.060000 |
| 7   | Ge   | 0.017200                | 0.250000 | 0.000000 | 0.000000                      | 0.000000 | 0.000000 | -0.000000                   | 0.007000 | 0.001000  |
| 8   | Ge   | 0.482800                | 0.250000 | 0.000000 | 0.000000                      | 0.000000 | 0.000000 | 0.000000                    | 0.008000 | -0.000000 |
| 9   | Ge   | 0.982800                | 0.750000 | 0.000000 | 0.000000                      | 0.000000 | 0.000000 | -0.001000                   | 0.008000 | 0.001000  |
| 10  | Ge   | 0.517200                | 0.750000 | 0.000000 | 0.000000                      | 0.000000 | 0.000000 | 0.000000                    | 0.007000 | -0.001000 |
| 11  | Ge   | 0.250000                | 0.482800 | 0.000000 | 0.000000                      | 0.000000 | 0.000000 | -0.000000                   | 0.006000 | 0.000000  |
| 12  | Ge   | 0.750000                | 0.517200 | 0.000000 | 0.000000                      | 0.000000 | 0.000000 | -0.000000                   | 0.006000 | -0.000000 |
| 13  | Ge   | 0.250000                | 0.017200 | 0.000000 | 0.000000                      | 0.000000 | 0.000000 | 0.000000                    | 0.008000 | -0.000000 |
| 14  | Ge   | 0.750000                | 0.982800 | 0.000000 | 0.000000                      | 0.000000 | 0.000000 | -0.000000                   | 0.008000 | -0.000000 |
| 15  | O    | 0.127600                | 0.372400 | 0.175500 | 0.000000                      | 0.000000 | 0.000000 | 0.023000                    | 0.019000 | 0.000000  |
| 16  | O    | 0.372400                | 0.372400 | 0.824500 | 0.000000                      | 0.000000 | 0.000000 | -0.023000                   | 0.019000 | -0.001000 |
| 17  | O    | 0.872400                | 0.627600 | 0.824500 | 0.000000                      | 0.000000 | 0.000000 | 0.023000                    | 0.019000 | 0.001000  |
| 18  | O    | 0.627600                | 0.627600 | 0.175500 | 0.000000                      | 0.000000 | 0.000000 | -0.023000                   | 0.019000 | -0.001000 |
| 19  | O    | 0.127600                | 0.127600 | 0.824500 | 0.000000                      | 0.000000 | 0.000000 | -0.022000                   | 0.020000 | 0.001000  |
| 20  | O    | 0.372400                | 0.127600 | 0.175500 | 0.000000                      | 0.000000 | 0.000000 | 0.022000                    | 0.019000 | -0.001000 |
| 21  | O    | 0.872400                | 0.872400 | 0.175500 | 0.000000                      | 0.000000 | 0.000000 | -0.022000                   | 0.019000 | 0.001000  |
| 22  | O    | 0.627600                | 0.872400 | 0.824500 | 0.000000                      | 0.000000 | 0.000000 | 0.022000                    | 0.020000 | -0.001000 |
| 23  | O    | 0.663300                | 0.073000 | 0.263600 | 0.000000                      | 0.000000 | 0.000000 | 0.035000                    | 0.029000 | -0.001000 |
| 24  | O    | 0.836700                | 0.073000 | 0.736400 | 0.000000                      | 0.000000 | 0.000000 | -0.035000                   | 0.029000 | 0.001000  |
| 25  | O    | 0.336700                | 0.927000 | 0.736400 | 0.000000                      | 0.000000 | 0.000000 | 0.035000                    | 0.029000 | -0.001000 |
| 26  | O    | 0.163300                | 0.927000 | 0.263600 | 0.000000                      | 0.000000 | 0.000000 | -0.035000                   | 0.030000 | 0.001000  |
| 27  | O    | 0.663300                | 0.427000 | 0.736400 | 0.000000                      | 0.000000 | 0.000000 | -0.042000                   | 0.032000 | -0.001000 |
| 28  | O    | 0.836700                | 0.427000 | 0.263600 | 0.000000                      | 0.000000 | 0.000000 | 0.041000                    | 0.032000 | 0.001000  |
| 29  | O    | 0.336700                | 0.573000 | 0.263600 | 0.000000                      | 0.000000 | 0.000000 | -0.041000                   | 0.032000 | -0.002000 |
| 30  | O    | 0.163300                | 0.573000 | 0.736400 | 0.000000                      | 0.000000 | 0.000000 | 0.042000                    | 0.032000 | 0.002000  |
| 31  | O    | 0.927000                | 0.163300 | 0.263600 | 0.000000                      | 0.000000 | 0.000000 | -0.034000                   | 0.030000 | 0.000000  |
| 32  | O    | 0.573000                | 0.163300 | 0.736400 | 0.000000                      | 0.000000 | 0.000000 | 0.034000                    | 0.029000 | -0.000000 |
| 33  | O    | 0.073000                | 0.836700 | 0.736400 | 0.000000                      | 0.000000 | 0.000000 | -0.034000                   | 0.030000 | 0.000000  |
| 34  | O    | 0.427000                | 0.836700 | 0.263600 | 0.000000                      | 0.000000 | 0.000000 | 0.035000                    | 0.030000 | -0.000000 |
| 35  | O    | 0.927000                | 0.336700 | 0.736400 | 0.000000                      | 0.000000 | 0.000000 | 0.031000                    | 0.026000 | 0.001000  |
| 36  | O    | 0.573000                | 0.336700 | 0.263600 | 0.000000                      | 0.000000 | 0.000000 | -0.031000                   | 0.026000 | -0.000000 |
| 37  | O    | 0.073000                | 0.663300 | 0.263600 | 0.000000                      | 0.000000 | 0.000000 | 0.031000                    | 0.026000 | 0.000000  |
| 38  | O    | 0.427000                | 0.663300 | 0.736400 | 0.000000                      | 0.000000 | 0.000000 | -0.031000                   | 0.025000 | -0.001000 |

FIG. 78. First-principles calculation results of  $0.314 \text{ ZrCo}_2\text{Ge}_4\text{O}_{12}$ . The band structure is shown in the left panel, and the Fermi-level-dependent AHC is plotted in the right panel. In both plots, the Fermi level is set to 0 eV.

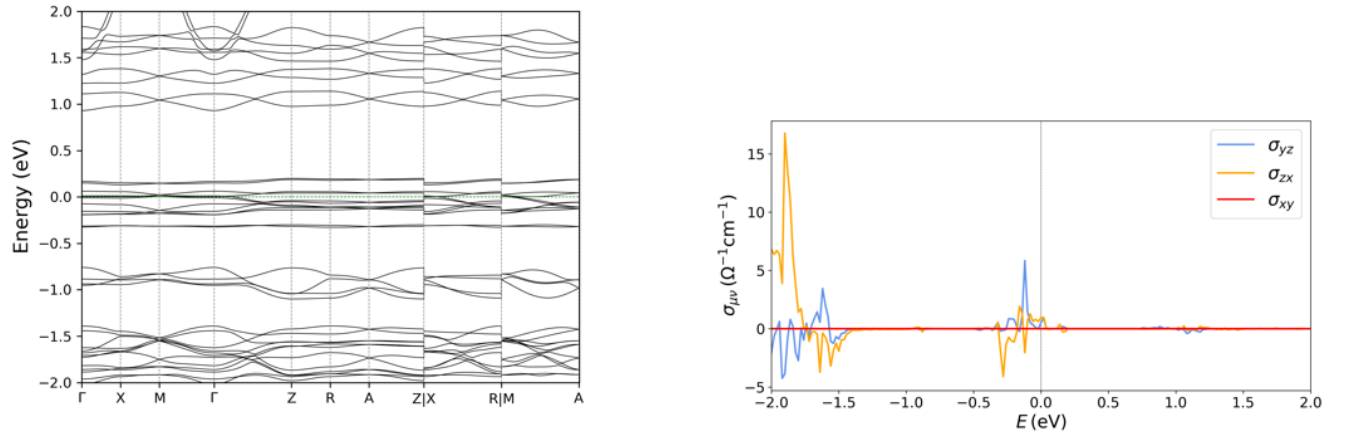



**0.318 Tm<sub>2</sub>CoMnO<sub>6</sub>** crystallizes in type III MSG 141.557, which hosts only SNLs. The symmetry-adapted AHC tensor of the MSG is  $(0, 0, \sigma_{xy})$ . Based on the first-principles calculation results, the comparison between the experimental and calculated magnetic moments is provided in Table SII81. The band structure is shown in the left panel of Fig. 79, and the Fermi-level-dependent AHC is plotted in the right panel.

TABLE SII81. The comparison between the experimental and calculated magnetic moments for 0.318 Tm<sub>2</sub>CoMnO<sub>6</sub>. The five columns contain the atom index in the structure file, the atom species, the fractional coordinates, the experimental magnetic moments, and the calculated magnetic moments. The lattice vectors are  $\vec{a}_1 = (5.18943, 0.0, 0.0)$ ,  $\vec{a}_2 = (0.0, 5.54304, 0.0)$ ,  $\vec{a}_3 = (-5.147213437, 0.0, 7.419226823)$ .

| No. | Atom | Coordinates(fractional) |          |          | Experimental magnetic moments |           |           | Calculated magnetic moments |           |           |
|-----|------|-------------------------|----------|----------|-------------------------------|-----------|-----------|-----------------------------|-----------|-----------|
| 1   | Tm   | 0.272800                | 0.573200 | 0.752000 | -1.371950                     | 0.919980  | 1.419740  | -1.346000                   | 0.900000  | 1.394000  |
| 2   | Tm   | 0.727200                | 0.426800 | 0.248000 | -1.371950                     | 0.919980  | 1.419740  | -1.346000                   | 0.900000  | 1.395000  |
| 3   | Tm   | 0.727200                | 0.073200 | 0.748000 | -1.371950                     | -0.919980 | 1.419740  | -1.341000                   | -0.900000 | 1.397000  |
| 4   | Tm   | 0.272800                | 0.926800 | 0.252000 | -1.371950                     | -0.919980 | 1.419740  | -1.341000                   | -0.900000 | 1.397000  |
| 5   | Co   | 0.000000                | 0.000000 | 0.500000 | 1.114530                      | 0.000000  | -2.599620 | 1.333000                    | 0.000000  | -3.109000 |
| 6   | Co   | 0.000000                | 0.500000 | 0.000000 | 1.114530                      | 0.000000  | -2.599620 | 1.334000                    | -0.000000 | -3.113000 |
| 7   | Mn   | 0.500000                | 0.000000 | 0.000000 | 1.114530                      | 0.000000  | -2.599620 | 1.576000                    | -0.001000 | -3.673000 |
| 8   | Mn   | 0.500000                | 0.500000 | 0.500000 | 1.114530                      | 0.000000  | -2.599620 | 1.576000                    | 0.000000  | -3.673000 |
| 9   | O    | 0.354600                | 0.817300 | 0.554100 | 0.000000                      | 0.000000  | 0.000000  | 0.082000                    | 0.009000  | -0.143000 |
| 10  | O    | 0.645400                | 0.182700 | 0.445900 | 0.000000                      | 0.000000  | 0.000000  | 0.082000                    | 0.009000  | -0.142000 |
| 11  | O    | 0.645400                | 0.317300 | 0.945900 | 0.000000                      | 0.000000  | 0.000000  | 0.083000                    | -0.010000 | -0.144000 |
| 12  | O    | 0.354600                | 0.682700 | 0.054100 | 0.000000                      | 0.000000  | 0.000000  | 0.083000                    | -0.010000 | -0.144000 |
| 13  | O    | 0.764500                | 0.793400 | 0.942300 | 0.000000                      | 0.000000  | 0.000000  | 0.067000                    | 0.007000  | -0.111000 |
| 14  | O    | 0.235500                | 0.206600 | 0.057700 | 0.000000                      | 0.000000  | 0.000000  | 0.067000                    | 0.007000  | -0.111000 |
| 15  | O    | 0.235500                | 0.293400 | 0.557700 | 0.000000                      | 0.000000  | 0.000000  | 0.069000                    | -0.007000 | -0.116000 |
| 16  | O    | 0.764500                | 0.706600 | 0.442300 | 0.000000                      | 0.000000  | 0.000000  | 0.069000                    | -0.007000 | -0.115000 |
| 17  | O    | 0.868400                | 0.462600 | 0.756100 | 0.000000                      | 0.000000  | 0.000000  | 0.039000                    | -0.002000 | -0.055000 |
| 18  | O    | 0.131600                | 0.537400 | 0.243900 | 0.000000                      | 0.000000  | 0.000000  | 0.039000                    | -0.002000 | -0.055000 |
| 19  | O    | 0.131600                | 0.962600 | 0.743900 | 0.000000                      | 0.000000  | 0.000000  | 0.039000                    | 0.002000  | -0.055000 |
| 20  | O    | 0.868400                | 0.037400 | 0.256100 | 0.000000                      | 0.000000  | 0.000000  | 0.039000                    | 0.002000  | -0.055000 |

FIG. 79. First-principles calculation results of 0.318 Tm<sub>2</sub>CoMnO<sub>6</sub>. The band structure is shown in the left panel, and the Fermi-level-dependent AHC is plotted in the right panel. In both plots, the Fermi level is set to 0 eV.

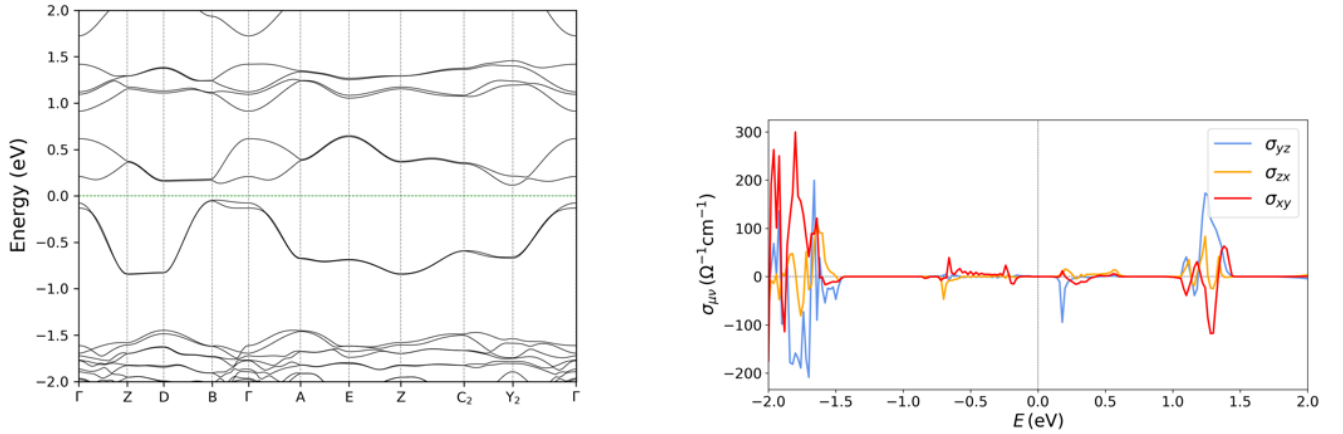

**0.327 CsMnF<sub>4</sub>** crystallizes in type III MSG 141.557, which hosts only SNLs. The symmetry-adapted AHC tensor of the MSG is  $(0, 0, \sigma_{xy})$ . Based on the first-principles calculation results, the comparison between the experimental and calculated magnetic moments is provided in Table SII82. The band structure is shown in the left panel of Fig. 80, and the Fermi-level-dependent AHC is plotted in the right panel.

TABLE SII82. The comparison between the experimental and calculated magnetic moments for 0.327 CsMnF<sub>4</sub>. The five columns contain the atom index in the structure file, the atom species, the fractional coordinates, the experimental magnetic moments, and the calculated magnetic moments. The lattice vectors are  $\vec{a}_1 = (7.944, 0.0, 0.0)$ ,  $\vec{a}_2 = (0.0, 7.944, 0.0)$ ,  $\vec{a}_3 = (0.0, 0.0, 6.3376)$ .

| No. | Atom | Coordinates(fractional) |          |          | Experimental magnetic moments |          |          | Calculated magnetic moments |           |           |
|-----|------|-------------------------|----------|----------|-------------------------------|----------|----------|-----------------------------|-----------|-----------|
| 1   | Mn   | 0.000000                | 0.000000 | 0.000000 | 3.999960                      | 0.000000 | 0.000000 | 4.307000                    | 0.000000  | 0.000000  |
| 2   | Mn   | 0.500000                | 0.000000 | 0.000000 | 3.999960                      | 0.000000 | 0.000000 | 4.307000                    | -0.000000 | -0.000000 |
| 3   | Mn   | 0.000000                | 0.500000 | 0.000000 | 3.999960                      | 0.000000 | 0.000000 | 4.307000                    | -0.000000 | 0.000000  |
| 4   | Mn   | 0.500000                | 0.500000 | 0.000000 | 3.999960                      | 0.000000 | 0.000000 | 4.307000                    | 0.000000  | -0.000000 |
| 5   | Cs   | 0.250000                | 0.250000 | 0.500000 | 0.000000                      | 0.000000 | 0.000000 | -0.001000                   | 0.000000  | -0.000000 |
| 6   | Cs   | 0.750000                | 0.750000 | 0.500000 | 0.000000                      | 0.000000 | 0.000000 | -0.001000                   | -0.000000 | -0.000000 |
| 7   | Cs   | 0.250000                | 0.750000 | 0.550600 | 0.000000                      | 0.000000 | 0.000000 | -0.004000                   | 0.000000  | -0.000000 |
| 8   | Cs   | 0.750000                | 0.250000 | 0.449400 | 0.000000                      | 0.000000 | 0.000000 | -0.004000                   | -0.000000 | -0.000000 |
| 9   | F    | 0.250000                | 0.003300 | 0.952000 | 0.000000                      | 0.000000 | 0.000000 | -0.073000                   | 0.000000  | 0.000000  |
| 10  | F    | 0.750000                | 0.996700 | 0.048000 | 0.000000                      | 0.000000 | 0.000000 | -0.073000                   | -0.000000 | -0.000000 |
| 11  | F    | 0.750000                | 0.503300 | 0.048000 | 0.000000                      | 0.000000 | 0.000000 | -0.073000                   | -0.000000 | 0.000000  |
| 12  | F    | 0.250000                | 0.496700 | 0.952000 | 0.000000                      | 0.000000 | 0.000000 | -0.073000                   | 0.000000  | -0.000000 |
| 13  | F    | 0.003300                | 0.250000 | 0.048000 | 0.000000                      | 0.000000 | 0.000000 | -0.073000                   | -0.000000 | -0.000000 |
| 14  | F    | 0.503300                | 0.750000 | 0.952000 | 0.000000                      | 0.000000 | 0.000000 | -0.073000                   | -0.000000 | 0.000000  |
| 15  | F    | 0.996700                | 0.750000 | 0.952000 | 0.000000                      | 0.000000 | 0.000000 | -0.073000                   | 0.000000  | -0.000000 |
| 16  | F    | 0.496700                | 0.250000 | 0.048000 | 0.000000                      | 0.000000 | 0.000000 | -0.073000                   | 0.000000  | 0.000000  |
| 17  | F    | 0.472400                | 0.972400 | 0.281400 | 0.000000                      | 0.000000 | 0.000000 | -0.120000                   | -0.000000 | -0.000000 |
| 18  | F    | 0.972400                | 0.027600 | 0.718600 | 0.000000                      | 0.000000 | 0.000000 | -0.120000                   | 0.000000  | 0.000000  |
| 19  | F    | 0.527600                | 0.027600 | 0.718600 | 0.000000                      | 0.000000 | 0.000000 | -0.120000                   | 0.000000  | -0.000000 |
| 20  | F    | 0.027600                | 0.972400 | 0.281400 | 0.000000                      | 0.000000 | 0.000000 | -0.120000                   | 0.000000  | 0.000000  |
| 21  | F    | 0.527600                | 0.472400 | 0.718600 | 0.000000                      | 0.000000 | 0.000000 | -0.120000                   | 0.000000  | -0.000000 |
| 22  | F    | 0.027600                | 0.527600 | 0.281400 | 0.000000                      | 0.000000 | 0.000000 | -0.120000                   | 0.000000  | 0.000000  |
| 23  | F    | 0.472400                | 0.527600 | 0.281400 | 0.000000                      | 0.000000 | 0.000000 | -0.120000                   | -0.000000 | -0.000000 |
| 24  | F    | 0.972400                | 0.472400 | 0.718600 | 0.000000                      | 0.000000 | 0.000000 | -0.120000                   | -0.000000 | 0.000000  |

FIG. 80. First-principles calculation results of 0.327 CsMnF<sub>4</sub>. The band structure is shown in the left panel, and the Fermi-level-dependent AHC is plotted in the right panel. In both plots, the Fermi level is set to 0 eV.

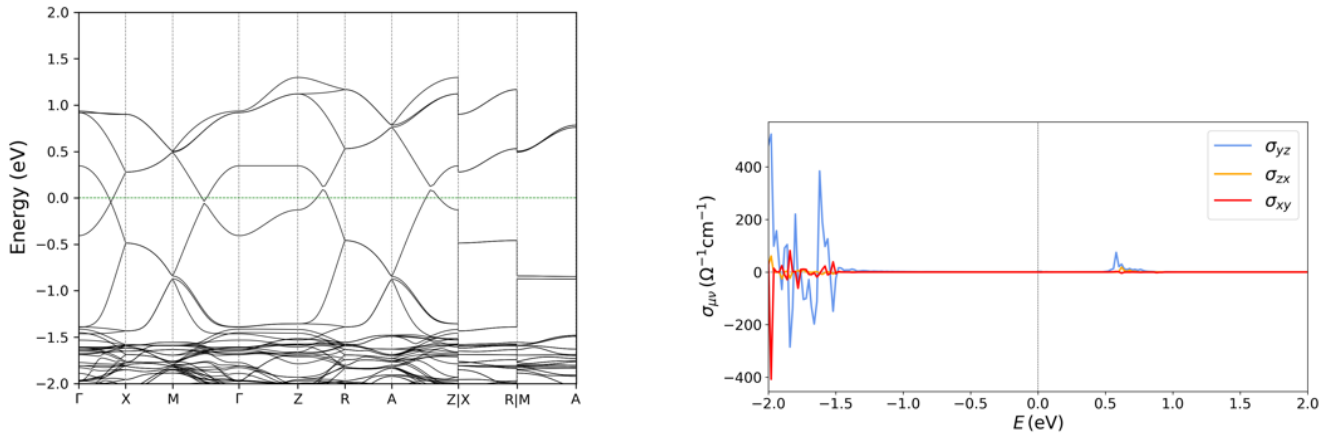

**0.371 NdMnO<sub>3</sub>** crystallizes in type III MSG 141.557, which hosts only SNLs. The symmetry-adapted AHC tensor of the MSG is  $(0, 0, \sigma_{xy})$ . Based on the first-principles calculation results, the comparison between the experimental and calculated magnetic moments is provided in Table SII83. The band structure is shown in the left panel of Fig. 81, and the Fermi-level-dependent AHC is plotted in the right panel.

TABLE SII83. The comparison between the experimental and calculated magnetic moments for 0.371 NdMnO<sub>3</sub>. The five columns contain the atom index in the structure file, the atom species, the fractional coordinates, the experimental magnetic moments, and the calculated magnetic moments. The lattice vectors are  $\vec{a}_1 = (5.7127, 0.0, 0.0)$ ,  $\vec{a}_2 = (0.0, 7.5801, 0.0)$ ,  $\vec{a}_3 = (0.0, 0.0, 5.4169)$ .

| No. | Atom | Coordinates(fractional) |          |          | Experimental magnetic moments |           |          | Calculated magnetic moments |           |           |
|-----|------|-------------------------|----------|----------|-------------------------------|-----------|----------|-----------------------------|-----------|-----------|
| 1   | Nd   | 0.560800                | 0.250000 | 0.487400 | 0.000000                      | -1.060000 | 0.000000 | 0.000000                    | -1.383000 | 0.000000  |
| 2   | Nd   | 0.439200                | 0.750000 | 0.512600 | 0.000000                      | -1.060000 | 0.000000 | 0.000000                    | -1.378000 | -0.000000 |
| 3   | Nd   | 0.060800                | 0.250000 | 0.012600 | 0.000000                      | -1.060000 | 0.000000 | -0.000000                   | -1.383000 | 0.000000  |
| 4   | Nd   | 0.939200                | 0.750000 | 0.987400 | 0.000000                      | -1.060000 | 0.000000 | -0.000000                   | -1.378000 | -0.000000 |
| 5   | Mn   | 0.000000                | 0.000000 | 0.500000 | 2.440010                      | -1.659970 | 0.000000 | 3.283000                    | -2.236000 | -0.001000 |
| 6   | Mn   | 0.000000                | 0.500000 | 0.500000 | -2.440010                     | -1.659970 | 0.000000 | -3.283000                   | -2.236000 | 0.000000  |
| 7   | Mn   | 0.500000                | 0.500000 | 0.000000 | -2.440010                     | -1.659970 | 0.000000 | -3.283000                   | -2.236000 | -0.001000 |
| 8   | Mn   | 0.500000                | 0.000000 | 0.000000 | 2.440010                      | -1.659970 | 0.000000 | 3.283000                    | -2.236000 | 0.000000  |
| 9   | O    | 0.972700                | 0.250000 | 0.586100 | 0.000000                      | 0.000000  | 0.000000 | 0.000000                    | 0.028000  | 0.002000  |
| 10  | O    | 0.027300                | 0.750000 | 0.413900 | 0.000000                      | 0.000000  | 0.000000 | 0.000000                    | 0.028000  | -0.002000 |
| 11  | O    | 0.472700                | 0.250000 | 0.913900 | 0.000000                      | 0.000000  | 0.000000 | 0.000000                    | 0.028000  | 0.002000  |
| 12  | O    | 0.527300                | 0.750000 | 0.086100 | 0.000000                      | 0.000000  | 0.000000 | 0.000000                    | 0.028000  | -0.002000 |
| 13  | O    | 0.813700                | 0.045200 | 0.209900 | 0.000000                      | 0.000000  | 0.000000 | -0.017000                   | 0.010000  | 0.000000  |
| 14  | O    | 0.186300                | 0.545200 | 0.790100 | 0.000000                      | 0.000000  | 0.000000 | 0.017000                    | 0.010000  | 0.000000  |
| 15  | O    | 0.186300                | 0.954800 | 0.790100 | 0.000000                      | 0.000000  | 0.000000 | -0.017000                   | 0.010000  | -0.000000 |
| 16  | O    | 0.813700                | 0.454800 | 0.209900 | 0.000000                      | 0.000000  | 0.000000 | 0.017000                    | 0.010000  | -0.000000 |
| 17  | O    | 0.313700                | 0.454800 | 0.290100 | 0.000000                      | 0.000000  | 0.000000 | 0.017000                    | 0.010000  | 0.000000  |
| 18  | O    | 0.686300                | 0.954800 | 0.709900 | 0.000000                      | 0.000000  | 0.000000 | -0.017000                   | 0.010000  | 0.000000  |
| 19  | O    | 0.686300                | 0.545200 | 0.709900 | 0.000000                      | 0.000000  | 0.000000 | 0.017000                    | 0.010000  | -0.000000 |
| 20  | O    | 0.313700                | 0.045200 | 0.290100 | 0.000000                      | 0.000000  | 0.000000 | -0.017000                   | 0.010000  | -0.000000 |

FIG. 81. First-principles calculation results of 0.371 NdMnO<sub>3</sub>. The band structure is shown in the left panel, and the Fermi-level-dependent AHC is plotted in the right panel. In both plots, the Fermi level is set to 0 eV.

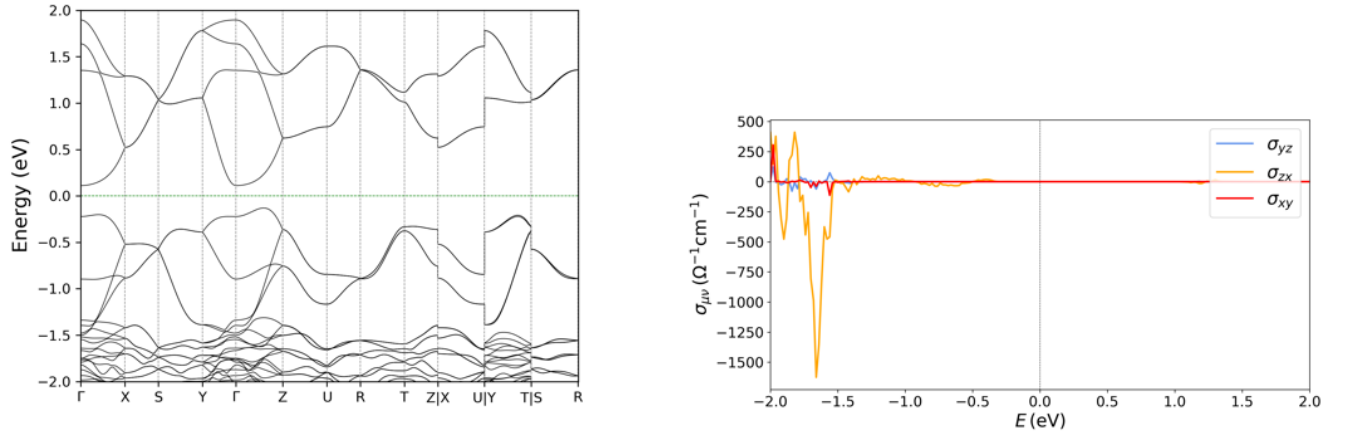

**0.515 CoFe<sub>3</sub>O<sub>5</sub>** crystallizes in type III MSG 141.557, which hosts only SNLs. The symmetry-adapted AHC tensor of the MSG is  $(0, 0, \sigma_{xy})$ . Based on the first-principles calculation results, the comparison between the experimental and calculated magnetic moments is provided in Table SII84. The band structure is shown in the left panel of Fig. 82, and the Fermi-level-dependent AHC is plotted in the right panel.

TABLE SII84. The comparison between the experimental and calculated magnetic moments for 0.515 CoFe<sub>3</sub>O<sub>5</sub>. The five columns contain the atom index in the structure file, the atom species, the fractional coordinates, the experimental magnetic moments, and the calculated magnetic moments. The lattice vectors are  $\vec{a}_1 = (2.88002, 0.0, 0.0)$ ,  $\vec{a}_2 = (0.0, 12.52485, 0.0)$ ,  $\vec{a}_3 = (-1.440010344, 0.0, 4.892335049)$ .

| No. | Atom | Coordinates(fractional) |          |          | Experimental magnetic moments |           |          | Calculated magnetic moments |           |           |
|-----|------|-------------------------|----------|----------|-------------------------------|-----------|----------|-----------------------------|-----------|-----------|
| 1   | Fe   | 0.261500                | 0.383400 | 0.523000 | -1.820000                     | -3.939940 | 0.000000 | -1.883000                   | -4.075000 | -0.000000 |
| 2   | Fe   | 0.738500                | 0.616600 | 0.477000 | -1.820000                     | -3.939940 | 0.000000 | -1.943000                   | -4.203000 | 0.000000  |
| 3   | Fe   | 0.738500                | 0.883400 | 0.477000 | -1.820000                     | 3.939940  | 0.000000 | -1.942000                   | 4.202000  | -0.000000 |
| 4   | Fe   | 0.261500                | 0.116600 | 0.523000 | -1.820000                     | 3.939940  | 0.000000 | -1.879000                   | 4.035000  | 0.000000  |
| 5   | Fe   | 0.000000                | 0.000000 | 0.000000 | 0.000000                      | -3.309940 | 0.000000 | 0.003000                    | -4.004000 | -0.000000 |
| 6   | Fe   | 0.000000                | 0.500000 | 0.000000 | 0.000000                      | 3.309940  | 0.000000 | -0.002000                   | 4.058000  | 0.000000  |
| 7   | Co   | 0.507000                | 0.250000 | 0.014000 | 2.559990                      | 0.000000  | 0.000000 | 2.760000                    | 0.002000  | -0.000000 |
| 8   | Co   | 0.493000                | 0.750000 | 0.986000 | 2.559990                      | 0.000000  | 0.000000 | 2.876000                    | 0.000000  | 0.000000  |
| 9   | Co   | 0.156300                | 0.250000 | 0.312600 | 0.000000                      | 0.000000  | 0.000000 | 0.362000                    | -0.075000 | -0.002000 |
| 10  | O    | 0.843700                | 0.750000 | 0.687400 | 0.000000                      | 0.000000  | 0.000000 | -0.005000                   | -0.001000 | 0.000000  |
| 11  | O    | 0.637400                | 0.455000 | 0.274800 | 0.000000                      | 0.000000  | 0.000000 | -0.025000                   | -0.004000 | -0.000000 |
| 12  | O    | 0.362600                | 0.545000 | 0.725200 | 0.000000                      | 0.000000  | 0.000000 | -0.036000                   | -0.031000 | -0.000000 |
| 13  | O    | 0.362600                | 0.955000 | 0.725200 | 0.000000                      | 0.000000  | 0.000000 | -0.033000                   | 0.032000  | -0.000000 |
| 14  | O    | 0.637400                | 0.045000 | 0.274800 | 0.000000                      | 0.000000  | 0.000000 | -0.036000                   | 0.021000  | 0.000000  |
| 15  | O    | 0.903300                | 0.356400 | 0.806600 | 0.000000                      | 0.000000  | 0.000000 | -0.001000                   | -0.010000 | 0.000000  |
| 16  | O    | 0.096700                | 0.643600 | 0.193400 | 0.000000                      | 0.000000  | 0.000000 | -0.008000                   | -0.048000 | 0.000000  |
| 17  | O    | 0.096700                | 0.856400 | 0.193400 | 0.000000                      | 0.000000  | 0.000000 | -0.009000                   | 0.046000  | 0.000000  |

FIG. 82. First-principles calculation results of 0.515 CoFe<sub>3</sub>O<sub>5</sub>. The band structure is shown in the left panel, and the Fermi-level-dependent AHC is plotted in the right panel. In both plots, the Fermi level is set to 0 eV.

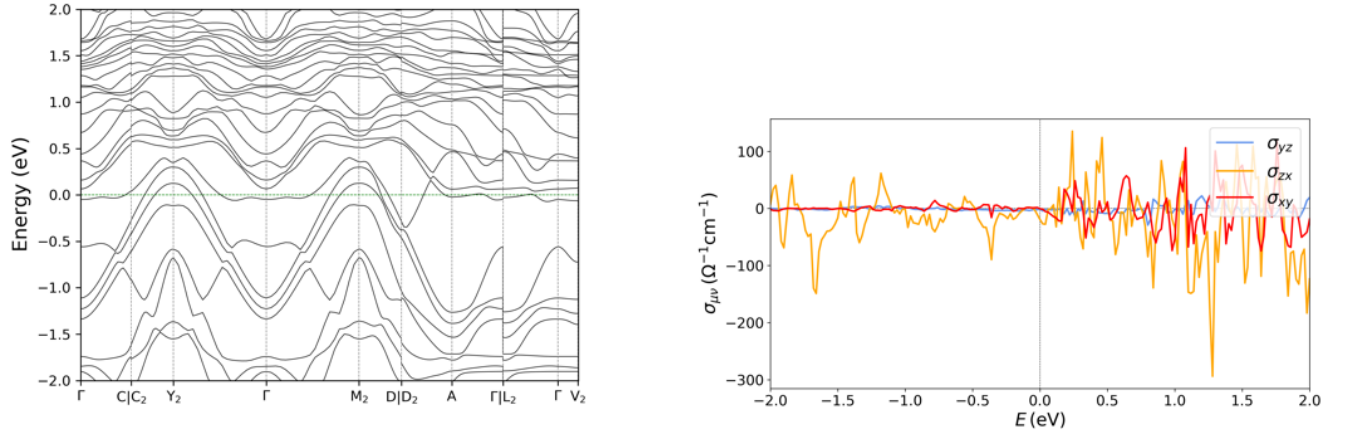

**0.7 ScMnO<sub>3</sub>** crystallizes in type III MSG 141.557, which hosts only SNLs. The symmetry-adapted AHC tensor of the MSG is  $(0, 0, \sigma_{xy})$ . Based on the first-principles calculation results, the comparison between the experimental and calculated magnetic moments is provided in Table SII85. The band structure is shown in the left panel of Fig. 83, and the Fermi-level-dependent AHC is plotted in the right panel.

TABLE SII85. The comparison between the experimental and calculated magnetic moments for 0.7 ScMnO<sub>3</sub>. The five columns contain the atom index in the structure file, the atom species, the fractional coordinates, the experimental magnetic moments, and the calculated magnetic moments. The lattice vectors are  $\vec{a}_1 = (5.83338, 0.0, 0.0)$ ,  $\vec{a}_2 = (-2.91669, 5.05185527, 0.0)$ ,  $\vec{a}_3 = (0.0, 0.0, 11.16862)$ .

| No. | Atom | Coordinates(fractional) |          |          | Experimental magnetic moments |           |          | Calculated magnetic moments |           |           |
|-----|------|-------------------------|----------|----------|-------------------------------|-----------|----------|-----------------------------|-----------|-----------|
| 1   | Sc   | 0.000000                | 0.000000 | 0.274700 | 0.000000                      | 0.000000  | 0.000000 | -0.000000                   | 0.001000  | -0.001000 |
| 2   | Sc   | 0.000000                | 0.000000 | 0.774700 | 0.000000                      | 0.000000  | 0.000000 | 0.000000                    | -0.001000 | -0.001000 |
| 3   | Sc   | 0.333333                | 0.666667 | 0.230800 | 0.000000                      | 0.000000  | 0.000000 | 0.001000                    | 0.002000  | -0.000000 |
| 4   | Sc   | 0.666667                | 0.333333 | 0.730800 | 0.000000                      | 0.000000  | 0.000000 | -0.001000                   | -0.002000 | -0.001000 |
| 5   | Sc   | 0.333333                | 0.666667 | 0.730800 | 0.000000                      | 0.000000  | 0.000000 | 0.002000                    | -0.000000 | -0.000000 |
| 6   | Sc   | 0.666667                | 0.333333 | 0.230800 | 0.000000                      | 0.000000  | 0.000000 | -0.002000                   | 0.000000  | -0.001000 |
| 7   | Mn   | 0.331600                | 0.000000 | 0.000000 | -3.029970                     | 0.000000  | 0.000000 | -3.389000                   | -0.002000 | -0.024000 |
| 8   | Mn   | 0.331600                | 0.331600 | 0.500000 | -1.514990                     | -2.624030 | 0.000000 | -1.698000                   | -2.933000 | -0.022000 |
| 9   | Mn   | 0.000000                | 0.331600 | 0.000000 | 1.514990                      | -2.624030 | 0.000000 | 1.693000                    | -2.934000 | -0.025000 |
| 10  | Mn   | 0.668400                | 0.000000 | 0.500000 | 3.029970                      | 0.000000  | 0.000000 | 3.389000                    | 0.002000  | -0.022000 |
| 11  | Mn   | 0.668400                | 0.668400 | 0.000000 | 1.514990                      | 2.624030  | 0.000000 | 1.697000                    | 2.933000  | -0.024000 |
| 12  | Mn   | 0.000000                | 0.668400 | 0.500000 | -1.514990                     | 2.624030  | 0.000000 | -1.693000                   | 2.934000  | -0.022000 |
| 13  | O    | 0.301800                | 0.000000 | 0.168000 | 0.000000                      | 0.000000  | 0.000000 | -0.012000                   | -0.001000 | -0.001000 |
| 14  | O    | 0.301800                | 0.301800 | 0.668000 | 0.000000                      | 0.000000  | 0.000000 | -0.007000                   | -0.009000 | -0.000000 |
| 15  | O    | 0.000000                | 0.301800 | 0.168000 | 0.000000                      | 0.000000  | 0.000000 | 0.006000                    | -0.010000 | 0.000000  |
| 16  | O    | 0.698200                | 0.000000 | 0.668000 | 0.000000                      | 0.000000  | 0.000000 | 0.012000                    | 0.001000  | 0.000000  |
| 17  | O    | 0.698200                | 0.698200 | 0.168000 | 0.000000                      | 0.000000  | 0.000000 | 0.007000                    | 0.009000  | -0.000000 |
| 18  | O    | 0.000000                | 0.698200 | 0.668000 | 0.000000                      | 0.000000  | 0.000000 | -0.006000                   | 0.010000  | -0.000000 |
| 19  | O    | 0.635700                | 0.000000 | 0.332900 | 0.000000                      | 0.000000  | 0.000000 | 0.020000                    | 0.001000  | -0.001000 |
| 20  | O    | 0.635700                | 0.635700 | 0.832900 | 0.000000                      | 0.000000  | 0.000000 | 0.011000                    | 0.018000  | -0.000000 |
| 21  | O    | 0.000000                | 0.635700 | 0.332900 | 0.000000                      | 0.000000  | 0.000000 | -0.008000                   | 0.015000  | 0.000000  |
| 22  | O    | 0.364300                | 0.000000 | 0.832900 | 0.000000                      | 0.000000  | 0.000000 | -0.020000                   | -0.001000 | 0.000000  |
| 23  | O    | 0.364300                | 0.364300 | 0.332900 | 0.000000                      | 0.000000  | 0.000000 | -0.011000                   | -0.018000 | -0.000000 |
| 24  | O    | 0.000000                | 0.364300 | 0.832900 | 0.000000                      | 0.000000  | 0.000000 | 0.008000                    | -0.015000 | -0.001000 |
| 25  | O    | 0.000000                | 0.000000 | 0.467800 | 0.000000                      | 0.000000  | 0.000000 | 0.002000                    | -0.004000 | -0.000000 |
| 26  | O    | 0.000000                | 0.000000 | 0.967800 | 0.000000                      | 0.000000  | 0.000000 | -0.002000                   | 0.004000  | 0.000000  |
| 27  | O    | 0.333333                | 0.666667 | 0.023800 | 0.000000                      | 0.000000  | 0.000000 | 0.005000                    | 0.000000  | 0.001000  |
| 28  | O    | 0.666667                | 0.333333 | 0.523800 | 0.000000                      | 0.000000  | 0.000000 | -0.005000                   | -0.000000 | -0.001000 |
| 29  | O    | 0.333333                | 0.666667 | 0.523800 | 0.000000                      | 0.000000  | 0.000000 | 0.003000                    | 0.003000  | 0.001000  |
| 30  | O    | 0.666667                | 0.333333 | 0.023800 | 0.000000                      | 0.000000  | 0.000000 | -0.003000                   | -0.003000 | -0.001000 |

FIG. 83. First-principles calculation results of 0.7 ScMnO<sub>3</sub>. The band structure is shown in the left panel, and the Fermi-level-dependent AHC is plotted in the right panel. In both plots, the Fermi level is set to 0 eV.

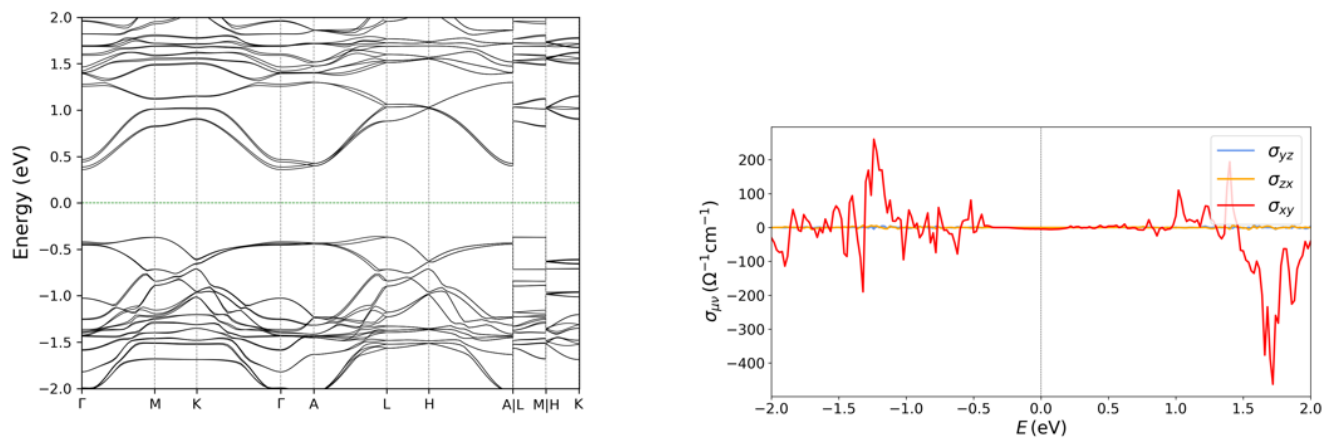

**0.709 MnNb<sub>4</sub>S<sub>8</sub>** crystallizes in type III MSG 141.557, which hosts only SNLs. The symmetry-adapted AHC tensor of the MSG is  $(0, 0, \sigma_{xy})$ . Based on the first-principles calculation results, the comparison between the experimental and calculated magnetic moments is provided in Table SII86. The band structure is shown in the left panel of Fig. 84, and the Fermi-level-dependent AHC is plotted in the right panel.

TABLE SII86. The comparison between the experimental and calculated magnetic moments for 0.709 MnNb<sub>4</sub>S<sub>8</sub>. The five columns contain the atom index in the structure file, the atom species, the fractional coordinates, the experimental magnetic moments, and the calculated magnetic moments. The lattice vectors are  $\vec{a}_1 = (3.33, -5.76773, 0.0)$ ,  $\vec{a}_2 = (3.33, 5.76773, 0.0)$ ,  $\vec{a}_3 = (0.0, 0.0, 12.44)$ .

| No. | Atom | Coordinates(fractional) |          |          | Experimental magnetic moments |          |          | Calculated magnetic moments |           |           |
|-----|------|-------------------------|----------|----------|-------------------------------|----------|----------|-----------------------------|-----------|-----------|
| 1   | Nb   | 0.000000                | 0.000000 | 0.250000 | 0.000000                      | 0.000000 | 0.000000 | -0.112000                   | 0.000000  | -0.015000 |
| 2   | Nb   | 0.000000                | 0.000000 | 0.750000 | 0.000000                      | 0.000000 | 0.000000 | -0.112000                   | 0.000000  | 0.015000  |
| 3   | Nb   | 0.494200                | 0.988400 | 0.250000 | 0.000000                      | 0.000000 | 0.000000 | -0.072000                   | -0.000000 | -0.012000 |
| 4   | Nb   | 0.988400                | 0.494200 | 0.750000 | 0.000000                      | 0.000000 | 0.000000 | -0.075000                   | -0.000000 | 0.011000  |
| 5   | Nb   | 0.505800                | 0.011600 | 0.750000 | 0.000000                      | 0.000000 | 0.000000 | -0.072000                   | 0.000000  | 0.012000  |
| 6   | Nb   | 0.011600                | 0.505800 | 0.250000 | 0.000000                      | 0.000000 | 0.000000 | -0.075000                   | 0.000000  | -0.011000 |
| 7   | Nb   | 0.494200                | 0.505800 | 0.250000 | 0.000000                      | 0.000000 | 0.000000 | -0.073000                   | 0.000000  | -0.011000 |
| 8   | Nb   | 0.505800                | 0.494200 | 0.750000 | 0.000000                      | 0.000000 | 0.000000 | -0.073000                   | 0.000000  | 0.011000  |
| 9   | Mn   | 0.000000                | 0.000000 | 0.000000 | 3.400000                      | 0.000000 | 0.000000 | 4.355000                    | 0.000000  | -0.000000 |
| 10  | Mn   | 0.000000                | 0.000000 | 0.500000 | 3.400000                      | 0.000000 | 0.000000 | 4.355000                    | -0.000000 | 0.000000  |
| 11  | S    | 0.666667                | 0.333333 | 0.615400 | 0.000000                      | 0.000000 | 0.000000 | 0.002000                    | -0.000000 | 0.002000  |
| 12  | S    | 0.333333                | 0.666667 | 0.384600 | 0.000000                      | 0.000000 | 0.000000 | 0.002000                    | -0.000000 | -0.002000 |
| 13  | S    | 0.666667                | 0.333333 | 0.884600 | 0.000000                      | 0.000000 | 0.000000 | 0.002000                    | 0.000000  | 0.002000  |
| 14  | S    | 0.333333                | 0.666667 | 0.115400 | 0.000000                      | 0.000000 | 0.000000 | 0.002000                    | -0.000000 | -0.002000 |
| 15  | S    | 0.672200                | 0.836100 | 0.871300 | 0.000000                      | 0.000000 | 0.000000 | 0.002000                    | 0.000000  | 0.001000  |
| 16  | S    | 0.836100                | 0.672200 | 0.128700 | 0.000000                      | 0.000000 | 0.000000 | 0.008000                    | -0.000000 | -0.001000 |
| 17  | S    | 0.327800                | 0.163900 | 0.128700 | 0.000000                      | 0.000000 | 0.000000 | 0.002000                    | -0.000000 | -0.001000 |
| 18  | S    | 0.163900                | 0.327800 | 0.871300 | 0.000000                      | 0.000000 | 0.000000 | 0.007000                    | -0.000000 | 0.001000  |
| 19  | S    | 0.163900                | 0.327800 | 0.628700 | 0.000000                      | 0.000000 | 0.000000 | 0.008000                    | -0.000000 | 0.001000  |
| 20  | S    | 0.327800                | 0.163900 | 0.371300 | 0.000000                      | 0.000000 | 0.000000 | 0.002000                    | -0.000000 | -0.001000 |
| 21  | S    | 0.836100                | 0.672200 | 0.371300 | 0.000000                      | 0.000000 | 0.000000 | 0.007000                    | 0.000000  | -0.001000 |
| 22  | S    | 0.672200                | 0.836100 | 0.628700 | 0.000000                      | 0.000000 | 0.000000 | 0.002000                    | -0.000000 | 0.001000  |
| 23  | S    | 0.163900                | 0.836100 | 0.871300 | 0.000000                      | 0.000000 | 0.000000 | 0.005000                    | 0.000000  | 0.001000  |
| 24  | S    | 0.836100                | 0.163900 | 0.128700 | 0.000000                      | 0.000000 | 0.000000 | 0.005000                    | 0.000000  | -0.001000 |
| 25  | S    | 0.163900                | 0.836100 | 0.628700 | 0.000000                      | 0.000000 | 0.000000 | 0.005000                    | 0.000000  | 0.001000  |
| 26  | S    | 0.836100                | 0.163900 | 0.371300 | 0.000000                      | 0.000000 | 0.000000 | 0.005000                    | 0.000000  | -0.001000 |

FIG. 84. First-principles calculation results of 0.709 MnNb<sub>4</sub>S<sub>8</sub>. The band structure is shown in the left panel, and the Fermi-level-dependent AHC is plotted in the right panel. In both plots, the Fermi level is set to 0 eV.

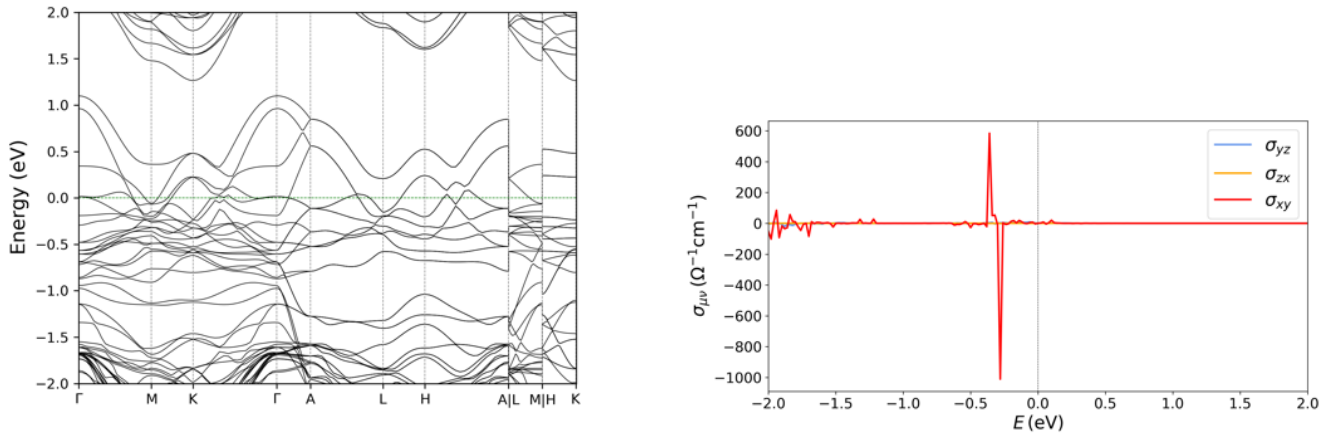



**0.711 MnTa<sub>4</sub>S<sub>8</sub>** crystallizes in type III MSG 141.557, which hosts only SNLs. The symmetry-adapted AHC tensor of the MSG is  $(0, 0, \sigma_{xy})$ . Based on the first-principles calculation results, the comparison between the experimental and calculated magnetic moments is provided in Table SII87. The band structure is shown in the left panel of Fig. 85, and the Fermi-level-dependent AHC is plotted in the right panel.

TABLE SII87. The comparison between the experimental and calculated magnetic moments for 0.711 MnTa<sub>4</sub>S<sub>8</sub>. The five columns contain the atom index in the structure file, the atom species, the fractional coordinates, the experimental magnetic moments, and the calculated magnetic moments. The lattice vectors are  $\vec{a}_1 = (3.32, -5.75041, 0.0)$ ,  $\vec{a}_2 = (3.32, 5.75041, 0.0)$ ,  $\vec{a}_3 = (0.0, 0.0, 12.51)$ .

| No. | Atom | Coordinates(fractional) |          |          | Experimental magnetic moments |          |          | Calculated magnetic moments |           |           |
|-----|------|-------------------------|----------|----------|-------------------------------|----------|----------|-----------------------------|-----------|-----------|
| 1   | Ta   | 0.000000                | 0.000000 | 0.250000 | 0.000000                      | 0.000000 | 0.000000 | -0.075000                   | 0.000000  | -0.031000 |
| 2   | Ta   | 0.000000                | 0.000000 | 0.750000 | 0.000000                      | 0.000000 | 0.000000 | -0.075000                   | 0.000000  | 0.031000  |
| 3   | Ta   | 0.492100                | 0.984200 | 0.250000 | 0.000000                      | 0.000000 | 0.000000 | -0.035000                   | 0.000000  | -0.022000 |
| 4   | Ta   | 0.984200                | 0.492100 | 0.750000 | 0.000000                      | 0.000000 | 0.000000 | -0.030000                   | -0.000000 | 0.017000  |
| 5   | Ta   | 0.507900                | 0.015800 | 0.750000 | 0.000000                      | 0.000000 | 0.000000 | -0.035000                   | 0.001000  | 0.021000  |
| 6   | Ta   | 0.015800                | 0.507900 | 0.250000 | 0.000000                      | 0.000000 | 0.000000 | -0.029000                   | 0.001000  | -0.018000 |
| 7   | Ta   | 0.492100                | 0.507900 | 0.250000 | 0.000000                      | 0.000000 | 0.000000 | -0.033000                   | -0.000000 | -0.020000 |
| 8   | Ta   | 0.507900                | 0.492100 | 0.750000 | 0.000000                      | 0.000000 | 0.000000 | -0.032000                   | -0.000000 | 0.020000  |
| 9   | Mn   | 0.000000                | 0.000000 | 0.000000 | 4.200000                      | 0.000000 | 0.000000 | 3.849000                    | 0.000000  | -0.000000 |
| 10  | Mn   | 0.000000                | 0.000000 | 0.500000 | 4.200000                      | 0.000000 | 0.000000 | 3.849000                    | -0.000000 | 0.000000  |
| 11  | S    | 0.666667                | 0.333333 | 0.622100 | 0.000000                      | 0.000000 | 0.000000 | 0.004000                    | -0.000000 | 0.003000  |
| 12  | S    | 0.333333                | 0.666667 | 0.377900 | 0.000000                      | 0.000000 | 0.000000 | 0.004000                    | 0.000000  | -0.004000 |
| 13  | S    | 0.666667                | 0.333333 | 0.877900 | 0.000000                      | 0.000000 | 0.000000 | 0.004000                    | 0.000000  | 0.004000  |
| 14  | S    | 0.333333                | 0.666667 | 0.122100 | 0.000000                      | 0.000000 | 0.000000 | 0.004000                    | 0.000000  | -0.003000 |
| 15  | S    | 0.663800                | 0.831900 | 0.875300 | 0.000000                      | 0.000000 | 0.000000 | 0.015000                    | -0.000000 | 0.002000  |
| 16  | S    | 0.831900                | 0.663800 | 0.124700 | 0.000000                      | 0.000000 | 0.000000 | 0.021000                    | -0.000000 | -0.002000 |
| 17  | S    | 0.336200                | 0.168100 | 0.124700 | 0.000000                      | 0.000000 | 0.000000 | 0.014000                    | -0.000000 | -0.001000 |
| 18  | S    | 0.168100                | 0.336200 | 0.875300 | 0.000000                      | 0.000000 | 0.000000 | 0.021000                    | -0.000000 | 0.001000  |
| 19  | S    | 0.168100                | 0.336200 | 0.624700 | 0.000000                      | 0.000000 | 0.000000 | 0.021000                    | -0.000000 | 0.002000  |
| 20  | S    | 0.336200                | 0.168100 | 0.375300 | 0.000000                      | 0.000000 | 0.000000 | 0.015000                    | -0.000000 | -0.002000 |
| 21  | S    | 0.831900                | 0.663800 | 0.375300 | 0.000000                      | 0.000000 | 0.000000 | 0.021000                    | 0.000000  | -0.001000 |
| 22  | S    | 0.663800                | 0.831900 | 0.624700 | 0.000000                      | 0.000000 | 0.000000 | 0.014000                    | 0.000000  | 0.001000  |
| 23  | S    | 0.168100                | 0.831900 | 0.875300 | 0.000000                      | 0.000000 | 0.000000 | 0.017000                    | 0.001000  | 0.001000  |
| 24  | S    | 0.831900                | 0.168100 | 0.124700 | 0.000000                      | 0.000000 | 0.000000 | 0.018000                    | -0.000000 | -0.002000 |
| 25  | S    | 0.168100                | 0.831900 | 0.624700 | 0.000000                      | 0.000000 | 0.000000 | 0.018000                    | -0.000000 | 0.002000  |
| 26  | S    | 0.831900                | 0.168100 | 0.375300 | 0.000000                      | 0.000000 | 0.000000 | 0.018000                    | 0.001000  | -0.001000 |

FIG. 85. First-principles calculation results of 0.711 MnTa<sub>4</sub>S<sub>8</sub>. The band structure is shown in the left panel, and the Fermi-level-dependent AHC is plotted in the right panel. In both plots, the Fermi level is set to 0 eV.

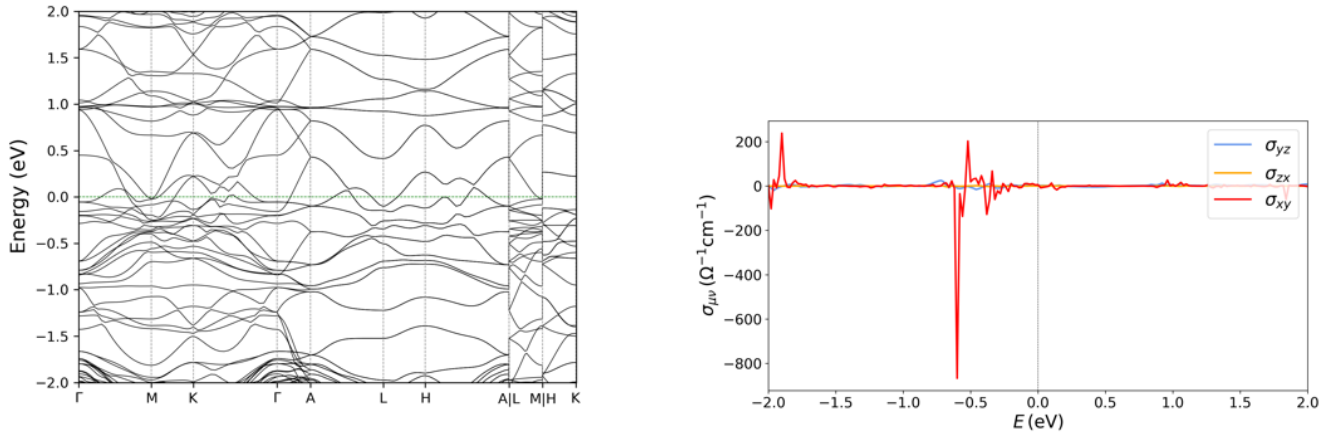

**0.739 YBaMn<sub>2</sub>O<sub>5</sub>** crystallizes in type III MSG 141.557, which hosts only SNLs. The symmetry-adapted AHC tensor of the MSG is  $(0, 0, \sigma_{xy})$ . Based on the first-principles calculation results, the comparison between the experimental and calculated magnetic moments is provided in Table SII88. The band structure is shown in the left panel of Fig. 86, and the Fermi-level-dependent AHC is plotted in the right panel.

TABLE SII88. The comparison between the experimental and calculated magnetic moments for 0.739 YBaMn<sub>2</sub>O<sub>5</sub>. The five columns contain the atom index in the structure file, the atom species, the fractional coordinates, the experimental magnetic moments, and the calculated magnetic moments. The lattice vectors are  $\vec{a}_1 = (5.5359, 0.0, 0.0)$ ,  $\vec{a}_2 = (0.0, 5.5359, 0.0)$ ,  $\vec{a}_3 = (0.0, 0.0, 7.6151)$ .

| No. | Atom | Coordinates(fractional) |          |          | Experimental magnetic moments |          |           | Calculated magnetic moments |           |           |
|-----|------|-------------------------|----------|----------|-------------------------------|----------|-----------|-----------------------------|-----------|-----------|
| 1   | Y    | 0.750000                | 0.250000 | 0.500000 | 0.000000                      | 0.000000 | 0.000000  | 0.000000                    | 0.000000  | 0.014000  |
| 2   | Y    | 0.250000                | 0.750000 | 0.500000 | 0.000000                      | 0.000000 | 0.000000  | -0.000000                   | -0.000000 | 0.014000  |
| 3   | Ba   | 0.750000                | 0.250000 | 0.000000 | 0.000000                      | 0.000000 | 0.000000  | 0.000000                    | 0.000000  | -0.004000 |
| 4   | Ba   | 0.250000                | 0.750000 | 0.000000 | 0.000000                      | 0.000000 | 0.000000  | -0.000000                   | -0.000000 | -0.004000 |
| 5   | Mn   | 0.250000                | 0.250000 | 0.720600 | 0.000000                      | 0.000000 | 2.899980  | 0.000000                    | -0.001000 | 3.127000  |
| 6   | Mn   | 0.750000                | 0.750000 | 0.279400 | 0.000000                      | 0.000000 | 2.899980  | -0.000000                   | 0.001000  | 3.127000  |
| 7   | Mn   | 0.250000                | 0.250000 | 0.251400 | 0.000000                      | 0.000000 | -3.900000 | -0.000000                   | 0.000000  | -4.043000 |
| 8   | Mn   | 0.750000                | 0.750000 | 0.748600 | 0.000000                      | 0.000000 | -3.900000 | 0.000000                    | -0.000000 | -4.043000 |
| 9   | O    | 0.991100                | 0.991100 | 0.316400 | 0.000000                      | 0.000000 | 0.000000  | 0.000000                    | 0.000000  | -0.007000 |
| 10  | O    | 0.508900                | 0.508900 | 0.316400 | 0.000000                      | 0.000000 | 0.000000  | -0.001000                   | 0.000000  | -0.007000 |
| 11  | O    | 0.508900                | 0.991100 | 0.316400 | 0.000000                      | 0.000000 | 0.000000  | -0.001000                   | -0.000000 | -0.008000 |
| 12  | O    | 0.991100                | 0.508900 | 0.316400 | 0.000000                      | 0.000000 | 0.000000  | 0.000000                    | 0.000000  | -0.008000 |
| 13  | O    | 0.008900                | 0.008900 | 0.683600 | 0.000000                      | 0.000000 | 0.000000  | 0.001000                    | -0.000000 | -0.007000 |
| 14  | O    | 0.491100                | 0.491100 | 0.683600 | 0.000000                      | 0.000000 | 0.000000  | -0.000000                   | -0.000000 | -0.007000 |
| 15  | O    | 0.491100                | 0.008900 | 0.683600 | 0.000000                      | 0.000000 | 0.000000  | -0.000000                   | -0.000000 | -0.008000 |
| 16  | O    | 0.008900                | 0.491100 | 0.683600 | 0.000000                      | 0.000000 | 0.000000  | 0.001000                    | 0.000000  | -0.008000 |
| 17  | O    | 0.250000                | 0.250000 | 0.993900 | 0.000000                      | 0.000000 | 0.000000  | 0.000000                    | -0.000000 | 0.003000  |
| 18  | O    | 0.750000                | 0.750000 | 0.006100 | 0.000000                      | 0.000000 | 0.000000  | -0.000000                   | 0.000000  | 0.003000  |

FIG. 86. First-principles calculation results of 0.739 YBaMn<sub>2</sub>O<sub>5</sub>. The band structure is shown in the left panel, and the Fermi-level-dependent AHC is plotted in the right panel. In both plots, the Fermi level is set to 0 eV.

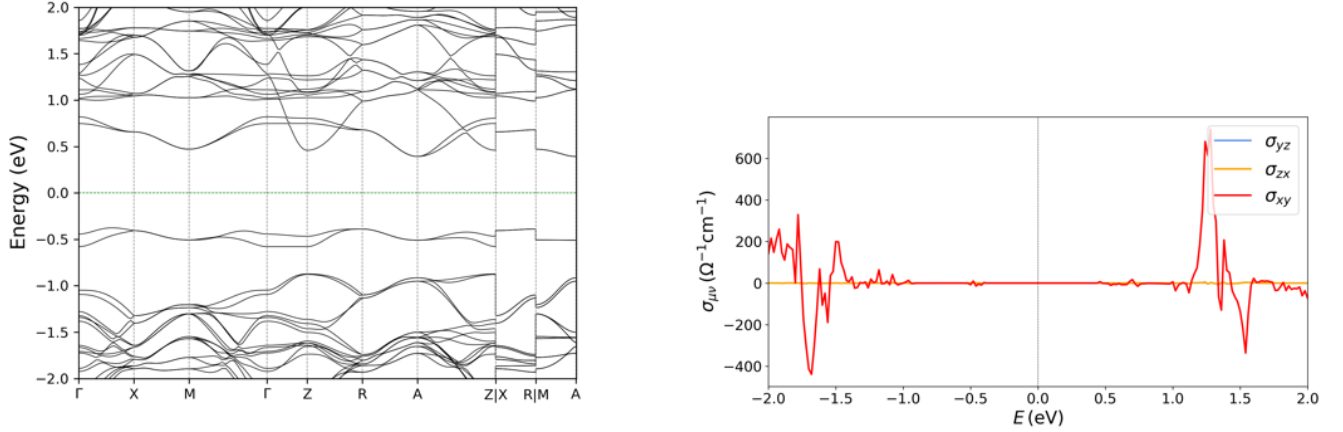

**0.776 CeMnSi<sub>2</sub>** crystallizes in type III MSG 141.557, which hosts only SNLs. The symmetry-adapted AHC tensor of the MSG is  $(0, 0, \sigma_{xy})$ . Based on the first-principles calculation results, the comparison between the experimental and calculated magnetic moments is provided in Table SII89. The band structure is shown in the left panel of Fig. 87, and the Fermi-level-dependent AHC is plotted in the right panel.

TABLE SII89. The comparison between the experimental and calculated magnetic moments for 0.776 CeMnSi<sub>2</sub>. The five columns contain the atom index in the structure file, the atom species, the fractional coordinates, the experimental magnetic moments, and the calculated magnetic moments. The lattice vectors are  $\vec{a}_1 = (2.0615, -8.775, 0.0)$ ,  $\vec{a}_2 = (2.0615, 8.775, 0.0)$ ,  $\vec{a}_3 = (0.0, 0.0, 4.035)$ .

| No. | Atom | Coordinates(fractional) |          |          |          | Experimental magnetic moments |          |           | Calculated magnetic moments |           |  |
|-----|------|-------------------------|----------|----------|----------|-------------------------------|----------|-----------|-----------------------------|-----------|--|
| 1   | Ce   | 0.899000                | 0.101000 | 0.250000 | 0.000000 | -0.230080                     | 0.000000 | 0.009000  | -0.319000                   | 0.002000  |  |
| 2   | Ce   | 0.101000                | 0.899000 | 0.750000 | 0.000000 | -0.230080                     | 0.000000 | -0.001000 | -0.319000                   | 0.002000  |  |
| 3   | Mn   | 0.249000                | 0.751000 | 0.250000 | 0.000000 | 2.240080                      | 0.000000 | -0.000000 | 3.563000                    | 0.000000  |  |
| 4   | Mn   | 0.751000                | 0.249000 | 0.750000 | 0.000000 | 2.240080                      | 0.000000 | -0.000000 | 3.564000                    | -0.000000 |  |
| 5   | Si   | 0.675000                | 0.325000 | 0.250000 | 0.000000 | 0.000000                      | 0.000000 | 0.000000  | -0.101000                   | 0.000000  |  |
| 6   | Si   | 0.325000                | 0.675000 | 0.750000 | 0.000000 | 0.000000                      | 0.000000 | 0.000000  | -0.101000                   | 0.000000  |  |
| 7   | Si   | 0.535000                | 0.465000 | 0.250000 | 0.000000 | 0.000000                      | 0.000000 | -0.002000 | -0.013000                   | 0.000000  |  |
| 8   | Si   | 0.465000                | 0.535000 | 0.750000 | 0.000000 | 0.000000                      | 0.000000 | 0.002000  | -0.013000                   | 0.001000  |  |

FIG. 87. First-principles calculation results of 0.776 CeMnSi<sub>2</sub>. The band structure is shown in the left panel, and the Fermi-level-dependent AHC is plotted in the right panel. In both plots, the Fermi level is set to 0 eV.

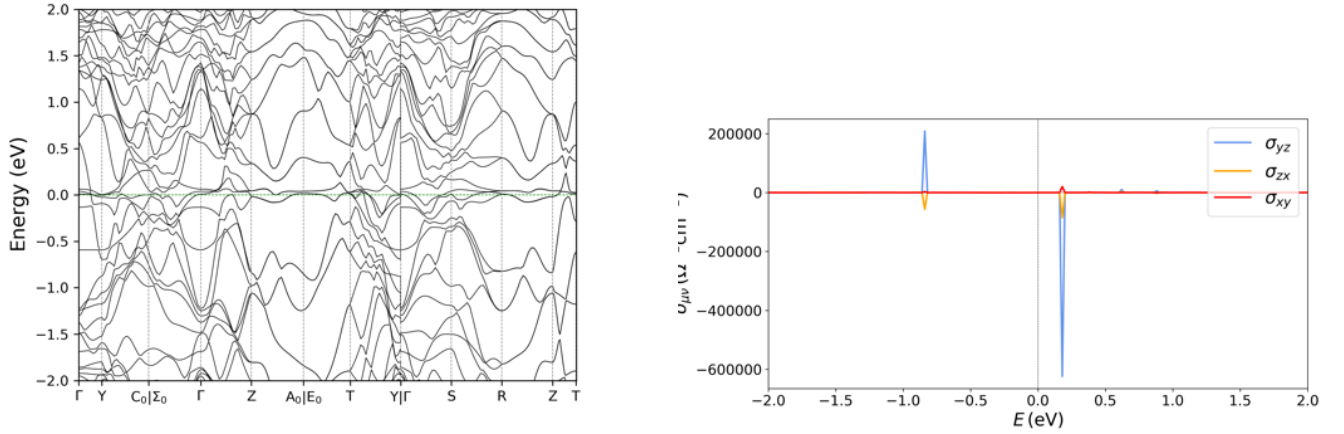

**0.787 YVO<sub>3</sub>** crystallizes in type III MSG 141.557, which hosts only SNLs. The symmetry-adapted AHC tensor of the MSG is  $(0, 0, \sigma_{xy})$ . Based on the first-principles calculation results, the comparison between the experimental and calculated magnetic moments is provided in Table SII90. The band structure is shown in the left panel of Fig. 88, and the Fermi-level-dependent AHC is plotted in the right panel.

TABLE SII90. The comparison between the experimental and calculated magnetic moments for 0.787 YVO<sub>3</sub>. The five columns contain the atom index in the structure file, the atom species, the fractional coordinates, the experimental magnetic moments, and the calculated magnetic moments. The lattice vectors are  $\vec{a}_1 = (5.5926, 0.0, 0.0)$ ,  $\vec{a}_2 = (0.0, 7.5561, 0.0)$ ,  $\vec{a}_3 = (0.0, 0.0, 5.2855)$ .

| No. | Atom | Coordinates(fractional) |          |          | Experimental magnetic moments |           |          | Calculated magnetic moments |           |           |
|-----|------|-------------------------|----------|----------|-------------------------------|-----------|----------|-----------------------------|-----------|-----------|
| 1   | Y    | 0.428500                | 0.250000 | 0.478300 | 0.000000                      | 0.000000  | 0.000000 | -0.000000                   | 0.000000  | 0.001000  |
| 2   | Y    | 0.071500                | 0.750000 | 0.978300 | 0.000000                      | 0.000000  | 0.000000 | 0.000000                    | 0.001000  | 0.001000  |
| 3   | Y    | 0.571500                | 0.750000 | 0.521700 | 0.000000                      | 0.000000  | 0.000000 | -0.000000                   | 0.001000  | 0.001000  |
| 4   | Y    | 0.928500                | 0.250000 | 0.021700 | 0.000000                      | 0.000000  | 0.000000 | 0.000000                    | 0.000000  | 0.001000  |
| 5   | V    | 0.000000                | 0.000000 | 0.500000 | 0.000000                      | -1.720000 | 0.000000 | 0.041000                    | -1.538000 | 0.036000  |
| 6   | V    | 0.500000                | 0.000000 | 0.000000 | 0.000000                      | 1.720000  | 0.000000 | -0.042000                   | 1.568000  | 0.037000  |
| 7   | V    | 0.500000                | 0.500000 | 0.000000 | 0.000000                      | -1.720000 | 0.000000 | -0.041000                   | -1.559000 | 0.040000  |
| 8   | V    | 0.000000                | 0.500000 | 0.500000 | 0.000000                      | 1.720000  | 0.000000 | 0.041000                    | 1.547000  | 0.039000  |
| 9   | O    | 0.037800                | 0.250000 | 0.612600 | 0.000000                      | 0.000000  | 0.000000 | -0.000000                   | 0.001000  | 0.000000  |
| 10  | O    | 0.462200                | 0.750000 | 0.112600 | 0.000000                      | 0.000000  | 0.000000 | -0.000000                   | 0.000000  | 0.000000  |
| 11  | O    | 0.962200                | 0.750000 | 0.387400 | 0.000000                      | 0.000000  | 0.000000 | -0.000000                   | 0.000000  | 0.000000  |
| 12  | O    | 0.537800                | 0.250000 | 0.887400 | 0.000000                      | 0.000000  | 0.000000 | 0.000000                    | 0.001000  | 0.000000  |
| 13  | O    | 0.299600                | 0.556630 | 0.687200 | 0.000000                      | 0.000000  | 0.000000 | -0.000000                   | -0.009000 | 0.000000  |
| 14  | O    | 0.200400                | 0.443370 | 0.187200 | 0.000000                      | 0.000000  | 0.000000 | -0.000000                   | 0.007000  | 0.000000  |
| 15  | O    | 0.700400                | 0.443370 | 0.312800 | 0.000000                      | 0.000000  | 0.000000 | 0.000000                    | -0.009000 | 0.000000  |
| 16  | O    | 0.799600                | 0.556630 | 0.812800 | 0.000000                      | 0.000000  | 0.000000 | 0.000000                    | 0.007000  | -0.000000 |
| 17  | O    | 0.799600                | 0.943370 | 0.812800 | 0.000000                      | 0.000000  | 0.000000 | -0.000000                   | -0.008000 | 0.000000  |
| 18  | O    | 0.700400                | 0.056630 | 0.312800 | 0.000000                      | 0.000000  | 0.000000 | 0.000000                    | 0.008000  | 0.000000  |
| 19  | O    | 0.200400                | 0.056630 | 0.187200 | 0.000000                      | 0.000000  | 0.000000 | -0.000000                   | -0.007000 | 0.000000  |
| 20  | O    | 0.299600                | 0.943370 | 0.687200 | 0.000000                      | 0.000000  | 0.000000 | 0.000000                    | 0.008000  | 0.000000  |

FIG. 88. First-principles calculation results of 0.787 YVO<sub>3</sub>. The band structure is shown in the left panel, and the Fermi-level-dependent AHC is plotted in the right panel. In both plots, the Fermi level is set to 0 eV.

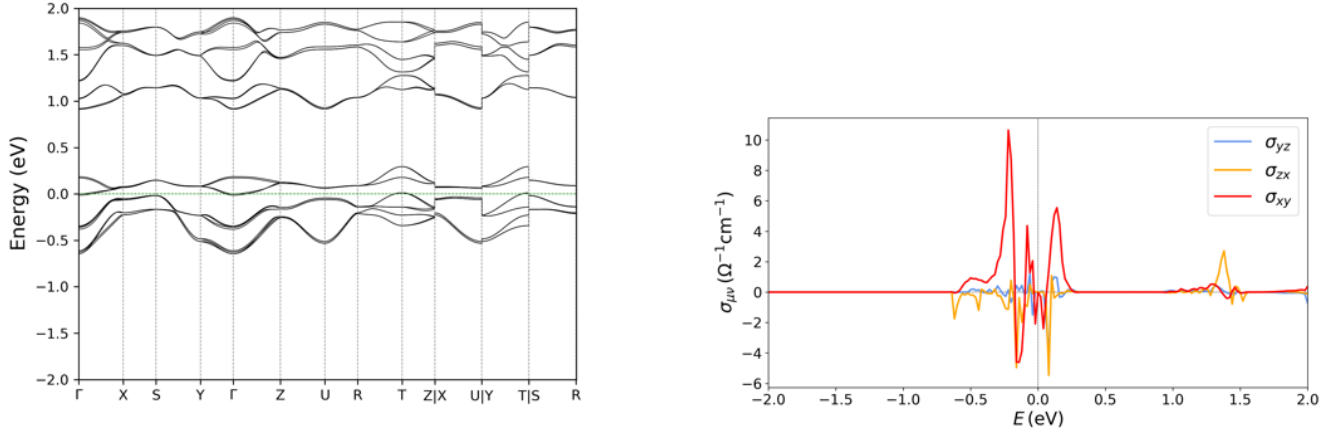

**0.825 Ca<sub>2</sub>MnGaO<sub>5</sub>** crystallizes in type III MSG 141.557, which hosts only SNLs. The symmetry-adapted AHC tensor of the MSG is  $(0, 0, \sigma_{xy})$ . Based on the first-principles calculation results, the comparison between the experimental and calculated magnetic moments is provided in Table SII91. The band structure is shown in the left panel of Fig. 89, and the Fermi-level-dependent AHC is plotted in the right panel.

TABLE SII91. The comparison between the experimental and calculated magnetic moments for 0.825 Ca<sub>2</sub>MnGaO<sub>5</sub>. The five columns contain the atom index in the structure file, the atom species, the fractional coordinates, the experimental magnetic moments, and the calculated magnetic moments. The lattice vectors are  $\vec{a}_1 = (5.2677, 0.0, 0.0)$ ,  $\vec{a}_2 = (0.0, 15.2928, 0.0)$ ,  $\vec{a}_3 = (0.0, 0.0, 5.4679)$ .

| No. | Atom | Coordinates(fractional) |          |          | Experimental magnetic moments |           |          | Calculated magnetic moments |           |           |
|-----|------|-------------------------|----------|----------|-------------------------------|-----------|----------|-----------------------------|-----------|-----------|
| 1   | Ca   | 0.990300                | 0.109500 | 0.023600 | 0.000000                      | 0.000000  | 0.000000 | 0.000000                    | 0.003000  | 0.000000  |
| 2   | Ca   | 0.490300                | 0.390500 | 0.476400 | 0.000000                      | 0.000000  | 0.000000 | 0.000000                    | -0.003000 | -0.000000 |
| 3   | Ca   | 0.009700                | 0.890500 | 0.976400 | 0.000000                      | 0.000000  | 0.000000 | 0.000000                    | 0.003000  | -0.000000 |
| 4   | Ca   | 0.509700                | 0.609500 | 0.523600 | 0.000000                      | 0.000000  | 0.000000 | -0.000000                   | -0.003000 | 0.000000  |
| 5   | Ca   | 0.009700                | 0.609500 | 0.976400 | 0.000000                      | 0.000000  | 0.000000 | 0.000000                    | -0.003000 | 0.000000  |
| 6   | Ca   | 0.509700                | 0.890500 | 0.523600 | 0.000000                      | 0.000000  | 0.000000 | 0.000000                    | 0.003000  | -0.000000 |
| 7   | Ca   | 0.990300                | 0.390500 | 0.023600 | 0.000000                      | 0.000000  | 0.000000 | 0.000000                    | -0.003000 | -0.000000 |
| 8   | Ca   | 0.490300                | 0.109500 | 0.476400 | 0.000000                      | 0.000000  | 0.000000 | -0.000000                   | 0.003000  | 0.000000  |
| 9   | Mn   | 0.000000                | 0.000000 | 0.500000 | 0.000000                      | 3.599930  | 0.000000 | -0.001000                   | 3.814000  | -0.001000 |
| 10  | Mn   | 0.500000                | 0.500000 | 0.000000 | 0.000000                      | -3.599930 | 0.000000 | -0.001000                   | -3.789000 | 0.001000  |
| 11  | Mn   | 0.000000                | 0.500000 | 0.500000 | 0.000000                      | -3.599930 | 0.000000 | 0.000000                    | -3.814000 | -0.001000 |
| 12  | Mn   | 0.500000                | 0.000000 | 0.000000 | 0.000000                      | 3.599930  | 0.000000 | 0.000000                    | 3.789000  | 0.001000  |
| 13  | Ga   | 0.972400                | 0.250000 | 0.565200 | 0.000000                      | 0.000000  | 0.000000 | 0.000000                    | 0.000000  | -0.000000 |
| 14  | Ga   | 0.472400                | 0.250000 | 0.934800 | 0.000000                      | 0.000000  | 0.000000 | -0.000000                   | 0.000000  | 0.000000  |
| 15  | Ga   | 0.027600                | 0.750000 | 0.434800 | 0.000000                      | 0.000000  | 0.000000 | 0.000000                    | -0.000000 | -0.000000 |
| 16  | Ga   | 0.527600                | 0.750000 | 0.065200 | 0.000000                      | 0.000000  | 0.000000 | -0.000000                   | -0.000000 | 0.000000  |
| 17  | O    | 0.748000                | 0.988600 | 0.238000 | 0.000000                      | 0.000000  | 0.000000 | -0.000000                   | -0.013000 | 0.000000  |
| 18  | O    | 0.248000                | 0.511400 | 0.262000 | 0.000000                      | 0.000000  | 0.000000 | 0.000000                    | 0.001000  | -0.000000 |
| 19  | O    | 0.252000                | 0.011400 | 0.762000 | 0.000000                      | 0.000000  | 0.000000 | 0.000000                    | -0.013000 | 0.000000  |
| 20  | O    | 0.752000                | 0.488600 | 0.738000 | 0.000000                      | 0.000000  | 0.000000 | 0.000000                    | 0.001000  | 0.000000  |
| 21  | O    | 0.252000                | 0.488600 | 0.762000 | 0.000000                      | 0.000000  | 0.000000 | -0.000000                   | 0.013000  | 0.000000  |
| 22  | O    | 0.752000                | 0.011400 | 0.738000 | 0.000000                      | 0.000000  | 0.000000 | 0.000000                    | -0.001000 | -0.000000 |
| 23  | O    | 0.748000                | 0.511400 | 0.238000 | 0.000000                      | 0.000000  | 0.000000 | 0.000000                    | 0.013000  | 0.000000  |
| 24  | O    | 0.248000                | 0.988600 | 0.262000 | 0.000000                      | 0.000000  | 0.000000 | 0.000000                    | -0.001000 | 0.000000  |
| 25  | O    | 0.517000                | 0.147000 | 0.067000 | 0.000000                      | 0.000000  | 0.000000 | -0.000000                   | 0.020000  | 0.000000  |
| 26  | O    | 0.017000                | 0.353000 | 0.433000 | 0.000000                      | 0.000000  | 0.000000 | 0.000000                    | -0.027000 | -0.000000 |
| 27  | O    | 0.483000                | 0.853000 | 0.933000 | 0.000000                      | 0.000000  | 0.000000 | 0.000000                    | 0.020000  | -0.000000 |
| 28  | O    | 0.983000                | 0.647000 | 0.567000 | 0.000000                      | 0.000000  | 0.000000 | -0.000000                   | -0.027000 | 0.000000  |
| 29  | O    | 0.483000                | 0.647000 | 0.933000 | 0.000000                      | 0.000000  | 0.000000 | -0.000000                   | -0.020000 | 0.000000  |
| 30  | O    | 0.983000                | 0.853000 | 0.567000 | 0.000000                      | 0.000000  | 0.000000 | 0.000000                    | 0.027000  | -0.000000 |
| 31  | O    | 0.517000                | 0.353000 | 0.067000 | 0.000000                      | 0.000000  | 0.000000 | 0.000000                    | -0.020000 | -0.000000 |
| 32  | O    | 0.017000                | 0.147000 | 0.433000 | 0.000000                      | 0.000000  | 0.000000 | -0.000000                   | 0.027000  | 0.000000  |
| 33  | O    | 0.102000                | 0.250000 | 0.877000 | 0.000000                      | 0.000000  | 0.000000 | -0.000000                   | 0.000000  | -0.000000 |
| 34  | O    | 0.602000                | 0.250000 | 0.623000 | 0.000000                      | 0.000000  | 0.000000 | 0.000000                    | -0.000000 | -0.000000 |
| 35  | O    | 0.898000                | 0.750000 | 0.123000 | 0.000000                      | 0.000000  | 0.000000 | -0.000000                   | -0.000000 | -0.000000 |
| 36  | O    | 0.398000                | 0.750000 | 0.377000 | 0.000000                      | 0.000000  | 0.000000 | 0.000000                    | 0.000000  | -0.000000 |

FIG. 89. First-principles calculation results of 0.825  $\text{Ca}_2\text{MnGaO}_5$ . The band structure is shown in the left panel, and the Fermi-level-dependent AHC is plotted in the right panel. In both plots, the Fermi level is set to 0 eV.

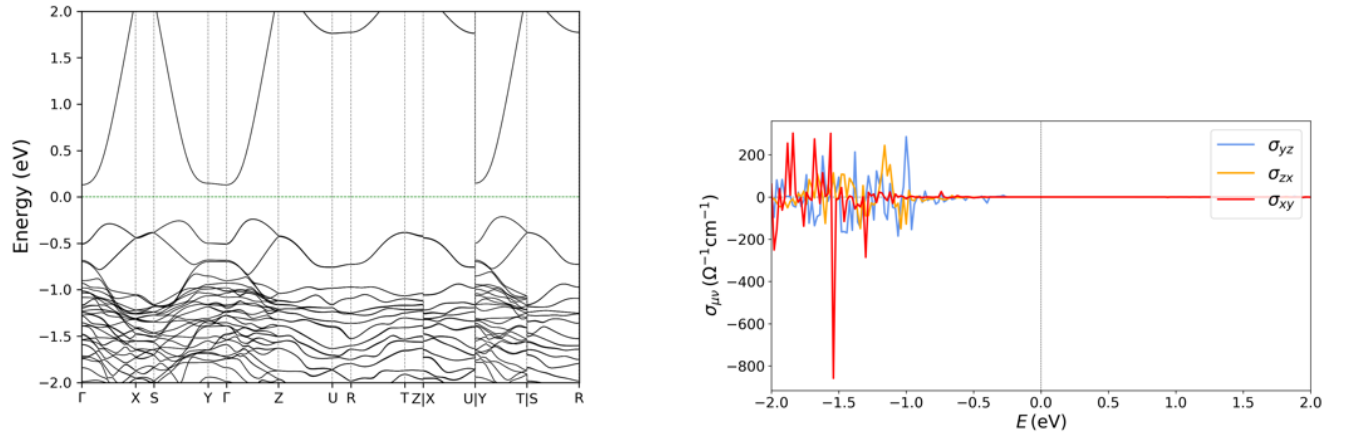

- 
- 
- [1] [https://cryst.ehu.es/cgi-bin/subperiodic/programs/nph-sub\\_wp](https://cryst.ehu.es/cgi-bin/subperiodic/programs/nph-sub_wp).
- [2] See the Supplemental Material I at XXX for all positions of all SNLs and FNSs in the 1651 MSGs for neglecting and considering SOC; the little groups of all the SNLs and FNSs; and all symmetry-related SNLs and FNSs.
